# Supplementary material for: The Complement Problem for Linklessly Embeddable Graphs
Source: arXiv:2108.12946 ancillary file (2022-08-16)
Supplement: Supplementary file 1 [file maxnillist-2.pdf]

## MaxnIL graphs of order up to 11

Order 6: 1 graph ( $K_6$  minus an edge):

$$\{\{1,2\},\{1,3\},\{1,4\},\{1,5\},\{1,6\},\{2,3\},\{2,4\},\{2,5\},\{2,6\},\{3,4\},\{3,5\},\{3,6\},\{4,5\},\{4,6\}\}$$

Order 7: 2 graphs, both are apex:

$$\begin{aligned} & \{\{1,3\},\{1,4\},\{1,5\},\{1,6\},\{1,7\},\{2,3\},\{2,4\},\{2,5\},\{2,6\},\{2,7\},\{3,5\}, \\ & \{3,6\},\{3,7\},\{4,5\},\{4,6\},\{4,7\},\{5,7\},\{6,7\}\}, \\ & \{\{1,3\},\{1,4\},\{1,5\},\{1,6\},\{1,7\},\{2,4\},\{2,5\},\{2,6\},\{2,7\},\{3,5\},\{3,6\}, \\ & \{3,7\},\{4,5\},\{4,6\},\{4,7\},\{5,6\},\{5,7\},\{6,7\}\} \end{aligned}$$

Order 8: 6 graphs, 5 of them apex:

$\{\{1,3\},\{1,4\},\{1,5\},\{1,7\},\{1,8\},\{2,4\},\{2,5\},\{2,6\},\{2,7\},\{2,8\},\{3,5\},$   
 $\{3,6\},\{3,7\},\{3,8\},\{4,6\},\{4,7\},\{4,8\},\{5,7\},\{5,8\},\{6,7\},\{6,8\}\},\{\{1,3\},$   
 $\{1,4\},\{1,5\},\{1,6\},\{1,7\},\{1,8\},\{2,4\},\{2,5\},\{2,6\},\{2,7\},\{2,8\},\{3,5\},$   
 $\{3,7\},\{3,8\},\{4,6\},\{4,7\},\{4,8\},\{5,6\},\{5,7\},\{5,8\},\{6,8\},\{7,8\}\},$   
 $\{\{1,3\},\{1,4\},\{1,6\},\{1,7\},\{1,8\},\{2,4\},\{2,5\},\{2,6\},\{2,7\},\{2,8\},\{3,5\},$   
 $\{3,6\},\{3,7\},\{3,8\},\{4,6\},\{4,7\},\{4,8\},\{5,6\},\{5,7\},\{5,8\},\{6,8\},\{7,8\}\},$   
 $\{\{1,3\},\{1,5\},\{1,6\},\{1,7\},\{1,8\},\{2,4\},\{2,5\},\{2,6\},\{2,7\},\{2,8\},\{3,5\},$   
 $\{3,7\},\{3,8\},\{4,6\},\{4,7\},\{4,8\},\{5,6\},\{5,7\},\{5,8\},\{6,7\},\{6,8\},\{7,8\}\},$   
 $\{\{1,4\},\{1,5\},\{1,6\},\{1,7\},\{1,8\},\{2,4\},\{2,6\},\{2,7\},\{2,8\},\{3,5\},\{3,6\},$   
 $\{3,7\},\{3,8\},\{4,6\},\{4,7\},\{4,8\},\{5,6\},\{5,7\},\{5,8\},\{6,7\},\{6,8\},\{7,8\}\},$   
 $\{\{1,4\},\{1,5\},\{1,7\},\{1,8\},\{2,4\},\{2,6\},\{2,7\},\{2,8\},\{3,5\},\{3,6\},\{3,7\},$   
 $\{3,8\},\{4,5\},\{4,6\},\{4,7\},\{4,8\},\{5,6\},\{5,7\},\{5,8\},\{6,7\},\{6,8\},\{7,8\}\}$

Order 9: 20 graphs, 14 of them are apex:

{1,3},{1,4},{1,6},{1,7},{1,9},{2,4},{2,5},{2,6},{2,7},{2,8},{2,9},  
{3,5},{3,6},{3,8},{3,9},{4,6},{4,7},{4,8},{5,7},{5,8},{5,9},{6,8},  
{6,9},{7,9}},{{1,4},{1,5},{1,6},{1,8},{1,9},{2,4},{2,7},{2,9},{3,5},  
{3,6},{3,7},{3,8},{3,9},{4,6},{4,7},{4,8},{4,9},{5,7},{5,8},{5,9},  
{6,8},{6,9},{7,8},{7,9}},{{1,4},{1,5},{1,7},{1,8},{1,9},{2,4},{2,6},  
{2,7},{2,8},{2,9},{3,5},{3,6},{3,8},{3,9},{4,6},{4,8},{4,9},{5,7},  
{5,8},{5,9},{6,8},{6,9},{7,8},{7,9}},{{1,3},{1,5},{1,6},{1,7},{1,8},  
{1,9},{2,4},{2,5},{2,6},{2,8},{2,9},{3,5},{3,7},{3,9},{4,6},{4,7},  
{4,8},{4,9},{5,7},{5,8},{5,9},{6,8},{6,9},{7,8},{7,9}},{{1,3},{1,5},  
{1,6},{1,7},{1,8},{2,4},{2,5},{2,7},{2,8},{2,9},{3,5},{3,6},{3,8},  
{3,9},{4,6},{4,7},{4,8},{4,9},{5,7},{5,8},{5,9},{6,7},{6,8},{6,9},  
{7,9}},{{1,3},{1,5},{1,6},{1,7},{1,8},{1,9},{2,4},{2,5},{2,6},{2,7},  
{2,8},{2,9},{3,5},{3,7},{3,9},{4,6},{4,8},{4,9},{5,7},{5,8},{5,9},  
{6,7},{6,8},{6,9},{7,9},{8,9}},{{1,3},{1,5},{1,6},{1,7},{1,8},{1,9},  
{2,4},{2,6},{2,7},{2,8},{2,9},{3,5},{3,7},{3,8},{3,9},{4,6},{4,7},  
{4,9},{5,8},{5,9},{6,7},{6,8},{6,9},{7,8},{7,9},{8,9}},{{1,3},{1,5},  
{1,6},{1,7},{1,8},{1,9},{2,4},{2,6},{2,7},{2,8},{2,9},{3,5},{3,7},  
{3,8},{3,9},{4,6},{4,8},{4,9},{5,8},{5,9},{6,7},{6,8},{6,9},{7,8},  
{7,9},{8,9}},{{1,3},{1,5},{1,6},{1,7},{1,9},{2,4},{2,5},{2,7},{2,8},  
{2,9},{3,5},{3,6},{3,8},{3,9},{4,6},{4,7},{4,8},{4,9},{5,7},{5,8},  
{5,9},{6,7},{6,8},{6,9},{7,9},{8,9}},{{1,3},{1,5},{1,6},{1,7},{1,9},  
{2,4},{2,6},{2,7},{2,8},{2,9},{3,5},{3,6},{3,8},{3,9},{4,6},{4,7},  
{4,8},{5,7},{5,8},{5,9},{6,7},{6,8},{6,9},{7,8},{7,9},{8,9}},{{1,3},



{5,8},{5,9},{6,8},{6,9},{6,10},{7,9},{7,10},{8,10},{1,4},{1,5},{1,7},{1,9},{1,10},{2,4},{2,6},{2,9},{2,10},{3,5},{3,6},{3,7},{3,8},{3,9},{3,10},{4,6},{4,7},{4,8},{4,10},{5,7},{5,8},{5,9},{6,8},{6,9},{7,8},{7,10},{9,10}},{1,4},{1,5},{1,7},{1,9},{1,10},{2,5},{2,6},{2,8},{2,9},{2,10},{3,6},{3,7},{3,9},{3,10},{4,8},{4,9},{4,10},{5,7},{5,9},{5,10},{6,8},{6,9},{6,10},{7,9},{7,10},{8,9},{8,10}},{1,4},{1,5},{1,8},{1,9},{1,10},{2,5},{2,6},{2,7},{2,9},{2,10},{3,6},{3,7},{3,8},{3,9},{3,10},{4,8},{4,10},{5,7},{5,9},{5,10},{6,8},{6,9},{6,10},{7,9},{7,10},{8,9},{8,10}},{1,4},{1,5},{1,9},{1,10},{2,5},{2,6},{2,7},{2,9},{2,10},{3,6},{3,7},{3,8},{3,9},{3,10},{4,8},{4,10},{5,7},{5,9},{5,10},{6,8},{6,9},{6,10},{7,9},{7,10},{8,9},{8,10}},{1,4},{1,5},{1,9},{1,10},{2,5},{2,6},{2,7},{2,9},{2,10},{3,6},{3,7},{3,8},{3,9},{3,10},{4,8},{4,9},{4,10},{5,7},{5,9},{5,10},{6,8},{6,9},{6,10},{7,9},{7,10},{8,9},{8,10}},{1,4},{1,7},{1,8},{1,9},{2,5},{2,6},{2,7},{2,9},{2,10},{3,5},{3,6},{3,8},{3,9},{3,10},{4,7},{4,8},{4,10},{5,7},{5,9},{5,10},{6,8},{6,9},{6,10},{7,9},{7,10},{8,9},{8,10}},{1,5},{1,6},{1,7},{1,8},{1,9},{2,5},{2,6},{2,8},{2,9},{2,10},{3,7},{3,8},{3,10},{4,7},{4,9},{4,10},{5,7},{5,8},{5,9},{6,8},{6,9},{6,10},{7,8},{7,9},{7,10},{8,10},{9,10}},{1,5},{1,6},{1,7},{1,8},{1,9},{2,6},{2,7},{2,9},{2,10},{3,6},{3,8},{3,9},{3,10},{4,7},{4,8},{4,9},{4,10},{5,6},{5,7},{5,8},{5,10},{6,9},{6,10},{7,9},{7,10},{8,9},{8,10}},{1,5},{1,6},{1,7},{1,9},{1,10},{2,5},{2,6},{2,8},{2,9},{3,5},{3,7},{3,8},{3,10},{4,6},{4,7},{4,8},{4,9},{4,10},{5,7},{5,8},{5,9},{6,8},{6,9},{6,10},{7,9},{7,10},{8,10}},{1,3},{1,5},{1,6},{1,8},{1,9},{1,10},{2,4},{2,6},{2,7},{2,8},{2,10},{3,5},{3,7},{3,8},{3,9},{3,10},{4,6},{4,7},{4,9},{4,10},{5,10},{6,8},{6,9},{6,10},{7,8},{7,9},{7,10},{8,9}},{1,3},{1,5},{1,6},{1,9},{1,10},{2,4},{2,6},{2,7},{2,8},{2,9},{3,5},{3,7},{3,9},{3,10},{4,6},{4,7},{4,8},{4,10},{5,8},{5,9},{5,10},{6,8},{6,9},{6,10},{7,9},{7,10},{8,9},{8,10}},{1,4},{1,5},{1,6},{1,8},{1,9},{1,10},{2,4},{2,7},{2,8},{2,9},{3,5},{3,6},{3,7},{3,8},{3,9},{3,10},{4,6},{4,7},{4,8},{4,10},{5,7},{5,9},{5,10},{6,8},{6,10},{7,9},{7,10},{8,9}},{1,4},{1,5},{1,6},{1,8},{1,9},{1,10},{2,4},{2,7},{2,8},{2,9},{3,5},{3,6},{3,7},{3,8},{3,9},{3,10},{4,6},{4,7},{4,8},{4,10},{5,7},{5,9},{5,10},{6,8},{6,10},{7,9},{7,10},{8,9}},{1,4},{1,5},{1,7},{1,8},{1,9},{1,10},{2,4},{2,6},{2,7},{2,8},{2,9},{3,7},{3,9},{3,10},{4,6},{4,8},{4,10},{5,7},{5,9},{5,10},{6,8},{6,9},{6,10},{7,8},{7,9},{7,10},{8,9}},{1,4},{1,5},{1,7},{1,8},{1,9},{1,10},{2,4},{2,6},{2,7},{2,8},{2,9},{3,7},{3,9},{3,10},{4,6},{4,8},{4,10},{5,7},{5,9},{5,10},{6,8},{6,9},{6,10},{7,8},{7,9},{7,10},{8,9}},{1,4},{1,5},{1,7},{1,8},{1,9},{1,10},{2,4},{2,6},{2,7},{2,8},{2,9},{3,5},{3,6},{3,7},{3,8},{3,9},{3,10},{4,6},{4,7},{4,8},{4,9},{4,10},{5,7},{5,8},{5,9},{5,10},{6,7},{6,8},{6,9},{6,10},{7,9},{7,10},{8,9},{9,10}},{1,4},{1,6},{1,7},

{1,9},{1,10},{2,5},{2,6},{2,8},{2,10},{3,5},{3,7},{3,9},{3,10},{4,7},  
{4,8},{4,9},{4,10},{5,6},{5,8},{5,9},{5,10},{6,8},{6,9},{6,10},{7,9},  
{7,10},{8,9},{8,10}},{{1,4},{1,6},{1,8},{1,9},{1,10},{2,5},{2,6},  
{2,7},{2,8},{2,10},{3,5},{3,9},{3,10},{4,7},{4,8},{4,9},{4,10},{5,6},  
{5,7},{5,9},{5,10},{6,7},{6,8},{6,9},{7,8},{7,9},{8,10},{9,10}},  
{{1,4},{1,7},{1,8},{1,10},{2,5},{2,6},{2,7},{2,9},{2,10},{3,5},{3,6},  
{3,8},{3,9},{3,10},{4,7},{4,8},{4,10},{5,7},{5,9},{5,10},{6,8},{6,9},  
{6,10},{7,8},{7,9},{7,10},{8,9},{8,10}},{{1,3},{1,5},{1,6},{1,7},  
{1,8},{1,9},{1,10},{2,4},{2,6},{2,7},{2,9},{2,10},{3,5},{3,7},{3,8},  
{3,10},{4,6},{4,8},{4,9},{4,10},{5,7},{5,8},{6,9},{6,10},{7,8},{7,9},  
{7,10},{8,9},{8,10}},{{1,3},{1,5},{1,6},{1,7},{1,8},{1,10},{2,4},  
{2,6},{2,7},{2,8},{2,9},{2,10},{3,5},{3,7},{3,8},{3,9},{4,6},{4,9},  
{4,10},{5,7},{5,9},{5,10},{6,8},{6,9},{6,10},{7,8},{7,10},{8,9},  
{9,10}},{{1,3},{1,5},{1,6},{1,7},{1,9},{1,10},{2,4},{2,6},{2,7},{2,8},  
{2,9},{2,10},{3,5},{3,7},{3,8},{3,9},{3,10},{4,6},{4,8},{4,9},{5,7},  
{5,10},{6,8},{6,9},{6,10},{7,9},{7,10},{8,9},{8,10}},{{1,3},{1,5},  
{1,6},{1,7},{1,9},{1,10},{2,4},{2,6},{2,7},{2,8},{2,9},{2,10},{3,5},  
{3,7},{3,8},{3,9},{3,10},{4,6},{4,8},{4,10},{5,7},{5,10},{6,8},{6,9},  
{6,10},{7,9},{7,10},{8,9},{8,10}},{{1,3},{1,5},{1,6},{1,8},{1,9},  
{1,10},{2,4},{2,6},{2,7},{2,8},{2,9},{3,5},{3,7},{3,8},{3,9},{3,10},  
{4,6},{4,7},{4,9},{4,10},{5,8},{5,10},{6,8},{6,9},{6,10},{7,8},{7,9},  
{7,10},{8,10}},{{1,4},{1,5},{1,7},{1,9},{1,10},{2,4},{2,6},{2,7},  
{2,8},{2,9},{2,10},{3,5},{3,6},{3,8},{3,9},{3,10},{4,7},{4,9},{4,10},  
{5,7},{5,8},{5,9},{5,10},{6,8},{6,9},{6,10},{7,8},{7,9},{8,10}},  
{{1,4},{1,6},{1,7},{1,8},{1,9},{2,5},{2,6},{2,8},{2,9},{2,10},{3,5},  
{3,7},{3,8},{3,9},{3,10},{4,6},{4,7},{4,9},{4,10},{5,8},{5,9},{5,10},  
{6,8},{6,9},{6,10},{7,8},{7,9},{7,10},{8,10}},{{1,4},{1,6},{1,7},  
{1,8},{1,9},{2,5},{2,7},{2,8},{2,10},{3,5},{3,7},{3,9},{3,10},{4,6},  
{4,8},{4,9},{4,10},{5,6},{5,7},{5,8},{5,9},{5,10},{6,8},{6,9},{7,8},  
{7,9},{7,10},{8,10},{9,10}},{{1,4},{1,6},{1,7},{1,8},{1,10},{2,5},  
{2,6},{2,7},{2,8},{2,9},{2,10},{3,5},{3,8},{3,9},{3,10},{4,6},{4,7},  
{4,9},{4,10},{5,8},{5,9},{5,10},{6,7},{6,8},{6,9},{7,10},{8,9},{8,10},  
{9,10}},{{1,4},{1,6},{1,7},{1,9},{1,10},{2,5},{2,6},{2,7},{2,8},{2,9},  
{3,5},{3,6},{3,8},{3,10},{4,7},{4,8},{4,9},{4,10},{5,6},{5,7},{5,8},  
{5,10},{6,8},{6,9},{6,10},{7,9},{7,10},{8,9},{8,10}},{{1,3},{1,5},  
{1,6},{1,7},{1,8},{1,9},{1,10},{2,4},{2,6},{2,7},{2,8},{2,9},{2,10},  
{3,5},{3,7},{3,9},{3,10},{4,6},{4,8},{4,10},{5,7},{5,9},{6,8},{6,9},  
{6,10},{7,8},{7,9},{7,10},{8,10},{9,10}},{{1,3},{1,5},{1,6},{1,8},  
{1,9},{1,10},{2,4},{2,6},{2,7},{2,8},{2,10},{3,5},{3,7},{3,8},{3,9},  
{3,10},{4,6},{4,7},{4,9},{4,10},{5,9},{5,10},{6,8},{6,9},{6,10},{7,8},  
{7,9},{7,10},{8,10},{9,10}},{{1,3},{1,5},{1,7},{1,8},{1,9},{1,10},  
{2,4},{2,6},{2,7},{2,8},{2,9},{2,10},{3,5},{3,7},{3,9},{3,10},{4,6},  
{4,8},{4,9},{4,10},{5,7},{5,9},{6,8},{6,10},{7,8},{7,9},{7,10},{8,9},  
{8,10},{9,10}},{{1,3},{1,5},{1,7},{1,8},{1,9},{1,10},{2,4},{2,6},  
{2,7},{2,8},{2,9},{2,10},{3,5},{3,7},{3,9},{3,10},{4,6},{4,8},{4,9},  
{4,10},{5,7},{5,10},{6,8},{6,10},{7,8},{7,9},{7,10},{8,9},{8,10},  
{9,10}},{{1,3},{1,5},{1,7},{1,8},{1,9},{2,4},{2,6},{2,7},{2,8},{2,9},  
{2,10},{3,5},{3,7},{3,8},{3,10},{4,6},{4,8},{4,9},{4,10},{5,7},{5,9},  
{5,10},{6,9},{6,10},{7,8},{7,9},{7,10},{8,9},{8,10},{9,10}},{{1,3},  
{1,5},{1,7},{1,8},{1,9},{2,4},{2,6},{2,7},{2,8},{2,10},{3,5},{3,7},

{3,9},{3,10},{4,6},{4,7},{4,9},{4,10},{5,8},{5,9},{5,10},{6,8},{6,9},  
{6,10},{7,8},{7,9},{7,10},{8,9},{8,10},{9,10}},{{1,3},{1,5},{1,7},  
{1,8},{1,10},{2,4},{2,6},{2,7},{2,8},{2,10},{3,5},{3,7},{3,9},{3,10},  
{4,6},{4,7},{4,9},{4,10},{5,8},{5,9},{5,10},{6,8},{6,9},{6,10},{7,8},  
{7,9},{7,10},{8,9},{8,10},{9,10}},{{1,4},{1,5},{1,7},{1,8},{1,9},  
{1,10},{2,5},{2,6},{2,7},{2,8},{2,9},{2,10},{3,6},{3,8},{3,9},{3,10},  
{4,7},{4,9},{4,10},{5,7},{5,8},{5,10},{6,8},{6,9},{6,10},{7,9},{7,10},  
{8,9},{8,10},{9,10}},{{1,4},{1,5},{1,7},{1,8},{1,9},{1,10},{2,5},  
{2,6},{2,8},{2,9},{2,10},{3,6},{3,7},{3,8},{3,9},{3,10},{4,7},{4,9},  
{4,10},{5,8},{5,9},{5,10},{6,8},{6,9},{6,10},{7,8},{7,9},{7,10},  
{8,10},{9,10}},{{1,4},{1,5},{1,7},{1,8},{1,9},{1,10},{2,5},{2,6},  
{2,8},{2,9},{2,10},{3,6},{3,7},{3,8},{3,10},{4,7},{4,9},{4,10},{5,8},  
{5,9},{5,10},{6,7},{6,8},{6,9},{6,10},{7,8},{7,9},{7,10},{8,10},  
{9,10}},{{1,4},{1,5},{1,7},{1,8},{1,9},{1,10},{2,5},{2,6},{2,8},{2,9},  
{2,10},{3,6},{3,7},{3,9},{3,10},{4,7},{4,9},{4,10},{5,8},{5,9},{5,10},  
{6,7},{6,8},{6,9},{6,10},{7,8},{7,9},{7,10},{8,10},{9,10}},{{1,4},  
{1,5},{1,7},{1,8},{1,9},{1,10},{2,6},{2,7},{2,8},{2,9},{2,10},{3,6},  
{3,7},{3,9},{3,10},{4,5},{4,8},{4,9},{4,10},{5,8},{5,10},{6,7},{6,9},  
{6,10},{7,8},{7,9},{7,10},{8,9},{8,10},{9,10}},{{1,4},{1,5},{1,7},  
{1,8},{1,9},{1,10},{2,6},{2,7},{2,8},{2,9},{2,10},{3,6},{3,8},{3,9},  
{3,10},{4,5},{4,7},{4,9},{4,10},{5,9},{5,10},{6,8},{6,9},{6,10},{7,8},  
{7,9},{7,10},{8,9},{8,10},{9,10}},{{1,4},{1,5},{1,7},{1,8},{1,9},  
{1,10},{2,6},{2,7},{2,8},{2,9},{3,6},{3,7},{3,8},{3,10},{4,5},{4,8},  
{4,9},{4,10},{5,9},{5,10},{6,7},{6,8},{6,9},{6,10},{7,8},{7,9},{7,10},  
{8,9},{8,10},{9,10}},{{1,4},{1,5},{1,7},{1,8},{1,9},{1,10},{2,6},  
{2,7},{2,8},{2,10},{3,6},{3,7},{3,9},{3,10},{4,5},{4,8},{4,9},{4,10},  
{5,9},{5,10},{6,7},{6,8},{6,9},{6,10},{7,8},{7,9},{7,10},{8,9},{8,10},  
{9,10}},{{1,4},{1,5},{1,7},{1,8},{1,9},{2,6},{2,7},{2,8},{2,9},{2,10},  
{3,6},{3,8},{3,9},{3,10},{4,5},{4,7},{4,8},{4,10},{5,7},{5,9},{5,10},  
{6,8},{6,9},{6,10},{7,8},{7,9},{7,10},{8,9},{8,10},{9,10}},{{1,4},  
{1,5},{1,7},{1,8},{1,9},{2,6},{2,7},{2,9},{2,10},{3,6},{3,8},{3,9},  
{3,10},{4,5},{4,7},{4,8},{4,10},{5,8},{5,9},{5,10},{6,7},{6,8},{6,9},  
{6,10},{7,8},{7,9},{7,10},{8,9},{8,10},{9,10}},{{1,4},{1,5},{1,7},  
{1,8},{1,10},{2,4},{2,6},{2,7},{2,9},{2,10},{3,5},{3,6},{3,8},{3,9},  
{3,10},{4,6},{4,7},{4,8},{4,10},{5,7},{5,8},{5,9},{5,10},{6,8},{6,9},  
{6,10},{7,9},{7,10},{8,10},{9,10}},{{1,4},{1,5},{1,7},{1,8},{1,10},  
{2,6},{2,7},{2,8},{2,9},{2,10},{3,6},{3,8},{3,9},{3,10},{4,5},{4,7},  
{4,9},{4,10},{5,8},{5,9},{5,10},{6,8},{6,9},{6,10},{7,8},{7,9},{7,10},  
{8,9},{8,10},{9,10}},{{1,4},{1,5},{1,7},{1,8},{1,10},{2,6},{2,7},  
{2,9},{2,10},{3,6},{3,8},{3,9},{3,10},{4,5},{4,7},{4,9},{4,10},{5,8},  
{5,9},{5,10},{6,7},{6,8},{6,9},{6,10},{7,8},{7,9},{7,10},{8,9},{8,10},  
{9,10}},{{1,4},{1,5},{1,7},{1,9},{1,10},{2,4},{2,6},{2,7},{2,8},{2,9},  
{2,10},{3,5},{3,6},{3,8},{3,9},{3,10},{4,7},{4,9},{4,10},{5,7},{5,8},  
{5,9},{5,10},{6,8},{6,9},{6,10},{7,8},{7,10},{8,10},{9,10}},{{1,4},  
{1,5},{1,7},{1,9},{1,10},{2,5},{2,6},{2,7},{2,8},{2,9},{2,10},{3,6},  
{3,8},{3,9},{3,10},{4,7},{4,9},{4,10},{5,7},{5,8},{5,9},{5,10},{6,8},  
{6,9},{6,10},{7,9},{7,10},{8,9},{8,10},{9,10}},{{1,4},{1,5},{1,7},  
{1,9},{1,10},{2,5},{2,6},{2,8},{2,9},{2,10},{3,6},{3,7},{3,8},{3,9},  
{3,10},{4,7},{4,9},{4,10},{5,7},{5,8},{5,9},{5,10},{6,8},{6,9},{6,10},  
{7,8},{7,9},{7,10},{8,10},{9,10}},{{1,4},{1,5},{1,8},{1,9},{1,10},

{2,5},{2,6},{2,8},{2,9},{2,10},{3,6},{3,7},{3,8},{3,9},{3,10},{4,7},  
{4,8},{4,9},{4,10},{5,8},{5,9},{5,10},{6,8},{6,9},{6,10},{7,8},{7,9},  
{7,10},{8,10},{9,10}},{{1,4},{1,6},{1,7},{1,8},{1,9},{1,10},{2,5},  
{2,6},{2,7},{2,8},{2,9},{2,10},{3,5},{3,8},{3,9},{3,10},{4,6},{4,7},  
{4,10},{5,8},{5,9},{5,10},{6,7},{6,8},{6,10},{7,9},{7,10},{8,9},  
{8,10},{9,10}},{{1,4},{1,6},{1,7},{1,8},{1,9},{1,10},{2,5},{2,6},  
{2,8},{2,10},{3,5},{3,7},{3,8},{3,9},{3,10},{4,7},{4,9},{4,10},{5,6},  
{5,8},{5,9},{5,10},{6,8},{6,9},{6,10},{7,8},{7,9},{7,10},{8,10},  
{9,10}},{{1,4},{1,6},{1,7},{1,8},{1,9},{1,10},{2,5},{2,6},{2,8},  
{2,10},{3,5},{3,7},{3,9},{3,10},{4,8},{4,9},{4,10},{5,6},{5,7},{5,8},  
{5,9},{5,10},{6,7},{6,8},{6,10},{7,9},{7,10},{8,9},{8,10},{9,10}},  
{{1,4},{1,6},{1,7},{1,8},{1,9},{1,10},{2,5},{2,6},{2,9},{2,10},{3,5},  
{3,7},{3,8},{3,9},{3,10},{4,7},{4,9},{4,10},{5,6},{5,8},{5,9},{5,10},  
{6,8},{6,9},{6,10},{7,8},{7,9},{7,10},{8,10},{9,10}},{{1,4},{1,6},  
{1,7},{1,8},{1,9},{1,10},{2,5},{2,7},{2,8},{2,9},{2,10},{3,6},{3,8},  
{3,9},{3,10},{4,6},{4,8},{4,10},{5,7},{5,9},{5,10},{6,8},{6,9},{6,10},  
{7,8},{7,9},{7,10},{8,9},{8,10},{9,10}},{{1,4},{1,6},{1,7},{1,8},  
{1,9},{1,10},{2,5},{2,7},{2,8},{2,9},{2,10},{3,6},{3,8},{3,9},{3,10},  
{4,6},{4,9},{4,10},{5,7},{5,9},{5,10},{6,8},{6,9},{6,10},{7,8},{7,9},  
{7,10},{8,9},{8,10},{9,10}},{{1,4},{1,6},{1,7},{1,8},{1,9},{1,10},  
{2,5},{2,7},{2,8},{2,9},{2,10},{3,6},{3,8},{3,9},{3,10},{4,7},{4,8},  
{4,10},{5,7},{5,9},{5,10},{6,8},{6,9},{6,10},{7,8},{7,9},{7,10},{8,9},  
{8,10},{9,10}},{{1,4},{1,6},{1,7},{1,8},{1,9},{1,10},{2,5},{2,7},  
{2,8},{2,9},{2,10},{3,6},{3,8},{3,9},{3,10},{4,7},{4,9},{4,10},{5,7},  
{5,9},{5,10},{6,8},{6,9},{6,10},{7,8},{7,9},{7,10},{8,9},{8,10},  
{9,10}},{{1,4},{1,6},{1,7},{1,8},{1,9},{1,10},{2,5},{2,7},{2,8},{2,9},  
{2,10},{3,6},{3,8},{3,9},{3,10},{4,7},{4,9},{4,10},{5,8},{5,9},{5,10},  
{6,8},{6,9},{6,10},{7,8},{7,9},{7,10},{8,9},{8,10},{9,10}},{{1,4},  
{1,6},{1,7},{1,8},{1,9},{1,10},{2,5},{2,7},{2,8},{2,10},{3,5},{3,7},  
{3,9},{3,10},{4,6},{4,9},{4,10},{5,6},{5,7},{5,8},{5,9},{5,10},{6,8},  
{6,9},{6,10},{7,8},{7,9},{7,10},{8,10},{9,10}},{{1,4},{1,6},{1,7},  
{1,8},{1,9},{2,5},{2,7},{2,8},{2,9},{2,10},{3,6},{3,8},{3,9},{3,10},  
{4,6},{4,7},{4,8},{4,10},{5,7},{5,9},{5,10},{6,8},{6,9},{6,10},{7,8},  
{7,9},{7,10},{8,9},{8,10},{9,10}},{{1,4},{1,6},{1,7},{1,8},{1,10},  
{2,5},{2,6},{2,7},{2,9},{2,10},{3,5},{3,8},{3,9},{3,10},{4,7},{4,8},  
{4,9},{4,10},{5,6},{5,8},{5,9},{5,10},{6,7},{6,8},{6,10},{7,9},{7,10},  
{8,9},{8,10},{9,10}},{{1,4},{1,6},{1,7},{1,8},{1,10},{2,5},{2,6},  
{2,8},{2,9},{2,10},{3,5},{3,7},{3,8},{3,9},{3,10},{4,6},{4,7},{4,9},  
{4,10},{5,8},{5,9},{5,10},{6,8},{6,9},{6,10},{7,8},{7,9},{7,10},  
{8,10},{9,10}},{{1,4},{1,6},{1,7},{1,8},{1,10},{2,5},{2,6},{2,8},  
{2,9},{2,10},{3,6},{3,7},{3,9},{3,10},{4,7},{4,8},{4,9},{4,10},{5,8},  
{5,9},{5,10},{6,7},{6,8},{6,9},{6,10},{7,9},{7,10},{8,9},{8,10},  
{9,10}},{{1,4},{1,6},{1,7},{1,8},{1,10},{2,5},{2,7},{2,8},{2,9},  
{2,10},{3,6},{3,8},{3,9},{3,10},{4,6},{4,7},{4,9},{4,10},{5,8},{5,9},  
{5,10},{6,8},{6,9},{6,10},{7,8},{7,9},{7,10},{8,9},{8,10},{9,10}},  
{{1,4},{1,6},{1,8},{1,9},{1,10},{2,5},{2,7},{2,8},{2,9},{2,10},{3,6},  
{3,7},{3,8},{3,9},{3,10},{4,6},{4,8},{4,10},{5,7},{5,9},{5,10},{6,8},  
{6,9},{6,10},{7,8},{7,9},{7,10},{8,9},{8,10},{9,10}},{{1,4},{1,6},  
{1,8},{1,9},{1,10},{2,5},{2,7},{2,8},{2,9},{2,10},{3,6},{3,7},{3,8},  
{3,9},{3,10},{4,6},{4,9},{4,10},{5,7},{5,9},{5,10},{6,8},{6,9},{6,10}

{7,8},{7,9},{7,10},{8,9},{8,10},{9,10},{1,4},{1,6},{1,8},{1,9},  
{1,10},{2,5},{2,7},{2,8},{2,9},{2,10},{3,6},{3,7},{3,8},{3,9},{3,10},  
{4,8},{4,9},{4,10},{5,7},{5,9},{5,10},{6,8},{6,9},{6,10},{7,8},{7,9},  
{7,10},{8,9},{8,10},{9,10}},{{1,4},{1,6},{1,8},{1,9},{1,10},{2,5},  
{2,7},{2,8},{2,9},{2,10},{3,6},{3,7},{3,8},{3,9},{4,6},{4,8},{4,10},  
{5,7},{5,9},{5,10},{6,7},{6,8},{6,9},{6,10},{7,8},{7,9},{7,10},{8,9},  
{8,10},{9,10}},{{1,4},{1,6},{1,8},{1,9},{1,10},{2,5},{2,7},{2,8},  
{2,9},{2,10},{3,6},{3,7},{3,8},{3,10},{4,6},{4,9},{4,10},{5,7},{5,9},  
{5,10},{6,7},{6,8},{6,9},{6,10},{7,8},{7,9},{7,10},{8,9},{8,10},  
{9,10}},{{1,4},{1,6},{1,8},{1,9},{1,10},{2,5},{2,7},{2,8},{2,9},  
{2,10},{3,6},{3,7},{3,9},{3,10},{4,6},{4,8},{4,10},{5,7},{5,9},{5,10},  
{6,7},{6,8},{6,9},{6,10},{7,8},{7,9},{7,10},{8,9},{8,10},{9,10}},  
{{1,4},{1,7},{1,8},{1,9},{1,10},{2,5},{2,6},{2,7},{2,8},{2,9},{2,10},  
{3,5},{3,6},{3,8},{3,9},{3,10},{4,7},{4,8},{4,9},{5,6},{5,8},{5,10},  
{6,9},{6,10},{7,8},{7,9},{7,10},{8,9},{8,10},{9,10}},{{1,4},{1,7},  
{1,8},{1,9},{1,10},{2,5},{2,6},{2,7},{2,8},{2,9},{2,10},{3,5},{3,6},  
{3,8},{3,9},{3,10},{4,7},{4,9},{4,10},{5,6},{5,8},{5,10},{6,9},{6,10},  
{7,8},{7,9},{7,10},{8,9},{8,10},{9,10}},{{1,4},{1,7},{1,8},{1,9},  
{1,10},{2,5},{2,6},{2,7},{2,8},{2,9},{2,10},{3,5},{3,6},{3,9},{3,10},  
{4,7},{4,8},{4,10},{5,6},{5,8},{5,9},{5,10},{6,9},{6,10},{7,8},{7,9},  
{7,10},{8,9},{8,10},{9,10}},{{1,4},{1,7},{1,8},{1,9},{1,10},{2,5},  
{2,6},{2,7},{2,8},{2,9},{3,5},{3,6},{3,9},{3,10},{4,7},{4,8},{4,10},  
{5,6},{5,7},{5,9},{5,10},{6,8},{6,9},{6,10},{7,8},{7,9},{7,10},{8,9},  
{8,10},{9,10}},{{1,4},{1,7},{1,8},{1,9},{1,10},{2,5},{2,6},{2,7},  
{2,8},{2,10},{3,5},{3,6},{3,9},{3,10},{4,7},{4,8},{4,10},{5,6},{5,7},  
{5,9},{5,10},{6,8},{6,9},{6,10},{7,8},{7,9},{7,10},{8,9},{8,10},  
{9,10}},{{1,4},{1,7},{1,8},{1,9},{1,10},{2,5},{2,6},{2,7},{2,9},  
{2,10},{3,5},{3,6},{3,8},{3,9},{3,10},{4,7},{4,8},{4,9},{5,6},{5,7},  
{5,8},{5,10},{6,9},{6,10},{7,8},{7,9},{7,10},{8,9},{8,10},{9,10}},  
{{1,4},{1,7},{1,8},{1,9},{1,10},{2,5},{2,6},{2,7},{2,9},{2,10},{3,5},  
{3,6},{3,8},{3,9},{3,10},{4,7},{4,8},{4,10},{5,6},{5,7},{5,8},{5,10},  
{6,9},{6,10},{7,8},{7,9},{7,10},{8,9},{8,10},{9,10}},{{1,5},{1,6},  
{1,7},{1,8},{1,9},{1,10},{2,5},{2,7},{2,9},{2,10},{3,6},{3,8},{3,9},  
{3,10},{4,7},{4,8},{4,9},{4,10},{5,7},{5,9},{5,10},{6,8},{6,9},{6,10},  
{7,8},{7,9},{7,10},{8,9},{8,10},{9,10}},{{1,5},{1,6},{1,7},{1,8},  
{1,10},{2,5},{2,7},{2,9},{2,10},{3,6},{3,8},{3,9},{3,10},{4,7},{4,8},  
{4,9},{4,10},{5,6},{5,7},{5,9},{5,10},{6,8},{6,9},{6,10},{7,8},{7,9},  
{7,10},{8,9},{8,10},{9,10}},{{1,5},{1,6},{1,8},{1,9},{1,10},{2,5},  
{2,7},{2,8},{2,9},{2,10},{3,6},{3,7},{3,8},{3,10},{4,6},{4,7},{4,9},  
{4,10},{5,8},{5,9},{5,10},{6,7},{6,8},{6,9},{6,10},{7,8},{7,9},{7,10},  
{8,10},{9,10}},{{1,5},{1,6},{1,8},{1,9},{1,10},{2,5},{2,7},{2,8},  
{2,9},{2,10},{3,6},{3,8},{3,9},{3,10},{4,7},{4,8},{4,9},{4,10},{5,8},  
{5,9},{5,10},{6,8},{6,9},{6,10},{7,8},{7,9},{7,10},{8,9},{8,10},  
{9,10}},{{1,5},{1,7},{1,8},{1,9},{1,10},{2,5},{2,7},{2,9},{2,10},  
{3,6},{3,7},{3,8},{3,9},{3,10},{4,6},{4,8},{4,9},{4,10},{5,7},{5,9},  
{5,10},{6,8},{6,9},{6,10},{7,8},{7,9},{7,10},{8,9},{8,10},{9,10}},  
{{1,5},{1,7},{1,8},{1,9},{1,10},{2,6},{2,7},{2,8},{2,9},{3,6},{3,7},  
{3,8},{3,10},{4,6},{4,7},{4,9},{4,10},{5,8},{5,9},{5,10},{6,7},{6,8},  
{6,9},{6,10},{7,8},{7,9},{7,10},{8,9},{8,10},{9,10}},{{1,5},{1,7},  
{1,8},{1,9},{1,10},{2,6},{2,7},{2,8},{2,10},{3,6},{3,7},{3,9},{3,10}

$\{4,6\}, \{4,8\}, \{4,9\}, \{4,10\}, \{5,8\}, \{5,9\}, \{5,10\}, \{6,7\}, \{6,8\}, \{6,9\}, \{6,10\},$   
 $\{7,8\}, \{7,9\}, \{7,10\}, \{8,9\}, \{8,10\}, \{9,10\}, \{\{1,5\}, \{1,7\}, \{1,8\}, \{1,9\},$   
 $\{2,5\}, \{2,7\}, \{2,8\}, \{2,10\}, \{3,6\}, \{3,7\}, \{3,9\}, \{3,10\}, \{4,6\}, \{4,8\}, \{4,9\},$   
 $\{4,10\}, \{5,7\}, \{5,8\}, \{5,9\}, \{5,10\}, \{6,7\}, \{6,8\}, \{6,9\}, \{6,10\}, \{7,8\}, \{7,9\},$   
 $\{7,10\}, \{8,9\}, \{8,10\}, \{9,10\}, \{\{1,5\}, \{1,7\}, \{1,8\}, \{1,10\}, \{2,5\}, \{2,7\},$   
 $\{2,9\}, \{2,10\}, \{3,6\}, \{3,7\}, \{3,8\}, \{3,9\}, \{3,10\}, \{4,6\}, \{4,8\}, \{4,9\}, \{4,10\},$   
 $\{5,7\}, \{5,8\}, \{5,9\}, \{5,10\}, \{6,8\}, \{6,9\}, \{6,10\}, \{7,8\}, \{7,9\}, \{7,10\}, \{8,9\},$   
 $\{8,10\}, \{9,10\}, \{\{1,5\}, \{1,7\}, \{1,8\}, \{1,10\}, \{2,5\}, \{2,8\}, \{2,9\}, \{2,10\},$   
 $\{3,6\}, \{3,7\}, \{3,9\}, \{3,10\}, \{4,6\}, \{4,8\}, \{4,9\}, \{4,10\}, \{5,7\}, \{5,8\}, \{5,9\},$   
 $\{5,10\}, \{6,7\}, \{6,8\}, \{6,9\}, \{6,10\}, \{7,8\}, \{7,9\}, \{7,10\}, \{8,9\}, \{8,10\},$   
 $\{9,10\}, \{\{1,5\}, \{1,7\}, \{1,9\}, \{1,10\}, \{2,5\}, \{2,8\}, \{2,9\}, \{2,10\}, \{3,6\},$   
 $\{3,7\}, \{3,8\}, \{3,9\}, \{3,10\}, \{4,6\}, \{4,8\}, \{4,9\}, \{4,10\}, \{5,7\}, \{5,8\}, \{5,9\},$   
 $\{5,10\}, \{6,8\}, \{6,9\}, \{6,10\}, \{7,8\}, \{7,9\}, \{7,10\}, \{8,9\}, \{8,10\}, \{9,10\},$   
 $\{\{1,5\}, \{1,7\}, \{1,9\}, \{1,10\}, \{2,5\}, \{2,8\}, \{2,9\}, \{2,10\}, \{3,6\}, \{3,7\}, \{3,9\},$   
 $\{3,10\}, \{4,6\}, \{4,8\}, \{4,9\}, \{4,10\}, \{5,7\}, \{5,8\}, \{5,9\}, \{5,10\}, \{6,7\}, \{6,8\},$   
 $\{6,9\}, \{6,10\}, \{7,8\}, \{7,9\}, \{7,10\}, \{8,9\}, \{8,10\}, \{9,10\}, \{\{1,6\}, \{1,7\},$   
 $\{1,8\}, \{1,9\}, \{2,6\}, \{2,7\}, \{2,8\}, \{2,10\}, \{3,6\}, \{3,7\}, \{3,9\}, \{3,10\}, \{4,6\},$   
 $\{4,8\}, \{4,9\}, \{4,10\}, \{5,7\}, \{5,8\}, \{5,9\}, \{5,10\}, \{6,7\}, \{6,8\}, \{6,9\}, \{6,10\},$   
 $\{7,8\}, \{7,9\}, \{7,10\}, \{8,9\}, \{8,10\}, \{9,10\}\}$

Order 11: 709 graphs, 233 of them are apex:

$\{\{1,2\}, \{1,3\}, \{1,6\}, \{1,7\}, \{1,8\}, \{1,9\}, \{1,10\}, \{1,11\}, \{2,3\}, \{2,4\}, \{2,5\},$   
 $\{2,6\}, \{2,8\}, \{2,9\}, \{2,10\}, \{3,4\}, \{3,6\}, \{3,7\}, \{3,8\}, \{3,9\}, \{3,10\}, \{3,11\},$   
 $\{4,5\}, \{4,6\}, \{4,8\}, \{5,6\}, \{5,8\}, \{6,8\}, \{6,9\}, \{7,8\}, \{7,10\}, \{7,11\}, \{8,10\},$   
 $\{8,11\}, \{\{1,2\}, \{1,3\}, \{1,5\}, \{1,6\}, \{1,7\}, \{1,8\}, \{1,9\}, \{1,11\}, \{2,3\}, \{2,7\},$   
 $\{2,10\}, \{2,11\}, \{3,4\}, \{3,7\}, \{3,8\}, \{3,10\}, \{4,5\}, \{4,7\}, \{4,8\}, \{4,10\},$   
 $\{4,11\}, \{5,6\}, \{5,7\}, \{5,8\}, \{5,9\}, \{5,11\}, \{6,7\}, \{6,9\}, \{6,11\}, \{7,8\}, \{7,9\},$   
 $\{7,10\}, \{7,11\}, \{10,11\}, \{\{1,2\}, \{1,3\}, \{1,6\}, \{1,7\}, \{1,8\}, \{1,9\}, \{1,11\},$   
 $\{2,3\}, \{2,6\}, \{2,7\}, \{3,4\}, \{3,5\}, \{3,6\}, \{3,7\}, \{3,8\}, \{3,9\}, \{3,10\}, \{3,11\},$   
 $\{4,5\}, \{4,8\}, \{4,10\}, \{5,7\}, \{5,8\}, \{5,10\}, \{6,7\}, \{6,9\}, \{6,10\}, \{7,8\}, \{7,10\},$   
 $\{8,9\}, \{8,10\}, \{8,11\}, \{9,10\}, \{9,11\}, \{\{1,2\}, \{1,3\}, \{1,7\}, \{1,8\}, \{1,9\},$   
 $\{1,11\}, \{2,3\}, \{2,4\}, \{2,5\}, \{2,7\}, \{2,8\}, \{2,9\}, \{2,10\}, \{2,11\}, \{3,7\}, \{3,8\},$   
 $\{3,10\}, \{3,11\}, \{4,5\}, \{4,6\}, \{4,10\}, \{4,11\}, \{5,6\}, \{5,9\}, \{5,11\}, \{6,9\},$   
 $\{6,10\}, \{6,11\}, \{7,9\}, \{7,10\}, \{8,11\}, \{9,10\}, \{9,11\}, \{10,11\}, \{\{1,2\}, \{1,3\},$   
 $\{1,5\}, \{1,10\}, \{2,3\}, \{2,5\}, \{2,9\}, \{2,10\}, \{3,4\}, \{3,5\}, \{3,6\}, \{3,7\}, \{3,8\},$   
 $\{3,9\}, \{3,10\}, \{3,11\}, \{4,5\}, \{4,6\}, \{4,8\}, \{5,6\}, \{5,7\}, \{5,8\}, \{5,9\}, \{5,10\},$   
 $\{5,11\}, \{6,8\}, \{6,10\}, \{7,8\}, \{7,9\}, \{7,11\}, \{8,9\}, \{8,10\}, \{9,10\}, \{9,11\},$   
 $\{\{1,2\}, \{1,3\}, \{1,4\}, \{1,6\}, \{1,7\}, \{1,8\}, \{1,9\}, \{2,3\}, \{2,6\}, \{2,7\}, \{3,4\},$   
 $\{3,6\}, \{3,7\}, \{4,5\}, \{4,6\}, \{4,7\}, \{4,8\}, \{4,9\}, \{4,10\}, \{4,11\}, \{5,6\}, \{5,8\},$   
 $\{5,9\}, \{5,10\}, \{5,11\}, \{6,7\}, \{6,9\}, \{6,10\}, \{7,8\}, \{7,10\}, \{7,11\}, \{8,9\},$   
 $\{8,11\}, \{10,11\}, \{\{1,2\}, \{1,3\}, \{1,6\}, \{1,8\}, \{1,9\}, \{1,10\}, \{1,11\}, \{2,3\},$   
 $\{2,5\}, \{2,6\}, \{2,8\}, \{3,4\}, \{3,5\}, \{3,7\}, \{3,8\}, \{3,9\}, \{3,10\}, \{3,11\}, \{4,5\},$   
 $\{4,8\}, \{4,11\}, \{5,6\}, \{5,8\}, \{5,11\}, \{6,8\}, \{6,11\}, \{7,8\}, \{7,9\}, \{7,10\},$   
 $\{7,11\}, \{8,9\}, \{8,11\}, \{9,10\}, \{10,11\}, \{\{1,2\}, \{1,4\}, \{1,5\}, \{1,6\}, \{1,7\},$   
 $\{1,9\}, \{1,10\}, \{1,11\}, \{2,3\}, \{2,4\}, \{2,5\}, \{2,6\}, \{2,7\}, \{2,8\}, \{2,9\}, \{2,10\},$   
 $\{2,11\}, \{3,4\}, \{3,6\}, \{3,7\}, \{3,8\}, \{3,9\}, \{4,8\}, \{4,9\}, \{4,10\}, \{4,11\}, \{5,6\},$   
 $\{5,7\}, \{6,7\}, \{6,8\}, \{6,11\}, \{7,9\}, \{8,11\}, \{9,10\}, \{\{1,2\}, \{1,3\}, \{1,4\},$   
 $\{1,5\}, \{1,6\}, \{1,8\}, \{1,9\}, \{1,11\}, \{2,3\}, \{2,4\}, \{2,5\}, \{2,6\}, \{2,7\}, \{2,9\},$   
 $\{2,10\}, \{2,11\}, \{3,4\}, \{3,5\}, \{3,6\}, \{3,7\}, \{3,8\}, \{3,10\}, \{4,8\}, \{4,9\}, \{4,11\},$   
 $\{5,6\}, \{5,8\}, \{5,9\}, \{5,10\}, \{6,7\}, \{6,10\}, \{7,10\}, \{8,9\}, \{9,11\}, \{\{1,2\},$



$\{1,3\}, \{1,6\}, \{1,7\}, \{1,9\}, \{1,10\}, \{2,4\}, \{2,6\}, \{2,8\}, \{2,9\}, \{2,10\}, \{3,5\},$   
 $\{3,6\}, \{3,7\}, \{3,9\}, \{3,10\}, \{4,5\}, \{4,6\}, \{4,8\}, \{4,9\}, \{4,11\}, \{5,6\}, \{5,9\},$   
 $\{5,10\}, \{5,11\}, \{6,10\}, \{7,9\}, \{8,9\}, \{8,10\}, \{8,11\}, \{9,11\}, \{10,11\}, \{\{1,2\},$   
 $\{1,4\}, \{1,5\}, \{1,7\}, \{1,8\}, \{1,9\}, \{1,10\}, \{1,11\}, \{2,3\}, \{2,4\}, \{2,5\}, \{2,6\},$   
 $\{2,7\}, \{2,8\}, \{2,10\}, \{3,7\}, \{3,8\}, \{3,10\}, \{4,5\}, \{4,6\}, \{4,7\}, \{4,8\}, \{4,9\},$   
 $\{4,11\}, \{5,6\}, \{5,9\}, \{6,8\}, \{6,9\}, \{6,11\}, \{7,8\}, \{7,10\}, \{8,10\}, \{8,11\},$   
 $\{9,11\}\}, \{\{1,2\}, \{1,4\}, \{1,6\}, \{1,10\}, \{2,3\}, \{2,4\}, \{2,5\}, \{2,6\}, \{2,7\},$   
 $\{2,10\}, \{2,11\}, \{3,4\}, \{3,6\}, \{3,7\}, \{4,5\}, \{4,6\}, \{4,7\}, \{4,8\}, \{4,10\}, \{5,7\},$   
 $\{5,10\}, \{6,7\}, \{6,8\}, \{6,9\}, \{6,10\}, \{6,11\}, \{7,8\}, \{7,9\}, \{7,10\}, \{7,11\},$   
 $\{8,10\}, \{9,10\}, \{9,11\}, \{10,11\}\}, \{\{1,2\}, \{1,3\}, \{1,6\}, \{1,11\}, \{2,3\}, \{2,4\},$   
 $\{2,6\}, \{2,7\}, \{2,9\}, \{2,10\}, \{2,11\}, \{3,4\}, \{3,5\}, \{3,6\}, \{3,7\}, \{3,8\}, \{3,10\},$   
 $\{3,11\}, \{4,5\}, \{4,6\}, \{4,8\}, \{4,10\}, \{4,11\}, \{5,8\}, \{5,10\}, \{6,7\}, \{6,8\}, \{6,9\},$   
 $\{6,10\}, \{6,11\}, \{7,9\}, \{7,10\}, \{8,10\}, \{9,10\}\}, \{\{1,2\}, \{1,4\}, \{1,5\}, \{1,6\},$   
 $\{1,8\}, \{2,5\}, \{2,6\}, \{2,7\}, \{2,8\}, \{3,4\}, \{3,5\}, \{3,6\}, \{3,7\}, \{3,9\}, \{4,5\},$   
 $\{4,6\}, \{4,7\}, \{4,8\}, \{4,9\}, \{4,10\}, \{4,11\}, \{5,6\}, \{5,7\}, \{5,8\}, \{5,9\}, \{5,10\},$   
 $\{5,11\}, \{6,7\}, \{6,9\}, \{6,10\}, \{7,8\}, \{9,10\}, \{9,11\}, \{10,11\}\}, \{\{1,2\}, \{1,3\},$   
 $\{1,4\}, \{1,7\}, \{1,10\}, \{1,11\}, \{2,3\}, \{2,4\}, \{2,5\}, \{2,7\}, \{2,11\}, \{3,4\}, \{3,5\},$   
 $\{3,6\}, \{3,7\}, \{3,8\}, \{3,9\}, \{3,10\}, \{3,11\}, \{4,5\}, \{4,8\}, \{4,9\}, \{4,10\}, \{5,6\},$   
 $\{5,7\}, \{5,8\}, \{6,7\}, \{6,8\}, \{7,8\}, \{7,10\}, \{7,11\}, \{8,9\}, \{8,10\}, \{9,10\}\},$   
 $\{\{1,2\}, \{1,3\}, \{1,5\}, \{1,6\}, \{1,7\}, \{1,11\}, \{2,3\}, \{2,4\}, \{2,7\}, \{2,8\}, \{2,10\},$   
 $\{2,11\}, \{3,4\}, \{3,5\}, \{3,6\}, \{3,7\}, \{3,9\}, \{3,10\}, \{3,11\}, \{4,7\}, \{4,8\}, \{4,10\},$   
 $\{5,6\}, \{5,10\}, \{5,11\}, \{6,7\}, \{6,9\}, \{6,10\}, \{7,8\}, \{7,9\}, \{7,10\}, \{8,10\},$   
 $\{9,10\}, \{10,11\}\}, \{\{1,2\}, \{1,3\}, \{1,4\}, \{1,5\}, \{1,6\}, \{2,3\}, \{2,5\}, \{2,6\},$   
 $\{2,9\}, \{2,10\}, \{3,4\}, \{3,5\}, \{3,6\}, \{3,7\}, \{3,8\}, \{3,9\}, \{3,10\}, \{3,11\}, \{4,5\},$   
 $\{4,6\}, \{4,7\}, \{4,8\}, \{4,9\}, \{4,11\}, \{5,9\}, \{6,7\}, \{6,10\}, \{7,8\}, \{7,9\}, \{7,10\},$   
 $\{8,9\}, \{8,11\}, \{9,10\}, \{9,11\}\}, \{\{1,2\}, \{1,5\}, \{1,6\}, \{1,7\}, \{1,8\}, \{1,10\},$   
 $\{1,11\}, \{2,3\}, \{2,4\}, \{2,5\}, \{2,6\}, \{2,7\}, \{2,8\}, \{2,9\}, \{2,10\}, \{2,11\}, \{3,4\},$   
 $\{3,8\}, \{3,9\}, \{4,8\}, \{4,9\}, \{4,10\}, \{5,6\}, \{5,8\}, \{6,8\}, \{6,9\}, \{6,11\}, \{7,8\},$   
 $\{7,10\}, \{8,9\}, \{8,10\}, \{9,10\}, \{9,11\}, \{10,11\}\}, \{\{1,2\}, \{1,3\}, \{1,4\}, \{1,5\},$   
 $\{1,6\}, \{1,7\}, \{1,8\}, \{1,11\}, \{2,3\}, \{2,4\}, \{2,6\}, \{2,7\}, \{2,8\}, \{2,9\}, \{2,11\},$   
 $\{3,4\}, \{3,5\}, \{3,9\}, \{3,10\}, \{4,5\}, \{4,6\}, \{4,7\}, \{4,8\}, \{4,9\}, \{4,10\}, \{4,11\},$   
 $\{5,8\}, \{5,9\}, \{5,10\}, \{6,7\}, \{6,8\}, \{7,11\}, \{8,9\}, \{9,10\}\}, \{\{1,2\}, \{1,3\},$   
 $\{1,4\}, \{1,8\}, \{1,9\}, \{1,10\}, \{1,11\}, \{2,3\}, \{2,4\}, \{2,5\}, \{2,6\}, \{2,7\}, \{2,8\},$   
 $\{2,11\}, \{3,4\}, \{3,5\}, \{3,8\}, \{4,5\}, \{4,6\}, \{4,7\}, \{4,8\}, \{4,9\}, \{5,6\}, \{5,8\},$   
 $\{6,8\}, \{7,8\}, \{7,9\}, \{7,11\}, \{8,9\}, \{8,10\}, \{8,11\}, \{9,10\}, \{9,11\}, \{10,11\}\},$   
 $\{\{1,2\}, \{1,6\}, \{1,7\}, \{1,10\}, \{1,11\}, \{2,4\}, \{2,7\}, \{2,9\}, \{2,10\}, \{2,11\},$   
 $\{3,4\}, \{3,7\}, \{3,8\}, \{3,10\}, \{4,5\}, \{4,6\}, \{4,7\}, \{4,8\}, \{4,9\}, \{4,10\}, \{4,11\},$   
 $\{5,6\}, \{5,8\}, \{5,10\}, \{6,7\}, \{6,8\}, \{6,10\}, \{6,11\}, \{7,8\}, \{7,9\}, \{7,10\},$   
 $\{8,10\}, \{9,10\}, \{10,11\}\}, \{\{1,2\}, \{1,3\}, \{1,4\}, \{1,5\}, \{1,6\}, \{1,7\}, \{1,8\},$   
 $\{1,10\}, \{1,11\}, \{2,3\}, \{2,7\}, \{2,9\}, \{2,10\}, \{2,11\}, \{3,5\}, \{3,9\}, \{3,10\},$   
 $\{4,5\}, \{4,6\}, \{4,11\}, \{5,6\}, \{5,8\}, \{5,9\}, \{5,10\}, \{5,11\}, \{6,8\}, \{6,11\},$   
 $\{7,10\}, \{7,11\}, \{8,10\}, \{8,11\}, \{9,10\}, \{9,11\}, \{10,11\}\}, \{\{1,2\}, \{1,3\}, \{1,4\},$   
 $\{1,5\}, \{1,6\}, \{1,7\}, \{1,8\}, \{1,9\}, \{1,10\}, \{1,11\}, \{2,4\}, \{2,7\}, \{2,10\}, \{3,4\},$   
 $\{3,6\}, \{3,9\}, \{3,11\}, \{4,5\}, \{4,6\}, \{4,7\}, \{4,8\}, \{4,9\}, \{4,10\}, \{4,11\}, \{5,6\},$   
 $\{5,8\}, \{5,9\}, \{6,9\}, \{7,9\}, \{7,10\}, \{8,9\}, \{9,10\}, \{9,11\}, \{10,11\}\}, \{\{1,2\},$   
 $\{1,3\}, \{1,4\}, \{1,5\}, \{1,6\}, \{1,7\}, \{1,9\}, \{1,10\}, \{1,11\}, \{2,3\}, \{2,7\}, \{2,10\},$   
 $\{3,4\}, \{3,7\}, \{3,9\}, \{3,10\}, \{4,5\}, \{4,6\}, \{4,7\}, \{4,8\}, \{4,9\}, \{4,10\}, \{4,11\},$   
 $\{5,6\}, \{5,7\}, \{5,8\}, \{5,11\}, \{6,7\}, \{6,10\}, \{7,8\}, \{7,9\}, \{7,10\}, \{7,11\},$   
 $\{8,11\}\}, \{\{1,2\}, \{1,4\}, \{1,6\}, \{1,7\}, \{1,9\}, \{2,3\}, \{2,4\}, \{2,5\}, \{2,6\}, \{2,7\},$   
 $\{2,8\}, \{2,9\}, \{2,10\}, \{2,11\}, \{3,4\}, \{3,5\}, \{3,6\}, \{3,8\}, \{3,10\}, \{4,5\}, \{4,6\},$

{4,7},{4,9},{5,7},{5,8},{5,10},{6,7},{6,8},{6,9},{6,11},{7,8},{7,11},  
 {8,10},{8,11}},{{1,2},{1,3},{1,4},{1,5},{1,8},{1,9},{1,11},{2,3},  
 {2,5},{2,6},{2,7},{2,9},{3,4},{3,5},{3,6},{3,7},{3,8},{3,9},{3,10},  
 {3,11},{4,6},{4,7},{4,8},{4,11},{5,7},{5,11},{6,7},{6,8},{6,9},{6,10},  
 {7,11},{8,9},{8,10},{9,10}},{{1,2},{1,3},{1,4},{1,6},{1,7},{1,10},  
 {2,6},{2,7},{2,9},{2,10},{2,11},{3,4},{3,5},{3,6},{3,10},{4,5},{4,6},  
 {4,7},{5,6},{5,7},{5,10},{6,7},{6,8},{6,9},{6,10},{6,11},{7,8},{7,9},  
 {7,10},{7,11},{8,9},{8,10},{9,10},{9,11}},{{1,2},{1,4},{1,6},{1,8},  
 {1,9},{2,4},{2,7},{2,8},{2,9},{3,4},{3,5},{3,7},{3,8},{3,10},{3,11},  
 {4,5},{4,6},{4,7},{4,8},{4,9},{4,10},{4,11},{5,6},{5,9},{5,10},{5,11},  
 {6,8},{6,9},{6,10},{7,8},{7,9},{7,11},{8,10},{9,11}},{{1,2},{1,3},  
 {1,5},{1,6},{1,7},{1,11},{2,4},{2,5},{2,6},{2,7},{2,8},{3,4},{3,6},  
 {3,7},{3,8},{3,11},{4,5},{4,6},{4,8},{4,9},{4,11},{5,6},{5,9},{5,10},  
 {5,11},{6,7},{6,8},{6,9},{6,10},{6,11},{7,8},{9,10},{9,11},{10,11}},  
 {{1,2},{1,3},{1,4},{1,10},{1,11},{2,3},{2,4},{2,7},{2,8},{2,9},{2,10},  
 {3,4},{3,5},{3,6},{3,7},{3,8},{3,10},{3,11},{4,7},{4,10},{4,11},{5,6},  
 {5,7},{5,10},{6,7},{6,8},{6,9},{6,10},{7,8},{7,9},{7,10},{8,9},{9,10},  
 {10,11}},{{1,2},{1,4},{1,5},{1,6},{1,7},{1,8},{2,3},{2,4},{2,5},{2,7},  
 {2,9},{3,4},{3,5},{3,6},{3,7},{3,9},{4,5},{4,6},{4,7},{4,8},{4,9},  
 {4,11},{5,6},{5,9},{6,7},{6,8},{6,10},{6,11},{7,8},{7,10},{7,11},  
 {8,10},{8,11},{10,11}},{{1,2},{1,3},{1,4},{1,6},{1,10},{2,4},{2,5},  
 {2,6},{2,10},{3,4},{3,6},{3,7},{3,8},{3,9},{3,10},{3,11},{4,5},{4,6},  
 {4,9},{5,6},{5,7},{5,9},{5,10},{5,11},{6,7},{6,8},{6,9},{6,10},{6,11},  
 {7,8},{7,10},{7,11},{8,11},{9,11}},{{1,2},{1,3},{1,4},{1,6},{1,7},  
 {1,10},{1,11},{2,5},{2,6},{2,7},{2,10},{2,11},{3,4},{3,6},{3,8},{3,9},  
 {4,7},{4,8},{4,9},{5,6},{5,7},{5,9},{6,8},{6,9},{6,10},{7,8},{7,9},  
 {7,11},{8,9},{8,10},{8,11},{10,11}},{{1,2},{1,3},{1,7},{1,10},{1,11},  
 {2,3},{2,5},{2,6},{2,7},{2,8},{2,9},{2,10},{2,11},{3,4},{3,5},{3,6},  
 {3,7},{3,8},{3,9},{3,11},{4,7},{4,9},{4,11},{5,6},{5,11},{6,9},{6,11},  
 {7,8},{7,9},{7,10},{7,11},{8,9},{9,11},{10,11}},{{1,2},{1,3},{1,7},  
 {1,9},{1,11},{2,3},{2,4},{2,5},{2,6},{2,7},{2,8},{2,9},{2,10},{2,11},  
 {3,4},{3,5},{3,6},{3,7},{3,11},{4,6},{4,7},{4,8},{4,10},{4,11},{5,6},  
 {5,7},{5,10},{6,10},{7,8},{7,9},{7,10},{8,9},{8,11},{9,11}},{{1,2},  
 {1,4},{1,8},{1,9},{1,11},{2,3},{2,4},{2,5},{2,6},{2,7},{2,8},{2,9},  
 {2,10},{2,11},{3,4},{3,5},{3,7},{3,10},{4,5},{4,6},{4,7},{4,8},{4,9},  
 {4,10},{5,6},{5,7},{5,8},{5,9},{5,10},{5,11},{6,10},{7,9},{8,11},  
 {9,11}},{{1,2},{1,3},{1,5},{1,7},{1,9},{2,4},{2,5},{2,7},{2,9},{3,4},  
 {3,5},{3,6},{3,7},{3,8},{3,9},{3,10},{3,11},{4,5},{4,7},{4,9},{4,10},  
 {4,11},{5,6},{5,7},{5,9},{5,10},{6,7},{6,8},{6,10},{7,8},{7,11},  
 {8,10},{8,11},{10,11}},{{1,2},{1,3},{1,4},{1,7},{1,11},{2,3},{2,4},  
 {2,5},{2,7},{2,8},{3,4},{3,5},{3,6},{3,7},{3,8},{3,9},{3,10},{3,11},  
 {4,5},{4,11},{5,6},{5,8},{5,9},{5,11},{6,7},{6,8},{6,9},{6,10},{6,11},  
 {7,8},{7,11},{9,10},{9,11},{10,11}},{{1,2},{1,5},{1,7},{1,8},{1,9},  
 {1,10},{1,11},{2,4},{2,5},{2,7},{2,8},{3,4},{3,5},{3,6},{3,8},{4,5},  
 {4,6},{4,7},{4,8},{4,10},{5,6},{5,7},{5,8},{5,9},{5,10},{5,11},{6,8},  
 {6,9},{6,10},{6,11},{7,10},{8,9},{9,11},{10,11}},{{1,2},{1,4},{1,5},  
 {1,6},{1,8},{2,4},{2,5},{2,6},{2,7},{2,8},{2,11},{3,4},{3,5},{3,6},  
 {3,7},{3,9},{3,10},{3,11},{4,5},{4,6},{4,7},{5,6},{5,7},{5,8},{5,9},  
 {5,10},{5,11},{6,8},{6,11},{7,9},{7,10},{7,11},{9,10},{10,11}},{{1,2},  
 {1,3},{1,5},{1,6},{1,7},{1,10},{1,11},{2,3},{2,4},{2,5},{2,6},{2,7},

$\{2,9\}, \{2,10\}, \{2,11\}, \{3,4\}, \{3,6\}, \{3,7\}, \{3,8\}, \{3,9\}, \{3,10\}, \{3,11\}, \{4,9\},$   
 $\{4,10\}, \{5,10\}, \{5,11\}, \{6,7\}, \{6,10\}, \{8,9\}, \{8,10\}, \{8,11\}, \{9,10\}, \{9,11\},$   
 $\{10,11\}\}, \{\{1,2\}, \{1,4\}, \{1,7\}, \{1,10\}, \{2,3\}, \{2,4\}, \{2,5\}, \{2,7\}, \{2,9\},$   
 $\{2,10\}, \{2,11\}, \{3,4\}, \{3,5\}, \{3,6\}, \{3,10\}, \{3,11\}, \{4,5\}, \{4,6\}, \{4,7\}, \{4,8\},$   
 $\{4,9\}, \{4,10\}, \{4,11\}, \{5,6\}, \{5,7\}, \{5,8\}, \{5,9\}, \{6,8\}, \{6,10\}, \{7,8\}, \{7,9\},$   
 $\{7,10\}, \{8,10\}, \{10,11\}\}, \{\{1,2\}, \{1,3\}, \{1,4\}, \{1,6\}, \{1,7\}, \{1,8\}, \{1,9\},$   
 $\{2,3\}, \{2,4\}, \{2,8\}, \{2,10\}, \{3,4\}, \{3,5\}, \{3,6\}, \{3,7\}, \{3,8\}, \{3,9\}, \{3,10\},$   
 $\{3,11\}, \{4,5\}, \{4,6\}, \{4,10\}, \{4,11\}, \{5,9\}, \{5,10\}, \{5,11\}, \{6,7\}, \{6,11\},$   
 $\{7,9\}, \{7,11\}, \{8,9\}, \{8,10\}, \{9,10\}, \{9,11\}\}, \{\{1,2\}, \{1,3\}, \{1,4\}, \{1,5\},$   
 $\{1,6\}, \{1,7\}, \{1,8\}, \{1,9\}, \{1,10\}, \{1,11\}, \{2,3\}, \{2,5\}, \{2,6\}, \{2,8\}, \{3,4\},$   
 $\{3,5\}, \{3,8\}, \{3,9\}, \{3,10\}, \{4,5\}, \{4,9\}, \{4,10\}, \{5,6\}, \{5,7\}, \{5,8\}, \{5,9\},$   
 $\{5,11\}, \{6,8\}, \{7,8\}, \{7,9\}, \{7,11\}, \{8,9\}, \{8,11\}, \{9,10\}\}, \{\{1,2\}, \{1,3\},$   
 $\{1,4\}, \{1,5\}, \{1,6\}, \{1,7\}, \{1,8\}, \{1,9\}, \{1,10\}, \{1,11\}, \{2,3\}, \{2,5\}, \{2,6\},$   
 $\{2,7\}, \{2,8\}, \{2,11\}, \{3,4\}, \{3,8\}, \{3,9\}, \{3,10\}, \{3,11\}, \{4,5\}, \{4,6\}, \{4,7\},$   
 $\{4,8\}, \{4,10\}, \{5,7\}, \{5,8\}, \{6,7\}, \{6,9\}, \{6,10\}, \{6,11\}, \{9,10\}, \{9,11\}\},$   
 $\{\{1,2\}, \{1,3\}, \{1,4\}, \{1,5\}, \{1,6\}, \{1,7\}, \{1,8\}, \{1,9\}, \{1,11\}, \{2,3\}, \{2,7\},$   
 $\{2,11\}, \{3,4\}, \{3,5\}, \{3,6\}, \{3,7\}, \{3,8\}, \{3,9\}, \{3,10\}, \{3,11\}, \{4,5\}, \{4,6\},$   
 $\{4,7\}, \{5,7\}, \{5,11\}, \{6,7\}, \{6,8\}, \{6,9\}, \{6,10\}, \{7,8\}, \{7,11\}, \{8,9\}, \{8,10\},$   
 $\{9,10\}\}, \{\{1,2\}, \{1,3\}, \{1,4\}, \{1,5\}, \{1,6\}, \{1,10\}, \{2,3\}, \{2,5\}, \{2,6\}, \{2,7\},$   
 $\{3,4\}, \{3,5\}, \{3,6\}, \{3,7\}, \{3,8\}, \{3,9\}, \{3,10\}, \{3,11\}, \{4,5\}, \{4,7\}, \{4,8\},$   
 $\{4,9\}, \{4,10\}, \{4,11\}, \{5,7\}, \{5,8\}, \{5,9\}, \{6,7\}, \{6,10\}, \{7,9\}, \{7,10\},$   
 $\{7,11\}, \{8,9\}, \{10,11\}\}, \{\{1,2\}, \{1,4\}, \{1,5\}, \{1,6\}, \{1,7\}, \{1,8\}, \{1,9\},$   
 $\{1,10\}, \{1,11\}, \{2,3\}, \{2,4\}, \{2,5\}, \{2,6\}, \{3,4\}, \{3,5\}, \{3,6\}, \{3,8\}, \{4,5\},$   
 $\{4,6\}, \{4,8\}, \{4,9\}, \{4,11\}, \{5,8\}, \{5,9\}, \{5,10\}, \{6,8\}, \{7,8\}, \{7,10\}, \{7,11\},$   
 $\{8,10\}, \{8,11\}, \{9,10\}, \{9,11\}, \{10,11\}\}, \{\{1,2\}, \{1,4\}, \{1,7\}, \{1,8\}, \{1,9\},$   
 $\{1,11\}, \{2,3\}, \{2,4\}, \{2,5\}, \{2,6\}, \{2,7\}, \{2,8\}, \{2,9\}, \{2,11\}, \{3,4\}, \{3,6\},$   
 $\{3,7\}, \{3,8\}, \{3,9\}, \{3,10\}, \{4,8\}, \{4,9\}, \{4,11\}, \{5,6\}, \{5,7\}, \{5,9\}, \{5,10\},$   
 $\{6,9\}, \{6,10\}, \{7,8\}, \{7,9\}, \{7,10\}, \{8,11\}, \{9,10\}\}, \{\{1,2\}, \{1,4\}, \{1,5\},$   
 $\{1,6\}, \{1,8\}, \{1,10\}, \{1,11\}, \{2,4\}, \{2,5\}, \{2,6\}, \{2,7\}, \{2,10\}, \{3,4\}, \{3,6\},$   
 $\{3,8\}, \{3,9\}, \{3,10\}, \{3,11\}, \{4,6\}, \{4,8\}, \{4,9\}, \{4,10\}, \{5,6\}, \{5,7\}, \{5,10\},$   
 $\{6,7\}, \{6,8\}, \{6,9\}, \{6,10\}, \{6,11\}, \{7,10\}, \{8,11\}, \{9,10\}, \{10,11\}\}, \{\{1,2\},$   
 $\{1,3\}, \{1,8\}, \{1,9\}, \{1,10\}, \{1,11\}, \{2,3\}, \{2,4\}, \{2,5\}, \{2,7\}, \{2,8\}, \{2,9\},$   
 $\{2,10\}, \{3,4\}, \{3,6\}, \{3,8\}, \{3,9\}, \{3,11\}, \{4,5\}, \{4,6\}, \{4,7\}, \{4,8\}, \{4,10\},$   
 $\{5,7\}, \{5,10\}, \{6,8\}, \{6,10\}, \{6,11\}, \{7,8\}, \{7,10\}, \{8,9\}, \{8,10\}, \{8,11\},$   
 $\{10,11\}\}, \{\{1,2\}, \{1,3\}, \{1,4\}, \{1,5\}, \{1,6\}, \{1,11\}, \{2,3\}, \{2,5\}, \{2,6\},$   
 $\{2,7\}, \{2,9\}, \{2,10\}, \{2,11\}, \{3,4\}, \{3,5\}, \{3,6\}, \{3,7\}, \{3,8\}, \{3,10\}, \{3,11\},$   
 $\{4,5\}, \{4,6\}, \{5,6\}, \{5,7\}, \{5,11\}, \{6,7\}, \{6,8\}, \{6,9\}, \{6,10\}, \{7,8\}, \{7,9\},$   
 $\{7,10\}, \{8,10\}, \{9,10\}\}, \{\{1,2\}, \{1,3\}, \{1,6\}, \{1,8\}, \{1,9\}, \{2,3\}, \{2,8\},$   
 $\{2,9\}, \{3,4\}, \{3,5\}, \{3,6\}, \{3,7\}, \{3,8\}, \{3,9\}, \{4,5\}, \{4,6\}, \{4,9\}, \{5,6\},$   
 $\{5,7\}, \{5,9\}, \{5,10\}, \{5,11\}, \{6,8\}, \{6,9\}, \{6,11\}, \{7,8\}, \{7,9\}, \{7,10\}, \{8,9\},$   
 $\{8,10\}, \{8,11\}, \{9,10\}, \{9,11\}, \{10,11\}\}, \{\{1,2\}, \{1,3\}, \{1,4\}, \{1,7\}, \{1,8\},$   
 $\{1,10\}, \{2,3\}, \{2,4\}, \{2,8\}, \{2,11\}, \{3,4\}, \{3,5\}, \{3,6\}, \{3,7\}, \{3,8\}, \{3,11\},$   
 $\{4,5\}, \{4,6\}, \{4,7\}, \{4,8\}, \{4,9\}, \{4,10\}, \{4,11\}, \{5,6\}, \{5,7\}, \{5,8\}, \{5,9\},$   
 $\{6,8\}, \{7,9\}, \{7,10\}, \{8,9\}, \{8,10\}, \{8,11\}, \{9,10\}\}, \{\{1,2\}, \{1,4\}, \{1,5\},$   
 $\{1,6\}, \{1,7\}, \{1,8\}, \{1,11\}, \{2,3\}, \{2,4\}, \{2,5\}, \{2,6\}, \{2,7\}, \{2,8\}, \{2,9\},$   
 $\{2,10\}, \{2,11\}, \{3,6\}, \{3,8\}, \{3,9\}, \{3,11\}, \{4,6\}, \{4,10\}, \{4,11\}, \{5,6\},$   
 $\{5,7\}, \{5,8\}, \{6,8\}, \{6,9\}, \{6,10\}, \{7,8\}, \{8,11\}, \{9,10\}, \{9,11\}, \{10,11\}\},$   
 $\{\{1,2\}, \{1,3\}, \{1,4\}, \{1,5\}, \{1,8\}, \{1,9\}, \{1,10\}, \{2,5\}, \{2,6\}, \{2,8\}, \{2,10\},$   
 $\{3,4\}, \{3,5\}, \{3,6\}, \{3,9\}, \{3,11\}, \{4,5\}, \{4,6\}, \{4,7\}, \{4,10\}, \{5,6\}, \{5,7\},$   
 $\{5,8\}, \{5,9\}, \{5,10\}, \{5,11\}, \{6,7\}, \{6,8\}, \{6,9\}, \{6,10\}, \{6,11\}, \{7,10\},$

$\{8,9\},\{9,11\},\{\{1,2\},\{1,6\},\{1,7\},\{1,8\},\{1,11\},\{2,3\},\{2,4\},\{2,5\},\{2,6\},$   
 $\{2,9\},\{2,10\},\{2,11\},\{3,4\},\{3,5\},\{3,7\},\{3,11\},\{4,5\},\{4,8\},\{4,9\},\{4,10\},$   
 $\{4,11\},\{5,7\},\{5,10\},\{6,7\},\{6,8\},\{6,9\},\{7,8\},\{7,9\},\{7,10\},\{7,11\},\{8,9\},$   
 $\{8,11\},\{9,10\}\},\{\{1,2\},\{1,3\},\{1,4\},\{1,5\},\{1,6\},\{1,7\},\{1,8\},\{1,10\},$   
 $\{2,4\},\{2,5\},\{2,8\},\{3,4\},\{3,7\},\{3,10\},\{4,5\},\{4,6\},\{4,7\},\{4,8\},\{4,9\},$   
 $\{4,10\},\{4,11\},\{5,6\},\{5,8\},\{6,7\},\{6,8\},\{6,9\},\{6,11\},\{7,8\},\{7,9\},\{7,10\},$   
 $\{7,11\},\{8,10\},\{8,11\},\{9,11\}\},\{\{1,2\},\{1,6\},\{1,7\},\{1,8\},\{2,4\},\{2,6\},$   
 $\{2,7\},\{2,8\},\{2,9\},\{3,4\},\{3,5\},\{3,6\},\{3,8\},\{3,10\},\{3,11\},\{4,6\},\{4,7\},$   
 $\{4,8\},\{4,9\},\{4,11\},\{5,6\},\{5,8\},\{5,10\},\{6,7\},\{6,8\},\{6,9\},\{6,10\},\{7,8\},$   
 $\{7,9\},\{7,10\},\{7,11\},\{8,10\},\{8,11\},\{10,11\}\},\{\{1,2\},\{1,4\},\{1,5\},\{1,9\},$   
 $\{1,10\},\{2,4\},\{2,6\},\{2,7\},\{2,8\},\{2,9\},\{2,10\},\{3,4\},\{3,6\},\{3,9\},\{3,11\},$   
 $\{4,5\},\{4,6\},\{4,9\},\{4,11\},\{5,6\},\{5,8\},\{5,9\},\{5,10\},\{5,11\},\{6,7\},\{6,8\},$   
 $\{6,9\},\{6,11\},\{7,8\},\{7,9\},\{8,9\},\{8,10\},\{9,10\},\{9,11\}\},\{\{1,2\},\{1,7\},$   
 $\{1,8\},\{1,9\},\{1,11\},\{2,5\},\{2,7\},\{2,9\},\{2,11\},\{3,4\},\{3,6\},\{3,9\},\{3,10\},$   
 $\{4,5\},\{4,6\},\{4,7\},\{4,9\},\{4,10\},\{5,6\},\{5,7\},\{5,9\},\{5,11\},\{6,7\},\{6,8\},$   
 $\{6,9\},\{6,10\},\{6,11\},\{7,8\},\{7,9\},\{7,10\},\{8,9\},\{8,11\},\{9,10\},\{9,11\}\},$   
 $\{\{1,2\},\{1,3\},\{1,4\},\{1,5\},\{1,7\},\{1,8\},\{1,9\},\{2,4\},\{2,8\},\{2,9\},\{2,10\},$   
 $\{2,11\},\{3,4\},\{3,5\},\{3,7\},\{3,9\},\{4,5\},\{4,6\},\{4,7\},\{4,8\},\{4,9\},\{4,10\},$   
 $\{4,11\},\{5,7\},\{6,7\},\{6,8\},\{6,9\},\{6,11\},\{7,8\},\{7,9\},\{8,10\},\{8,11\},$   
 $\{9,11\},\{10,11\}\},\{\{1,2\},\{1,3\},\{1,4\},\{1,5\},\{1,6\},\{1,7\},\{1,8\},\{1,9\},$   
 $\{1,10\},\{1,11\},\{2,3\},\{2,4\},\{2,5\},\{2,9\},\{2,10\},\{2,11\},\{3,4\},\{3,7\},\{3,9\},$   
 $\{3,11\},\{4,5\},\{4,7\},\{4,8\},\{5,6\},\{5,7\},\{5,8\},\{5,10\},\{6,7\},\{6,8\},\{7,8\},$   
 $\{7,9\},\{7,10\},\{9,10\},\{9,11\}\},\{\{1,2\},\{1,6\},\{1,7\},\{1,8\},\{1,9\},\{1,10\},$   
 $\{1,11\},\{2,5\},\{2,6\},\{2,8\},\{2,10\},\{3,4\},\{3,5\},\{3,9\},\{3,10\},\{4,5\},\{4,7\},$   
 $\{4,8\},\{4,9\},\{4,10\},\{5,6\},\{5,8\},\{5,9\},\{5,10\},\{6,9\},\{6,10\},\{6,11\},\{7,8\},$   
 $\{7,9\},\{7,10\},\{8,10\},\{9,10\},\{9,11\},\{10,11\}\},\{\{1,2\},\{1,6\},\{1,7\},\{1,8\},$   
 $\{1,10\},\{2,3\},\{2,4\},\{2,6\},\{2,8\},\{2,9\},\{2,10\},\{3,4\},\{3,5\},\{3,6\},\{3,8\},$   
 $\{3,9\},\{4,5\},\{4,6\},\{4,8\},\{4,9\},\{4,10\},\{4,11\},\{5,6\},\{5,8\},\{6,7\},\{6,8\},$   
 $\{6,10\},\{6,11\},\{7,8\},\{7,10\},\{8,9\},\{8,10\},\{8,11\},\{10,11\}\},\{\{1,2\},\{1,3\},$   
 $\{1,4\},\{1,5\},\{1,6\},\{1,7\},\{1,8\},\{1,9\},\{1,10\},\{1,11\},\{2,3\},\{2,4\},\{2,5\},$   
 $\{2,7\},\{2,9\},\{2,10\},\{2,11\},\{3,4\},\{3,5\},\{3,7\},\{4,6\},\{4,7\},\{4,8\},\{4,9\},$   
 $\{5,7\},\{6,7\},\{6,8\},\{6,10\},\{7,10\},\{7,11\},\{8,9\},\{8,10\},\{9,10\},\{10,11\}\},$   
 $\{\{1,2\},\{1,6\},\{1,8\},\{1,10\},\{2,3\},\{2,4\},\{2,5\},\{2,6\},\{2,8\},\{2,10\},\{3,4\},$   
 $\{3,7\},\{3,8\},\{3,9\},\{3,10\},\{4,5\},\{4,6\},\{4,7\},\{4,10\},\{5,6\},\{5,10\},\{6,7\},$   
 $\{6,8\},\{6,10\},\{6,11\},\{7,8\},\{7,9\},\{7,10\},\{7,11\},\{8,9\},\{8,10\},\{8,11\},$   
 $\{9,10\},\{10,11\}\},\{\{1,2\},\{1,3\},\{1,5\},\{1,6\},\{1,7\},\{1,9\},\{1,10\},\{1,11\},$   
 $\{2,3\},\{2,6\},\{2,10\},\{2,11\},\{3,4\},\{3,6\},\{3,7\},\{3,10\},\{4,6\},\{4,7\},\{4,9\},$   
 $\{4,10\},\{5,6\},\{5,7\},\{5,8\},\{5,9\},\{6,7\},\{6,8\},\{6,9\},\{6,10\},\{6,11\},\{7,8\},$   
 $\{7,9\},\{8,9\},\{9,10\},\{10,11\}\},\{\{1,2\},\{1,4\},\{1,7\},\{1,11\},\{2,3\},\{2,4\},$   
 $\{2,5\},\{2,6\},\{2,7\},\{2,8\},\{2,9\},\{2,10\},\{2,11\},\{3,6\},\{3,8\},\{3,9\},\{4,5\},$   
 $\{4,6\},\{4,7\},\{4,8\},\{4,9\},\{4,10\},\{4,11\},\{5,7\},\{5,8\},\{6,8\},\{6,9\},\{6,10\},$   
 $\{6,11\},\{7,8\},\{7,11\},\{8,9\},\{8,11\},\{9,10\}\},\{\{1,2\},\{1,3\},\{1,6\},\{1,8\},$   
 $\{2,3\},\{2,5\},\{2,6\},\{2,7\},\{2,8\},\{3,5\},\{3,6\},\{3,7\},\{3,8\},\{3,9\},\{4,5\},$   
 $\{4,8\},\{4,9\},\{4,10\},\{4,11\},\{5,7\},\{5,8\},\{5,9\},\{5,10\},\{5,11\},\{6,7\},\{6,8\},$   
 $\{7,8\},\{7,9\},\{7,10\},\{8,9\},\{8,10\},\{9,10\},\{9,11\},\{10,11\}\},\{\{1,2\},\{1,4\},$   
 $\{1,6\},\{1,7\},\{1,9\},\{2,6\},\{2,7\},\{2,9\},\{3,4\},\{3,5\},\{3,7\},\{3,8\},\{3,9\},$   
 $\{3,10\},\{4,6\},\{4,7\},\{4,8\},\{4,9\},\{5,7\},\{5,8\},\{5,10\},\{5,11\},\{6,7\},\{6,8\},$   
 $\{6,9\},\{6,11\},\{7,8\},\{7,9\},\{7,10\},\{7,11\},\{8,11\},\{9,10\},\{9,11\},\{10,11\}\},$   
 $\{\{1,2\},\{1,4\},\{1,5\},\{1,6\},\{1,7\},\{1,8\},\{1,11\},\{2,5\},\{2,7\},\{2,8\},\{2,9\},$   
 $\{2,10\},\{3,4\},\{3,5\},\{3,7\},\{3,8\},\{3,9\},\{4,5\},\{4,6\},\{4,7\},\{4,8\},\{5,8\},$

{5,9},{6,7},{6,8},{6,11},{7,8},{7,9},{7,10},{7,11},{8,9},{8,10},  
 {8,11},{9,10}},{{1,2},{1,3},{1,4},{1,5},{1,7},{1,9},{2,5},{2,7},{2,9},  
 {3,4},{3,7},{3,8},{3,9},{4,5},{4,7},{4,8},{4,10},{5,6},{5,7},{5,8},  
 {5,9},{5,10},{6,7},{6,8},{6,10},{6,11},{7,8},{7,9},{7,10},{7,11},  
 {8,9},{8,10},{8,11},{10,11}},{{1,2},{1,4},{1,5},{1,8},{2,4},{2,5},  
 {2,6},{2,8},{2,9},{2,10},{2,11},{3,4},{3,5},{3,7},{3,8},{3,10},{4,5},  
 {4,6},{4,7},{4,8},{5,7},{5,8},{5,9},{5,11},{6,7},{6,9},{6,10},{7,9},  
 {7,10},{8,10},{9,10},{9,11}},{{1,2},{1,3},{1,4},{1,5},{1,6},{1,8},  
 {1,9},{1,11},{2,3},{2,4},{2,5},{2,6},{2,7},{2,8},{2,10},{2,11},{3,5},  
 {3,6},{3,7},{3,10},{3,11},{4,6},{4,8},{4,9},{5,6},{5,7},{5,8},{5,9},  
 {6,7},{6,9},{6,10},{6,11},{7,10},{8,9}},{{1,2},{1,5},{1,9},{1,10},  
 {2,4},{2,5},{2,6},{2,9},{2,10},{2,11},{3,4},{3,6},{3,7},{3,8},{3,9},  
 {3,10},{4,6},{4,8},{4,9},{4,10},{5,6},{5,7},{5,9},{5,10},{5,11},{6,7},  
 {6,10},{6,11},{7,9},{7,10},{8,9},{8,10},{9,10},{10,11}},{{1,2},{1,3},  
 {1,4},{1,5},{1,7},{1,8},{1,9},{1,11},{2,3},{2,4},{2,10},{2,11},{3,4},  
 {3,7},{3,10},{4,5},{4,6},{4,7},{4,8},{4,9},{4,10},{4,11},{5,6},{5,8},  
 {5,9},{5,11},{6,9},{6,10},{6,11},{7,9},{7,10},{8,9},{9,10},{10,11}},  
 {{1,2},{1,3},{1,4},{1,5},{1,6},{1,7},{1,8},{1,9},{1,10},{1,11},{2,3},  
 {2,4},{2,10},{3,4},{3,5},{3,6},{3,8},{3,9},{3,10},{4,5},{4,6},{4,7},  
 {4,10},{5,7},{5,8},{6,7},{6,8},{6,9},{6,10},{6,11},{7,8},{8,9},{8,11},  
 {9,11}},{{1,2},{1,3},{1,5},{1,6},{1,7},{1,8},{1,9},{2,3},{2,4},{2,5},  
 {2,6},{2,9},{2,10},{3,6},{3,7},{3,10},{3,11},{4,5},{4,8},{4,10},{5,6},  
 {5,8},{5,9},{6,8},{6,9},{6,11},{7,8},{7,10},{7,11},{8,10},{8,11},  
 {10,11}},{{1,2},{1,3},{1,4},{1,5},{1,6},{1,7},{1,8},{1,9},{1,10},  
 {1,11},{2,6},{2,7},{2,11},{3,4},{3,5},{3,6},{3,8},{3,9},{3,10},{4,5},  
 {4,6},{4,8},{4,10},{5,6},{5,7},{5,8},{5,9},{6,7},{6,9},{6,10},{6,11},  
 {7,9},{7,11},{9,11}},{{1,2},{1,5},{1,6},{1,10},{2,3},{2,5},{2,6},  
 {2,8},{2,10},{3,4},{3,5},{3,6},{3,7},{3,8},{3,10},{3,11},{4,5},{4,7},  
 {4,9},{4,10},{4,11},{5,6},{5,7},{5,8},{5,9},{5,10},{5,11},{6,10},  
 {7,8},{7,9},{8,9},{8,10},{9,10},{10,11}},{{1,2},{1,3},{1,4},{1,5},  
 {1,7},{1,8},{1,9},{2,4},{2,5},{2,6},{2,7},{2,9},{3,4},{3,7},{3,8},  
 {4,5},{4,6},{4,7},{4,8},{4,9},{4,10},{5,6},{5,8},{5,9},{6,7},{6,8},  
 {6,10},{6,11},{7,8},{7,10},{7,11},{8,10},{8,11},{10,11}},{{1,2},{1,3},  
 {1,4},{1,5},{1,7},{1,8},{1,9},{1,10},{1,11},{2,5},{2,6},{2,7},{2,10},  
 {3,4},{3,5},{3,6},{3,7},{3,8},{3,9},{3,10},{3,11},{4,7},{4,8},{5,6},  
 {5,10},{5,11},{6,7},{6,10},{7,8},{7,10},{8,9},{8,10},{9,10},{10,11}},  
 {{1,2},{1,4},{1,7},{1,8},{2,3},{2,4},{2,7},{2,8},{2,9},{3,6},{3,7},  
 {3,8},{3,9},{3,10},{4,5},{4,7},{4,8},{4,9},{4,10},{4,11},{5,6},{5,7},  
 {5,9},{5,10},{6,7},{6,9},{6,10},{7,8},{7,9},{7,10},{7,11},{8,10},  
 {8,11},{10,11}},{{1,2},{1,3},{1,5},{1,6},{1,7},{1,9},{1,11},{2,3},  
 {2,4},{2,5},{2,6},{2,7},{2,8},{2,11},{3,4},{3,6},{3,7},{4,6},{4,7},  
 {5,6},{5,10},{5,11},{6,7},{6,10},{7,8},{7,9},{7,10},{8,9},{8,10},  
 {8,11},{9,10},{9,11},{10,11}},{{1,2},{1,3},{1,4},{1,5},{1,6},{1,7},  
 {1,8},{1,9},{1,10},{1,11},{2,4},{2,5},{2,6},{2,7},{2,8},{2,11},{3,4},  
 {3,8},{3,11},{4,5},{4,8},{4,10},{4,11},{5,6},{5,9},{5,10},{6,7},{6,8},  
 {6,9},{7,8},{8,9},{8,10},{8,11},{9,10}},{{1,2},{1,3},{1,4},{1,6},  
 {1,7},{1,8},{1,10},{1,11},{2,3},{2,5},{2,6},{2,7},{2,8},{2,9},{2,10},  
 {2,11},{3,6},{3,7},{4,5},{4,7},{4,9},{4,10},{4,11},{5,7},{5,9},{5,10},  
 {6,7},{6,8},{7,8},{7,10},{8,10},{9,10},{9,11},{10,11}},{{1,2},{1,3},  
 {1,4},{1,5},{1,6},{1,8},{2,5},{2,6},{2,7},{2,8},{2,9},{2,10},{3,4},

$\{3,5\}, \{3,6\}, \{3,7\}, \{3,9\}, \{3,10\}, \{4,6\}, \{4,8\}, \{4,10\}, \{4,11\}, \{5,6\}, \{5,7\},$   
 $\{6,7\}, \{6,8\}, \{6,9\}, \{6,10\}, \{6,11\}, \{7,9\}, \{8,10\}, \{8,11\}, \{9,10\}, \{10,11\},$   
 $\{\{1,2\}, \{1,4\}, \{1,5\}, \{1,7\}, \{1,9\}, \{1,10\}, \{1,11\}, \{2,3\}, \{2,4\}, \{2,5\}, \{2,6\},$   
 $\{2,7\}, \{2,8\}, \{2,9\}, \{2,10\}, \{2,11\}, \{3,4\}, \{3,6\}, \{3,7\}, \{3,8\}, \{4,5\}, \{4,6\},$   
 $\{4,7\}, \{4,9\}, \{5,9\}, \{6,8\}, \{6,9\}, \{6,10\}, \{7,8\}, \{7,10\}, \{7,11\}, \{8,10\},$   
 $\{9,10\}, \{10,11\}, \{\{1,2\}, \{1,4\}, \{1,5\}, \{1,6\}, \{1,7\}, \{1,11\}, \{2,4\}, \{2,6\},$   
 $\{2,7\}, \{3,4\}, \{3,5\}, \{3,6\}, \{3,7\}, \{3,8\}, \{3,11\}, \{4,5\}, \{4,6\}, \{4,7\}, \{4,8\},$   
 $\{4,9\}, \{4,10\}, \{5,7\}, \{5,8\}, \{5,9\}, \{5,10\}, \{5,11\}, \{6,7\}, \{6,11\}, \{7,8\}, \{7,9\},$   
 $\{7,10\}, \{7,11\}, \{8,9\}, \{9,10\}, \{\{1,2\}, \{1,3\}, \{1,4\}, \{1,6\}, \{1,8\}, \{1,10\},$   
 $\{2,3\}, \{2,4\}, \{2,5\}, \{2,6\}, \{2,7\}, \{2,9\}, \{2,10\}, \{2,11\}, \{3,4\}, \{3,6\}, \{4,6\},$   
 $\{4,8\}, \{4,9\}, \{5,7\}, \{5,10\}, \{5,11\}, \{6,7\}, \{6,8\}, \{6,9\}, \{6,10\}, \{6,11\},$   
 $\{7,10\}, \{7,11\}, \{8,9\}, \{8,10\}, \{9,10\}, \{9,11\}, \{10,11\}, \{\{1,2\}, \{1,5\}, \{1,7\},$   
 $\{1,8\}, \{1,9\}, \{2,3\}, \{2,4\}, \{2,5\}, \{2,6\}, \{2,7\}, \{2,8\}, \{2,9\}, \{2,10\}, \{2,11\},$   
 $\{3,4\}, \{3,5\}, \{3,9\}, \{3,11\}, \{4,5\}, \{4,6\}, \{4,9\}, \{4,10\}, \{5,6\}, \{5,8\}, \{5,9\},$   
 $\{5,11\}, \{6,8\}, \{6,10\}, \{7,8\}, \{7,9\}, \{8,9\}, \{8,10\}, \{9,10\}, \{9,11\}, \{\{1,2\},$   
 $\{1,4\}, \{1,7\}, \{1,8\}, \{1,9\}, \{2,6\}, \{2,7\}, \{2,8\}, \{2,9\}, \{2,10\}, \{3,4\}, \{3,5\},$   
 $\{3,7\}, \{3,8\}, \{3,11\}, \{4,5\}, \{4,7\}, \{4,8\}, \{4,9\}, \{4,10\}, \{4,11\}, \{5,8\}, \{5,10\},$   
 $\{5,11\}, \{6,7\}, \{6,8\}, \{6,10\}, \{7,8\}, \{7,9\}, \{7,10\}, \{7,11\}, \{8,10\}, \{9,10\},$   
 $\{10,11\}, \{\{1,2\}, \{1,4\}, \{1,5\}, \{1,8\}, \{2,3\}, \{2,4\}, \{2,5\}, \{2,7\}, \{2,8\}, \{2,9\},$   
 $\{3,4\}, \{3,6\}, \{3,7\}, \{3,9\}, \{3,10\}, \{3,11\}, \{4,5\}, \{4,6\}, \{4,7\}, \{4,8\}, \{4,9\},$   
 $\{4,10\}, \{4,11\}, \{5,6\}, \{5,8\}, \{5,9\}, \{6,8\}, \{6,9\}, \{6,10\}, \{6,11\}, \{7,8\},$   
 $\{7,11\}, \{8,11\}, \{9,10\}, \{\{1,2\}, \{1,4\}, \{1,5\}, \{1,6\}, \{1,7\}, \{1,8\}, \{1,9\},$   
 $\{1,10\}, \{2,3\}, \{2,4\}, \{2,8\}, \{2,10\}, \{3,4\}, \{3,8\}, \{3,10\}, \{4,5\}, \{4,6\}, \{4,7\},$   
 $\{4,8\}, \{4,10\}, \{4,11\}, \{5,6\}, \{5,7\}, \{5,9\}, \{6,7\}, \{6,9\}, \{6,10\}, \{6,11\}, \{7,8\},$   
 $\{7,9\}, \{7,11\}, \{8,10\}, \{8,11\}, \{10,11\}, \{\{1,2\}, \{1,3\}, \{1,4\}, \{1,5\}, \{1,6\},$   
 $\{1,7\}, \{1,8\}, \{1,9\}, \{1,10\}, \{1,11\}, \{2,3\}, \{2,4\}, \{2,5\}, \{2,6\}, \{2,10\}, \{2,11\},$   
 $\{3,4\}, \{3,5\}, \{3,7\}, \{3,8\}, \{4,8\}, \{4,11\}, \{5,7\}, \{5,10\}, \{6,9\}, \{6,10\}, \{6,11\},$   
 $\{7,8\}, \{7,9\}, \{7,10\}, \{8,9\}, \{8,11\}, \{9,10\}, \{9,11\}, \{\{1,2\}, \{1,4\}, \{1,5\},$   
 $\{1,6\}, \{1,11\}, \{2,5\}, \{2,6\}, \{2,11\}, \{3,4\}, \{3,5\}, \{3,6\}, \{3,8\}, \{4,5\}, \{4,6\},$   
 $\{4,7\}, \{4,8\}, \{4,9\}, \{4,10\}, \{4,11\}, \{5,6\}, \{5,7\}, \{5,8\}, \{5,9\}, \{5,10\}, \{5,11\},$   
 $\{6,8\}, \{6,11\}, \{7,8\}, \{7,9\}, \{7,10\}, \{7,11\}, \{8,11\}, \{9,10\}, \{10,11\}, \{\{1,2\},$   
 $\{1,3\}, \{1,4\}, \{1,5\}, \{1,6\}, \{1,8\}, \{1,9\}, \{1,10\}, \{2,5\}, \{2,9\}, \{2,10\}, \{2,11\},$   
 $\{3,4\}, \{3,9\}, \{3,10\}, \{3,11\}, \{4,6\}, \{4,8\}, \{4,10\}, \{4,11\}, \{5,6\}, \{5,7\},$   
 $\{5,10\}, \{5,11\}, \{6,7\}, \{6,8\}, \{6,10\}, \{6,11\}, \{7,10\}, \{7,11\}, \{8,10\}, \{9,10\},$   
 $\{9,11\}, \{10,11\}, \{\{1,2\}, \{1,5\}, \{1,6\}, \{1,7\}, \{1,8\}, \{1,9\}, \{1,10\}, \{1,11\},$   
 $\{2,3\}, \{2,6\}, \{2,7\}, \{2,9\}, \{2,10\}, \{2,11\}, \{3,4\}, \{3,5\}, \{3,6\}, \{3,7\}, \{3,9\},$   
 $\{4,5\}, \{4,6\}, \{4,9\}, \{5,6\}, \{5,7\}, \{5,8\}, \{5,9\}, \{6,9\}, \{6,11\}, \{7,8\}, \{7,9\},$   
 $\{7,10\}, \{8,9\}, \{9,10\}, \{9,11\}, \{\{1,2\}, \{1,4\}, \{1,5\}, \{1,8\}, \{1,11\}, \{2,3\},$   
 $\{2,4\}, \{2,5\}, \{2,8\}, \{3,4\}, \{3,5\}, \{3,8\}, \{3,9\}, \{4,5\}, \{4,9\}, \{4,11\}, \{5,6\},$   
 $\{5,7\}, \{5,8\}, \{5,9\}, \{5,10\}, \{5,11\}, \{6,7\}, \{6,8\}, \{6,9\}, \{6,10\}, \{6,11\}, \{7,8\},$   
 $\{7,9\}, \{8,9\}, \{8,11\}, \{9,10\}, \{9,11\}, \{10,11\}, \{\{1,2\}, \{1,3\}, \{1,5\}, \{1,6\},$   
 $\{1,9\}, \{2,3\}, \{2,4\}, \{2,6\}, \{2,9\}, \{2,11\}, \{3,4\}, \{3,5\}, \{3,6\}, \{3,7\}, \{3,8\},$   
 $\{3,9\}, \{3,10\}, \{3,11\}, \{4,5\}, \{4,6\}, \{4,7\}, \{4,8\}, \{4,9\}, \{4,10\}, \{4,11\}, \{5,6\},$   
 $\{5,9\}, \{6,10\}, \{6,11\}, \{7,8\}, \{7,10\}, \{8,10\}, \{8,11\}, \{10,11\}, \{\{1,2\}, \{1,5\},$   
 $\{1,6\}, \{1,7\}, \{1,8\}, \{1,9\}, \{1,11\}, \{2,5\}, \{2,7\}, \{2,8\}, \{3,4\}, \{3,5\}, \{3,6\},$   
 $\{3,8\}, \{3,10\}, \{4,5\}, \{4,6\}, \{4,7\}, \{4,9\}, \{4,10\}, \{4,11\}, \{5,6\}, \{5,7\}, \{5,8\},$   
 $\{6,9\}, \{6,10\}, \{7,8\}, \{7,11\}, \{8,9\}, \{8,10\}, \{8,11\}, \{9,10\}, \{9,11\}, \{\{1,2\},$   
 $\{1,3\}, \{1,5\}, \{1,6\}, \{1,8\}, \{1,11\}, \{2,4\}, \{2,6\}, \{2,7\}, \{2,8\}, \{2,9\}, \{2,10\},$   
 $\{2,11\}, \{3,4\}, \{3,5\}, \{3,6\}, \{3,7\}, \{3,8\}, \{3,9\}, \{3,10\}, \{3,11\}, \{4,6\}, \{4,7\},$   
 $\{4,10\}, \{5,6\}, \{5,11\}, \{6,7\}, \{6,8\}, \{6,9\}, \{6,10\}, \{6,11\}, \{7,9\}, \{8,10\},$

{9,11}}, {{1,2},{1,4},{1,5},{1,6},{1,8},{1,9},{2,5},{2,7},{2,8},{2,9},  
 {3,4},{3,5},{3,6},{3,7},{3,8},{3,10},{4,6},{4,7},{4,8},{4,9},{4,11},  
 {5,6},{5,7},{5,8},{5,10},{6,8},{6,10},{7,8},{7,9},{7,11},{8,9},{8,10},  
 {8,11},{9,11}}, {{1,2},{1,3},{1,5},{1,9},{2,3},{2,4},{2,5},{2,9},  
 {2,10},{3,4},{3,5},{3,6},{3,7},{3,9},{4,5},{4,7},{4,10},{5,6},{5,7},  
 {5,9},{5,10},{5,11},{6,7},{6,9},{7,8},{7,9},{7,10},{7,11},{8,9},  
 {8,10},{8,11},{9,10},{9,11},{10,11}}, {{1,2},{1,3},{1,4},{1,5},{1,7},  
 {1,8},{1,9},{1,10},{2,3},{2,4},{2,5},{2,6},{2,7},{2,8},{2,9},{2,11},  
 {3,4},{3,5},{3,6},{3,7},{3,8},{3,9},{3,10},{3,11},{4,5},{4,9},{4,10},  
 {4,11},{5,6},{5,7},{5,10},{5,11},{6,7},{7,8}}, {{1,2},{1,3},{1,4},  
 {1,6},{1,8},{1,9},{1,10},{1,11},{2,3},{2,4},{2,6},{2,7},{2,9},{2,10},  
 {3,4},{3,5},{3,6},{3,8},{3,9},{4,5},{4,7},{4,8},{4,9},{4,10},{4,11},  
 {5,8},{5,9},{5,11},{6,9},{7,9},{7,10},{8,11},{9,10},{9,11}}, {{1,2},  
 {1,3},{1,4},{1,5},{1,6},{1,7},{1,8},{1,9},{1,10},{1,11},{2,4},{2,6},  
 {2,7},{2,8},{2,9},{2,10},{3,4},{3,5},{3,6},{3,11},{4,6},{4,9},{4,11},  
 {5,6},{5,7},{5,8},{5,9},{5,11},{6,7},{6,10},{7,8},{7,10},{8,9},  
 {9,11}}, {{1,2},{1,3},{1,4},{1,5},{1,8},{1,11},{2,3},{2,4},{2,8},{3,4},  
 {3,5},{3,6},{3,7},{3,8},{3,9},{3,10},{4,5},{4,6},{4,8},{4,10},{4,11},  
 {5,6},{5,7},{5,9},{5,10},{5,11},{6,7},{6,8},{6,9},{6,10},{6,11},{7,9},  
 {8,11},{9,10}}, {{1,2},{1,3},{1,4},{1,6},{1,11},{2,3},{2,4},{2,5},  
 {2,6},{2,7},{2,9},{2,10},{3,4},{3,5},{3,6},{3,7},{3,8},{3,10},{3,11},  
 {4,6},{4,7},{4,8},{4,11},{5,6},{5,7},{5,8},{5,9},{5,10},{6,8},{6,9},  
 {6,10},{6,11},{7,8},{9,10}}, {{1,2},{1,3},{1,4},{1,5},{1,6},{1,7},  
 {1,8},{1,9},{1,11},{2,3},{2,5},{2,6},{2,9},{3,4},{3,5},{3,6},{4,5},  
 {4,6},{4,7},{4,8},{4,9},{4,10},{4,11},{5,7},{5,9},{5,10},{5,11},{6,9},  
 {7,8},{7,9},{7,10},{7,11},{8,9},{9,10}}, {{1,2},{1,3},{1,4},{1,5},  
 {1,6},{1,7},{1,8},{1,9},{1,10},{2,3},{2,5},{2,8},{2,9},{2,10},{2,11},  
 {3,4},{3,5},{3,9},{4,5},{4,6},{4,9},{5,6},{5,8},{5,9},{6,9},{7,8},  
 {7,9},{7,10},{7,11},{8,9},{8,10},{8,11},{9,11},{10,11}}, {{1,2},{1,3},  
 {1,4},{1,5},{1,7},{1,8},{1,10},{2,6},{2,7},{2,8},{2,9},{2,10},{2,11},  
 {3,4},{3,5},{3,6},{3,7},{3,8},{3,9},{3,10},{4,5},{4,7},{4,8},{5,7},  
 {6,7},{6,8},{6,9},{7,8},{8,9},{8,10},{8,11},{9,10},{9,11},{10,11}},  
 {{1,2},{1,3},{1,4},{1,5},{1,6},{1,11},{2,3},{2,4},{2,6},{3,4},{3,5},  
 {3,6},{3,7},{3,11},{4,5},{4,6},{4,7},{4,8},{4,9},{4,10},{4,11},{5,6},  
 {5,7},{5,8},{5,9},{5,11},{6,7},{6,8},{7,8},{7,9},{7,10},{8,9},{8,10},  
 {9,10}}, {{1,2},{1,3},{1,5},{1,8},{1,9},{1,11},{2,3},{2,5},{2,7},{2,8},  
 {3,4},{3,5},{3,7},{3,11},{4,5},{4,6},{4,7},{4,10},{4,11},{5,6},{5,7},  
 {5,8},{5,9},{5,10},{5,11},{6,7},{6,8},{6,9},{6,10},{6,11},{7,8},  
 {7,10},{8,9},{9,11}}, {{1,2},{1,3},{1,4},{1,5},{1,6},{1,7},{1,8},{1,9},  
 {1,11},{2,6},{2,7},{2,8},{3,4},{3,5},{3,9},{3,10},{4,5},{4,10},{4,11},  
 {5,6},{5,7},{5,8},{5,9},{5,10},{5,11},{6,7},{6,8},{7,8},{7,10},{7,11},  
 {8,9},{8,10},{9,10},{10,11}}, {{1,2},{1,3},{1,4},{1,5},{1,6},{1,8},  
 {1,9},{2,4},{2,5},{2,8},{2,9},{2,10},{3,4},{3,5},{3,6},{3,11},{4,5},  
 {4,9},{4,10},{4,11},{5,6},{5,7},{5,8},{5,9},{5,10},{5,11},{6,7},{6,8},  
 {6,11},{7,8},{7,11},{8,10},{8,11},{10,11}}, {{1,2},{1,3},{1,5},{1,6},  
 {1,7},{1,8},{1,9},{1,10},{1,11},{2,5},{2,6},{2,7},{3,5},{3,7},{3,11},  
 {4,5},{4,6},{4,9},{4,11},{5,6},{5,7},{5,9},{5,11},{6,7},{6,8},{6,9},  
 {6,10},{6,11},{7,11},{8,9},{8,10},{8,11},{9,10},{9,11}}, {{1,2},{1,3},  
 {1,4},{1,5},{1,7},{1,9},{1,10},{2,4},{2,6},{2,7},{2,9},{3,4},{3,5},  
 {3,7},{3,8},{3,10},{4,5},{4,6},{4,7},{4,8},{4,9},{4,10},{4,11},{5,8},

{5,9},{5,11},{6,7},{6,9},{6,11},{7,8},{7,10},{7,11},{8,11},{9,11}},  
 {{1,2},{1,3},{1,4},{1,5},{1,6},{1,9},{1,11},{2,3},{2,4},{2,5},{2,8},  
 {2,9},{3,5},{3,6},{3,9},{4,5},{4,8},{4,9},{4,10},{5,6},{5,7},{5,8},  
 {5,9},{5,10},{5,11},{6,7},{6,9},{6,11},{7,9},{7,11},{8,9},{8,10},  
 {9,10},{9,11}},{{1,2},{1,3},{1,7},{1,8},{1,9},{1,10},{2,3},{2,4},  
 {2,5},{2,6},{2,7},{2,8},{2,9},{2,10},{2,11},{3,4},{3,5},{3,6},{3,8},  
 {3,9},{3,10},{4,5},{4,8},{4,9},{5,6},{5,9},{5,11},{6,9},{6,11},{7,8},  
 {7,9},{8,9},{8,10},{9,11}},{{1,2},{1,4},{1,5},{1,7},{1,10},{2,4},  
 {2,5},{2,6},{2,7},{2,8},{2,9},{2,10},{2,11},{3,4},{3,8},{3,9},{3,11},  
 {4,5},{4,8},{4,9},{4,10},{4,11},{5,7},{5,11},{6,7},{6,9},{6,11},{7,9},  
 {7,10},{7,11},{8,9},{8,11},{9,10},{9,11}},{{1,2},{1,4},{1,6},{1,10},  
 {2,4},{2,6},{2,8},{2,9},{2,10},{2,11},{3,4},{3,5},{3,6},{3,8},{3,9},  
 {3,11},{4,5},{4,6},{4,7},{4,8},{4,9},{4,10},{4,11},{5,8},{5,9},{6,7},  
 {6,8},{6,10},{6,11},{7,10},{7,11},{8,9},{9,11},{10,11}},{{1,2},{1,3},  
 {1,4},{1,8},{1,11},{2,3},{2,5},{2,6},{2,8},{2,10},{2,11},{3,4},{3,5},  
 {3,6},{3,7},{3,11},{4,5},{4,8},{4,11},{5,6},{5,7},{5,8},{5,9},{5,10},  
 {5,11},{6,7},{6,9},{6,10},{6,11},{7,11},{8,11},{9,10},{9,11},{10,11}},  
 {{1,2},{1,3},{1,5},{1,6},{1,7},{1,11},{2,5},{2,6},{2,10},{2,11},{3,4},  
 {3,5},{3,6},{3,7},{3,10},{3,11},{4,6},{4,8},{4,9},{4,10},{4,11},{5,6},  
 {5,10},{6,7},{6,8},{6,9},{6,10},{6,11},{7,11},{8,9},{8,10},{9,10},  
 {9,11},{10,11}},{{1,2},{1,3},{1,4},{1,6},{1,9},{2,4},{2,5},{2,6},  
 {2,8},{2,9},{2,10},{2,11},{3,4},{3,6},{3,7},{3,8},{3,9},{4,5},{4,6},  
 {4,8},{5,6},{5,8},{6,7},{6,8},{6,9},{6,10},{6,11},{7,8},{7,9},{8,9},  
 {8,10},{8,11},{9,11},{10,11}},{{1,2},{1,5},{1,6},{1,8},{1,9},{1,10},  
 {1,11},{2,5},{2,6},{2,9},{3,4},{3,5},{3,6},{3,8},{3,9},{3,10},{4,7},  
 {4,8},{4,9},{4,10},{5,6},{5,8},{5,9},{5,11},{6,9},{6,10},{7,8},{7,9},  
 {7,10},{8,9},{8,10},{8,11},{9,10},{9,11}},{{1,2},{1,4},{1,5},{1,10},  
 {2,4},{2,5},{2,6},{2,9},{2,10},{3,4},{3,5},{3,7},{3,8},{3,10},{3,11},  
 {4,5},{4,6},{4,7},{4,9},{4,10},{5,7},{5,9},{5,10},{5,11},{6,7},{6,9},  
 {6,10},{7,8},{7,9},{7,10},{7,11},{8,10},{8,11},{10,11}},{{1,2},{1,3},  
 {1,5},{1,6},{1,11},{2,3},{2,5},{2,6},{3,4},{3,5},{3,6},{3,7},{3,8},  
 {3,9},{3,10},{3,11},{4,5},{4,7},{4,8},{4,9},{4,10},{4,11},{5,6},{5,9},  
 {5,11},{6,7},{6,9},{6,11},{7,9},{7,10},{7,11},{8,9},{8,10},{9,10}},  
 {{1,2},{1,3},{1,4},{1,5},{1,6},{1,7},{1,8},{1,9},{1,10},{1,11},{2,3},  
 {2,4},{2,6},{2,7},{2,8},{2,10},{3,4},{3,6},{4,5},{4,6},{4,8},{4,9},  
 {5,6},{5,9},{5,10},{5,11},{6,10},{7,8},{7,9},{7,10},{7,11},{8,9},  
 {9,11},{10,11}},{{1,2},{1,3},{1,4},{1,5},{1,6},{1,7},{1,10},{2,4},  
 {2,7},{2,8},{2,9},{2,11},{3,4},{3,5},{3,6},{3,8},{3,10},{4,5},{4,8},  
 {4,9},{5,6},{5,7},{5,9},{5,10},{6,7},{6,8},{6,10},{7,8},{7,9},{7,11},  
 {8,9},{8,11},{9,11}},{{1,2},{1,4},{1,5},{1,7},{1,8},{1,9},{1,10},  
 {2,3},{2,4},{2,5},{2,6},{2,8},{2,9},{2,11},{3,4},{3,5},{3,9},{3,10},  
 {4,5},{4,6},{4,7},{4,10},{4,11},{5,6},{5,7},{5,8},{5,9},{5,10},{5,11},  
 {6,7},{6,8},{6,11},{7,8},{9,10}},{{1,2},{1,5},{1,6},{1,8},{2,3},{2,4},  
 {2,5},{2,6},{2,7},{2,8},{2,9},{2,10},{3,4},{3,6},{3,8},{4,5},{4,6},  
 {4,8},{4,10},{5,6},{5,7},{5,8},{5,9},{5,10},{5,11},{6,7},{6,8},{6,10},  
 {6,11},{7,9},{7,10},{7,11},{9,10},{10,11}},{{1,2},{1,3},{1,4},{1,5},  
 {1,6},{1,9},{1,10},{2,4},{2,5},{2,6},{2,7},{2,9},{2,10},{3,4},{3,5},  
 {3,8},{3,10},{3,11},{4,5},{4,6},{4,7},{4,8},{4,9},{4,10},{4,11},{5,6},  
 {5,7},{5,8},{5,10},{5,11},{7,10},{8,11},{9,10},{10,11}},{{1,2},{1,3},  
 {1,6},{1,7},{2,3},{2,4},{2,5},{2,6},{2,7},{2,8},{2,9},{2,11},{3,4},



$\{3,5\}, \{3,6\}, \{3,7\}, \{3,8\}, \{3,11\}, \{4,5\}, \{4,6\}, \{4,11\}, \{5,6\}, \{5,7\}, \{5,8\},$   
 $\{5,9\}, \{5,10\}, \{5,11\}, \{6,7\}, \{7,8\}, \{7,9\}, \{7,10\}, \{8,9\}, \{8,10\}, \{9,10\},$   
 $\{\{1,2\}, \{1,4\}, \{1,5\}, \{1,7\}, \{1,8\}, \{1,9\}, \{1,10\}, \{2,4\}, \{2,6\}, \{2,8\}, \{2,9\},$   
 $\{2,10\}, \{3,4\}, \{3,7\}, \{3,8\}, \{3,9\}, \{3,11\}, \{4,7\}, \{4,8\}, \{4,9\}, \{4,11\}, \{5,6\},$   
 $\{5,8\}, \{5,9\}, \{5,10\}, \{6,8\}, \{6,9\}, \{6,10\}, \{7,8\}, \{7,9\}, \{7,11\}, \{8,9\}, \{8,11\},$   
 $\{9,10\}\}, \{\{1,2\}, \{1,3\}, \{1,4\}, \{1,5\}, \{1,6\}, \{1,7\}, \{1,8\}, \{1,10\}, \{1,11\},$   
 $\{2,4\}, \{2,5\}, \{2,8\}, \{2,11\}, \{3,4\}, \{3,6\}, \{3,8\}, \{3,10\}, \{4,5\}, \{4,6\}, \{4,7\},$   
 $\{4,8\}, \{4,9\}, \{4,10\}, \{4,11\}, \{5,11\}, \{6,7\}, \{6,8\}, \{6,9\}, \{6,10\}, \{6,11\},$   
 $\{7,10\}, \{8,9\}, \{8,11\}, \{9,11\}\}, \{\{1,2\}, \{1,3\}, \{1,7\}, \{1,8\}, \{1,9\}, \{1,11\},$   
 $\{2,4\}, \{2,5\}, \{2,7\}, \{2,8\}, \{2,9\}, \{2,11\}, \{3,4\}, \{3,5\}, \{3,6\}, \{3,8\}, \{3,9\},$   
 $\{3,10\}, \{3,11\}, \{4,5\}, \{4,6\}, \{4,8\}, \{4,9\}, \{5,6\}, \{5,8\}, \{5,10\}, \{5,11\}, \{6,8\},$   
 $\{7,8\}, \{7,11\}, \{8,9\}, \{8,10\}, \{8,11\}, \{10,11\}\}, \{\{1,2\}, \{1,4\}, \{1,5\}, \{1,9\},$   
 $\{1,10\}, \{2,3\}, \{2,4\}, \{2,5\}, \{2,6\}, \{2,7\}, \{2,8\}, \{2,9\}, \{2,10\}, \{2,11\}, \{3,4\},$   
 $\{3,5\}, \{3,9\}, \{4,5\}, \{4,9\}, \{5,6\}, \{5,7\}, \{5,8\}, \{5,9\}, \{5,10\}, \{5,11\}, \{6,8\},$   
 $\{6,10\}, \{6,11\}, \{7,8\}, \{7,11\}, \{8,9\}, \{8,10\}, \{8,11\}, \{9,10\}\}, \{\{1,2\}, \{1,3\},$   
 $\{1,6\}, \{1,7\}, \{1,8\}, \{1,9\}, \{1,10\}, \{1,11\}, \{2,3\}, \{2,4\}, \{2,5\}, \{2,6\}, \{2,7\},$   
 $\{2,8\}, \{2,10\}, \{2,11\}, \{3,4\}, \{3,5\}, \{3,6\}, \{3,8\}, \{3,9\}, \{3,10\}, \{3,11\}, \{4,5\},$   
 $\{4,6\}, \{4,9\}, \{4,10\}, \{5,10\}, \{6,9\}, \{6,11\}, \{7,8\}, \{7,10\}, \{8,10\}, \{9,10\}\},$   
 $\{\{1,2\}, \{1,3\}, \{1,4\}, \{1,5\}, \{2,3\}, \{2,4\}, \{2,5\}, \{2,6\}, \{2,7\}, \{2,10\}, \{3,4\},$   
 $\{3,5\}, \{3,6\}, \{3,7\}, \{3,8\}, \{3,9\}, \{3,10\}, \{4,5\}, \{4,6\}, \{4,7\}, \{4,9\}, \{4,10\},$   
 $\{4,11\}, \{5,7\}, \{6,7\}, \{6,8\}, \{6,9\}, \{6,10\}, \{6,11\}, \{7,8\}, \{7,9\}, \{7,11\}, \{8,9\},$   
 $\{9,11\}\}, \{\{1,2\}, \{1,3\}, \{1,4\}, \{1,5\}, \{1,6\}, \{1,7\}, \{1,8\}, \{1,9\}, \{1,10\},$   
 $\{1,11\}, \{2,3\}, \{2,4\}, \{2,6\}, \{2,10\}, \{2,11\}, \{3,4\}, \{3,6\}, \{3,8\}, \{3,9\}, \{4,7\},$   
 $\{4,8\}, \{4,10\}, \{5,6\}, \{5,7\}, \{5,9\}, \{5,10\}, \{5,11\}, \{6,9\}, \{6,11\}, \{7,8\}, \{7,9\},$   
 $\{7,10\}, \{8,9\}, \{10,11\}\}, \{\{1,2\}, \{1,5\}, \{1,6\}, \{1,8\}, \{1,9\}, \{1,11\}, \{2,3\},$   
 $\{2,5\}, \{2,8\}, \{2,9\}, \{2,11\}, \{3,4\}, \{3,5\}, \{3,6\}, \{3,9\}, \{3,10\}, \{3,11\}, \{4,6\},$   
 $\{4,7\}, \{4,9\}, \{4,10\}, \{5,6\}, \{5,8\}, \{5,9\}, \{6,7\}, \{6,9\}, \{6,11\}, \{7,9\}, \{7,10\},$   
 $\{7,11\}, \{8,9\}, \{9,10\}, \{9,11\}, \{10,11\}\}, \{\{1,2\}, \{1,3\}, \{1,4\}, \{1,6\}, \{1,7\},$   
 $\{1,8\}, \{1,9\}, \{1,11\}, \{2,3\}, \{2,4\}, \{2,5\}, \{2,6\}, \{2,8\}, \{2,9\}, \{2,10\}, \{2,11\},$   
 $\{3,4\}, \{3,5\}, \{3,6\}, \{3,7\}, \{3,8\}, \{3,9\}, \{3,10\}, \{4,5\}, \{4,9\}, \{4,10\}, \{4,11\},$   
 $\{5,6\}, \{5,10\}, \{5,11\}, \{6,11\}, \{7,8\}, \{7,9\}, \{8,9\}\}, \{\{1,2\}, \{1,3\}, \{1,5\},$   
 $\{1,6\}, \{1,10\}, \{2,3\}, \{2,4\}, \{2,5\}, \{2,6\}, \{2,9\}, \{2,10\}, \{3,4\}, \{3,5\}, \{3,6\},$   
 $\{3,7\}, \{3,8\}, \{3,10\}, \{3,11\}, \{4,8\}, \{4,9\}, \{4,10\}, \{5,6\}, \{5,7\}, \{5,8\}, \{5,9\},$   
 $\{5,10\}, \{5,11\}, \{7,8\}, \{7,11\}, \{8,9\}, \{8,10\}, \{8,11\}, \{9,10\}, \{10,11\}\}, \{\{1,2\},$   
 $\{1,5\}, \{1,7\}, \{1,9\}, \{1,11\}, \{2,3\}, \{2,5\}, \{2,7\}, \{2,8\}, \{2,9\}, \{2,10\}, \{3,4\},$   
 $\{3,7\}, \{3,8\}, \{3,9\}, \{3,10\}, \{3,11\}, \{4,5\}, \{4,6\}, \{4,8\}, \{4,9\}, \{4,11\}, \{5,6\},$   
 $\{5,8\}, \{5,9\}, \{5,11\}, \{6,8\}, \{6,11\}, \{7,9\}, \{7,10\}, \{7,11\}, \{8,11\}, \{9,10\}\},$   
 $\{\{1,2\}, \{1,4\}, \{1,5\}, \{1,9\}, \{1,10\}, \{2,3\}, \{2,4\}, \{2,5\}, \{2,6\}, \{2,7\}, \{2,8\},$   
 $\{2,9\}, \{2,10\}, \{2,11\}, \{3,4\}, \{3,8\}, \{3,9\}, \{3,11\}, \{4,5\}, \{4,6\}, \{4,8\}, \{4,9\},$   
 $\{5,6\}, \{5,7\}, \{5,8\}, \{5,10\}, \{6,8\}, \{7,8\}, \{7,10\}, \{7,11\}, \{8,11\}, \{9,10\},$   
 $\{9,11\}, \{10,11\}\}, \{\{1,2\}, \{1,3\}, \{1,6\}, \{1,7\}, \{1,10\}, \{2,3\}, \{2,5\}, \{2,6\},$   
 $\{2,7\}, \{2,11\}, \{3,4\}, \{3,6\}, \{3,8\}, \{3,9\}, \{3,10\}, \{3,11\}, \{4,5\}, \{4,7\}, \{4,8\},$   
 $\{4,9\}, \{4,10\}, \{4,11\}, \{5,6\}, \{5,7\}, \{5,10\}, \{5,11\}, \{6,10\}, \{7,10\}, \{7,11\},$   
 $\{8,9\}, \{8,11\}, \{9,11\}\}, \{\{1,2\}, \{1,4\}, \{1,5\}, \{1,6\}, \{1,7\}, \{1,8\}, \{1,9\},$   
 $\{1,10\}, \{1,11\}, \{2,4\}, \{2,5\}, \{2,10\}, \{3,4\}, \{3,5\}, \{3,6\}, \{3,10\}, \{4,5\}, \{4,6\},$   
 $\{4,7\}, \{4,10\}, \{4,11\}, \{5,6\}, \{5,10\}, \{5,11\}, \{6,7\}, \{6,8\}, \{6,10\}, \{6,11\},$   
 $\{7,8\}, \{7,9\}, \{7,10\}, \{8,9\}, \{8,10\}, \{9,10\}\}, \{\{1,2\}, \{1,3\}, \{1,5\}, \{1,6\},$   
 $\{1,7\}, \{1,9\}, \{1,10\}, \{2,3\}, \{2,4\}, \{2,5\}, \{2,6\}, \{2,7\}, \{2,8\}, \{2,9\}, \{2,11\},$   
 $\{3,4\}, \{3,5\}, \{3,6\}, \{3,7\}, \{3,8\}, \{3,9\}, \{3,10\}, \{3,11\}, \{4,5\}, \{4,7\}, \{4,8\},$   
 $\{4,10\}, \{5,6\}, \{5,10\}, \{6,9\}, \{6,11\}, \{7,8\}, \{7,10\}, \{9,11\}\}, \{\{1,2\}, \{1,3\},$

$\{1,4\},\{1,7\},\{1,8\},\{1,10\},\{2,3\},\{2,4\},\{2,7\},\{2,8\},\{2,9\},\{2,10\},\{2,11\},$   
 $\{3,4\},\{3,7\},\{3,8\},\{4,5\},\{4,6\},\{4,7\},\{4,9\},\{4,10\},\{4,11\},\{5,6\},\{5,7\},$   
 $\{5,9\},\{5,10\},\{6,7\},\{6,9\},\{7,8\},\{7,9\},\{7,10\},\{9,10\},\{9,11\},\{10,11\}\},$   
 $\{\{1,2\},\{1,3\},\{1,4\},\{1,7\},\{1,9\},\{1,10\},\{2,3\},\{2,4\},\{2,8\},\{2,9\},\{3,4\},$   
 $\{3,5\},\{3,6\},\{3,8\},\{3,9\},\{3,10\},\{3,11\},\{4,5\},\{4,6\},\{4,7\},\{4,8\},\{4,9\},$   
 $\{4,10\},\{4,11\},\{5,6\},\{5,11\},\{6,8\},\{6,9\},\{6,11\},\{7,9\},\{7,10\},\{8,9\},$   
 $\{8,11\},\{9,10\}\},\{\{1,2\},\{1,4\},\{1,5\},\{1,6\},\{1,8\},\{1,11\},\{2,3\},\{2,4\},$   
 $\{2,6\},\{2,7\},\{2,8\},\{3,4\},\{3,5\},\{3,7\},\{3,8\},\{3,9\},\{3,10\},\{3,11\},\{4,5\},$   
 $\{4,9\},\{4,10\},\{4,11\},\{5,8\},\{5,9\},\{5,10\},\{5,11\},\{6,7\},\{6,8\},\{6,11\},$   
 $\{7,8\},\{7,11\},\{9,10\},\{10,11\}\},\{\{1,2\},\{1,6\},\{1,7\},\{1,10\},\{2,3\},\{2,4\},$   
 $\{2,5\},\{2,6\},\{2,7\},\{2,8\},\{2,9\},\{2,10\},\{3,4\},\{3,9\},\{3,10\},\{4,5\},\{4,6\},$   
 $\{4,7\},\{4,9\},\{4,10\},\{4,11\},\{5,6\},\{5,8\},\{5,9\},\{5,10\},\{5,11\},\{6,7\},$   
 $\{6,10\},\{6,11\},\{7,10\},\{8,9\},\{8,10\},\{9,10\},\{10,11\}\},\{\{1,2\},\{1,3\},\{1,8\},$   
 $\{1,9\},\{1,11\},\{2,3\},\{2,4\},\{2,5\},\{2,6\},\{2,8\},\{2,9\},\{2,10\},\{2,11\},\{3,4\},$   
 $\{3,5\},\{3,6\},\{3,8\},\{3,11\},\{4,5\},\{4,6\},\{5,6\},\{5,7\},\{5,8\},\{5,9\},\{5,10\},$   
 $\{5,11\},\{6,7\},\{6,8\},\{6,10\},\{7,8\},\{7,10\},\{8,9\},\{8,10\},\{9,11\}\},\{\{1,2\},$   
 $\{1,4\},\{1,5\},\{1,6\},\{1,7\},\{1,8\},\{1,9\},\{1,11\},\{2,4\},\{2,6\},\{2,7\},\{2,10\},$   
 $\{2,11\},\{3,4\},\{3,6\},\{3,9\},\{3,10\},\{4,5\},\{4,6\},\{4,8\},\{4,9\},\{4,10\},\{4,11\},$   
 $\{5,6\},\{5,9\},\{6,7\},\{6,8\},\{6,9\},\{6,10\},\{6,11\},\{7,9\},\{7,10\},\{8,11\},$   
 $\{9,10\}\},\{\{1,2\},\{1,5\},\{1,7\},\{1,8\},\{1,9\},\{1,11\},\{2,3\},\{2,5\},\{2,6\},\{2,7\},$   
 $\{2,8\},\{2,9\},\{3,5\},\{3,6\},\{3,9\},\{4,5\},\{4,6\},\{4,8\},\{4,9\},\{4,10\},\{5,6\},$   
 $\{5,8\},\{5,9\},\{5,10\},\{6,8\},\{6,9\},\{7,8\},\{7,9\},\{7,11\},\{8,9\},\{8,10\},\{8,11\},$   
 $\{9,10\},\{9,11\}\},\{\{1,2\},\{1,3\},\{1,4\},\{1,5\},\{1,6\},\{1,7\},\{2,3\},\{2,4\},\{2,5\},$   
 $\{3,4\},\{3,5\},\{3,7\},\{3,11\},\{4,5\},\{4,6\},\{4,11\},\{5,6\},\{5,7\},\{5,8\},\{5,11\},$   
 $\{6,7\},\{6,8\},\{6,9\},\{6,10\},\{6,11\},\{7,8\},\{7,9\},\{7,10\},\{7,11\},\{8,9\},$   
 $\{8,11\},\{9,10\},\{9,11\},\{10,11\}\},\{\{1,2\},\{1,3\},\{1,5\},\{1,6\},\{1,9\},\{1,10\},$   
 $\{2,3\},\{2,4\},\{2,5\},\{2,6\},\{2,7\},\{2,8\},\{2,11\},\{3,4\},\{3,5\},\{3,6\},\{3,7\},$   
 $\{3,8\},\{3,9\},\{3,10\},\{3,11\},\{4,8\},\{4,11\},\{5,6\},\{5,7\},\{5,9\},\{5,10\},\{6,7\},$   
 $\{6,8\},\{6,10\},\{7,8\},\{7,11\},\{8,11\},\{9,10\}\},\{\{1,2\},\{1,4\},\{1,5\},\{1,7\},$   
 $\{1,8\},\{2,3\},\{2,4\},\{2,5\},\{2,8\},\{3,4\},\{3,5\},\{3,8\},\{3,11\},\{4,5\},\{4,7\},$   
 $\{4,9\},\{4,10\},\{4,11\},\{5,6\},\{5,7\},\{5,8\},\{5,9\},\{5,10\},\{5,11\},\{6,7\},\{6,8\},$   
 $\{6,9\},\{7,8\},\{7,9\},\{7,10\},\{8,9\},\{8,11\},\{9,10\},\{9,11\}\},\{\{1,2\},\{1,3\},$   
 $\{1,5\},\{1,6\},\{1,7\},\{1,8\},\{1,9\},\{1,10\},\{1,11\},\{2,6\},\{2,7\},\{2,9\},\{2,10\},$   
 $\{3,4\},\{3,6\},\{3,7\},\{3,8\},\{3,9\},\{3,11\},\{4,5\},\{4,6\},\{4,7\},\{4,11\},\{5,6\},$   
 $\{5,7\},\{5,11\},\{6,7\},\{6,8\},\{6,9\},\{6,10\},\{7,9\},\{7,10\},\{7,11\},\{8,9\}\},$   
 $\{\{1,2\},\{1,4\},\{1,5\},\{1,8\},\{1,10\},\{1,11\},\{2,3\},\{2,4\},\{2,5\},\{2,7\},\{2,8\},$   
 $\{2,10\},\{3,4\},\{3,7\},\{3,8\},\{3,9\},\{4,6\},\{4,7\},\{4,8\},\{4,9\},\{4,11\},\{5,8\},$   
 $\{5,10\},\{6,7\},\{6,8\},\{6,11\},\{7,8\},\{7,9\},\{7,10\},\{7,11\},\{8,9\},\{8,10\},$   
 $\{8,11\},\{10,11\}\},\{\{1,2\},\{1,3\},\{1,4\},\{1,5\},\{1,8\},\{1,9\},\{1,10\},\{2,5\},$   
 $\{2,6\},\{2,8\},\{2,9\},\{3,4\},\{3,5\},\{3,6\},\{3,7\},\{3,9\},\{3,10\},\{3,11\},\{4,5\},$   
 $\{4,10\},\{5,6\},\{5,7\},\{5,8\},\{5,9\},\{5,10\},\{5,11\},\{6,7\},\{6,8\},\{6,9\},\{7,8\},$   
 $\{7,11\},\{8,10\},\{8,11\},\{10,11\}\},\{\{1,2\},\{1,3\},\{1,5\},\{1,6\},\{1,8\},\{1,11\},$   
 $\{2,3\},\{2,5\},\{2,6\},\{2,7\},\{2,11\},\{3,4\},\{3,5\},\{3,6\},\{3,11\},\{4,5\},\{4,6\},$   
 $\{4,7\},\{4,8\},\{4,9\},\{4,10\},\{5,7\},\{5,8\},\{6,7\},\{6,8\},\{6,9\},\{6,10\},\{6,11\},$   
 $\{7,8\},\{7,9\},\{8,9\},\{8,10\},\{9,10\}\},\{\{1,2\},\{1,3\},\{1,5\},\{1,8\},\{1,9\},$   
 $\{1,10\},\{2,3\},\{2,4\},\{2,5\},\{2,6\},\{2,7\},\{2,8\},\{2,9\},\{2,10\},\{2,11\},\{3,5\},$   
 $\{3,6\},\{3,8\},\{4,7\},\{4,8\},\{4,9\},\{4,11\},\{5,6\},\{5,10\},\{6,7\},\{6,8\},\{6,9\},$   
 $\{6,10\},\{7,8\},\{7,9\},\{8,9\},\{8,11\},\{9,10\},\{9,11\}\},\{\{1,2\},\{1,3\},\{1,4\},$   
 $\{1,5\},\{1,6\},\{1,8\},\{2,3\},\{2,4\},\{2,5\},\{2,6\},\{2,7\},\{2,8\},\{2,9\},\{2,10\},$   
 $\{2,11\},\{3,4\},\{3,6\},\{3,7\},\{3,11\},\{4,6\},\{4,7\},\{4,8\},\{4,10\},\{5,6\},\{5,8\},$

{6,7},{6,8},{6,9},{6,10},{6,11},{7,9},{7,10},{7,11},{9,10}},{1,2},  
{1,3},{1,5},{1,6},{1,7},{1,8},{1,9},{1,10},{1,11},{2,3},{2,4},{2,5},  
{2,6},{2,7},{2,8},{2,10},{3,7},{3,8},{3,9},{3,11},{4,6},{4,7},{4,10},  
{5,6},{5,8},{6,7},{6,8},{6,9},{6,10},{7,9},{7,10},{7,11},{8,9},  
{9,11}},{1,2},{1,4},{1,5},{1,6},{2,3},{2,4},{2,5},{2,9},{3,4},{3,5},  
{3,7},{3,9},{4,6},{4,7},{4,8},{4,9},{5,6},{5,7},{5,9},{5,10},{5,11},  
{6,7},{6,8},{6,10},{6,11},{7,8},{7,10},{7,11},{8,9},{8,10},{9,10},  
{10,11}},{1,2},{1,3},{1,4},{1,5},{1,6},{2,4},{2,5},{2,6},{3,4},{3,5},  
{3,6},{3,7},{3,8},{3,10},{3,11},{4,5},{4,6},{4,8},{4,11},{5,6},{5,7},  
{5,8},{5,9},{5,10},{6,10},{6,11},{7,8},{7,9},{7,10},{8,9},{8,10},  
{8,11},{9,10},{10,11}},{1,2},{1,5},{1,6},{1,7},{1,9},{2,3},{2,5},  
{2,6},{2,9},{3,4},{3,5},{3,6},{3,7},{3,8},{3,9},{3,10},{3,11},{4,5},  
{4,7},{4,11},{5,6},{5,7},{5,11},{6,7},{6,8},{6,9},{6,10},{6,11},{7,8},  
{7,9},{7,10},{7,11},{8,10},{9,10}},{1,2},{1,3},{1,7},{1,8},{1,10},  
{2,3},{2,4},{2,6},{2,7},{2,10},{2,11},{3,4},{3,5},{3,6},{3,7},{3,8},  
{3,9},{3,10},{3,11},{4,6},{4,7},{4,11},{5,6},{5,7},{5,8},{5,9},{5,10},  
{6,7},{6,10},{6,11},{7,8},{7,9},{8,9},{8,10}},{1,2},{1,4},{1,5},  
{1,7},{1,8},{2,3},{2,5},{2,6},{2,7},{2,8},{3,4},{3,5},{3,6},{3,7},  
{3,8},{3,9},{3,11},{4,5},{4,7},{4,8},{4,9},{4,10},{4,11},{5,6},{5,7},  
{5,8},{5,9},{5,10},{6,7},{7,9},{7,10},{7,11},{9,10},{9,11}},{1,2},  
{1,3},{1,5},{1,6},{1,8},{1,9},{2,3},{2,4},{2,5},{2,6},{2,8},{2,9},  
{2,10},{3,5},{3,6},{4,7},{4,8},{4,9},{4,10},{4,11},{5,6},{5,8},{6,7},  
{6,8},{6,9},{6,10},{6,11},{7,8},{7,9},{7,11},{8,9},{9,10},{9,11},  
{10,11}},{1,2},{1,3},{1,4},{1,5},{1,7},{1,8},{1,9},{1,10},{1,11},  
{2,3},{2,7},{2,8},{2,9},{2,11},{3,4},{3,7},{3,8},{3,11},{4,8},{4,11},  
{5,6},{5,7},{5,8},{5,9},{5,10},{6,7},{6,8},{6,9},{7,8},{7,9},{7,10},  
{8,9},{8,11},{9,10}},{1,2},{1,3},{1,4},{1,5},{1,6},{1,7},{1,8},{1,9},  
{1,10},{2,3},{2,4},{2,5},{3,4},{3,5},{3,8},{3,9},{3,10},{4,5},{4,6},  
{4,7},{4,8},{4,10},{4,11},{5,10},{6,7},{6,8},{6,9},{6,10},{6,11},  
{7,8},{7,11},{8,9},{8,11},{9,10}},{1,2},{1,3},{1,4},{1,6},{1,7},  
{1,10},{1,11},{2,3},{2,6},{2,9},{2,10},{2,11},{3,4},{3,5},{3,6},{3,7},  
{3,8},{3,9},{3,10},{4,6},{4,7},{5,6},{5,8},{5,10},{6,7},{6,8},{6,9},  
{6,10},{6,11},{7,10},{8,9},{8,10},{9,10},{10,11}},{1,2},{1,4},{1,5},  
{1,6},{1,7},{1,8},{2,5},{2,7},{2,8},{2,9},{2,11},{3,4},{3,5},{3,6},  
{3,7},{3,8},{3,9},{3,10},{3,11},{4,5},{4,6},{4,7},{4,10},{5,7},{5,11},  
{6,7},{6,8},{6,10},{7,8},{7,9},{7,10},{7,11},{8,9},{9,11}},{1,2},  
{1,4},{1,5},{1,6},{1,7},{1,10},{2,4},{2,5},{2,6},{2,9},{2,10},{3,4},  
{3,5},{3,6},{3,7},{3,8},{3,9},{3,10},{3,11},{4,5},{4,7},{4,8},{4,9},  
{5,10},{6,7},{6,9},{6,10},{7,8},{7,9},{7,11},{8,9},{8,11},{9,11}},  
{1,2},{1,3},{1,4},{1,5},{1,6},{1,7},{1,8},{1,9},{2,3},{2,4},{2,5},  
{2,6},{2,7},{2,8},{2,9},{2,10},{2,11},{3,4},{3,7},{4,7},{4,8},{4,9},  
{4,10},{5,6},{5,8},{5,9},{5,10},{5,11},{6,8},{7,8},{8,10},{8,11},  
{9,10},{10,11}},{1,2},{1,3},{1,7},{1,8},{1,9},{1,11},{2,6},{2,7},  
{2,8},{2,9},{3,5},{3,8},{3,11},{4,5},{4,6},{4,7},{4,8},{4,9},{4,10},  
{5,7},{5,8},{5,10},{5,11},{6,7},{6,8},{6,9},{7,10},{7,11},{8,9},  
{9,10},{9,11},{10,11}},{1,2},{1,4},{1,5},{1,6},{1,7},{1,8},{1,9},  
{1,10},{2,3},{2,4},{2,7},{2,8},{3,4},{3,5},{3,7},{3,8},{4,5},{4,6},  
{4,7},{4,8},{4,9},{4,10},{4,11},{5,6},{5,7},{5,8},{5,9},{6,9},{8,9},  
{8,10},{8,11},{9,10},{9,11},{10,11}},{1,2},{1,3},{1,4},{1,5},{1,6},  
{1,7},{1,8},{1,10},{1,11},{2,4},{2,6},{2,8},{2,10},{3,4},{3,5},{3,9},

$\{3, 11\}, \{4, 5\}, \{4, 6\}, \{4, 7\}, \{4, 8\}, \{4, 9\}, \{4, 10\}, \{4, 11\}, \{5, 7\}, \{5, 9\}, \{6, 10\},$   
 $\{7, 8\}, \{7, 9\}, \{8, 9\}, \{8, 10\}, \{9, 10\}, \{9, 11\}, \{10, 11\}, \{\{1, 2\}, \{1, 3\}, \{1, 5\},$   
 $\{1, 10\}, \{2, 3\}, \{2, 4\}, \{2, 5\}, \{2, 6\}, \{2, 7\}, \{2, 10\}, \{2, 11\}, \{3, 4\}, \{3, 5\}, \{3, 6\},$   
 $\{3, 7\}, \{3, 8\}, \{3, 9\}, \{3, 10\}, \{4, 5\}, \{4, 6\}, \{4, 7\}, \{5, 6\}, \{5, 7\}, \{5, 8\}, \{5, 10\},$   
 $\{5, 11\}, \{6, 8\}, \{6, 9\}, \{6, 10\}, \{6, 11\}, \{8, 9\}, \{8, 10\}, \{9, 10\}, \{10, 11\}, \{\{1, 2\},$   
 $\{1, 3\}, \{1, 8\}, \{1, 9\}, \{2, 3\}, \{2, 4\}, \{2, 5\}, \{2, 6\}, \{2, 8\}, \{2, 9\}, \{2, 10\}, \{3, 4\},$   
 $\{3, 5\}, \{3, 6\}, \{3, 7\}, \{3, 8\}, \{3, 9\}, \{3, 10\}, \{3, 11\}, \{4, 5\}, \{4, 8\}, \{5, 7\}, \{5, 8\},$   
 $\{5, 10\}, \{6, 7\}, \{6, 9\}, \{6, 10\}, \{6, 11\}, \{7, 8\}, \{7, 9\}, \{7, 10\}, \{7, 11\}, \{8, 9\},$   
 $\{10, 11\}, \{\{1, 2\}, \{1, 4\}, \{1, 6\}, \{1, 8\}, \{1, 10\}, \{1, 11\}, \{2, 3\}, \{2, 4\}, \{2, 5\},$   
 $\{2, 6\}, \{2, 7\}, \{2, 8\}, \{2, 9\}, \{2, 10\}, \{2, 11\}, \{3, 4\}, \{3, 9\}, \{3, 10\}, \{4, 5\}, \{4, 6\},$   
 $\{4, 7\}, \{4, 8\}, \{4, 9\}, \{4, 10\}, \{4, 11\}, \{5, 6\}, \{5, 8\}, \{6, 8\}, \{6, 11\}, \{7, 8\}, \{7, 9\},$   
 $\{8, 9\}, \{8, 10\}, \{9, 10\}, \{\{1, 2\}, \{1, 4\}, \{1, 5\}, \{1, 6\}, \{1, 7\}, \{1, 9\}, \{1, 10\},$   
 $\{2, 4\}, \{2, 5\}, \{2, 6\}, \{2, 7\}, \{2, 11\}, \{3, 4\}, \{3, 7\}, \{3, 8\}, \{3, 9\}, \{3, 10\}, \{3, 11\},$   
 $\{4, 5\}, \{4, 8\}, \{4, 9\}, \{4, 10\}, \{4, 11\}, \{6, 7\}, \{6, 10\}, \{6, 11\}, \{7, 9\}, \{7, 11\},$   
 $\{8, 10\}, \{8, 11\}, \{9, 10\}, \{10, 11\}, \{\{1, 2\}, \{1, 3\}, \{1, 6\}, \{1, 8\}, \{1, 9\}, \{1, 10\},$   
 $\{2, 3\}, \{2, 4\}, \{2, 5\}, \{2, 6\}, \{2, 7\}, \{2, 9\}, \{2, 11\}, \{3, 4\}, \{3, 6\}, \{3, 7\}, \{3, 9\},$   
 $\{3, 10\}, \{4, 5\}, \{4, 6\}, \{4, 7\}, \{4, 9\}, \{4, 11\}, \{5, 6\}, \{5, 11\}, \{6, 7\}, \{6, 8\}, \{6, 9\},$   
 $\{6, 10\}, \{6, 11\}, \{7, 11\}, \{8, 9\}, \{8, 10\}, \{9, 10\}, \{\{1, 2\}, \{1, 3\}, \{1, 7\}, \{1, 8\},$   
 $\{2, 3\}, \{2, 4\}, \{2, 7\}, \{2, 8\}, \{2, 9\}, \{2, 11\}, \{3, 4\}, \{3, 5\}, \{3, 6\}, \{3, 7\}, \{3, 8\},$   
 $\{4, 5\}, \{4, 6\}, \{4, 7\}, \{4, 8\}, \{4, 9\}, \{4, 10\}, \{5, 6\}, \{5, 7\}, \{6, 7\}, \{6, 8\}, \{6, 10\},$   
 $\{7, 8\}, \{7, 9\}, \{7, 10\}, \{7, 11\}, \{8, 9\}, \{8, 10\}, \{8, 11\}, \{9, 11\}, \{\{1, 2\}, \{1, 3\},$   
 $\{1, 4\}, \{1, 5\}, \{1, 7\}, \{1, 8\}, \{1, 9\}, \{1, 10\}, \{2, 3\}, \{2, 4\}, \{2, 7\}, \{2, 8\}, \{3, 4\},$   
 $\{3, 5\}, \{3, 8\}, \{3, 9\}, \{3, 11\}, \{4, 5\}, \{4, 6\}, \{4, 7\}, \{4, 9\}, \{4, 10\}, \{4, 11\}, \{5, 6\},$   
 $\{5, 9\}, \{5, 10\}, \{5, 11\}, \{6, 9\}, \{6, 10\}, \{7, 8\}, \{7, 9\}, \{8, 9\}, \{9, 10\}, \{9, 11\},$   
 $\{\{1, 2\}, \{1, 6\}, \{1, 8\}, \{1, 10\}, \{2, 3\}, \{2, 5\}, \{2, 8\}, \{2, 9\}, \{2, 10\}, \{3, 4\}, \{3, 7\},$   
 $\{3, 8\}, \{3, 9\}, \{3, 10\}, \{3, 11\}, \{4, 5\}, \{4, 6\}, \{4, 7\}, \{4, 8\}, \{4, 11\}, \{5, 6\}, \{5, 8\},$   
 $\{5, 9\}, \{5, 11\}, \{6, 8\}, \{6, 10\}, \{6, 11\}, \{7, 8\}, \{9, 10\}, \{9, 11\}, \{10, 11\}, \{\{1, 2\},$   
 $\{1, 3\}, \{1, 4\}, \{1, 5\}, \{1, 8\}, \{1, 9\}, \{1, 10\}, \{2, 4\}, \{2, 8\}, \{2, 9\}, \{2, 10\}, \{3, 4\},$   
 $\{3, 5\}, \{3, 6\}, \{3, 8\}, \{3, 11\}, \{4, 6\}, \{4, 8\}, \{4, 9\}, \{4, 10\}, \{4, 11\}, \{5, 6\}, \{5, 7\},$   
 $\{5, 8\}, \{5, 9\}, \{6, 7\}, \{6, 8\}, \{6, 9\}, \{6, 11\}, \{7, 8\}, \{7, 9\}, \{8, 9\}, \{8, 11\}, \{9, 10\},$   
 $\{\{1, 2\}, \{1, 4\}, \{1, 5\}, \{1, 6\}, \{1, 7\}, \{1, 8\}, \{1, 9\}, \{1, 10\}, \{1, 11\}, \{2, 4\}, \{2, 6\},$   
 $\{2, 11\}, \{3, 4\}, \{3, 5\}, \{3, 8\}, \{3, 9\}, \{3, 10\}, \{4, 5\}, \{4, 6\}, \{4, 7\}, \{4, 8\}, \{4, 9\},$   
 $\{4, 11\}, \{5, 6\}, \{5, 7\}, \{5, 8\}, \{5, 9\}, \{5, 10\}, \{5, 11\}, \{6, 11\}, \{7, 8\}, \{8, 10\},$   
 $\{9, 10\}, \{9, 11\}, \{\{1, 2\}, \{1, 3\}, \{1, 6\}, \{1, 7\}, \{1, 8\}, \{2, 3\}, \{2, 6\}, \{2, 8\},$   
 $\{2, 11\}, \{3, 6\}, \{3, 7\}, \{3, 11\}, \{4, 5\}, \{4, 6\}, \{4, 7\}, \{4, 8\}, \{4, 10\}, \{4, 11\}, \{5, 6\},$   
 $\{5, 7\}, \{5, 9\}, \{5, 10\}, \{6, 7\}, \{6, 8\}, \{6, 9\}, \{6, 10\}, \{6, 11\}, \{7, 8\}, \{7, 9\}, \{7, 11\},$   
 $\{8, 9\}, \{8, 10\}, \{8, 11\}, \{9, 10\}, \{\{1, 2\}, \{1, 3\}, \{1, 8\}, \{1, 10\}, \{2, 3\}, \{2, 4\},$   
 $\{2, 5\}, \{2, 6\}, \{2, 7\}, \{2, 8\}, \{2, 9\}, \{2, 10\}, \{2, 11\}, \{3, 4\}, \{3, 7\}, \{3, 8\}, \{3, 9\},$   
 $\{3, 10\}, \{4, 7\}, \{4, 8\}, \{5, 6\}, \{5, 7\}, \{5, 8\}, \{5, 9\}, \{6, 8\}, \{6, 9\}, \{6, 11\}, \{7, 8\},$   
 $\{7, 9\}, \{8, 10\}, \{8, 11\}, \{9, 10\}, \{9, 11\}, \{10, 11\}, \{\{1, 2\}, \{1, 3\}, \{1, 4\}, \{1, 5\},$   
 $\{1, 6\}, \{1, 8\}, \{1, 9\}, \{1, 10\}, \{1, 11\}, \{2, 3\}, \{2, 4\}, \{2, 5\}, \{2, 6\}, \{2, 7\}, \{2, 8\},$   
 $\{2, 9\}, \{2, 10\}, \{2, 11\}, \{3, 7\}, \{3, 8\}, \{3, 9\}, \{3, 11\}, \{4, 5\}, \{4, 6\}, \{4, 7\}, \{4, 10\},$   
 $\{4, 11\}, \{5, 6\}, \{6, 10\}, \{7, 9\}, \{7, 10\}, \{7, 11\}, \{8, 9\}, \{9, 10\}, \{\{1, 2\}, \{1, 4\},$   
 $\{1, 6\}, \{1, 7\}, \{1, 8\}, \{1, 9\}, \{1, 10\}, \{1, 11\}, \{2, 3\}, \{2, 4\}, \{2, 5\}, \{2, 6\}, \{2, 9\},$   
 $\{2, 11\}, \{3, 4\}, \{3, 5\}, \{3, 8\}, \{3, 11\}, \{4, 5\}, \{4, 6\}, \{4, 7\}, \{4, 8\}, \{4, 9\}, \{4, 10\},$   
 $\{4, 11\}, \{5, 6\}, \{5, 7\}, \{5, 8\}, \{6, 7\}, \{7, 8\}, \{8, 10\}, \{8, 11\}, \{9, 11\}, \{10, 11\},$   
 $\{\{1, 2\}, \{1, 4\}, \{1, 5\}, \{1, 6\}, \{1, 8\}, \{1, 9\}, \{1, 10\}, \{1, 11\}, \{2, 3\}, \{2, 5\}, \{2, 6\},$   
 $\{2, 7\}, \{2, 8\}, \{2, 9\}, \{2, 10\}, \{3, 5\}, \{3, 9\}, \{3, 10\}, \{4, 5\}, \{4, 9\}, \{4, 10\}, \{4, 11\},$   
 $\{5, 6\}, \{5, 7\}, \{5, 9\}, \{5, 10\}, \{6, 7\}, \{6, 8\}, \{7, 8\}, \{7, 9\}, \{8, 9\}, \{9, 10\}, \{9, 11\},$   
 $\{10, 11\}, \{\{1, 2\}, \{1, 4\}, \{1, 6\}, \{1, 7\}, \{1, 10\}, \{1, 11\}, \{2, 5\}, \{2, 6\}, \{2, 7\},$

{2,10},{2,11},{3,4},{3,5},{3,6},{3,7},{3,8},{3,9},{4,6},{4,7},{4,8},  
{4,9},{4,11},{5,6},{5,7},{5,9},{5,11},{6,7},{6,8},{6,9},{6,10},{6,11},  
{7,10},{8,9},{9,11}},{1,2},{1,3},{1,4},{1,5},{1,6},{1,7},{1,8},{2,4},  
{2,5},{2,7},{2,8},{3,4},{3,5},{3,6},{3,7},{3,8},{3,10},{4,5},{4,6},  
{4,7},{4,9},{4,10},{4,11},{5,8},{6,7},{6,9},{6,10},{6,11},{7,8},  
{7,10},{7,11},{9,10},{9,11},{10,11}},{1,2},{1,3},{1,4},{1,6},{1,9},  
{2,3},{2,4},{2,6},{2,11},{3,4},{3,5},{3,7},{3,8},{3,9},{3,11},{4,5},  
{4,6},{5,6},{5,7},{5,8},{5,9},{5,10},{5,11},{6,9},{6,11},{7,8},{7,9},  
{7,10},{7,11},{8,9},{8,10},{9,10},{9,11}},{1,2},{1,3},{1,4},{1,5},  
{1,6},{1,7},{1,10},{1,11},{2,3},{2,4},{2,5},{2,7},{2,8},{2,9},{3,4},  
{3,5},{3,6},{3,7},{3,8},{3,9},{3,10},{3,11},{4,5},{4,6},{4,8},{4,9},  
{4,10},{5,9},{5,10},{6,7},{6,8},{6,11},{7,8},{7,11}},{1,2},{1,3},  
{1,4},{1,6},{1,7},{1,9},{2,3},{2,4},{2,5},{2,6},{2,7},{2,9},{3,4},  
{3,7},{4,5},{4,7},{4,8},{4,9},{4,10},{4,11},{5,7},{5,8},{5,9},{5,10},  
{5,11},{6,7},{6,9},{7,9},{7,10},{8,9},{8,10},{8,11},{9,10},{10,11}},  
{1,2},{1,3},{1,4},{1,5},{1,6},{1,8},{1,10},{2,3},{2,6},{2,7},{2,9},  
{2,10},{3,4},{3,7},{3,10},{4,5},{4,7},{4,10},{4,11},{5,7},{5,8},  
{5,11},{6,7},{6,8},{6,9},{6,10},{7,8},{7,9},{7,11},{8,10},{8,11},  
{10,11}},{1,2},{1,6},{1,7},{1,9},{1,10},{2,5},{2,6},{2,7},{2,10},  
{3,4},{3,5},{3,6},{3,9},{4,5},{4,6},{4,7},{4,8},{4,9},{4,11},{5,6},  
{5,7},{5,9},{5,10},{5,11},{6,7},{6,8},{6,9},{6,10},{6,11},{7,8},{7,9},  
{7,11},{8,9},{9,10}},{1,2},{1,3},{1,5},{1,6},{1,7},{1,10},{2,3},  
{2,4},{2,5},{2,6},{2,9},{2,10},{3,7},{3,8},{3,9},{3,10},{4,5},{4,7},  
{4,9},{4,10},{4,11},{5,6},{5,7},{5,10},{6,10},{7,8},{7,9},{7,11},  
{8,9},{8,10},{8,11},{9,11},{10,11}},{1,2},{1,3},{1,4},{1,5},{1,6},  
{1,7},{1,8},{1,10},{1,11},{2,3},{2,4},{2,10},{2,11},{3,4},{3,5},  
{3,10},{4,5},{4,6},{4,7},{4,8},{4,9},{4,10},{4,11},{5,7},{5,8},{5,9},  
{5,10},{6,7},{6,8},{7,8},{7,9},{8,9},{8,10},{10,11}},{1,2},{1,3},  
{1,4},{1,6},{1,7},{2,3},{2,4},{2,6},{2,7},{2,9},{2,10},{3,4},{3,5},  
{3,6},{3,7},{3,8},{3,9},{3,10},{3,11},{4,5},{4,6},{4,9},{4,10},{4,11},  
{5,6},{5,8},{5,9},{5,11},{6,7},{6,8},{6,9},{6,11},{8,11},{9,10}},  
{1,2},{1,3},{1,4},{1,9},{1,10},{2,3},{2,4},{2,10},{2,11},{3,4},{3,5},  
{3,6},{3,7},{3,8},{3,9},{3,11},{4,5},{4,7},{4,8},{4,9},{4,10},{4,11},  
{5,6},{5,8},{5,9},{5,10},{5,11},{6,7},{6,8},{6,11},{7,8},{7,11},  
{9,10},{10,11}},{1,2},{1,3},{1,4},{1,5},{1,6},{1,7},{1,8},{1,9},  
{1,10},{2,3},{2,5},{2,6},{2,8},{3,6},{3,7},{3,8},{3,9},{3,10},{3,11},  
{4,7},{4,9},{4,10},{5,6},{5,7},{5,8},{5,9},{6,9},{7,8},{7,9},{7,10},  
{7,11},{9,10},{9,11},{10,11}},{1,2},{1,6},{1,7},{1,9},{1,10},{2,3},  
{2,4},{2,5},{2,6},{2,7},{2,8},{2,9},{2,10},{2,11},{3,6},{3,9},{3,11},  
{4,5},{4,7},{4,8},{5,7},{5,8},{5,9},{5,11},{6,7},{6,9},{6,11},{7,8},  
{7,9},{7,10},{7,11},{8,9},{9,10},{9,11}},{1,2},{1,3},{1,4},{1,6},  
{1,7},{1,9},{1,10},{2,3},{2,4},{2,5},{2,6},{2,7},{2,8},{2,11},{3,4},  
{3,5},{3,6},{3,7},{3,8},{3,9},{3,10},{3,11},{4,9},{4,10},{4,11},{5,6},  
{5,7},{6,7},{7,8},{7,9},{8,9},{8,11},{9,10},{9,11}},{1,2},{1,4},  
{1,6},{1,9},{2,3},{2,4},{2,6},{2,7},{2,8},{2,9},{2,11},{3,4},{3,6},  
{3,8},{4,5},{4,6},{4,7},{4,8},{4,9},{4,10},{4,11},{5,7},{5,8},{5,10},  
{6,7},{6,8},{6,9},{6,10},{7,8},{7,9},{7,10},{7,11},{8,10},{9,11}},  
{1,2},{1,4},{1,5},{1,6},{1,7},{1,8},{1,9},{1,11},{2,3},{2,4},{2,5},  
{2,6},{2,10},{3,4},{3,5},{3,10},{4,5},{4,6},{4,7},{4,8},{4,9},{4,10},  
{4,11},{5,7},{5,9},{5,10},{5,11},{6,8},{6,10},{7,8},{7,9},{7,10},

$\{8,10\}, \{9,11\}, \{\{1,2\}, \{1,3\}, \{1,5\}, \{1,6\}, \{1,7\}, \{1,8\}, \{2,3\}, \{2,4\}, \{2,5\},$   
 $\{2,6\}, \{2,8\}, \{2,9\}, \{2,10\}, \{2,11\}, \{3,4\}, \{3,6\}, \{3,7\}, \{3,8\}, \{3,9\}, \{3,10\},$   
 $\{4,8\}, \{4,9\}, \{5,6\}, \{5,7\}, \{5,10\}, \{6,7\}, \{6,8\}, \{6,9\}, \{6,10\}, \{6,11\}, \{7,10\},$   
 $\{8,9\}, \{8,11\}, \{9,11\}, \{\{1,2\}, \{1,4\}, \{1,5\}, \{1,6\}, \{1,7\}, \{1,8\}, \{1,10\},$   
 $\{2,3\}, \{2,4\}, \{2,5\}, \{2,6\}, \{2,7\}, \{2,8\}, \{2,9\}, \{2,10\}, \{3,4\}, \{3,6\}, \{3,10\},$   
 $\{4,5\}, \{4,6\}, \{4,8\}, \{4,9\}, \{4,10\}, \{4,11\}, \{5,6\}, \{5,8\}, \{5,9\}, \{5,11\}, \{6,7\},$   
 $\{6,10\}, \{7,10\}, \{8,9\}, \{8,11\}, \{9,11\}, \{\{1,2\}, \{1,3\}, \{1,4\}, \{1,5\}, \{1,6\},$   
 $\{1,7\}, \{1,8\}, \{1,9\}, \{1,10\}, \{2,4\}, \{2,5\}, \{2,8\}, \{2,9\}, \{2,10\}, \{2,11\}, \{3,4\},$   
 $\{3,6\}, \{3,7\}, \{3,8\}, \{3,9\}, \{4,5\}, \{4,8\}, \{4,9\}, \{4,10\}, \{4,11\}, \{5,8\}, \{6,7\},$   
 $\{6,8\}, \{7,8\}, \{7,9\}, \{8,9\}, \{9,10\}, \{9,11\}, \{10,11\}, \{\{1,2\}, \{1,5\}, \{1,7\},$   
 $\{1,8\}, \{1,9\}, \{1,10\}, \{1,11\}, \{2,3\}, \{2,4\}, \{2,5\}, \{2,6\}, \{2,10\}, \{3,4\}, \{3,5\},$   
 $\{3,6\}, \{3,8\}, \{3,10\}, \{4,6\}, \{4,10\}, \{5,6\}, \{5,7\}, \{5,8\}, \{5,11\}, \{6,10\},$   
 $\{6,11\}, \{7,8\}, \{7,9\}, \{7,11\}, \{8,9\}, \{8,10\}, \{8,11\}, \{9,11\}, \{10,11\}, \{\{1,2\},$   
 $\{1,4\}, \{1,5\}, \{1,8\}, \{1,10\}, \{2,3\}, \{2,4\}, \{2,5\}, \{2,6\}, \{2,7\}, \{2,8\}, \{2,9\},$   
 $\{2,10\}, \{2,11\}, \{3,4\}, \{3,7\}, \{3,9\}, \{3,10\}, \{3,11\}, \{4,6\}, \{4,7\}, \{4,8\},$   
 $\{4,10\}, \{5,8\}, \{5,10\}, \{6,7\}, \{6,8\}, \{7,8\}, \{7,9\}, \{8,9\}, \{8,10\}, \{9,10\},$   
 $\{9,11\}, \{10,11\}, \{\{1,2\}, \{1,3\}, \{1,4\}, \{1,5\}, \{1,6\}, \{1,7\}, \{1,8\}, \{1,9\},$   
 $\{1,11\}, \{2,3\}, \{2,4\}, \{2,5\}, \{2,7\}, \{2,8\}, \{2,9\}, \{2,10\}, \{2,11\}, \{3,4\}, \{3,6\},$   
 $\{3,8\}, \{3,9\}, \{4,6\}, \{4,7\}, \{5,6\}, \{5,7\}, \{5,8\}, \{6,7\}, \{6,8\}, \{8,9\}, \{8,10\},$   
 $\{8,11\}, \{9,10\}, \{9,11\}, \{10,11\}, \{\{1,2\}, \{1,5\}, \{1,9\}, \{1,11\}, \{2,3\}, \{2,4\},$   
 $\{2,5\}, \{2,6\}, \{2,7\}, \{2,8\}, \{2,9\}, \{2,10\}, \{2,11\}, \{3,4\}, \{3,6\}, \{3,7\}, \{3,8\},$   
 $\{3,9\}, \{4,6\}, \{4,8\}, \{4,10\}, \{5,6\}, \{5,9\}, \{5,10\}, \{5,11\}, \{6,9\}, \{6,10\},$   
 $\{6,11\}, \{7,8\}, \{7,9\}, \{7,10\}, \{8,10\}, \{9,10\}, \{9,11\}, \{\{1,2\}, \{1,3\}, \{1,4\},$   
 $\{1,5\}, \{1,7\}, \{1,8\}, \{1,9\}, \{1,10\}, \{2,3\}, \{2,4\}, \{2,5\}, \{2,6\}, \{2,9\}, \{2,10\},$   
 $\{3,4\}, \{3,5\}, \{3,7\}, \{3,8\}, \{3,11\}, \{4,6\}, \{4,8\}, \{4,9\}, \{4,10\}, \{5,7\}, \{5,8\},$   
 $\{5,9\}, \{5,11\}, \{6,9\}, \{6,10\}, \{7,8\}, \{7,11\}, \{8,9\}, \{8,11\}, \{9,10\}, \{\{1,2\},$   
 $\{1,7\}, \{1,8\}, \{1,9\}, \{2,4\}, \{2,5\}, \{2,6\}, \{2,7\}, \{2,8\}, \{2,9\}, \{3,4\}, \{3,5\},$   
 $\{3,6\}, \{3,8\}, \{3,10\}, \{4,5\}, \{4,6\}, \{4,8\}, \{5,6\}, \{5,7\}, \{5,10\}, \{6,9\}, \{6,10\},$   
 $\{7,8\}, \{7,9\}, \{7,10\}, \{7,11\}, \{8,9\}, \{8,10\}, \{8,11\}, \{9,10\}, \{9,11\}, \{10,11\},$   
 $\{\{1,2\}, \{1,3\}, \{1,4\}, \{1,5\}, \{1,6\}, \{1,7\}, \{1,8\}, \{1,9\}, \{1,10\}, \{1,11\}, \{2,3\},$   
 $\{2,4\}, \{2,5\}, \{2,6\}, \{2,7\}, \{2,8\}, \{2,11\}, \{3,4\}, \{3,5\}, \{3,10\}, \{4,9\}, \{4,10\},$   
 $\{4,11\}, \{5,8\}, \{5,10\}, \{6,7\}, \{6,9\}, \{6,11\}, \{7,8\}, \{7,9\}, \{7,10\}, \{8,10\},$   
 $\{9,10\}, \{9,11\}, \{\{1,2\}, \{1,4\}, \{1,5\}, \{1,6\}, \{1,7\}, \{1,8\}, \{1,9\}, \{1,10\},$   
 $\{1,11\}, \{2,7\}, \{2,8\}, \{2,10\}, \{3,4\}, \{3,5\}, \{3,6\}, \{3,8\}, \{3,11\}, \{4,5\}, \{4,6\},$   
 $\{4,8\}, \{5,6\}, \{5,11\}, \{6,7\}, \{6,8\}, \{6,9\}, \{6,10\}, \{6,11\}, \{7,8\}, \{7,10\}, \{8,9\},$   
 $\{8,10\}, \{8,11\}, \{9,10\}, \{9,11\}, \{\{1,2\}, \{1,3\}, \{1,5\}, \{1,6\}, \{1,7\}, \{1,10\},$   
 $\{1,11\}, \{2,3\}, \{2,5\}, \{2,6\}, \{2,11\}, \{3,4\}, \{3,5\}, \{3,6\}, \{3,7\}, \{3,8\}, \{3,9\},$   
 $\{3,10\}, \{3,11\}, \{4,5\}, \{4,6\}, \{4,9\}, \{5,6\}, \{5,7\}, \{5,8\}, \{5,9\}, \{5,10\}, \{6,7\},$   
 $\{6,9\}, \{6,11\}, \{7,8\}, \{7,9\}, \{7,10\}, \{8,9\}, \{\{1,2\}, \{1,3\}, \{1,6\}, \{1,7\}, \{1,8\},$   
 $\{1,9\}, \{2,3\}, \{2,7\}, \{2,8\}, \{2,10\}, \{3,4\}, \{3,5\}, \{3,6\}, \{3,7\}, \{3,10\}, \{3,11\},$   
 $\{4,5\}, \{4,7\}, \{4,10\}, \{4,11\}, \{5,6\}, \{5,7\}, \{5,8\}, \{5,10\}, \{5,11\}, \{6,7\}, \{6,8\},$   
 $\{6,9\}, \{7,8\}, \{7,9\}, \{7,10\}, \{7,11\}, \{8,9\}, \{8,10\}, \{\{1,2\}, \{1,3\}, \{1,7\},$   
 $\{1,11\}, \{2,3\}, \{2,5\}, \{2,6\}, \{2,7\}, \{2,8\}, \{2,9\}, \{2,10\}, \{2,11\}, \{3,4\}, \{3,5\},$   
 $\{3,6\}, \{3,7\}, \{3,8\}, \{3,10\}, \{3,11\}, \{4,5\}, \{4,8\}, \{4,9\}, \{4,10\}, \{5,6\}, \{5,8\},$   
 $\{5,9\}, \{6,7\}, \{6,8\}, \{6,11\}, \{7,8\}, \{7,11\}, \{8,9\}, \{8,10\}, \{9,10\}, \{\{1,2\},$   
 $\{1,3\}, \{1,4\}, \{1,5\}, \{1,6\}, \{1,7\}, \{1,8\}, \{1,9\}, \{1,10\}, \{1,11\}, \{2,3\}, \{2,5\},$   
 $\{2,11\}, \{3,4\}, \{3,5\}, \{3,6\}, \{3,10\}, \{3,11\}, \{4,5\}, \{4,6\}, \{4,7\}, \{4,8\}, \{4,10\},$   
 $\{5,6\}, \{5,8\}, \{5,11\}, \{7,8\}, \{7,10\}, \{8,9\}, \{8,10\}, \{8,11\}, \{9,10\}, \{9,11\},$   
 $\{10,11\}, \{\{1,2\}, \{1,3\}, \{1,4\}, \{1,7\}, \{1,10\}, \{1,11\}, \{2,3\}, \{2,7\}, \{2,8\},$   
 $\{2,9\}, \{2,10\}, \{3,4\}, \{3,5\}, \{3,6\}, \{3,7\}, \{3,8\}, \{4,5\}, \{4,7\}, \{4,11\}, \{5,6\},$

{5,7},{5,10},{5,11},{6,7},{6,8},{6,9},{6,10},{7,8},{7,9},{7,10},  
{7,11},{8,9},{9,10},{10,11}},{{1,2},{1,3},{1,6},{1,7},{1,8},{1,9},  
{1,10},{2,4},{2,5},{2,6},{2,8},{2,9},{2,10},{3,4},{3,6},{3,7},{3,8},  
{3,10},{4,6},{4,8},{4,10},{5,6},{5,8},{5,9},{5,11},{6,7},{6,8},{6,9},  
{6,10},{6,11},{7,10},{8,9},{8,11},{9,11}},{{1,2},{1,3},{1,5},{1,6},  
{1,7},{1,8},{1,9},{1,10},{2,3},{2,4},{2,5},{2,7},{3,4},{3,5},{3,6},  
{3,7},{3,8},{3,10},{3,11},{4,5},{4,7},{5,7},{5,8},{5,9},{5,11},{6,7},  
{6,8},{6,10},{7,8},{7,9},{7,10},{7,11},{8,9},{8,11}},{{1,2},{1,4},  
{1,7},{1,8},{1,10},{1,11},{2,5},{2,7},{2,8},{2,9},{2,10},{3,4},{3,5},  
{3,9},{4,5},{4,6},{4,7},{4,9},{4,10},{4,11},{5,6},{5,8},{5,9},{5,10},  
{6,8},{6,10},{6,11},{7,8},{7,9},{8,9},{8,11},{10,11}},{{1,2},{1,3},  
{1,5},{1,7},{1,8},{1,9},{1,10},{1,11},{2,9},{2,10},{2,11},{3,4},{3,5},  
{3,9},{3,10},{4,5},{4,6},{4,9},{4,10},{5,6},{5,7},{5,9},{5,10},{6,9},  
{6,10},{7,8},{7,9},{7,10},{8,9},{8,10},{8,11},{9,10},{9,11},{10,11}},  
{{1,2},{1,6},{1,7},{1,9},{2,3},{2,4},{2,6},{2,7},{2,8},{2,9},{2,10},  
{3,4},{3,5},{3,6},{3,8},{3,10},{4,5},{4,7},{4,8},{4,10},{5,6},{5,7},  
{5,8},{6,7},{6,8},{6,9},{6,11},{7,8},{7,9},{7,11},{8,9},{8,10},{8,11},  
{9,11}},{{1,2},{1,3},{1,4},{1,8},{1,9},{1,10},{2,3},{2,4},{2,5},{2,6},  
{2,7},{2,9},{2,10},{2,11},{3,4},{3,5},{3,6},{3,7},{3,8},{3,9},{3,10},  
{3,11},{4,6},{4,8},{5,6},{5,7},{5,8},{5,9},{5,11},{6,7},{6,8},{8,9},  
{9,10},{9,11}},{{1,2},{1,5},{1,8},{1,11},{2,3},{2,4},{2,5},{2,6},  
{2,7},{2,8},{2,9},{2,10},{2,11},{3,4},{3,5},{3,6},{3,8},{3,9},{3,11},  
{4,5},{4,6},{5,6},{5,7},{5,8},{5,9},{5,10},{5,11},{6,7},{6,8},{6,10},  
{7,10},{8,10},{8,11},{9,11}},{{1,2},{1,4},{1,8},{1,9},{1,10},{1,11},  
{2,3},{2,4},{2,5},{2,7},{2,10},{2,11},{3,4},{3,5},{3,7},{3,10},{4,5},  
{4,7},{4,8},{4,10},{5,6},{5,7},{5,8},{5,9},{5,10},{5,11},{6,8},{6,9},  
{6,10},{8,9},{8,10},{9,10},{9,11},{10,11}},{{1,2},{1,3},{1,4},{1,5},  
{1,6},{1,7},{1,8},{1,9},{1,11},{2,3},{2,4},{2,5},{2,6},{2,7},{2,8},  
{2,10},{3,4},{3,5},{3,7},{3,9},{3,11},{4,5},{4,7},{4,8},{4,10},{4,11},  
{5,9},{5,11},{6,7},{6,8},{6,10},{7,10},{8,10},{9,11}},{{1,2},{1,6},  
{1,7},{1,11},{2,3},{2,4},{2,5},{2,6},{2,7},{2,8},{2,10},{2,11},{3,4},  
{3,7},{3,10},{4,7},{4,8},{4,10},{5,6},{5,8},{5,10},{6,7},{6,8},{6,9},  
{6,10},{6,11},{7,8},{7,9},{7,10},{7,11},{8,9},{8,10},{8,11},{9,10}},  
{{1,2},{1,3},{1,4},{1,5},{1,7},{1,8},{1,9},{1,10},{2,3},{2,4},{2,7},  
{2,8},{2,9},{2,10},{2,11},{3,4},{3,5},{3,6},{3,7},{3,8},{3,9},{4,9},  
{4,10},{4,11},{5,6},{5,8},{5,9},{6,8},{6,9},{7,8},{8,9},{9,10},{9,11},  
{10,11}},{{1,2},{1,3},{1,4},{1,9},{1,10},{2,3},{2,8},{2,9},{2,10},  
{2,11},{3,4},{3,5},{3,6},{3,8},{3,10},{3,11},{4,5},{4,7},{4,9},{4,10},  
{5,6},{5,7},{5,9},{6,7},{6,8},{6,9},{6,10},{7,9},{7,10},{8,9},{8,10},  
{8,11},{10,11}},{{1,2},{1,3},{1,4},{1,5},{1,6},{1,7},{1,8},{1,9},  
{1,10},{1,11},{2,3},{2,4},{2,5},{3,4},{3,5},{3,8},{3,11},{4,5},{4,7},  
{4,8},{4,9},{4,10},{5,7},{5,11},{6,7},{6,8},{6,9},{6,11},{7,9},{7,10},  
{7,11},{8,9},{8,11},{9,10}},{{1,2},{1,3},{1,4},{1,5},{1,6},{1,7},  
{1,8},{1,9},{1,10},{1,11},{2,3},{2,6},{2,9},{2,10},{3,4},{3,5},{3,6},  
{3,7},{3,8},{3,9},{3,11},{4,5},{4,11},{5,6},{5,7},{5,8},{5,11},{6,8},  
{6,9},{6,10},{6,11},{7,8},{8,9},{9,10}},{{1,2},{1,3},{1,4},{1,5},  
{1,6},{1,8},{1,10},{2,3},{2,7},{2,8},{2,9},{2,10},{2,11},{3,4},{3,5},  
{3,6},{3,7},{3,8},{3,9},{3,10},{4,5},{4,6},{5,6},{5,8},{6,8},{6,9},  
{6,10},{7,9},{7,10},{7,11},{8,9},{9,10},{9,11},{10,11}},{{1,2},{1,3},  
{1,4},{1,5},{1,6},{1,7},{1,8},{1,9},{1,10},{2,3},{2,6},{2,10},{3,4},

{3,5},{3,6},{3,8},{3,9},{3,10},{3,11},{4,5},{4,7},{4,9},{4,10},{4,11},  
{5,6},{5,7},{5,8},{5,10},{5,11},{6,8},{6,10},{7,9},{7,11},{9,11}},  
{{1,2},{1,4},{1,8},{1,10},{1,11},{2,3},{2,4},{2,6},{2,8},{2,10},  
{2,11},{3,4},{3,5},{3,6},{3,7},{3,8},{4,5},{4,8},{4,9},{4,10},{4,11},  
{5,6},{5,7},{5,9},{6,7},{6,9},{6,10},{7,8},{7,9},{8,9},{8,10},{8,11},  
{9,10}},{{1,2},{1,5},{1,9},{1,10},{1,11},{2,3},{2,4},{2,5},{2,7},  
{2,9},{2,11},{3,4},{3,5},{3,6},{3,10},{4,6},{4,7},{4,10},{5,6},{5,10},  
{5,11},{6,7},{6,8},{6,9},{6,10},{6,11},{7,8},{7,9},{7,10},{8,9},  
{8,10},{9,10},{9,11}},{{1,2},{1,3},{1,4},{1,5},{1,6},{1,7},{1,8},  
{1,9},{1,10},{1,11},{2,3},{2,10},{2,11},{3,4},{3,5},{3,6},{3,7},{3,9},  
{3,10},{3,11},{4,5},{4,6},{4,8},{4,10},{5,6},{6,7},{6,8},{7,8},{7,9},  
{7,11},{8,10},{8,11},{9,11},{10,11}},{{1,2},{1,3},{1,4},{1,6},{1,7},  
{1,8},{1,9},{1,10},{1,11},{2,5},{2,6},{2,7},{2,11},{3,4},{3,6},{3,7},  
{3,9},{3,10},{4,7},{4,10},{5,6},{5,7},{5,11},{6,7},{6,8},{6,9},{6,10},  
{6,11},{7,9},{7,10},{7,11},{8,9},{8,11},{9,11}},{{1,2},{1,3},{1,4},  
{1,6},{1,9},{1,10},{1,11},{2,3},{2,4},{2,7},{2,8},{2,9},{3,8},{3,9},  
{3,10},{4,5},{4,6},{4,7},{4,8},{4,9},{4,10},{4,11},{5,7},{5,8},{5,9},  
{6,9},{6,10},{6,11},{7,8},{7,9},{8,9},{8,10},{9,10},{9,11}},{{1,2},  
{1,3},{1,6},{1,7},{1,8},{2,3},{2,5},{2,6},{2,7},{2,9},{2,10},{2,11},  
{3,4},{3,5},{3,7},{3,8},{4,5},{4,7},{4,8},{5,7},{5,8},{5,11},{6,7},  
{6,8},{6,10},{7,8},{7,9},{7,10},{7,11},{8,10},{8,11},{9,10},{9,11},  
{10,11}},{{1,2},{1,3},{1,4},{1,5},{1,6},{1,7},{1,8},{1,9},{2,3},{2,4},  
{2,5},{2,6},{2,8},{2,10},{2,11},{3,4},{3,5},{3,6},{3,7},{3,11},{4,8},  
{4,10},{4,11},{5,6},{5,7},{5,9},{6,7},{6,8},{6,9},{6,11},{7,9},{8,10},  
{8,11},{10,11}},{{1,2},{1,3},{1,4},{1,5},{1,6},{1,7},{1,8},{1,9},  
{1,10},{1,11},{2,3},{2,5},{2,6},{2,7},{2,8},{2,9},{2,10},{2,11},{3,9},  
{3,10},{4,5},{4,6},{4,11},{5,6},{5,8},{5,9},{5,11},{6,7},{6,9},{6,11},  
{7,9},{7,10},{8,9},{9,10}},{{1,2},{1,3},{1,4},{1,5},{1,6},{1,7},{2,3},  
{2,5},{2,6},{2,9},{3,4},{3,6},{3,9},{4,5},{4,7},{4,8},{4,9},{4,10},  
{4,11},{5,7},{5,8},{5,9},{5,10},{5,11},{6,7},{6,8},{6,9},{7,8},{7,10},  
{8,9},{8,10},{8,11},{9,11}},{{1,2},{1,3},{1,4},{1,5},{1,6},{1,7},  
{1,8},{1,9},{1,10},{1,11},{2,3},{2,4},{2,5},{2,6},{2,7},{2,11},{3,5},  
{3,6},{3,8},{3,11},{4,7},{4,11},{5,11},{6,7},{6,8},{6,9},{6,10},{7,8},  
{7,10},{7,11},{8,9},{8,10},{8,11},{9,10}},{{1,2},{1,3},{1,4},{1,5},  
{1,6},{1,7},{1,8},{1,9},{1,11},{2,5},{2,6},{2,8},{3,4},{3,5},{3,6},  
{3,9},{3,10},{4,5},{4,6},{4,8},{4,11},{5,6},{5,7},{5,8},{5,10},{5,11},  
{6,7},{6,8},{6,9},{6,10},{7,9},{7,10},{8,11},{9,10}},{{1,2},{1,4},  
{1,5},{1,6},{1,7},{1,8},{1,9},{1,10},{1,11},{2,3},{2,4},{2,5},{2,6},  
{2,7},{2,11},{3,5},{3,6},{3,7},{3,11},{4,5},{4,6},{4,9},{4,10},{5,6},  
{5,7},{5,8},{5,10},{6,8},{6,9},{6,11},{7,11},{8,9},{8,10},{9,10}},  
{{1,2},{1,5},{1,6},{1,7},{1,8},{1,10},{1,11},{2,3},{2,5},{2,8},{2,10},  
{2,11},{3,4},{3,5},{3,7},{3,8},{3,9},{3,11},{4,5},{4,6},{4,7},{4,9},  
{5,6},{5,7},{6,7},{6,9},{6,11},{7,8},{8,10},{8,11},{9,11},{10,11}},  
{{1,2},{1,3},{1,4},{1,5},{1,6},{1,7},{1,8},{1,9},{1,10},{1,11},{2,4},  
{2,6},{2,7},{2,10},{3,4},{3,8},{3,9},{3,10},{4,5},{4,7},{4,8},{4,9},  
{4,10},{4,11},{5,6},{5,9},{5,10},{5,11},{6,7},{6,10},{6,11},{7,11},  
{8,10},{9,10}},{{1,2},{1,6},{1,8},{1,9},{1,11},{2,3},{2,4},{2,6},  
{2,7},{2,8},{2,9},{2,10},{2,11},{3,5},{3,6},{3,7},{3,10},{4,5},{4,6},  
{4,7},{4,8},{4,9},{4,10},{4,11},{5,6},{5,7},{5,10},{6,7},{6,9},{6,10},  
{6,11},{7,11},{8,9},{8,11}},{{1,2},{1,3},{1,4},{1,7},{2,3},{2,4},



$\{2,5\}, \{2,7\}, \{2,8\}, \{2,9\}, \{2,10\}, \{3,4\}, \{3,7\}, \{3,8\}, \{3,9\}, \{4,5\}, \{4,6\},$   
 $\{4,7\}, \{4,9\}, \{4,11\}, \{5,6\}, \{5,7\}, \{5,9\}, \{6,7\}, \{6,9\}, \{6,11\}, \{7,8\}, \{7,9\},$   
 $\{7,10\}, \{7,11\}, \{8,9\}, \{8,10\}, \{9,10\}, \{9,11\}, \{\{1,2\}, \{1,5\}, \{1,8\}, \{1,9\},$   
 $\{1,11\}, \{2,3\}, \{2,4\}, \{2,6\}, \{2,7\}, \{2,8\}, \{2,9\}, \{2,10\}, \{2,11\}, \{3,4\}, \{3,5\},$   
 $\{3,8\}, \{3,9\}, \{4,5\}, \{4,6\}, \{4,7\}, \{4,9\}, \{4,10\}, \{4,11\}, \{5,8\}, \{5,9\}, \{5,11\},$   
 $\{6,7\}, \{6,9\}, \{6,10\}, \{6,11\}, \{7,9\}, \{8,9\}, \{9,11\}, \{10,11\}, \{\{1,2\}, \{1,3\},$   
 $\{1,4\}, \{1,6\}, \{1,7\}, \{1,8\}, \{1,10\}, \{2,3\}, \{2,5\}, \{2,6\}, \{2,8\}, \{2,9\}, \{2,11\},$   
 $\{3,5\}, \{3,7\}, \{3,8\}, \{3,10\}, \{4,5\}, \{4,6\}, \{4,7\}, \{4,9\}, \{4,11\}, \{5,7\}, \{5,9\},$   
 $\{5,11\}, \{6,11\}, \{7,9\}, \{7,10\}, \{8,9\}, \{8,10\}, \{9,10\}, \{9,11\}, \{\{1,2\}, \{1,3\},$   
 $\{1,4\}, \{1,7\}, \{1,8\}, \{1,9\}, \{2,4\}, \{2,5\}, \{2,7\}, \{2,8\}, \{2,9\}, \{2,10\}, \{3,4\},$   
 $\{3,5\}, \{3,7\}, \{3,8\}, \{4,5\}, \{4,7\}, \{4,9\}, \{5,6\}, \{5,7\}, \{5,8\}, \{5,10\}, \{5,11\},$   
 $\{6,7\}, \{6,8\}, \{6,10\}, \{6,11\}, \{7,8\}, \{7,9\}, \{7,10\}, \{8,10\}, \{8,11\}, \{10,11\},$   
 $\{\{1,2\}, \{1,3\}, \{1,4\}, \{1,6\}, \{1,7\}, \{1,8\}, \{1,9\}, \{1,11\}, \{2,4\}, \{2,6\}, \{2,7\},$   
 $\{3,4\}, \{3,7\}, \{3,9\}, \{3,10\}, \{4,5\}, \{4,6\}, \{4,7\}, \{4,8\}, \{4,9\}, \{4,10\}, \{4,11\},$   
 $\{5,6\}, \{5,8\}, \{5,9\}, \{5,10\}, \{6,7\}, \{6,8\}, \{6,10\}, \{6,11\}, \{7,10\}, \{8,9\},$   
 $\{8,11\}, \{9,10\}, \{\{1,2\}, \{1,3\}, \{1,4\}, \{1,6\}, \{1,7\}, \{1,8\}, \{1,9\}, \{1,11\},$   
 $\{2,4\}, \{2,5\}, \{2,6\}, \{2,9\}, \{2,11\}, \{3,4\}, \{3,5\}, \{3,6\}, \{3,11\}, \{4,5\}, \{4,6\},$   
 $\{4,7\}, \{4,8\}, \{4,9\}, \{4,10\}, \{4,11\}, \{5,6\}, \{5,11\}, \{7,8\}, \{7,9\}, \{8,9\}, \{8,10\},$   
 $\{8,11\}, \{9,10\}, \{9,11\}, \{10,11\}, \{\{1,2\}, \{1,5\}, \{1,6\}, \{1,11\}, \{2,5\}, \{2,6\},$   
 $\{2,8\}, \{2,9\}, \{2,11\}, \{3,4\}, \{3,5\}, \{3,6\}, \{3,7\}, \{3,10\}, \{3,11\}, \{4,6\}, \{4,7\},$   
 $\{4,11\}, \{5,6\}, \{5,8\}, \{5,10\}, \{5,11\}, \{6,7\}, \{6,8\}, \{6,9\}, \{6,11\}, \{7,8\},$   
 $\{7,10\}, \{7,11\}, \{8,9\}, \{8,10\}, \{8,11\}, \{9,11\}, \{10,11\}, \{\{1,2\}, \{1,3\}, \{1,4\},$   
 $\{1,5\}, \{1,6\}, \{1,7\}, \{1,8\}, \{1,9\}, \{1,10\}, \{1,11\}, \{2,3\}, \{2,9\}, \{2,10\}, \{3,4\},$   
 $\{3,8\}, \{3,9\}, \{3,10\}, \{4,5\}, \{4,6\}, \{4,7\}, \{4,8\}, \{4,10\}, \{5,6\}, \{5,7\}, \{5,8\},$   
 $\{5,11\}, \{6,7\}, \{6,11\}, \{7,8\}, \{7,9\}, \{7,10\}, \{7,11\}, \{8,9\}, \{9,10\}, \{\{1,2\},$   
 $\{1,3\}, \{1,4\}, \{1,5\}, \{1,6\}, \{1,7\}, \{1,8\}, \{1,9\}, \{1,10\}, \{1,11\}, \{2,3\}, \{2,5\},$   
 $\{2,10\}, \{2,11\}, \{3,4\}, \{3,5\}, \{3,6\}, \{3,7\}, \{3,11\}, \{4,5\}, \{4,7\}, \{4,8\}, \{4,9\},$   
 $\{4,11\}, \{5,6\}, \{5,7\}, \{5,9\}, \{5,10\}, \{5,11\}, \{6,7\}, \{7,8\}, \{7,9\}, \{8,9\},$   
 $\{10,11\}, \{\{1,2\}, \{1,4\}, \{1,5\}, \{1,6\}, \{1,7\}, \{1,8\}, \{1,11\}, \{2,3\}, \{2,4\},$   
 $\{2,7\}, \{2,8\}, \{2,11\}, \{3,4\}, \{3,6\}, \{3,7\}, \{3,9\}, \{3,10\}, \{4,5\}, \{4,6\}, \{4,8\},$   
 $\{4,9\}, \{5,6\}, \{6,7\}, \{6,9\}, \{6,10\}, \{7,9\}, \{7,10\}, \{7,11\}, \{8,9\}, \{8,11\},$   
 $\{9,10\}, \{9,11\}, \{\{1,2\}, \{1,3\}, \{1,4\}, \{1,5\}, \{1,7\}, \{1,8\}, \{1,10\}, \{1,11\},$   
 $\{2,4\}, \{2,7\}, \{2,10\}, \{2,11\}, \{3,8\}, \{3,9\}, \{3,10\}, \{3,11\}, \{4,5\}, \{4,6\}, \{4,7\},$   
 $\{4,8\}, \{4,9\}, \{4,10\}, \{4,11\}, \{5,7\}, \{5,11\}, \{6,9\}, \{6,10\}, \{6,11\}, \{7,11\},$   
 $\{8,9\}, \{8,11\}, \{9,10\}, \{9,11\}, \{10,11\}, \{\{1,2\}, \{1,3\}, \{1,4\}, \{1,5\}, \{1,6\},$   
 $\{1,7\}, \{1,9\}, \{1,10\}, \{1,11\}, \{2,3\}, \{2,7\}, \{2,11\}, \{3,6\}, \{3,7\}, \{3,10\},$   
 $\{3,11\}, \{4,5\}, \{4,7\}, \{4,8\}, \{4,10\}, \{5,7\}, \{5,8\}, \{5,9\}, \{6,7\}, \{6,8\}, \{6,9\},$   
 $\{6,10\}, \{7,8\}, \{7,9\}, \{7,10\}, \{7,11\}, \{8,9\}, \{8,10\}, \{10,11\}, \{\{1,2\}, \{1,4\},$   
 $\{1,8\}, \{1,9\}, \{2,4\}, \{2,5\}, \{2,7\}, \{2,8\}, \{2,9\}, \{2,10\}, \{3,4\}, \{3,7\}, \{3,8\},$   
 $\{3,10\}, \{4,5\}, \{4,6\}, \{4,7\}, \{4,8\}, \{4,9\}, \{4,10\}, \{4,11\}, \{5,6\}, \{5,8\}, \{5,9\},$   
 $\{5,10\}, \{5,11\}, \{6,8\}, \{6,11\}, \{7,8\}, \{7,10\}, \{8,9\}, \{8,10\}, \{8,11\}, \{9,11\},$   
 $\{\{1,2\}, \{1,3\}, \{1,4\}, \{1,8\}, \{1,10\}, \{2,3\}, \{2,4\}, \{2,7\}, \{2,8\}, \{3,4\}, \{3,7\},$   
 $\{3,9\}, \{3,10\}, \{4,5\}, \{4,6\}, \{4,7\}, \{4,8\}, \{4,9\}, \{4,10\}, \{4,11\}, \{5,6\}, \{5,8\},$   
 $\{5,10\}, \{5,11\}, \{6,7\}, \{6,8\}, \{6,9\}, \{6,11\}, \{7,8\}, \{7,9\}, \{8,10\}, \{9,10\},$   
 $\{9,11\}, \{10,11\}, \{\{1,2\}, \{1,3\}, \{1,6\}, \{1,7\}, \{1,9\}, \{2,4\}, \{2,7\}, \{2,8\},$   
 $\{2,9\}, \{2,10\}, \{2,11\}, \{3,4\}, \{3,5\}, \{3,6\}, \{3,7\}, \{3,8\}, \{3,10\}, \{3,11\}, \{4,5\},$   
 $\{4,6\}, \{4,8\}, \{4,9\}, \{4,10\}, \{5,6\}, \{5,10\}, \{6,9\}, \{6,10\}, \{7,8\}, \{7,11\},$   
 $\{8,11\}, \{9,10\}, \{10,11\}, \{\{1,2\}, \{1,3\}, \{1,5\}, \{1,10\}, \{2,3\}, \{2,5\}, \{2,8\},$   
 $\{2,10\}, \{3,4\}, \{3,5\}, \{3,7\}, \{3,8\}, \{3,9\}, \{3,10\}, \{3,11\}, \{4,5\}, \{4,6\}, \{4,7\},$   
 $\{4,8\}, \{5,6\}, \{5,7\}, \{5,8\}, \{5,10\}, \{6,7\}, \{6,8\}, \{7,8\}, \{7,9\}, \{7,10\}, \{7,11\},$

$\{8,9\}, \{8,10\}, \{9,10\}, \{9,11\}, \{10,11\}, \{1,2\}, \{1,4\}, \{1,7\}, \{1,8\}, \{1,9\},$   
 $\{2,4\}, \{2,7\}, \{2,9\}, \{3,4\}, \{3,5\}, \{3,6\}, \{3,9\}, \{4,5\}, \{4,6\}, \{4,7\}, \{4,8\},$   
 $\{4,9\}, \{5,6\}, \{5,7\}, \{5,8\}, \{5,9\}, \{5,10\}, \{5,11\}, \{6,7\}, \{6,9\}, \{7,8\}, \{7,9\},$   
 $\{7,10\}, \{7,11\}, \{8,9\}, \{8,10\}, \{9,10\}, \{9,11\}, \{10,11\}, \{1,2\}, \{1,3\}, \{1,4\},$   
 $\{1,5\}, \{2,3\}, \{2,4\}, \{2,5\}, \{2,8\}, \{2,10\}, \{2,11\}, \{3,4\}, \{3,5\}, \{3,7\}, \{3,8\},$   
 $\{3,9\}, \{4,5\}, \{4,8\}, \{4,9\}, \{4,10\}, \{4,11\}, \{5,6\}, \{5,7\}, \{5,8\}, \{5,9\}, \{5,10\},$   
 $\{5,11\}, \{6,7\}, \{6,8\}, \{6,9\}, \{7,8\}, \{7,9\}, \{8,9\}, \{8,11\}, \{10,11\}, \{1,2\},$   
 $\{1,3\}, \{1,4\}, \{1,5\}, \{1,7\}, \{1,9\}, \{1,10\}, \{1,11\}, \{2,3\}, \{2,4\}, \{2,8\}, \{2,9\},$   
 $\{2,11\}, \{3,4\}, \{3,11\}, \{4,5\}, \{4,8\}, \{4,9\}, \{4,11\}, \{5,6\}, \{5,7\}, \{5,9\}, \{5,10\},$   
 $\{5,11\}, \{6,7\}, \{6,9\}, \{6,10\}, \{6,11\}, \{7,10\}, \{7,11\}, \{8,9\}, \{8,11\}, \{9,10\},$   
 $\{9,11\}, \{1,2\}, \{1,3\}, \{1,5\}, \{1,7\}, \{2,3\}, \{2,5\}, \{2,6\}, \{2,7\}, \{2,8\}, \{2,9\},$   
 $\{2,11\}, \{3,5\}, \{3,6\}, \{3,7\}, \{3,9\}, \{3,10\}, \{4,5\}, \{4,8\}, \{4,9\}, \{4,10\}, \{4,11\},$   
 $\{5,6\}, \{5,7\}, \{5,10\}, \{5,11\}, \{6,7\}, \{6,8\}, \{6,10\}, \{8,9\}, \{8,10\}, \{8,11\},$   
 $\{9,10\}, \{9,11\}, \{1,2\}, \{1,3\}, \{1,4\}, \{1,5\}, \{1,10\}, \{1,11\}, \{2,3\}, \{2,4\},$   
 $\{2,6\}, \{2,7\}, \{2,8\}, \{2,9\}, \{2,10\}, \{2,11\}, \{3,4\}, \{3,5\}, \{3,6\}, \{3,8\}, \{3,9\},$   
 $\{3,10\}, \{3,11\}, \{4,5\}, \{4,6\}, \{4,7\}, \{4,8\}, \{4,9\}, \{4,10\}, \{4,11\}, \{5,10\},$   
 $\{6,7\}, \{6,8\}, \{6,9\}, \{7,8\}, \{8,10\}, \{1,2\}, \{1,4\}, \{1,5\}, \{1,6\}, \{1,7\}, \{1,8\},$   
 $\{1,9\}, \{1,10\}, \{1,11\}, \{2,5\}, \{2,7\}, \{2,10\}, \{3,4\}, \{3,5\}, \{3,6\}, \{3,8\}, \{3,9\},$   
 $\{4,5\}, \{4,6\}, \{4,8\}, \{4,9\}, \{4,11\}, \{5,6\}, \{5,7\}, \{5,8\}, \{5,10\}, \{5,11\}, \{6,7\},$   
 $\{6,9\}, \{6,11\}, \{7,10\}, \{7,11\}, \{8,9\}, \{10,11\}, \{1,2\}, \{1,3\}, \{1,4\}, \{1,6\},$   
 $\{1,7\}, \{2,3\}, \{2,6\}, \{2,7\}, \{2,11\}, \{3,4\}, \{3,6\}, \{3,11\}, \{4,5\}, \{4,6\}, \{4,7\},$   
 $\{4,8\}, \{4,9\}, \{4,10\}, \{4,11\}, \{5,6\}, \{5,7\}, \{5,8\}, \{6,7\}, \{6,8\}, \{6,11\}, \{7,8\},$   
 $\{7,9\}, \{7,10\}, \{7,11\}, \{8,9\}, \{8,11\}, \{9,10\}, \{9,11\}, \{10,11\}, \{1,2\}, \{1,3\},$   
 $\{1,4\}, \{1,5\}, \{1,9\}, \{1,10\}, \{1,11\}, \{2,3\}, \{2,4\}, \{2,5\}, \{2,8\}, \{2,9\}, \{3,4\},$   
 $\{3,5\}, \{3,6\}, \{3,7\}, \{3,8\}, \{3,9\}, \{3,10\}, \{3,11\}, \{4,5\}, \{4,7\}, \{4,8\}, \{4,10\},$   
 $\{5,6\}, \{5,7\}, \{5,8\}, \{5,9\}, \{5,10\}, \{5,11\}, \{6,7\}, \{6,8\}, \{7,8\}, \{9,11\},$   
 $\{1,2\}, \{1,3\}, \{1,4\}, \{1,7\}, \{1,8\}, \{1,10\}, \{1,11\}, \{2,3\}, \{2,4\}, \{2,5\}, \{2,7\},$   
 $\{2,10\}, \{3,4\}, \{3,5\}, \{3,6\}, \{3,7\}, \{3,8\}, \{3,9\}, \{3,11\}, \{4,7\}, \{4,8\}, \{5,6\},$   
 $\{5,7\}, \{5,10\}, \{5,11\}, \{6,7\}, \{6,9\}, \{6,11\}, \{7,8\}, \{7,9\}, \{7,10\}, \{7,11\},$   
 $\{9,11\}, \{10,11\}, \{1,2\}, \{1,3\}, \{1,4\}, \{1,5\}, \{1,7\}, \{1,10\}, \{1,11\}, \{2,3\},$   
 $\{2,4\}, \{2,5\}, \{3,4\}, \{3,5\}, \{3,7\}, \{3,8\}, \{3,9\}, \{4,5\}, \{4,6\}, \{4,9\}, \{4,11\},$   
 $\{5,6\}, \{5,7\}, \{5,8\}, \{5,9\}, \{5,10\}, \{5,11\}, \{6,9\}, \{6,11\}, \{7,8\}, \{7,9\}, \{7,10\},$   
 $\{8,9\}, \{9,10\}, \{9,11\}, \{10,11\}, \{1,2\}, \{1,3\}, \{1,5\}, \{1,6\}, \{1,7\}, \{1,8\},$   
 $\{1,9\}, \{1,11\}, \{2,3\}, \{2,5\}, \{2,6\}, \{2,8\}, \{3,4\}, \{3,5\}, \{3,8\}, \{3,9\}, \{3,10\},$   
 $\{3,11\}, \{4,5\}, \{4,8\}, \{4,10\}, \{5,6\}, \{5,7\}, \{5,8\}, \{5,10\}, \{6,8\}, \{7,8\}, \{7,9\},$   
 $\{7,10\}, \{8,9\}, \{8,10\}, \{8,11\}, \{9,10\}, \{9,11\}, \{1,2\}, \{1,3\}, \{1,4\}, \{1,5\},$   
 $\{1,7\}, \{1,8\}, \{1,10\}, \{1,11\}, \{2,3\}, \{2,4\}, \{2,5\}, \{2,6\}, \{2,7\}, \{2,10\}, \{2,11\},$   
 $\{3,6\}, \{3,7\}, \{3,8\}, \{4,5\}, \{4,7\}, \{4,10\}, \{4,11\}, \{5,6\}, \{5,7\}, \{5,8\}, \{5,9\},$   
 $\{5,11\}, \{6,7\}, \{6,8\}, \{6,9\}, \{7,8\}, \{7,9\}, \{8,9\}, \{10,11\}, \{1,2\}, \{1,3\},$   
 $\{1,4\}, \{1,5\}, \{1,7\}, \{1,9\}, \{1,11\}, \{2,3\}, \{2,4\}, \{2,5\}, \{2,6\}, \{2,7\}, \{2,9\},$   
 $\{3,4\}, \{3,6\}, \{3,8\}, \{3,9\}, \{3,11\}, \{4,5\}, \{4,6\}, \{4,7\}, \{4,8\}, \{4,9\}, \{4,10\},$   
 $\{4,11\}, \{5,7\}, \{6,7\}, \{6,8\}, \{6,10\}, \{7,10\}, \{7,11\}, \{8,10\}, \{8,11\}, \{10,11\},$   
 $\{1,2\}, \{1,3\}, \{1,4\}, \{1,6\}, \{1,7\}, \{1,8\}, \{1,9\}, \{1,10\}, \{1,11\}, \{2,3\}, \{2,4\},$   
 $\{2,7\}, \{3,4\}, \{3,5\}, \{3,6\}, \{3,7\}, \{3,8\}, \{3,9\}, \{3,10\}, \{3,11\}, \{4,7\}, \{4,9\},$   
 $\{5,6\}, \{5,7\}, \{5,9\}, \{6,7\}, \{6,8\}, \{6,9\}, \{6,10\}, \{7,9\}, \{8,10\}, \{8,11\}, \{9,10\},$   
 $\{10,11\}, \{1,2\}, \{1,3\}, \{1,4\}, \{1,6\}, \{1,10\}, \{2,4\}, \{2,6\}, \{2,10\}, \{2,11\},$   
 $\{3,4\}, \{3,6\}, \{3,10\}, \{4,5\}, \{4,6\}, \{4,7\}, \{4,8\}, \{4,9\}, \{4,10\}, \{4,11\}, \{5,6\},$   
 $\{5,7\}, \{5,8\}, \{5,9\}, \{5,10\}, \{6,7\}, \{6,8\}, \{6,9\}, \{6,10\}, \{6,11\}, \{7,8\}, \{7,10\},$   
 $\{7,11\}, \{8,9\}, \{10,11\}, \{1,2\}, \{1,3\}, \{1,4\}, \{1,8\}, \{1,9\}, \{2,3\}, \{2,4\},$   
 $\{2,5\}, \{2,6\}, \{2,7\}, \{2,8\}, \{2,9\}, \{2,10\}, \{2,11\}, \{3,4\}, \{3,5\}, \{3,6\}, \{3,8\},$

{3,9},{3,10},{4,5},{4,7},{4,9},{5,7},{5,9},{5,10},{5,11},{6,9},{6,10},  
 {7,9},{8,9},{9,10},{9,11},{10,11},{1,2},{1,3},{1,4},{1,9},{2,3},  
 {2,4},{2,5},{2,8},{2,9},{2,11},{3,4},{3,5},{3,6},{3,9},{4,5},{4,8},  
 {4,9},{4,10},{5,6},{5,8},{6,7},{6,8},{6,9},{6,10},{6,11},{7,9},{7,10},  
 {7,11},{8,10},{8,11},{9,10},{9,11},{10,11},{1,2},{1,4},{1,5},{1,6},  
 {1,7},{1,10},{2,3},{2,4},{2,5},{2,7},{2,8},{2,9},{2,11},{3,5},{3,7},  
 {3,8},{3,9},{3,11},{4,5},{4,6},{4,7},{4,8},{4,10},{5,6},{5,7},{5,8},  
 {5,9},{5,10},{6,7},{6,10},{7,8},{7,9},{7,11},{8,11},{1,2},{1,3},  
 {1,4},{1,6},{1,9},{1,10},{1,11},{2,3},{2,4},{2,5},{2,7},{2,8},{2,9},  
 {2,10},{3,4},{3,5},{3,6},{3,10},{4,5},{4,7},{4,8},{4,10},{4,11},{5,6},  
 {5,7},{5,8},{6,7},{6,9},{6,11},{7,8},{7,9},{7,11},{9,11},{1,2},  
 {1,3},{1,4},{1,8},{1,9},{1,10},{1,11},{2,4},{2,5},{2,6},{2,7},{2,8},  
 {2,11},{3,4},{3,5},{3,6},{3,7},{3,8},{3,9},{4,7},{4,9},{5,6},{5,8},  
 {5,10},{5,11},{6,7},{6,9},{6,10},{7,9},{8,11},{9,10},{10,11},{1,2},  
 {1,3},{1,4},{1,6},{1,9},{2,3},{2,4},{2,5},{2,7},{2,8},{2,9},{2,11},  
 {3,4},{3,5},{3,6},{3,7},{3,8},{3,9},{3,10},{3,11},{4,6},{4,7},{4,10},  
 {5,6},{5,8},{5,9},{5,11},{6,7},{6,9},{6,10},{6,11},{7,10},{7,11},  
 {8,9},{1,2},{1,3},{1,5},{1,6},{1,9},{2,3},{2,4},{2,5},{2,6},{2,7},  
 {2,8},{2,9},{2,10},{2,11},{3,4},{3,6},{3,7},{3,8},{3,9},{3,11},{4,6},  
 {4,7},{4,10},{4,11},{5,6},{5,9},{6,7},{6,9},{7,8},{7,9},{7,10},{7,11},  
 {8,9},{10,11},{1,2},{1,3},{1,4},{1,7},{1,9},{1,10},{1,11},{2,3},  
 {2,5},{2,6},{2,7},{2,8},{2,9},{2,10},{3,4},{3,5},{3,6},{3,7},{3,10},  
 {3,11},{4,6},{4,8},{4,9},{4,10},{4,11},{5,7},{5,10},{6,8},{6,9},  
 {7,10},{8,9},{8,10},{10,11},{1,2},{1,3},{1,5},{1,6},{1,9},{1,10},  
 {2,3},{2,5},{2,9},{3,4},{3,5},{3,6},{3,7},{3,9},{3,11},{4,6},{4,9},  
 {4,11},{5,6},{5,7},{5,8},{5,9},{5,10},{6,7},{6,8},{6,9},{6,10},{6,11},  
 {7,8},{7,9},{7,11},{8,9},{9,10},{9,11},{1,2},{1,3},{1,4},{1,5},  
 {1,6},{1,7},{1,8},{1,9},{1,10},{1,11},{2,4},{2,8},{2,11},{3,4},{3,5},  
 {3,6},{3,7},{3,8},{3,9},{3,10},{4,5},{4,8},{4,11},{5,6},{5,8},{5,9},  
 {5,10},{5,11},{6,9},{7,8},{7,10},{8,10},{8,11},{9,10},{1,2},{1,3},  
 {1,5},{1,7},{1,8},{1,9},{2,3},{2,4},{2,5},{2,6},{2,7},{2,9},{2,11},  
 {3,4},{3,5},{3,7},{3,8},{3,9},{4,5},{4,6},{4,9},{5,6},{5,9},{5,10},  
 {5,11},{6,9},{6,10},{6,11},{7,8},{7,9},{8,9},{9,10},{9,11},{10,11},  
 {1,2},{1,5},{1,7},{1,8},{1,9},{1,10},{2,3},{2,4},{2,5},{2,6},{2,7},  
 {2,8},{2,9},{2,11},{3,4},{3,5},{3,7},{3,11},{4,5},{4,6},{4,7},{4,9},  
 {4,11},{5,7},{5,8},{5,9},{5,10},{6,7},{6,11},{7,8},{7,9},{7,10},  
 {7,11},{9,10},{1,2},{1,5},{1,6},{1,7},{1,9},{2,3},{2,5},{2,6},{2,7},  
 {2,8},{2,9},{2,11},{3,4},{3,5},{3,6},{3,8},{3,9},{3,10},{4,5},{4,6},  
 {4,8},{4,11},{5,6},{5,7},{5,9},{5,10},{5,11},{6,7},{6,8},{6,9},{6,10},  
 {6,11},{8,11},{9,10},{1,2},{1,3},{1,4},{1,5},{1,6},{1,8},{1,11},  
 {2,4},{2,6},{2,9},{2,11},{3,4},{3,8},{3,11},{4,5},{4,6},{4,7},{4,8},  
 {4,9},{4,10},{4,11},{5,6},{5,8},{6,7},{6,8},{6,9},{6,10},{6,11},  
 {7,10},{7,11},{8,10},{8,11},{9,11},{10,11},{1,2},{1,3},{1,4},{1,5},  
 {1,6},{1,7},{1,8},{1,9},{1,10},{2,3},{2,5},{2,6},{2,7},{2,9},{2,10},  
 {2,11},{3,4},{3,5},{3,8},{3,9},{3,10},{4,5},{4,10},{5,6},{5,7},{5,10},  
 {5,11},{6,7},{6,11},{7,10},{7,11},{8,9},{8,10},{9,10},{1,2},{1,3},  
 {1,4},{1,5},{1,6},{1,8},{1,9},{1,10},{2,3},{2,4},{2,5},{2,6},{2,7},  
 {2,8},{2,9},{2,10},{2,11},{3,4},{3,6},{4,6},{4,7},{4,10},{5,6},{5,9},  
 {6,7},{6,9},{6,11},{7,9},{7,10},{7,11},{8,9},{8,10},{9,10},{9,11},  
 {1,2},{1,3},{1,4},{1,5},{1,6},{1,8},{1,9},{1,10},{2,3},{2,4},{2,6},

$\{2,7\}, \{2,8\}, \{2,10\}, \{2,11\}, \{3,4\}, \{3,5\}, \{3,8\}, \{4,5\}, \{4,6\}, \{4,8\}, \{4,9\},$   
 $\{5,8\}, \{5,9\}, \{6,7\}, \{6,8\}, \{6,10\}, \{6,11\}, \{7,8\}, \{7,10\}, \{7,11\}, \{8,9\},$   
 $\{8,10\}, \{8,11\}, \{\{1,2\}, \{1,5\}, \{1,6\}, \{1,10\}, \{2,4\}, \{2,5\}, \{2,8\}, \{2,10\},$   
 $\{2,11\}, \{3,4\}, \{3,5\}, \{3,6\}, \{4,5\}, \{4,6\}, \{4,7\}, \{4,8\}, \{4,11\}, \{5,6\}, \{5,9\},$   
 $\{5,11\}, \{6,7\}, \{6,9\}, \{6,10\}, \{7,8\}, \{7,9\}, \{7,10\}, \{8,9\}, \{8,10\}, \{8,11\},$   
 $\{9,10\}, \{9,11\}, \{\{1,2\}, \{1,3\}, \{1,4\}, \{1,5\}, \{1,6\}, \{1,7\}, \{1,8\}, \{1,9\},$   
 $\{1,10\}, \{1,11\}, \{2,3\}, \{2,4\}, \{2,5\}, \{2,6\}, \{2,7\}, \{2,11\}, \{3,4\}, \{3,6\}, \{3,7\},$   
 $\{3,8\}, \{3,9\}, \{3,10\}, \{3,11\}, \{4,5\}, \{4,7\}, \{4,8\}, \{4,9\}, \{4,10\}, \{4,11\},$   
 $\{5,11\}, \{6,11\}, \{7,10\}, \{8,9\}, \{8,10\}, \{\{1,2\}, \{1,3\}, \{1,4\}, \{1,5\}, \{1,8\},$   
 $\{1,9\}, \{2,3\}, \{2,5\}, \{2,6\}, \{2,7\}, \{2,8\}, \{2,9\}, \{2,11\}, \{3,4\}, \{3,5\}, \{3,7\},$   
 $\{4,5\}, \{4,7\}, \{4,8\}, \{5,6\}, \{5,7\}, \{5,8\}, \{5,9\}, \{5,10\}, \{5,11\}, \{6,7\}, \{6,8\},$   
 $\{6,10\}, \{6,11\}, \{7,8\}, \{7,10\}, \{7,11\}, \{8,9\}, \{8,10\}, \{\{1,2\}, \{1,3\}, \{1,4\},$   
 $\{1,6\}, \{1,10\}, \{2,3\}, \{2,4\}, \{2,6\}, \{2,8\}, \{3,4\}, \{3,5\}, \{3,6\}, \{3,7\}, \{3,8\},$   
 $\{3,9\}, \{3,10\}, \{3,11\}, \{4,5\}, \{4,6\}, \{4,7\}, \{4,8\}, \{4,9\}, \{4,10\}, \{5,6\}, \{5,7\},$   
 $\{5,8\}, \{6,8\}, \{6,9\}, \{6,10\}, \{6,11\}, \{7,8\}, \{9,10\}, \{9,11\}, \{10,11\}, \{\{1,2\},$   
 $\{1,4\}, \{1,5\}, \{1,6\}, \{1,7\}, \{1,8\}, \{1,9\}, \{1,10\}, \{1,11\}, \{2,3\}, \{2,7\}, \{2,8\},$   
 $\{2,9\}, \{2,11\}, \{3,8\}, \{3,9\}, \{3,11\}, \{4,5\}, \{4,6\}, \{4,7\}, \{4,9\}, \{5,6\}, \{5,9\},$   
 $\{5,10\}, \{6,7\}, \{6,8\}, \{6,9\}, \{6,10\}, \{7,8\}, \{7,9\}, \{8,9\}, \{8,11\}, \{9,10\},$   
 $\{9,11\}, \{\{1,2\}, \{1,3\}, \{1,6\}, \{1,8\}, \{1,10\}, \{2,3\}, \{2,6\}, \{2,7\}, \{2,10\},$   
 $\{3,4\}, \{3,6\}, \{3,10\}, \{4,6\}, \{4,7\}, \{4,8\}, \{4,9\}, \{4,10\}, \{4,11\}, \{5,6\}, \{5,7\},$   
 $\{5,8\}, \{5,11\}, \{6,7\}, \{6,8\}, \{6,9\}, \{6,11\}, \{7,8\}, \{7,9\}, \{7,10\}, \{7,11\},$   
 $\{8,10\}, \{8,11\}, \{9,11\}, \{\{1,2\}, \{1,3\}, \{1,4\}, \{1,5\}, \{1,6\}, \{1,7\}, \{1,8\},$   
 $\{1,9\}, \{1,10\}, \{1,11\}, \{2,3\}, \{2,4\}, \{2,7\}, \{2,9\}, \{2,10\}, \{2,11\}, \{3,4\}, \{3,5\},$   
 $\{3,6\}, \{3,7\}, \{3,8\}, \{3,9\}, \{4,7\}, \{5,6\}, \{5,8\}, \{5,9\}, \{6,9\}, \{7,8\}, \{7,10\},$   
 $\{8,9\}, \{8,10\}, \{9,10\}, \{9,11\}, \{10,11\}, \{\{1,2\}, \{1,7\}, \{1,8\}, \{1,9\}, \{2,5\},$   
 $\{2,7\}, \{2,8\}, \{2,9\}, \{2,10\}, \{2,11\}, \{3,4\}, \{3,5\}, \{3,6\}, \{3,7\}, \{3,8\}, \{4,5\},$   
 $\{4,7\}, \{4,8\}, \{4,9\}, \{5,6\}, \{5,7\}, \{5,8\}, \{5,9\}, \{5,10\}, \{6,7\}, \{6,8\}, \{7,8\},$   
 $\{7,9\}, \{7,10\}, \{7,11\}, \{8,9\}, \{8,10\}, \{8,11\}, \{10,11\}, \{\{1,2\}, \{1,4\}, \{1,5\},$   
 $\{1,7\}, \{1,8\}, \{1,9\}, \{1,10\}, \{2,5\}, \{2,8\}, \{2,10\}, \{3,4\}, \{3,7\}, \{3,9\}, \{3,11\},$   
 $\{4,5\}, \{4,6\}, \{4,7\}, \{4,9\}, \{4,10\}, \{4,11\}, \{5,6\}, \{5,7\}, \{5,8\}, \{5,9\}, \{5,10\},$   
 $\{6,7\}, \{6,9\}, \{6,11\}, \{7,8\}, \{7,9\}, \{7,10\}, \{7,11\}, \{8,10\}, \{9,11\}, \{\{1,2\},$   
 $\{1,3\}, \{1,5\}, \{1,6\}, \{1,8\}, \{1,9\}, \{2,3\}, \{2,5\}, \{2,6\}, \{2,7\}, \{2,10\}, \{2,11\},$   
 $\{3,5\}, \{3,7\}, \{3,8\}, \{3,10\}, \{3,11\}, \{4,5\}, \{4,6\}, \{4,8\}, \{4,9\}, \{4,11\}, \{5,6\},$   
 $\{5,7\}, \{5,8\}, \{5,9\}, \{5,11\}, \{6,9\}, \{6,11\}, \{7,10\}, \{7,11\}, \{8,9\}, \{8,11\},$   
 $\{10,11\}, \{\{1,2\}, \{1,3\}, \{1,4\}, \{1,5\}, \{1,6\}, \{1,8\}, \{1,9\}, \{1,10\}, \{1,11\},$   
 $\{2,5\}, \{2,8\}, \{2,9\}, \{3,4\}, \{3,5\}, \{3,6\}, \{3,7\}, \{3,9\}, \{3,11\}, \{4,6\}, \{4,7\},$   
 $\{4,11\}, \{5,6\}, \{5,8\}, \{5,9\}, \{5,10\}, \{5,11\}, \{6,7\}, \{6,8\}, \{6,9\}, \{6,10\},$   
 $\{6,11\}, \{7,11\}, \{8,9\}, \{10,11\}, \{\{1,2\}, \{1,3\}, \{1,4\}, \{1,6\}, \{1,10\}, \{2,3\},$   
 $\{2,7\}, \{2,8\}, \{2,9\}, \{2,10\}, \{2,11\}, \{3,4\}, \{3,5\}, \{3,6\}, \{3,7\}, \{4,6\}, \{4,7\},$   
 $\{4,8\}, \{4,10\}, \{5,6\}, \{5,7\}, \{5,9\}, \{6,9\}, \{6,10\}, \{7,8\}, \{7,9\}, \{7,11\}, \{8,9\},$   
 $\{8,10\}, \{8,11\}, \{9,10\}, \{9,11\}, \{\{1,2\}, \{1,4\}, \{1,7\}, \{1,8\}, \{1,9\}, \{1,11\},$   
 $\{2,5\}, \{2,6\}, \{2,8\}, \{2,9\}, \{2,11\}, \{3,4\}, \{3,5\}, \{3,6\}, \{3,7\}, \{3,8\}, \{3,9\},$   
 $\{3,10\}, \{3,11\}, \{4,6\}, \{4,7\}, \{4,11\}, \{5,6\}, \{5,7\}, \{5,9\}, \{5,10\}, \{6,10\},$   
 $\{6,11\}, \{7,9\}, \{8,9\}, \{8,11\}, \{\{1,2\}, \{1,3\}, \{1,5\}, \{1,10\}, \{1,11\}, \{2,3\},$   
 $\{2,5\}, \{2,7\}, \{2,8\}, \{2,10\}, \{3,4\}, \{3,5\}, \{3,6\}, \{3,7\}, \{3,9\}, \{3,10\}, \{3,11\},$   
 $\{4,5\}, \{4,6\}, \{4,10\}, \{5,6\}, \{5,7\}, \{5,8\}, \{5,9\}, \{5,10\}, \{5,11\}, \{6,7\}, \{6,9\},$   
 $\{6,10\}, \{7,8\}, \{7,9\}, \{7,10\}, \{8,10\}, \{10,11\}, \{\{1,2\}, \{1,3\}, \{1,5\}, \{1,6\},$   
 $\{1,7\}, \{1,8\}, \{1,9\}, \{1,11\}, \{2,3\}, \{2,4\}, \{2,5\}, \{2,9\}, \{2,10\}, \{3,4\}, \{3,6\},$   
 $\{3,7\}, \{3,8\}, \{3,9\}, \{3,11\}, \{4,5\}, \{4,7\}, \{4,9\}, \{4,10\}, \{5,7\}, \{5,9\}, \{5,10\},$   
 $\{6,7\}, \{6,8\}, \{7,8\}, \{7,9\}, \{8,9\}, \{8,11\}, \{9,10\}, \{9,11\}, \{\{1,2\}, \{1,3\},$

{1,4},{1,5},{1,6},{1,7},{1,9},{1,10},{1,11},{2,3},{2,7},{2,8},{2,10},  
{2,11},{3,4},{3,5},{3,6},{3,7},{3,8},{3,9},{3,10},{4,6},{4,7},{5,7},  
{5,10},{6,7},{6,9},{7,8},{7,9},{7,10},{7,11},{8,9},{8,11},{9,11}},  
{{1,2},{1,3},{1,4},{1,5},{1,7},{1,9},{1,10},{1,11},{2,3},{2,7},{2,8},  
{2,9},{3,4},{3,5},{3,6},{3,7},{3,8},{3,9},{3,10},{3,11},{4,5},{4,6},  
{4,10},{5,6},{5,9},{6,7},{6,8},{6,9},{6,10},{6,11},{7,8},{7,11},{8,9},  
{10,11}},{{1,2},{1,3},{1,5},{1,6},{1,7},{1,8},{1,9},{1,11},{2,5},  
{2,6},{2,7},{2,11},{3,4},{3,5},{3,6},{3,7},{3,8},{3,9},{3,10},{4,5},  
{4,6},{4,9},{4,10},{5,6},{5,7},{5,8},{5,9},{5,10},{5,11},{6,7},{6,9},  
{6,11},{8,9},{9,10}},{{1,2},{1,3},{1,4},{1,6},{1,9},{1,10},{1,11},  
{2,3},{2,4},{2,5},{2,6},{2,7},{2,9},{2,10},{3,4},{3,5},{3,7},{3,8},  
{3,10},{4,5},{4,9},{4,10},{5,7},{5,8},{5,10},{6,9},{6,10},{6,11},  
{7,8},{7,10},{8,10},{9,10},{9,11},{10,11}},{{1,2},{1,3},{1,4},{1,7},  
{1,8},{1,9},{1,11},{2,3},{2,4},{2,5},{2,8},{2,9},{2,11},{3,5},{3,6},  
{3,7},{3,8},{3,10},{3,11},{4,5},{4,7},{4,9},{4,11},{5,6},{5,7},{5,10},  
{5,11},{6,7},{6,10},{7,10},{7,11},{8,11},{9,11},{10,11}},{{1,2},{1,3},  
{1,4},{1,5},{1,6},{2,3},{2,4},{2,5},{2,6},{2,7},{2,9},{2,10},{2,11},  
{3,4},{3,6},{3,7},{3,8},{3,9},{4,5},{4,6},{4,8},{4,11},{5,6},{6,7},  
{6,8},{6,9},{6,10},{6,11},{7,8},{7,9},{7,10},{7,11},{8,11},{9,10}},  
{{1,2},{1,3},{1,6},{1,8},{2,3},{2,4},{2,5},{2,6},{2,7},{2,8},{2,9},  
{2,10},{2,11},{3,4},{3,5},{3,6},{3,7},{3,8},{3,9},{3,10},{4,5},{4,6},  
{4,7},{4,8},{4,9},{4,10},{4,11},{5,6},{6,8},{6,11},{7,8},{7,10},  
{8,11},{9,10}},{{1,2},{1,3},{1,4},{1,5},{1,6},{1,7},{1,8},{1,9},  
{1,10},{1,11},{2,3},{2,7},{2,9},{2,10},{3,4},{3,5},{3,7},{3,8},{3,9},  
{3,10},{4,5},{4,8},{5,6},{5,7},{5,8},{5,9},{6,7},{6,8},{6,11},{7,8},  
{7,9},{7,11},{8,11},{9,10}},{{1,2},{1,3},{1,4},{1,9},{1,10},{1,11},  
{2,3},{2,9},{2,10},{2,11},{3,4},{3,5},{3,6},{3,7},{3,8},{3,9},{3,11},  
{4,7},{4,9},{4,11},{5,6},{5,7},{5,8},{6,7},{6,8},{6,9},{6,11},{7,8},  
{7,9},{7,11},{8,11},{9,10},{9,11},{10,11}},{{1,2},{1,6},{1,7},{1,8},  
{2,3},{2,4},{2,5},{2,6},{2,7},{2,8},{2,11},{3,4},{3,5},{3,6},{3,7},  
{3,8},{3,10},{4,5},{4,6},{4,8},{4,9},{4,10},{4,11},{5,6},{5,9},{5,10},  
{5,11},{6,7},{6,8},{6,9},{6,10},{6,11},{7,8},{9,10}},{{1,2},{1,3},  
{1,4},{1,7},{1,10},{1,11},{2,3},{2,5},{2,6},{2,7},{2,8},{2,10},{2,11},  
{3,4},{3,5},{3,10},{3,11},{4,5},{4,6},{4,7},{4,11},{5,6},{5,7},{5,8},  
{5,9},{6,7},{6,8},{6,9},{6,11},{7,8},{7,9},{8,9},{10,11}},{{1,2},  
{1,5},{1,6},{1,7},{1,8},{1,10},{2,3},{2,5},{2,6},{2,7},{2,9},{2,10},  
{2,11},{3,4},{3,6},{3,10},{3,11},{4,6},{4,10},{4,11},{5,6},{5,8},  
{5,9},{6,7},{6,8},{6,9},{6,10},{6,11},{7,8},{7,9},{7,10},{7,11},{8,9},  
{10,11}},{{1,2},{1,3},{1,4},{1,5},{1,6},{1,9},{1,10},{2,4},{2,6},  
{2,7},{2,8},{2,11},{3,4},{3,5},{3,6},{3,8},{3,9},{3,10},{4,5},{4,7},  
{4,8},{4,10},{4,11},{5,6},{5,7},{5,9},{5,10},{6,7},{6,8},{6,9},{7,8},  
{7,11},{8,11}},{{1,2},{1,3},{1,5},{1,6},{1,7},{1,8},{1,9},{1,11},  
{2,3},{2,4},{2,5},{2,7},{2,8},{2,9},{2,10},{2,11},{3,4},{3,7},{3,8},  
{3,11},{4,8},{4,10},{4,11},{5,8},{5,11},{6,7},{6,8},{6,9},{7,8},{7,9},  
{8,9},{8,10},{8,11},{10,11}},{{1,2},{1,3},{1,4},{1,5},{1,6},{1,9},  
{1,10},{1,11},{2,3},{2,8},{2,9},{2,10},{3,6},{3,7},{3,8},{3,9},{3,11},  
{4,5},{4,6},{4,10},{5,6},{5,7},{5,9},{5,10},{6,7},{6,10},{6,11},{7,8},  
{7,9},{7,10},{8,9},{8,10}},{{1,2},{1,7},{1,8},{1,10},{1,11},{2,3},  
{2,5},{2,6},{2,7},{2,10},{2,11},{3,4},{3,5},{3,6},{3,7},{4,5},{4,6},  
{4,7},{5,6},{5,7},{5,9},{5,11},{6,7},{6,9},{6,10},{7,8},{7,9},{7,10},

$\{7,11\}, \{8,10\}, \{8,11\}, \{9,10\}, \{9,11\}, \{10,11\}, \{\{1,2\}, \{1,4\}, \{1,5\}, \{1,7\},$   
 $\{1,8\}, \{1,9\}, \{1,10\}, \{2,3\}, \{2,4\}, \{2,5\}, \{2,6\}, \{2,8\}, \{2,10\}, \{3,4\}, \{3,5\},$   
 $\{3,9\}, \{3,10\}, \{4,6\}, \{4,7\}, \{4,9\}, \{4,10\}, \{4,11\}, \{5,9\}, \{5,10\}, \{6,7\}, \{6,8\},$   
 $\{6,10\}, \{6,11\}, \{7,8\}, \{7,10\}, \{7,11\}, \{8,10\}, \{9,10\}, \{10,11\}, \{\{1,2\}, \{1,5\},$   
 $\{1,6\}, \{1,7\}, \{1,8\}, \{1,10\}, \{2,3\}, \{2,6\}, \{2,10\}, \{2,11\}, \{3,4\}, \{3,6\}, \{3,10\},$   
 $\{3,11\}, \{4,5\}, \{4,6\}, \{4,7\}, \{4,8\}, \{4,9\}, \{4,10\}, \{5,6\}, \{5,8\}, \{5,9\}, \{6,9\},$   
 $\{6,11\}, \{7,8\}, \{7,10\}, \{7,11\}, \{8,9\}, \{8,11\}, \{9,11\}, \{10,11\}, \{\{1,2\}, \{1,3\},$   
 $\{1,4\}, \{1,5\}, \{1,6\}, \{1,7\}, \{1,8\}, \{1,9\}, \{1,10\}, \{1,11\}, \{2,3\}, \{2,5\}, \{2,9\},$   
 $\{3,4\}, \{3,5\}, \{3,6\}, \{3,7\}, \{3,8\}, \{3,9\}, \{3,10\}, \{3,11\}, \{4,5\}, \{4,7\}, \{4,8\},$   
 $\{5,6\}, \{5,7\}, \{5,8\}, \{5,9\}, \{5,10\}, \{5,11\}, \{6,7\}, \{6,10\}, \{8,9\}, \{10,11\}\},$   
 $\{\{1,2\}, \{1,3\}, \{1,5\}, \{1,6\}, \{1,9\}, \{1,10\}, \{1,11\}, \{2,4\}, \{2,5\}, \{2,6\}, \{2,7\},$   
 $\{2,10\}, \{3,4\}, \{3,5\}, \{3,6\}, \{3,7\}, \{3,8\}, \{3,9\}, \{3,10\}, \{3,11\}, \{4,5\}, \{4,6\},$   
 $\{4,7\}, \{5,6\}, \{5,7\}, \{5,8\}, \{5,9\}, \{5,10\}, \{5,11\}, \{6,8\}, \{6,9\}, \{7,10\}, \{8,9\},$   
 $\{9,11\}\}, \{\{1,2\}, \{1,4\}, \{1,5\}, \{1,6\}, \{1,7\}, \{1,9\}, \{1,11\}, \{2,3\}, \{2,5\}, \{2,6\},$   
 $\{2,8\}, \{2,9\}, \{2,10\}, \{2,11\}, \{3,4\}, \{3,6\}, \{3,9\}, \{3,10\}, \{4,6\}, \{4,9\}, \{4,10\},$   
 $\{4,11\}, \{5,7\}, \{5,8\}, \{5,11\}, \{6,7\}, \{6,8\}, \{6,11\}, \{7,8\}, \{7,11\}, \{8,11\},$   
 $\{9,10\}, \{10,11\}\}, \{\{1,2\}, \{1,3\}, \{1,4\}, \{1,5\}, \{1,7\}, \{1,9\}, \{2,3\}, \{2,5\},$   
 $\{2,6\}, \{2,7\}, \{2,8\}, \{2,9\}, \{2,10\}, \{2,11\}, \{3,4\}, \{3,5\}, \{3,6\}, \{3,8\}, \{3,9\},$   
 $\{3,10\}, \{4,5\}, \{4,9\}, \{5,6\}, \{5,7\}, \{5,8\}, \{5,9\}, \{5,11\}, \{6,8\}, \{6,9\}, \{6,10\},$   
 $\{7,9\}, \{7,11\}, \{9,10\}, \{9,11\}\}, \{\{1,2\}, \{1,3\}, \{1,4\}, \{1,7\}, \{1,8\}, \{1,9\},$   
 $\{1,10\}, \{1,11\}, \{2,3\}, \{2,4\}, \{2,8\}, \{2,11\}, \{3,4\}, \{3,8\}, \{4,8\}, \{4,9\}, \{4,11\},$   
 $\{5,6\}, \{5,7\}, \{5,8\}, \{5,10\}, \{5,11\}, \{6,7\}, \{6,8\}, \{6,9\}, \{6,10\}, \{7,8\}, \{7,10\},$   
 $\{8,9\}, \{8,11\}, \{9,10\}, \{9,11\}, \{10,11\}\}, \{\{1,2\}, \{1,5\}, \{1,6\}, \{1,9\}, \{1,11\},$   
 $\{2,4\}, \{2,7\}, \{2,8\}, \{2,9\}, \{2,10\}, \{2,11\}, \{3,4\}, \{3,5\}, \{3,6\}, \{3,8\}, \{3,11\},$   
 $\{4,5\}, \{4,7\}, \{4,8\}, \{4,9\}, \{4,10\}, \{5,6\}, \{5,9\}, \{6,7\}, \{6,8\}, \{6,9\}, \{6,11\},$   
 $\{7,8\}, \{7,9\}, \{7,10\}, \{8,11\}, \{9,10\}\}, \{\{1,2\}, \{1,5\}, \{1,6\}, \{1,7\}, \{1,8\},$   
 $\{2,5\}, \{2,7\}, \{2,8\}, \{2,9\}, \{3,4\}, \{3,5\}, \{3,7\}, \{3,8\}, \{3,9\}, \{3,11\}, \{4,5\},$   
 $\{4,6\}, \{4,8\}, \{4,10\}, \{4,11\}, \{5,6\}, \{5,7\}, \{5,9\}, \{6,7\}, \{6,8\}, \{6,10\}, \{6,11\},$   
 $\{7,9\}, \{7,11\}, \{8,9\}, \{8,10\}, \{8,11\}, \{10,11\}\}, \{\{1,2\}, \{1,5\}, \{1,6\}, \{1,7\},$   
 $\{1,8\}, \{1,9\}, \{1,10\}, \{2,3\}, \{2,6\}, \{2,7\}, \{2,8\}, \{2,9\}, \{3,4\}, \{3,7\}, \{3,9\},$   
 $\{3,10\}, \{3,11\}, \{4,7\}, \{4,10\}, \{4,11\}, \{5,6\}, \{5,9\}, \{5,10\}, \{5,11\}, \{6,7\},$   
 $\{6,8\}, \{6,11\}, \{7,8\}, \{7,10\}, \{7,11\}, \{9,10\}, \{10,11\}\}, \{\{1,2\}, \{1,3\}, \{1,4\},$   
 $\{1,6\}, \{1,7\}, \{1,8\}, \{1,9\}, \{1,10\}, \{1,11\}, \{2,3\}, \{2,5\}, \{2,6\}, \{2,7\}, \{2,9\},$   
 $\{3,4\}, \{3,5\}, \{3,6\}, \{3,7\}, \{3,8\}, \{3,9\}, \{3,10\}, \{3,11\}, \{4,6\}, \{4,8\}, \{5,6\},$   
 $\{5,7\}, \{6,7\}, \{6,8\}, \{6,9\}, \{6,10\}, \{6,11\}, \{7,8\}, \{9,10\}, \{10,11\}\}, \{\{1,2\},$   
 $\{1,4\}, \{1,5\}, \{1,6\}, \{1,7\}, \{1,9\}, \{1,10\}, \{2,3\}, \{2,4\}, \{2,5\}, \{2,7\}, \{3,4\},$   
 $\{3,5\}, \{3,6\}, \{3,7\}, \{4,5\}, \{4,6\}, \{5,6\}, \{5,7\}, \{5,8\}, \{5,10\}, \{5,11\}, \{6,7\},$   
 $\{6,8\}, \{6,9\}, \{7,9\}, \{7,11\}, \{8,9\}, \{8,10\}, \{8,11\}, \{9,10\}, \{9,11\}, \{10,11\}\},$   
 $\{\{1,2\}, \{1,5\}, \{1,6\}, \{1,7\}, \{1,9\}, \{1,10\}, \{2,4\}, \{2,5\}, \{2,6\}, \{2,7\}, \{2,8\},$   
 $\{2,9\}, \{2,10\}, \{2,11\}, \{3,4\}, \{3,5\}, \{3,7\}, \{3,9\}, \{4,5\}, \{4,7\}, \{4,8\}, \{4,9\},$   
 $\{4,11\}, \{5,7\}, \{5,9\}, \{5,10\}, \{6,7\}, \{6,10\}, \{7,9\}, \{7,10\}, \{7,11\}, \{8,9\},$   
 $\{8,11\}, \{9,11\}\}, \{\{1,2\}, \{1,3\}, \{1,5\}, \{1,8\}, \{1,9\}, \{1,10\}, \{2,3\}, \{2,4\},$   
 $\{2,7\}, \{2,8\}, \{2,10\}, \{2,11\}, \{3,4\}, \{3,5\}, \{3,6\}, \{3,8\}, \{3,9\}, \{4,6\}, \{4,9\},$   
 $\{4,10\}, \{4,11\}, \{5,7\}, \{5,8\}, \{5,9\}, \{5,11\}, \{6,9\}, \{7,8\}, \{7,11\}, \{9,10\},$   
 $\{9,11\}, \{10,11\}\}, \{\{1,2\}, \{1,6\}, \{1,8\}, \{1,9\}, \{2,5\}, \{2,6\}, \{2,8\}, \{2,9\},$   
 $\{3,4\}, \{3,5\}, \{3,6\}, \{3,7\}, \{3,8\}, \{3,10\}, \{4,6\}, \{4,7\}, \{4,8\}, \{5,6\}, \{5,7\},$   
 $\{5,8\}, \{5,9\}, \{5,10\}, \{5,11\}, \{6,7\}, \{6,8\}, \{6,9\}, \{6,10\}, \{6,11\}, \{7,8\}, \{8,9\},$   
 $\{8,10\}, \{8,11\}, \{9,11\}, \{10,11\}\}, \{\{1,2\}, \{1,7\}, \{1,8\}, \{1,11\}, \{2,4\}, \{2,5\},$   
 $\{2,6\}, \{2,7\}, \{2,8\}, \{2,9\}, \{2,10\}, \{2,11\}, \{3,4\}, \{3,5\}, \{3,7\}, \{3,8\}, \{3,9\},$   
 $\{3,10\}, \{3,11\}, \{4,7\}, \{4,9\}, \{4,11\}, \{5,6\}, \{5,7\}, \{5,9\}, \{5,10\}, \{6,7\}, \{6,9\},$

$\{7,8\},\{7,9\},\{7,10\},\{7,11\},\{8,10\},\{8,11\},\{\{1,2\},\{1,3\},\{1,5\},\{1,7\},$   
 $\{1,8\},\{2,3\},\{2,7\},\{2,8\},\{2,10\},\{3,5\},\{3,6\},\{3,10\},\{3,11\},\{4,5\},\{4,6\},$   
 $\{4,7\},\{4,9\},\{4,10\},\{4,11\},\{5,7\},\{5,8\},\{5,11\},\{6,9\},\{6,10\},\{6,11\},$   
 $\{7,8\},\{7,10\},\{8,9\},\{8,10\},\{8,11\},\{9,10\},\{9,11\},\{\{1,2\},\{1,4\},\{1,5\},$   
 $\{1,6\},\{1,7\},\{1,9\},\{2,3\},\{2,4\},\{2,5\},\{2,6\},\{2,7\},\{2,8\},\{2,10\},\{2,11\},$   
 $\{3,7\},\{3,8\},\{3,11\},\{4,5\},\{4,6\},\{4,7\},\{4,9\},\{4,10\},\{5,7\},\{5,8\},\{5,10\},$   
 $\{5,11\},\{6,7\},\{6,9\},\{7,8\},\{7,9\},\{7,10\},\{7,11\},\{8,11\},\{10,11\},\{\{1,2\},$   
 $\{1,4\},\{1,5\},\{1,8\},\{1,11\},\{2,3\},\{2,4\},\{2,8\},\{2,9\},\{2,10\},\{2,11\},\{3,4\},$   
 $\{3,8\},\{3,10\},\{4,5\},\{4,6\},\{4,8\},\{4,9\},\{4,10\},\{4,11\},\{5,6\},\{5,7\},\{5,8\},$   
 $\{5,11\},\{6,7\},\{6,8\},\{6,11\},\{7,8\},\{7,11\},\{8,10\},\{8,11\},\{9,10\},\{9,11\},$   
 $\{10,11\},\{\{1,2\},\{1,3\},\{1,4\},\{1,5\},\{1,6\},\{1,7\},\{1,8\},\{1,9\},\{1,10\},$   
 $\{1,11\},\{2,3\},\{2,4\},\{2,6\},\{2,8\},\{2,9\},\{2,11\},\{3,4\},\{3,6\},\{3,7\},\{3,8\},$   
 $\{3,11\},\{4,8\},\{4,9\},\{4,10\},\{5,6\},\{5,7\},\{5,11\},\{6,7\},\{6,11\},\{7,11\},$   
 $\{8,9\},\{8,10\},\{8,11\},\{9,10\},\{\{1,2\},\{1,3\},\{1,4\},\{1,5\},\{1,7\},\{1,10\},$   
 $\{1,11\},\{2,3\},\{2,4\},\{2,5\},\{2,6\},\{2,7\},\{2,8\},\{2,10\},\{2,11\},\{3,4\},\{3,10\},$   
 $\{4,5\},\{4,6\},\{4,7\},\{4,8\},\{4,9\},\{4,10\},\{4,11\},\{5,7\},\{5,8\},\{6,7\},\{6,8\},$   
 $\{6,9\},\{7,8\},\{7,9\},\{7,11\},\{8,9\},\{10,11\},\{\{1,2\},\{1,4\},\{1,7\},\{1,9\},$   
 $\{1,10\},\{1,11\},\{2,4\},\{2,5\},\{2,6\},\{2,8\},\{2,9\},\{2,10\},\{3,4\},\{3,5\},\{3,6\},$   
 $\{3,7\},\{3,8\},\{3,10\},\{4,7\},\{4,8\},\{4,9\},\{4,11\},\{5,6\},\{5,8\},\{5,10\},\{6,7\},$   
 $\{6,9\},\{7,9\},\{7,10\},\{7,11\},\{8,10\},\{9,11\},\{\{1,2\},\{1,4\},\{1,6\},\{1,7\},$   
 $\{1,8\},\{1,9\},\{1,11\},\{2,3\},\{2,4\},\{2,5\},\{2,6\},\{2,8\},\{3,4\},\{3,5\},\{3,8\},$   
 $\{4,5\},\{4,8\},\{4,10\},\{4,11\},\{5,6\},\{5,7\},\{5,8\},\{5,9\},\{5,10\},\{6,7\},\{6,10\},$   
 $\{6,11\},\{7,9\},\{7,10\},\{7,11\},\{8,9\},\{10,11\},\{\{1,2\},\{1,4\},\{1,6\},\{1,7\},$   
 $\{1,9\},\{2,3\},\{2,4\},\{2,6\},\{2,7\},\{3,4\},\{3,5\},\{3,6\},\{3,7\},\{3,8\},\{3,10\},$   
 $\{4,5\},\{4,6\},\{4,7\},\{4,9\},\{5,6\},\{5,7\},\{5,8\},\{5,11\},\{6,7\},\{6,9\},\{6,10\},$   
 $\{6,11\},\{7,8\},\{7,9\},\{7,10\},\{7,11\},\{8,10\},\{8,11\},\{10,11\},\{\{1,2\},\{1,3\},$   
 $\{1,5\},\{1,10\},\{2,3\},\{2,5\},\{2,7\},\{2,9\},\{2,10\},\{2,11\},\{3,4\},\{3,5\},\{3,6\},$   
 $\{3,7\},\{3,10\},\{3,11\},\{4,5\},\{4,6\},\{4,7\},\{4,8\},\{4,10\},\{5,6\},\{5,7\},\{5,8\},$   
 $\{5,9\},\{5,10\},\{6,7\},\{7,8\},\{7,9\},\{7,10\},\{7,11\},\{8,10\},\{9,10\},\{10,11\},$   
 $\{\{1,2\},\{1,4\},\{1,5\},\{1,7\},\{1,8\},\{1,10\},\{1,11\},\{2,3\},\{2,4\},\{2,5\},\{2,6\},$   
 $\{2,7\},\{2,9\},\{2,11\},\{3,4\},\{3,6\},\{3,7\},\{3,9\},\{4,5\},\{4,6\},\{4,7\},\{4,8\},$   
 $\{4,9\},\{4,10\},\{4,11\},\{5,7\},\{5,9\},\{5,10\},\{6,7\},\{7,8\},\{7,9\},\{7,10\},$   
 $\{7,11\},\{8,10\},\{\{1,2\},\{1,3\},\{1,4\},\{1,6\},\{1,7\},\{1,9\},\{2,3\},\{2,4\},\{2,5\},$   
 $\{2,6\},\{2,7\},\{2,8\},\{2,9\},\{2,10\},\{2,11\},\{3,4\},\{3,7\},\{3,8\},\{4,7\},\{4,8\},$   
 $\{4,9\},\{5,6\},\{5,7\},\{5,9\},\{5,10\},\{5,11\},\{6,7\},\{6,9\},\{6,10\},\{6,11\},\{7,8\},$   
 $\{7,9\},\{7,11\},\{10,11\},\{\{1,2\},\{1,4\},\{1,5\},\{1,6\},\{1,7\},\{1,8\},\{1,9\},$   
 $\{2,4\},\{2,6\},\{2,7\},\{2,11\},\{3,4\},\{3,5\},\{3,7\},\{3,10\},\{4,5\},\{4,6\},\{4,7\},$   
 $\{4,8\},\{4,9\},\{4,10\},\{4,11\},\{5,6\},\{5,7\},\{5,8\},\{5,10\},\{6,7\},\{6,8\},\{6,9\},$   
 $\{6,10\},\{6,11\},\{7,10\},\{7,11\},\{8,9\},\{\{1,2\},\{1,3\},\{1,4\},\{1,5\},\{1,6\},$   
 $\{1,7\},\{1,8\},\{1,9\},\{1,10\},\{1,11\},\{2,4\},\{2,6\},\{2,8\},\{2,10\},\{2,11\},\{3,6\},$   
 $\{3,8\},\{3,10\},\{4,5\},\{4,6\},\{4,11\},\{5,6\},\{5,11\},\{6,7\},\{6,8\},\{6,9\},\{6,10\},$   
 $\{6,11\},\{7,9\},\{7,10\},\{8,10\},\{9,10\},\{9,11\},\{10,11\},\{\{1,2\},\{1,4\},\{1,6\},$   
 $\{1,8\},\{1,9\},\{1,11\},\{2,3\},\{2,4\},\{2,6\},\{2,7\},\{2,9\},\{3,4\},\{3,5\},\{3,7\},$   
 $\{3,10\},\{4,5\},\{4,6\},\{4,10\},\{4,11\},\{5,7\},\{5,8\},\{5,9\},\{5,10\},\{5,11\},$   
 $\{6,7\},\{6,9\},\{6,10\},\{7,9\},\{7,10\},\{8,9\},\{8,11\},\{\{1,2\},\{1,4\},\{1,5\},$   
 $\{1,6\},\{1,7\},\{1,8\},\{1,11\},\{2,3\},\{2,4\},\{2,6\},\{2,9\},\{3,4\},\{3,5\},\{3,6\},$   
 $\{3,9\},\{4,5\},\{4,7\},\{4,9\},\{5,6\},\{5,7\},\{5,8\},\{5,11\},\{6,9\},\{6,10\},\{6,11\},$   
 $\{7,8\},\{7,9\},\{8,9\},\{8,10\},\{8,11\},\{9,10\},\{10,11\},\{\{1,2\},\{1,3\},\{1,4\},$   
 $\{1,5\},\{1,6\},\{1,7\},\{1,8\},\{1,9\},\{1,10\},\{2,7\},\{2,8\},\{2,9\},\{2,11\},\{3,4\},$   
 $\{3,6\},\{3,7\},\{3,10\},\{4,5\},\{4,6\},\{4,7\},\{4,8\},\{4,9\},\{4,10\},\{4,11\},\{5,6\},$

{5,10},{6,7},{6,9},{6,10},{7,8},{7,9},{7,11},{8,11},{9,11}},{{1,2},  
{1,3},{1,4},{1,5},{1,6},{1,10},{1,11},{2,4},{2,6},{2,9},{2,10},{2,11},  
{3,4},{3,5},{3,6},{3,7},{3,10},{4,5},{4,6},{4,7},{4,8},{4,9},{4,10},  
{4,11},{5,6},{5,7},{5,8},{6,7},{6,8},{6,9},{6,10},{6,11},{7,8},  
{9,10}},{{1,2},{1,4},{1,5},{1,6},{1,7},{1,8},{1,9},{1,11},{2,3},{2,4},  
{2,5},{2,6},{2,8},{2,10},{3,4},{3,5},{3,8},{3,10},{4,5},{4,8},{4,10},  
{5,6},{5,7},{5,8},{5,9},{6,7},{6,8},{6,9},{6,11},{7,8},{7,9},{7,11},  
{8,10},{9,11}},{{1,2},{1,3},{1,4},{1,5},{1,8},{1,10},{1,11},{2,3},  
{2,4},{2,5},{2,6},{2,7},{2,8},{2,9},{2,11},{3,4},{3,5},{3,6},{3,7},  
{3,8},{3,9},{3,10},{4,5},{4,6},{4,8},{4,10},{4,11},{5,6},{5,7},{5,9},  
{5,10},{5,11},{6,9},{7,9}},{{1,2},{1,3},{1,4},{1,5},{1,6},{1,11},  
{2,4},{2,5},{2,6},{3,4},{3,5},{3,6},{3,8},{3,11},{4,5},{4,6},{4,7},  
{4,8},{4,9},{4,10},{4,11},{5,6},{5,7},{5,8},{5,9},{5,10},{6,7},{6,8},  
{6,11},{7,8},{7,9},{7,10},{8,10},{9,10}},{{1,2},{1,4},{1,5},{1,6},  
{1,7},{1,9},{1,10},{1,11},{2,5},{2,7},{2,10},{2,11},{3,4},{3,5},{3,6},  
{3,7},{3,8},{3,9},{3,10},{4,6},{4,7},{4,8},{4,9},{5,6},{5,7},{5,10},  
{6,8},{6,9},{7,10},{7,11},{8,9},{9,10},{10,11}},{{1,2},{1,3},{1,4},  
{1,5},{1,7},{1,9},{2,4},{2,6},{2,8},{2,9},{2,11},{3,4},{3,5},{3,7},  
{3,9},{3,10},{3,11},{4,5},{4,6},{4,7},{4,8},{4,11},{5,6},{5,7},{5,9},  
{6,8},{6,9},{6,11},{8,11},{9,10},{9,11},{10,11}},{{1,2},{1,4},{1,8},  
{1,9},{2,4},{2,5},{2,6},{2,8},{2,9},{2,10},{2,11},{3,4},{3,5},{3,7},  
{3,8},{3,9},{4,5},{4,8},{4,9},{5,6},{5,7},{5,8},{5,9},{6,8},{6,9},  
{6,10},{6,11},{7,8},{7,9},{8,9},{8,11},{9,10},{9,11},{10,11}},{{1,2},  
{1,5},{1,10},{1,11},{2,3},{2,5},{2,7},{2,9},{2,10},{2,11},{3,4},{3,5},  
{3,6},{3,7},{3,8},{3,9},{3,10},{3,11},{4,5},{4,6},{4,7},{4,8},{4,10},  
{5,6},{5,7},{5,10},{5,11},{6,7},{7,8},{7,9},{7,10},{8,10},{9,10},  
{10,11}},{{1,2},{1,3},{1,4},{1,5},{1,7},{1,8},{1,10},{1,11},{2,5},  
{2,6},{2,7},{2,8},{2,9},{3,4},{3,5},{3,8},{3,10},{3,11},{4,5},{4,10},  
{5,6},{5,7},{5,8},{5,9},{5,10},{5,11},{6,7},{6,9},{7,8},{7,9},{7,10},  
{8,9},{8,10},{8,11}},{{1,2},{1,3},{1,5},{1,7},{1,11},{2,3},{2,4},  
{2,5},{2,6},{2,7},{2,8},{2,9},{2,10},{2,11},{3,4},{3,5},{3,6},{3,7},  
{3,10},{3,11},{4,5},{4,11},{5,6},{5,7},{5,8},{5,9},{5,10},{5,11},  
{6,10},{7,8},{7,9},{7,10},{8,9},{9,10}},{{1,2},{1,5},{1,9},{1,10},  
{2,4},{2,5},{2,9},{2,10},{3,4},{3,5},{3,7},{3,8},{3,9},{4,5},{4,6},  
{4,7},{4,9},{4,10},{5,6},{5,7},{5,8},{5,9},{5,10},{5,11},{6,7},{6,10},  
{7,8},{7,9},{7,10},{7,11},{8,9},{9,10},{9,11},{10,11}},{{1,2},{1,3},  
{1,4},{1,5},{1,6},{1,7},{1,8},{1,9},{2,5},{2,9},{2,10},{2,11},{3,4},  
{3,6},{3,7},{3,8},{3,9},{4,5},{4,7},{4,8},{4,9},{4,10},{5,8},{5,10},  
{5,11},{6,8},{6,9},{7,8},{8,9},{8,11},{9,10},{9,11},{10,11}},{{1,2},  
{1,3},{1,6},{1,8},{1,10},{2,3},{2,5},{2,6},{2,7},{2,9},{2,10},{3,4},  
{3,5},{3,7},{3,8},{4,5},{4,6},{4,7},{4,8},{4,9},{4,11},{5,7},{5,9},  
{6,7},{6,8},{6,10},{6,11},{7,11},{8,9},{8,10},{9,10}},{{1,2},{1,3},  
{1,4},{1,6},{1,11},{2,3},{2,4},{2,5},{2,6},{2,9},{3,4},{3,7},{3,9},  
{3,10},{4,5},{4,10},{4,11},{5,6},{5,7},{5,8},{5,10},{5,11},{6,7},  
{6,9},{6,11},{7,8},{7,9},{7,10},{8,10},{10,11}},{{1,2},{1,3},{1,4},  
{1,5},{1,6},{1,7},{1,8},{1,9},{1,10},{1,11},{2,4},{2,5},{2,6},{2,8},  
{2,10},{3,4},{3,5},{3,8},{3,11},{4,5},{4,6},{4,8},{5,6},{5,7},{5,8},  
{5,9},{5,10},{5,11},{7,8},{7,9},{8,9},{8,10},{8,11},{9,11}},{{1,2},  
{1,3},{1,5},{1,7},{1,8},{1,10},{1,11},{2,3},{2,5},{2,6},{2,8},{2,9},  
{2,10},{3,4},{3,5},{3,7},{3,8},{3,10},{4,6},{4,7},{4,8},{4,11},{5,8},



$\{6,7\}, \{6,8\}, \{6,9\}, \{6,10\}, \{6,11\}, \{7,10\}, \{7,11\}, \{8,11\}, \{9,10\}, \{\{1,2\},$   
 $\{1,6\}, \{1,7\}, \{1,8\}, \{1,11\}, \{2,3\}, \{2,4\}, \{2,5\}, \{2,6\}, \{2,7\}, \{2,8\}, \{2,9\},$   
 $\{2,11\}, \{3,4\}, \{3,6\}, \{3,8\}, \{3,11\}, \{4,5\}, \{4,6\}, \{4,7\}, \{4,9\}, \{4,10\}, \{4,11\},$   
 $\{5,6\}, \{5,7\}, \{5,9\}, \{5,10\}, \{6,7\}, \{6,8\}, \{7,9\}, \{7,10\}, \{7,11\}, \{8,11\},$   
 $\{9,10\}\}, \{\{1,2\}, \{1,3\}, \{1,4\}, \{1,5\}, \{1,6\}, \{1,8\}, \{1,9\}, \{1,10\}, \{1,11\},$   
 $\{2,3\}, \{2,4\}, \{2,8\}, \{2,11\}, \{3,4\}, \{3,8\}, \{4,5\}, \{4,8\}, \{4,11\}, \{5,6\}, \{5,7\},$   
 $\{5,8\}, \{5,9\}, \{5,11\}, \{6,9\}, \{6,11\}, \{7,8\}, \{7,9\}, \{7,11\}, \{8,9\}, \{8,10\},$   
 $\{8,11\}, \{9,10\}, \{9,11\}, \{10,11\}\}, \{\{1,2\}, \{1,3\}, \{1,5\}, \{1,6\}, \{1,7\}, \{1,8\},$   
 $\{1,9\}, \{2,3\}, \{2,4\}, \{2,6\}, \{2,7\}, \{2,8\}, \{2,10\}, \{3,4\}, \{3,5\}, \{3,9\}, \{3,10\},$   
 $\{3,11\}, \{4,5\}, \{4,6\}, \{4,10\}, \{4,11\}, \{5,6\}, \{5,9\}, \{5,11\}, \{6,7\}, \{6,8\}, \{7,8\},$   
 $\{7,9\}, \{7,10\}, \{9,10\}\}, \{\{1,2\}, \{1,3\}, \{1,5\}, \{1,8\}, \{1,10\}, \{1,11\}, \{2,3\},$   
 $\{2,10\}, \{2,11\}, \{3,4\}, \{3,5\}, \{3,6\}, \{3,8\}, \{3,10\}, \{3,11\}, \{4,5\}, \{4,6\}, \{4,7\},$   
 $\{4,8\}, \{4,10\}, \{5,6\}, \{5,7\}, \{5,8\}, \{5,9\}, \{5,10\}, \{6,7\}, \{6,8\}, \{6,9\}, \{7,8\},$   
 $\{7,9\}, \{8,9\}, \{8,10\}, \{8,11\}, \{10,11\}\}, \{\{1,2\}, \{1,3\}, \{1,4\}, \{1,6\}, \{2,3\},$   
 $\{2,4\}, \{2,6\}, \{2,7\}, \{2,8\}, \{3,4\}, \{3,5\}, \{3,6\}, \{3,7\}, \{3,8\}, \{3,10\}, \{4,5\},$   
 $\{4,6\}, \{4,7\}, \{4,9\}, \{4,10\}, \{4,11\}, \{5,6\}, \{5,7\}, \{5,9\}, \{5,10\}, \{5,11\}, \{6,7\},$   
 $\{6,8\}, \{7,8\}, \{7,9\}, \{7,10\}, \{7,11\}, \{9,11\}, \{10,11\}\}, \{\{1,2\}, \{1,5\}, \{1,6\},$   
 $\{1,7\}, \{1,10\}, \{1,11\}, \{2,6\}, \{2,7\}, \{2,8\}, \{2,9\}, \{2,11\}, \{3,4\}, \{3,5\}, \{3,7\},$   
 $\{3,8\}, \{4,5\}, \{4,6\}, \{4,7\}, \{4,8\}, \{4,10\}, \{5,7\}, \{5,8\}, \{5,10\}, \{6,7\}, \{6,10\},$   
 $\{6,11\}, \{7,8\}, \{7,9\}, \{8,9\}, \{8,10\}, \{8,11\}, \{10,11\}\}, \{\{1,2\}, \{1,4\}, \{1,5\},$   
 $\{1,7\}, \{1,9\}, \{1,10\}, \{1,11\}, \{2,5\}, \{2,9\}, \{2,11\}, \{3,4\}, \{3,5\}, \{3,6\}, \{3,8\},$   
 $\{3,9\}, \{4,5\}, \{4,7\}, \{4,8\}, \{4,9\}, \{4,10\}, \{5,6\}, \{5,7\}, \{5,8\}, \{5,9\}, \{5,10\},$   
 $\{5,11\}, \{6,8\}, \{6,9\}, \{7,9\}, \{7,11\}, \{8,9\}, \{8,10\}, \{9,10\}, \{9,11\}\}, \{\{1,2\},$   
 $\{1,5\}, \{1,6\}, \{1,7\}, \{1,8\}, \{2,5\}, \{2,7\}, \{2,8\}, \{3,4\}, \{3,5\}, \{3,6\}, \{3,8\},$   
 $\{3,9\}, \{4,5\}, \{4,8\}, \{4,9\}, \{4,10\}, \{4,11\}, \{5,6\}, \{5,7\}, \{5,8\}, \{5,11\}, \{6,7\},$   
 $\{6,8\}, \{6,9\}, \{7,8\}, \{7,9\}, \{7,10\}, \{7,11\}, \{8,10\}, \{9,10\}, \{9,11\}, \{10,11\}\},$   
 $\{\{1,2\}, \{1,4\}, \{1,5\}, \{1,7\}, \{1,11\}, \{2,3\}, \{2,5\}, \{2,6\}, \{2,8\}, \{2,10\}, \{2,11\},$   
 $\{3,7\}, \{3,8\}, \{3,9\}, \{3,10\}, \{3,11\}, \{4,5\}, \{4,7\}, \{4,9\}, \{4,10\}, \{5,6\}, \{5,7\},$   
 $\{5,10\}, \{6,7\}, \{6,8\}, \{6,10\}, \{7,8\}, \{7,9\}, \{7,11\}, \{8,10\}, \{9,10\}, \{9,11\}\},$   
 $\{\{1,2\}, \{1,4\}, \{1,5\}, \{1,6\}, \{1,7\}, \{1,9\}, \{2,3\}, \{2,6\}, \{2,8\}, \{2,9\}, \{2,10\},$   
 $\{3,4\}, \{3,5\}, \{3,6\}, \{3,8\}, \{3,10\}, \{4,5\}, \{4,7\}, \{4,9\}, \{4,10\}, \{4,11\}, \{5,6\},$   
 $\{6,7\}, \{6,8\}, \{7,8\}, \{7,9\}, \{7,10\}, \{7,11\}, \{8,10\}, \{9,10\}, \{9,11\}, \{10,11\}\},$   
 $\{\{1,2\}, \{1,3\}, \{1,5\}, \{1,7\}, \{1,8\}, \{1,9\}, \{1,10\}, \{2,3\}, \{2,4\}, \{2,5\}, \{2,6\},$   
 $\{2,7\}, \{3,4\}, \{3,5\}, \{3,10\}, \{4,6\}, \{4,7\}, \{4,8\}, \{4,10\}, \{4,11\}, \{5,6\}, \{5,8\},$   
 $\{5,9\}, \{5,10\}, \{6,7\}, \{6,8\}, \{7,8\}, \{8,9\}, \{8,10\}, \{8,11\}, \{9,10\}, \{10,11\}\},$   
 $\{\{1,2\}, \{1,3\}, \{1,4\}, \{1,9\}, \{1,10\}, \{2,3\}, \{2,4\}, \{2,6\}, \{2,7\}, \{2,9\}, \{2,10\},$   
 $\{2,11\}, \{3,4\}, \{3,6\}, \{3,7\}, \{3,8\}, \{3,10\}, \{4,5\}, \{4,6\}, \{4,7\}, \{4,9\}, \{4,10\},$   
 $\{5,6\}, \{5,7\}, \{5,8\}, \{5,11\}, \{6,8\}, \{6,11\}, \{7,8\}, \{7,10\}, \{7,11\}, \{8,11\},$   
 $\{9,10\}\}, \{\{1,2\}, \{1,3\}, \{1,4\}, \{1,5\}, \{1,7\}, \{1,8\}, \{2,5\}, \{2,6\}, \{2,7\}, \{2,8\},$   
 $\{2,10\}, \{2,11\}, \{3,4\}, \{3,5\}, \{3,7\}, \{3,9\}, \{3,11\}, \{4,8\}, \{4,9\}, \{4,11\}, \{5,7\},$   
 $\{5,11\}, \{6,7\}, \{6,9\}, \{6,10\}, \{7,9\}, \{8,9\}, \{8,10\}, \{8,11\}, \{9,10\}, \{9,11\}\},$   
 $\{\{1,2\}, \{1,3\}, \{1,4\}, \{1,5\}, \{1,6\}, \{1,7\}, \{1,8\}, \{1,9\}, \{1,10\}, \{1,11\}, \{2,5\},$   
 $\{2,9\}, \{2,10\}, \{3,4\}, \{3,8\}, \{3,11\}, \{4,5\}, \{4,6\}, \{4,8\}, \{4,9\}, \{4,11\}, \{5,7\},$   
 $\{5,9\}, \{5,10\}, \{5,11\}, \{6,8\}, \{6,9\}, \{7,10\}, \{7,11\}, \{8,9\}, \{8,11\}, \{9,10\},$   
 $\{9,11\}, \{10,11\}\}, \{\{1,2\}, \{1,3\}, \{1,5\}, \{1,6\}, \{1,7\}, \{1,8\}, \{2,3\}, \{2,4\},$   
 $\{2,5\}, \{2,6\}, \{2,7\}, \{2,8\}, \{2,9\}, \{2,10\}, \{2,11\}, \{3,4\}, \{3,5\}, \{3,6\}, \{3,7\},$   
 $\{3,8\}, \{3,9\}, \{3,10\}, \{3,11\}, \{4,8\}, \{4,9\}, \{4,11\}, \{5,6\}, \{5,7\}, \{5,10\}, \{7,8\},$   
 $\{7,10\}, \{7,11\}, \{8,9\}, \{8,11\}\}, \{\{1,2\}, \{1,3\}, \{1,4\}, \{1,8\}, \{1,9\}, \{1,10\},$   
 $\{2,3\}, \{2,6\}, \{2,8\}, \{2,9\}, \{3,4\}, \{3,5\}, \{3,6\}, \{3,7\}, \{3,8\}, \{3,10\}, \{3,11\},$   
 $\{4,5\}, \{4,6\}, \{4,7\}, \{4,8\}, \{4,9\}, \{4,10\}, \{4,11\}, \{5,6\}, \{5,8\}, \{6,8\}, \{6,9\},$

$\{7,8\},\{7,10\},\{7,11\},\{8,9\},\{8,10\},\{8,11\},\{\{1,2\},\{1,4\},\{1,9\},\{1,10\},$   
 $\{2,3\},\{2,4\},\{2,6\},\{2,7\},\{2,8\},\{2,9\},\{2,10\},\{2,11\},\{3,4\},\{3,8\},\{3,9\},$   
 $\{3,10\},\{4,5\},\{4,6\},\{4,8\},\{4,9\},\{4,10\},\{4,11\},\{5,6\},\{5,7\},\{5,10\},$   
 $\{5,11\},\{6,7\},\{6,8\},\{6,10\},\{6,11\},\{7,10\},\{7,11\},\{8,10\},\{9,10\},\{\{1,2\},$   
 $\{1,3\},\{1,4\},\{1,5\},\{1,6\},\{1,7\},\{1,8\},\{1,9\},\{1,10\},\{1,11\},\{2,3\},\{2,6\},$   
 $\{2,7\},\{2,8\},\{3,4\},\{3,6\},\{3,7\},\{4,6\},\{4,7\},\{4,10\},\{5,6\},\{5,7\},\{5,10\},$   
 $\{5,11\},\{6,8\},\{6,9\},\{6,10\},\{6,11\},\{7,8\},\{7,9\},\{7,10\},\{7,11\},\{8,9\},$   
 $\{9,11\},\{\{1,2\},\{1,5\},\{1,6\},\{1,7\},\{1,8\},\{2,3\},\{2,4\},\{2,5\},\{2,6\},\{2,7\},$   
 $\{2,8\},\{2,9\},\{2,10\},\{2,11\},\{3,4\},\{3,7\},\{3,8\},\{3,9\},\{3,11\},\{4,7\},\{4,8\},$   
 $\{4,11\},\{5,7\},\{5,8\},\{5,9\},\{5,10\},\{6,7\},\{6,8\},\{7,8\},\{7,9\},\{8,9\},\{8,10\},$   
 $\{8,11\},\{9,10\},\{\{1,2\},\{1,3\},\{1,4\},\{1,5\},\{1,8\},\{1,10\},\{2,3\},\{2,5\},$   
 $\{2,9\},\{3,4\},\{3,6\},\{3,8\},\{3,9\},\{4,6\},\{4,8\},\{4,10\},\{4,11\},\{5,6\},\{5,7\},$   
 $\{5,9\},\{5,10\},\{5,11\},\{6,7\},\{6,9\},\{6,11\},\{7,8\},\{7,9\},\{7,11\},\{8,9\},$   
 $\{8,11\},\{10,11\},\{\{1,2\},\{1,5\},\{1,6\},\{1,10\},\{1,11\},\{2,3\},\{2,5\},\{2,9\},$   
 $\{2,11\},\{3,7\},\{3,9\},\{3,11\},\{4,5\},\{4,6\},\{4,7\},\{4,8\},\{4,10\},\{5,6\},\{5,8\},$   
 $\{5,9\},\{6,8\},\{6,10\},\{6,11\},\{7,8\},\{7,9\},\{7,10\},\{7,11\},\{8,9\},\{8,11\},$   
 $\{10,11\},\{\{1,2\},\{1,5\},\{1,7\},\{1,9\},\{2,3\},\{2,5\},\{2,7\},\{2,9\},\{2,11\},$   
 $\{3,4\},\{3,8\},\{3,9\},\{3,10\},\{3,11\},\{4,6\},\{4,8\},\{4,9\},\{4,10\},\{5,6\},\{5,7\},$   
 $\{5,9\},\{5,11\},\{6,8\},\{6,9\},\{6,11\},\{7,9\},\{7,10\},\{7,11\},\{8,10\},\{8,11\},$   
 $\{9,10\},\{10,11\},\{\{1,2\},\{1,5\},\{1,6\},\{1,8\},\{1,9\},\{1,11\},\{2,3\},\{2,4\},$   
 $\{2,5\},\{2,7\},\{2,9\},\{3,4\},\{3,7\},\{3,9\},\{3,10\},\{4,5\},\{4,7\},\{4,10\},\{5,6\},$   
 $\{5,7\},\{5,8\},\{5,10\},\{6,8\},\{6,10\},\{6,11\},\{7,8\},\{7,9\},\{8,9\},\{8,11\},$   
 $\{9,10\},\{9,11\},\{10,11\},\{\{1,2\},\{1,3\},\{1,4\},\{1,5\},\{1,6\},\{1,7\},\{1,8\},$   
 $\{1,9\},\{1,10\},\{1,11\},\{2,3\},\{2,4\},\{2,5\},\{2,6\},\{2,7\},\{2,10\},\{2,11\},\{3,5\},$   
 $\{3,6\},\{3,10\},\{4,5\},\{4,7\},\{4,8\},\{4,9\},\{4,11\},\{5,6\},\{5,7\},\{5,8\},\{5,10\},$   
 $\{8,9\},\{8,10\},\{8,11\},\{9,11\},\{10,11\},\{\{1,2\},\{1,3\},\{1,4\},\{1,5\},\{1,6\},$   
 $\{1,8\},\{2,3\},\{2,4\},\{2,5\},\{2,6\},\{2,11\},\{3,4\},\{3,5\},\{3,7\},\{3,8\},\{3,9\},$   
 $\{3,10\},\{4,5\},\{4,6\},\{4,7\},\{4,8\},\{4,9\},\{4,10\},\{4,11\},\{5,6\},\{5,8\},\{5,9\},$   
 $\{5,11\},\{6,11\},\{7,8\},\{7,9\},\{7,10\},\{8,9\},\{8,10\},\{\{1,2\},\{1,3\},\{1,6\},$   
 $\{1,9\},\{2,3\},\{2,4\},\{2,5\},\{2,6\},\{2,8\},\{2,9\},\{3,4\},\{3,5\},\{3,6\},\{3,7\},$   
 $\{3,9\},\{3,10\},\{4,5\},\{4,6\},\{4,7\},\{4,9\},\{4,11\},\{5,8\},\{5,10\},\{5,11\},\{6,9\},$   
 $\{7,8\},\{7,9\},\{7,10\},\{7,11\},\{8,9\},\{8,10\},\{8,11\},\{10,11\},\{\{1,2\},\{1,3\},$   
 $\{1,4\},\{1,5\},\{1,6\},\{1,7\},\{1,8\},\{1,9\},\{1,10\},\{1,11\},\{2,5\},\{2,6\},\{2,7\},$   
 $\{2,8\},\{2,9\},\{2,10\},\{3,4\},\{3,7\},\{3,8\},\{3,10\},\{3,11\},\{4,7\},\{4,10\},\{5,6\},$   
 $\{5,7\},\{5,9\},\{6,7\},\{6,8\},\{6,9\},\{7,8\},\{7,10\},\{7,11\},\{8,10\},\{8,11\},$   
 $\{\{1,2\},\{1,6\},\{1,7\},\{1,11\},\{2,3\},\{2,5\},\{2,6\},\{2,7\},\{2,8\},\{2,11\},\{3,4\},$   
 $\{3,5\},\{3,8\},\{3,9\},\{4,5\},\{4,6\},\{4,8\},\{4,9\},\{5,6\},\{5,7\},\{5,9\},\{6,7\},$   
 $\{6,8\},\{6,11\},\{7,8\},\{7,9\},\{7,10\},\{7,11\},\{8,9\},\{8,10\},\{8,11\},\{9,10\},$   
 $\{\{1,2\},\{1,3\},\{1,4\},\{1,5\},\{1,6\},\{1,7\},\{1,8\},\{1,9\},\{1,10\},\{2,3\},\{2,4\},$   
 $\{2,5\},\{2,7\},\{2,8\},\{2,9\},\{2,10\},\{2,11\},\{3,4\},\{3,5\},\{3,6\},\{3,9\},\{4,6\},$   
 $\{4,9\},\{5,7\},\{5,8\},\{5,9\},\{6,9\},\{7,8\},\{7,10\},\{7,11\},\{8,9\},\{8,10\},\{8,11\},$   
 $\{10,11\},\{\{1,2\},\{1,3\},\{1,4\},\{1,7\},\{1,8\},\{1,10\},\{1,11\},\{2,5\},\{2,6\},$   
 $\{2,7\},\{2,8\},\{2,9\},\{2,10\},\{3,4\},\{3,5\},\{3,10\},\{3,11\},\{4,5\},\{4,7\},\{4,11\},$   
 $\{5,7\},\{5,9\},\{5,10\},\{5,11\},\{6,7\},\{6,8\},\{6,9\},\{7,8\},\{7,9\},\{8,9\},\{8,11\},$   
 $\{9,11\},\{\{1,2\},\{1,3\},\{1,5\},\{1,6\},\{1,8\},\{1,10\},\{1,11\},\{2,4\},\{2,6\},$   
 $\{2,7\},\{2,10\},\{3,4\},\{3,5\},\{3,8\},\{3,9\},\{3,10\},\{3,11\},\{4,5\},\{4,6\},\{4,7\},$   
 $\{4,9\},\{4,10\},\{5,6\},\{5,7\},\{5,8\},\{6,7\},\{7,8\},\{7,10\},\{7,11\},\{8,11\},$   
 $\{9,10\},\{10,11\},\{\{1,2\},\{1,3\},\{1,5\},\{1,6\},\{1,7\},\{1,8\},\{1,10\},\{2,3\},$   
 $\{2,4\},\{2,5\},\{2,7\},\{2,8\},\{2,9\},\{3,4\},\{3,6\},\{3,7\},\{3,8\},\{3,9\},\{3,10\},$   
 $\{3,11\},\{4,5\},\{4,6\},\{4,7\},\{4,9\},\{4,11\},\{5,6\},\{5,7\},\{6,7\},\{6,10\},\{6,11\},$

$\{7,8\},\{7,9\},\{7,10\},\{7,11\},\{\{1,2\},\{1,7\},\{1,8\},\{1,10\},\{2,4\},\{2,5\},$   
 $\{2,6\},\{2,7\},\{2,8\},\{2,10\},\{3,4\},\{3,5\},\{3,6\},\{3,9\},\{3,10\},\{3,11\},\{4,5\},$   
 $\{4,7\},\{4,8\},\{4,9\},\{5,6\},\{5,7\},\{5,11\},\{6,10\},\{6,11\},\{7,8\},\{7,10\},$   
 $\{7,11\},\{8,9\},\{8,10\},\{9,10\},\{10,11\},\{\{1,2\},\{1,3\},\{1,5\},\{1,7\},\{1,8\},$   
 $\{1,10\},\{2,3\},\{2,10\},\{3,6\},\{3,8\},\{3,9\},\{3,10\},\{3,11\},\{4,5\},\{4,6\},\{4,7\},$   
 $\{4,8\},\{4,9\},\{5,6\},\{5,7\},\{5,9\},\{5,10\},\{5,11\},\{6,8\},\{6,10\},\{6,11\},\{7,8\},$   
 $\{7,9\},\{8,9\},\{9,11\},\{10,11\},\{\{1,2\},\{1,4\},\{1,5\},\{1,6\},\{1,7\},\{1,8\},$   
 $\{1,9\},\{1,11\},\{2,3\},\{2,4\},\{2,5\},\{2,6\},\{2,7\},\{2,8\},\{2,10\},\{3,6\},\{3,7\},$   
 $\{3,8\},\{3,9\},\{4,5\},\{4,7\},\{4,8\},\{4,10\},\{4,11\},\{5,10\},\{5,11\},\{6,7\},\{6,9\},$   
 $\{7,8\},\{7,9\},\{8,9\},\{8,10\},\{8,11\},\{10,11\},\{\{1,2\},\{1,3\},\{1,4\},\{1,6\},$   
 $\{1,8\},\{1,9\},\{1,10\},\{1,11\},\{2,4\},\{2,5\},\{2,7\},\{2,9\},\{3,4\},\{3,7\},\{3,8\},$   
 $\{3,10\},\{4,5\},\{4,7\},\{4,8\},\{5,6\},\{5,7\},\{5,8\},\{5,9\},\{6,8\},\{6,9\},\{6,10\},$   
 $\{6,11\},\{7,9\},\{7,10\},\{9,10\},\{9,11\},\{10,11\},\{\{1,2\},\{1,5\},\{1,7\},\{1,8\},$   
 $\{1,9\},\{1,10\},\{1,11\},\{2,3\},\{2,4\},\{2,5\},\{2,6\},\{2,11\},\{3,4\},\{3,5\},\{3,6\},$   
 $\{3,8\},\{3,9\},\{3,10\},\{4,6\},\{4,7\},\{4,8\},\{4,11\},\{5,10\},\{6,7\},\{6,9\},\{7,8\},$   
 $\{7,9\},\{7,11\},\{8,9\},\{9,10\},\{\{1,2\},\{1,5\},\{1,6\},\{1,7\},\{1,9\},\{2,5\},\{2,6\},$   
 $\{2,7\},\{2,8\},\{2,9\},\{2,10\},\{2,11\},\{3,4\},\{3,5\},\{3,6\},\{3,7\},\{3,11\},\{4,5\},$   
 $\{4,7\},\{4,11\},\{5,6\},\{5,7\},\{5,8\},\{5,9\},\{5,10\},\{5,11\},\{6,7\},\{6,9\},\{6,10\},$   
 $\{6,11\},\{7,8\},\{7,11\},\{8,11\},\{10,11\},\{\{1,2\},\{1,3\},\{1,4\},\{1,5\},\{1,6\},$   
 $\{1,7\},\{1,8\},\{1,11\},\{2,4\},\{2,6\},\{2,8\},\{2,9\},\{2,10\},\{3,4\},\{3,6\},\{3,7\},$   
 $\{4,5\},\{4,6\},\{4,7\},\{4,10\},\{5,7\},\{5,8\},\{5,9\},\{5,10\},\{5,11\},\{6,7\},\{6,9\},$   
 $\{7,9\},\{8,9\},\{8,10\},\{8,11\},\{9,10\},\{\{1,2\},\{1,6\},\{1,7\},\{1,8\},\{1,9\},$   
 $\{1,10\},\{2,3\},\{2,4\},\{2,5\},\{2,6\},\{2,7\},\{2,8\},\{2,9\},\{2,10\},\{2,11\},\{3,4\},$   
 $\{3,5\},\{3,7\},\{3,8\},\{4,5\},\{4,7\},\{5,6\},\{5,7\},\{5,8\},\{6,7\},\{6,8\},\{6,9\},$   
 $\{6,10\},\{6,11\},\{7,8\},\{7,9\},\{9,10\},\{9,11\},\{10,11\},\{\{1,2\},\{1,3\},\{1,7\},$   
 $\{1,8\},\{1,10\},\{2,3\},\{2,4\},\{2,8\},\{2,9\},\{2,10\},\{3,4\},\{3,7\},\{3,8\},\{4,5\},$   
 $\{4,6\},\{4,7\},\{4,9\},\{4,10\},\{4,11\},\{5,6\},\{5,7\},\{5,10\},\{5,11\},\{6,7\},\{6,8\},$   
 $\{6,9\},\{6,10\},\{6,11\},\{7,8\},\{7,10\},\{8,9\},\{9,10\},\{10,11\},\{\{1,2\},\{1,3\},$   
 $\{1,5\},\{1,7\},\{1,8\},\{1,9\},\{1,11\},\{2,3\},\{2,4\},\{2,5\},\{2,6\},\{2,9\},\{2,10\},$   
 $\{3,4\},\{3,5\},\{3,6\},\{3,10\},\{3,11\},\{4,6\},\{4,7\},\{4,10\},\{5,6\},\{5,7\},\{6,7\},$   
 $\{7,8\},\{7,10\},\{7,11\},\{8,9\},\{8,10\},\{8,11\},\{9,10\},\{10,11\},\{\{1,2\},\{1,3\},$   
 $\{1,4\},\{1,6\},\{1,9\},\{1,10\},\{2,3\},\{2,5\},\{2,10\},\{3,4\},\{3,5\},\{3,7\},\{4,6\},$   
 $\{4,7\},\{4,8\},\{4,10\},\{4,11\},\{5,7\},\{5,9\},\{5,10\},\{5,11\},\{6,7\},\{6,8\},\{6,9\},$   
 $\{6,11\},\{7,8\},\{7,11\},\{8,11\},\{9,10\},\{9,11\},\{10,11\},\{\{1,2\},\{1,3\},\{1,4\},$   
 $\{1,11\},\{2,3\},\{2,4\},\{2,7\},\{2,11\},\{3,4\},\{3,7\},\{3,8\},\{3,11\},\{4,5\},\{4,6\},$   
 $\{4,7\},\{4,8\},\{4,9\},\{4,10\},\{4,11\},\{5,6\},\{5,7\},\{5,11\},\{6,7\},\{6,9\},\{6,10\},$   
 $\{6,11\},\{7,8\},\{7,9\},\{7,11\},\{8,9\},\{8,11\},\{9,10\},\{9,11\},\{10,11\},\{\{1,2\},$   
 $\{1,3\},\{1,4\},\{1,7\},\{1,11\},\{2,3\},\{2,4\},\{2,5\},\{2,7\},\{2,8\},\{3,4\},\{3,6\},$   
 $\{3,8\},\{3,9\},\{3,10\},\{3,11\},\{4,5\},\{4,6\},\{4,7\},\{5,6\},\{5,7\},\{5,8\},\{5,9\},$   
 $\{5,11\},\{6,9\},\{6,10\},\{7,11\},\{8,9\},\{8,11\},\{9,10\},\{9,11\},\{\{1,2\},\{1,3\},$   
 $\{1,6\},\{1,8\},\{1,11\},\{2,3\},\{2,5\},\{2,6\},\{2,8\},\{3,4\},\{3,5\},\{3,6\},\{3,7\},$   
 $\{3,10\},\{3,11\},\{4,5\},\{4,6\},\{4,8\},\{4,9\},\{4,10\},\{5,8\},\{5,9\},\{5,10\},\{6,8\},$   
 $\{7,10\},\{7,11\},\{8,9\},\{8,11\},\{9,10\},\{9,11\},\{10,11\},\{\{1,2\},\{1,3\},\{1,5\},$   
 $\{1,7\},\{1,9\},\{1,10\},\{2,7\},\{2,8\},\{2,10\},\{3,4\},\{3,5\},\{3,7\},\{3,8\},\{3,9\},$   
 $\{3,11\},\{4,6\},\{4,8\},\{4,9\},\{4,10\},\{4,11\},\{5,6\},\{5,9\},\{5,11\},\{6,9\},$   
 $\{6,10\},\{6,11\},\{7,8\},\{8,10\},\{8,11\},\{9,10\},\{\{1,2\},\{1,4\},\{1,5\},\{1,7\},$   
 $\{1,8\},\{1,9\},\{1,10\},\{1,11\},\{2,7\},\{2,9\},\{2,10\},\{3,4\},\{3,5\},\{3,6\},\{3,10\},$   
 $\{3,11\},\{4,5\},\{4,6\},\{4,11\},\{5,6\},\{5,8\},\{5,9\},\{5,10\},\{6,9\},\{6,11\},\{7,8\},$   
 $\{7,9\},\{7,10\},\{8,9\},\{8,10\},\{9,10\},\{9,11\},\{10,11\},\{\{1,2\},\{1,5\},\{1,6\},$   
 $\{1,9\},\{2,4\},\{2,5\},\{2,6\},\{2,7\},\{2,9\},\{2,10\},\{2,11\},\{3,4\},\{3,6\},\{3,7\},$

$\{3,8\}, \{3,9\}, \{3,10\}, \{3,11\}, \{4,7\}, \{4,9\}, \{4,11\}, \{5,6\}, \{5,9\}, \{6,7\}, \{6,8\},$   
 $\{6,9\}, \{6,10\}, \{7,8\}, \{7,10\}, \{8,10\}, \{9,11\}, \{10,11\}, \{\{1,2\}, \{1,6\}, \{1,7\},$   
 $\{1,8\}, \{1,9\}, \{1,10\}, \{2,3\}, \{2,4\}, \{2,7\}, \{2,8\}, \{2,9\}, \{2,11\}, \{3,4\}, \{3,5\},$   
 $\{3,6\}, \{3,8\}, \{3,11\}, \{4,5\}, \{4,9\}, \{4,11\}, \{5,6\}, \{5,9\}, \{5,11\}, \{6,8\}, \{6,9\},$   
 $\{6,10\}, \{6,11\}, \{7,8\}, \{7,10\}, \{7,11\}, \{8,10\}, \{10,11\}, \{\{1,2\}, \{1,3\}, \{1,4\},$   
 $\{1,5\}, \{1,8\}, \{1,9\}, \{2,3\}, \{2,4\}, \{2,5\}, \{2,6\}, \{2,7\}, \{2,11\}, \{3,6\}, \{3,9\},$   
 $\{4,5\}, \{4,7\}, \{4,8\}, \{4,9\}, \{5,8\}, \{5,9\}, \{5,10\}, \{5,11\}, \{6,7\}, \{6,9\}, \{6,11\},$   
 $\{7,9\}, \{7,11\}, \{8,9\}, \{9,10\}, \{9,11\}, \{10,11\}, \{\{1,2\}, \{1,5\}, \{1,6\}, \{1,8\},$   
 $\{1,9\}, \{1,10\}, \{2,3\}, \{2,5\}, \{2,6\}, \{2,7\}, \{2,8\}, \{2,11\}, \{3,4\}, \{3,5\}, \{3,6\},$   
 $\{3,7\}, \{3,8\}, \{3,9\}, \{3,10\}, \{3,11\}, \{4,5\}, \{4,10\}, \{5,6\}, \{5,7\}, \{5,10\}, \{6,7\},$   
 $\{6,9\}, \{6,11\}, \{7,11\}, \{8,9\}, \{8,10\}, \{9,10\}, \{\{1,2\}, \{1,5\}, \{1,6\}, \{1,10\},$   
 $\{1,11\}, \{2,3\}, \{2,4\}, \{2,6\}, \{2,7\}, \{2,8\}, \{2,10\}, \{3,4\}, \{3,6\}, \{3,7\}, \{3,8\},$   
 $\{3,9\}, \{4,6\}, \{4,8\}, \{5,6\}, \{5,9\}, \{5,10\}, \{5,11\}, \{6,8\}, \{6,9\}, \{6,11\}, \{7,8\},$   
 $\{7,9\}, \{7,10\}, \{7,11\}, \{8,11\}, \{9,10\}, \{10,11\}, \{\{1,2\}, \{1,3\}, \{1,4\}, \{1,5\},$   
 $\{1,6\}, \{1,7\}, \{1,9\}, \{1,10\}, \{1,11\}, \{2,4\}, \{2,5\}, \{2,6\}, \{2,7\}, \{2,8\}, \{2,9\},$   
 $\{2,10\}, \{2,11\}, \{3,5\}, \{3,6\}, \{3,7\}, \{3,8\}, \{4,7\}, \{4,9\}, \{4,10\}, \{4,11\}, \{5,6\},$   
 $\{5,7\}, \{5,8\}, \{5,9\}, \{6,8\}, \{7,8\}, \{7,9\}, \{7,10\}, \{10,11\}, \{\{1,2\}, \{1,4\},$   
 $\{1,5\}, \{1,6\}, \{1,9\}, \{2,5\}, \{2,7\}, \{2,8\}, \{2,9\}, \{2,10\}, \{3,4\}, \{3,6\}, \{3,7\},$   
 $\{3,9\}, \{3,10\}, \{3,11\}, \{4,5\}, \{4,6\}, \{4,7\}, \{5,6\}, \{5,7\}, \{5,8\}, \{5,10\}, \{6,9\},$   
 $\{6,10\}, \{7,8\}, \{7,10\}, \{7,11\}, \{8,10\}, \{9,10\}, \{10,11\}, \{\{1,2\}, \{1,3\}, \{1,5\},$   
 $\{1,7\}, \{1,9\}, \{2,3\}, \{2,4\}, \{2,5\}, \{2,6\}, \{2,9\}, \{2,10\}, \{3,6\}, \{3,7\}, \{3,8\},$   
 $\{3,9\}, \{3,11\}, \{4,5\}, \{4,6\}, \{4,10\}, \{5,6\}, \{5,7\}, \{5,8\}, \{5,10\}, \{6,8\}, \{6,10\},$   
 $\{7,8\}, \{7,9\}, \{7,10\}, \{7,11\}, \{8,10\}, \{8,11\}, \{9,10\}, \{\{1,2\}, \{1,3\}, \{1,7\},$   
 $\{1,8\}, \{1,9\}, \{1,10\}, \{2,3\}, \{2,4\}, \{2,5\}, \{2,6\}, \{2,7\}, \{2,8\}, \{2,9\}, \{2,10\},$   
 $\{2,11\}, \{3,7\}, \{3,8\}, \{4,5\}, \{4,6\}, \{4,7\}, \{4,9\}, \{4,10\}, \{4,11\}, \{5,6\}, \{5,7\},$   
 $\{5,11\}, \{6,7\}, \{6,10\}, \{7,8\}, \{7,9\}, \{7,10\}, \{7,11\}, \{8,9\}, \{9,10\}, \{\{1,2\},$   
 $\{1,5\}, \{1,6\}, \{1,8\}, \{1,10\}, \{2,3\}, \{2,5\}, \{2,6\}, \{2,7\}, \{2,10\}, \{3,4\}, \{3,5\},$   
 $\{3,7\}, \{3,8\}, \{3,9\}, \{3,10\}, \{4,5\}, \{4,6\}, \{4,7\}, \{4,8\}, \{4,9\}, \{4,11\}, \{5,7\},$   
 $\{5,8\}, \{5,9\}, \{6,7\}, \{6,8\}, \{6,10\}, \{6,11\}, \{7,9\}, \{8,10\}, \{8,11\}, \{\{1,2\},$   
 $\{1,3\}, \{1,4\}, \{1,8\}, \{1,9\}, \{2,4\}, \{2,6\}, \{2,8\}, \{2,9\}, \{3,4\}, \{3,5\}, \{3,6\},$   
 $\{3,7\}, \{3,8\}, \{3,11\}, \{4,5\}, \{4,6\}, \{4,9\}, \{4,10\}, \{5,6\}, \{5,7\}, \{5,8\}, \{5,9\},$   
 $\{5,10\}, \{6,7\}, \{6,8\}, \{6,11\}, \{7,8\}, \{7,11\}, \{8,9\}, \{8,11\}, \{9,10\}, \{\{1,2\},$   
 $\{1,3\}, \{1,5\}, \{1,6\}, \{1,7\}, \{1,9\}, \{2,3\}, \{2,4\}, \{2,5\}, \{2,7\}, \{2,9\}, \{3,5\},$   
 $\{3,7\}, \{3,9\}, \{3,11\}, \{4,5\}, \{4,6\}, \{4,7\}, \{4,8\}, \{4,10\}, \{5,6\}, \{5,8\}, \{5,9\},$   
 $\{5,10\}, \{5,11\}, \{6,7\}, \{6,8\}, \{6,10\}, \{7,10\}, \{7,11\}, \{8,10\}, \{10,11\}, \{\{1,2\},$   
 $\{1,3\}, \{1,4\}, \{1,5\}, \{1,7\}, \{1,8\}, \{1,9\}, \{1,10\}, \{1,11\}, \{2,3\}, \{2,6\}, \{2,8\},$   
 $\{2,9\}, \{3,6\}, \{3,7\}, \{3,8\}, \{4,5\}, \{4,6\}, \{4,8\}, \{4,9\}, \{4,10\}, \{4,11\}, \{5,6\},$   
 $\{5,7\}, \{5,9\}, \{6,7\}, \{6,8\}, \{6,9\}, \{8,10\}, \{8,11\}, \{10,11\}, \{\{1,2\}, \{1,6\},$   
 $\{1,7\}, \{1,8\}, \{1,9\}, \{1,10\}, \{1,11\}, \{2,3\}, \{2,4\}, \{2,5\}, \{2,6\}, \{2,7\}, \{2,9\},$   
 $\{3,4\}, \{3,5\}, \{3,6\}, \{3,8\}, \{3,9\}, \{4,5\}, \{4,6\}, \{4,7\}, \{4,10\}, \{4,11\}, \{5,6\},$   
 $\{6,8\}, \{6,10\}, \{7,9\}, \{7,11\}, \{8,9\}, \{8,10\}, \{10,11\}, \{\{1,2\}, \{1,4\}, \{1,6\},$   
 $\{1,10\}, \{2,3\}, \{2,4\}, \{2,5\}, \{2,6\}, \{2,7\}, \{2,10\}, \{3,4\}, \{3,5\}, \{3,6\}, \{3,8\},$   
 $\{3,10\}, \{3,11\}, \{4,6\}, \{4,7\}, \{4,10\}, \{4,11\}, \{5,7\}, \{5,8\}, \{5,11\}, \{6,10\},$   
 $\{7,8\}, \{7,9\}, \{7,10\}, \{7,11\}, \{8,9\}, \{8,10\}, \{8,11\}, \{9,10\}, \{\{1,2\}, \{1,3\},$   
 $\{1,6\}, \{1,7\}, \{1,8\}, \{1,9\}, \{1,10\}, \{1,11\}, \{2,4\}, \{2,5\}, \{2,7\}, \{2,9\}, \{2,11\},$   
 $\{3,4\}, \{3,6\}, \{3,10\}, \{3,11\}, \{4,5\}, \{4,6\}, \{4,10\}, \{4,11\}, \{5,6\}, \{5,7\}, \{5,8\},$   
 $\{5,9\}, \{5,10\}, \{6,9\}, \{7,8\}, \{7,9\}, \{8,10\}, \{10,11\}, \{\{1,2\}, \{1,5\}, \{1,6\},$   
 $\{1,8\}, \{2,3\}, \{2,5\}, \{2,6\}, \{2,7\}, \{2,8\}, \{3,4\}, \{3,5\}, \{3,7\}, \{3,10\}, \{3,11\},$   
 $\{4,5\}, \{4,6\}, \{4,7\}, \{4,10\}, \{4,11\}, \{5,6\}, \{5,8\}, \{5,9\}, \{5,10\}, \{5,11\}, \{6,7\},$   
 $\{6,8\}, \{7,8\}, \{7,10\}, \{8,9\}, \{8,10\}, \{9,10\}, \{10,11\}, \{\{1,2\}, \{1,3\}, \{1,5\},$

$\{1,6\}, \{1,7\}, \{1,9\}, \{2,3\}, \{2,4\}, \{2,6\}, \{2,8\}, \{2,10\}, \{3,4\}, \{3,5\}, \{3,7\},$   
 $\{3,9\}, \{3,10\}, \{4,7\}, \{4,8\}, \{4,10\}, \{5,6\}, \{5,7\}, \{5,9\}, \{5,10\}, \{6,7\}, \{6,8\},$   
 $\{6,10\}, \{6,11\}, \{7,8\}, \{7,9\}, \{7,11\}, \{8,10\}, \{8,11\}, \{\{1,2\}, \{1,3\}, \{1,4\},$   
 $\{1,5\}, \{1,6\}, \{1,8\}, \{2,4\}, \{2,6\}, \{2,9\}, \{2,11\}, \{3,4\}, \{3,5\}, \{3,6\}, \{3,7\},$   
 $\{3,8\}, \{3,10\}, \{4,10\}, \{4,11\}, \{5,6\}, \{5,8\}, \{5,9\}, \{5,10\}, \{6,7\}, \{6,8\}, \{6,9\},$   
 $\{7,9\}, \{7,10\}, \{7,11\}, \{9,10\}, \{9,11\}, \{10,11\}, \{\{1,2\}, \{1,4\}, \{1,7\}, \{1,8\},$   
 $\{2,4\}, \{2,7\}, \{2,8\}, \{3,4\}, \{3,6\}, \{3,7\}, \{3,9\}, \{3,10\}, \{3,11\}, \{4,7\}, \{4,8\},$   
 $\{4,9\}, \{4,10\}, \{5,6\}, \{5,7\}, \{5,8\}, \{5,9\}, \{5,11\}, \{6,7\}, \{6,8\}, \{6,11\}, \{7,8\},$   
 $\{7,9\}, \{8,10\}, \{8,11\}, \{9,10\}, \{9,11\}, \{10,11\}, \{\{1,2\}, \{1,3\}, \{1,4\}, \{1,5\},$   
 $\{1,7\}, \{1,8\}, \{1,9\}, \{2,5\}, \{2,7\}, \{2,8\}, \{2,9\}, \{2,10\}, \{2,11\}, \{3,4\}, \{3,7\},$   
 $\{3,9\}, \{4,6\}, \{4,7\}, \{4,8\}, \{4,9\}, \{4,10\}, \{5,7\}, \{5,8\}, \{6,7\}, \{6,8\}, \{6,10\},$   
 $\{7,8\}, \{7,9\}, \{7,10\}, \{7,11\}, \{8,10\}, \{9,10\}, \{9,11\}, \{10,11\}, \{\{1,2\}, \{1,3\},$   
 $\{1,6\}, \{1,9\}, \{1,10\}, \{1,11\}, \{2,7\}, \{2,8\}, \{2,9\}, \{2,10\}, \{2,11\}, \{3,6\},$   
 $\{3,10\}, \{4,5\}, \{4,6\}, \{4,7\}, \{4,8\}, \{4,9\}, \{4,11\}, \{5,6\}, \{5,7\}, \{5,9\}, \{6,7\},$   
 $\{6,8\}, \{6,9\}, \{6,10\}, \{7,8\}, \{7,9\}, \{8,10\}, \{8,11\}, \{9,11\}, \{10,11\}, \{\{1,2\},$   
 $\{1,4\}, \{1,5\}, \{1,6\}, \{1,7\}, \{1,10\}, \{2,3\}, \{2,5\}, \{2,7\}, \{2,10\}, \{2,11\}, \{3,4\},$   
 $\{3,7\}, \{3,8\}, \{3,9\}, \{3,10\}, \{3,11\}, \{4,5\}, \{4,6\}, \{4,7\}, \{4,8\}, \{4,9\}, \{4,10\},$   
 $\{5,9\}, \{5,10\}, \{5,11\}, \{6,7\}, \{7,9\}, \{7,11\}, \{8,10\}, \{9,11\}, \{\{1,2\}, \{1,3\},$   
 $\{1,5\}, \{1,6\}, \{1,7\}, \{2,3\}, \{2,5\}, \{2,6\}, \{2,8\}, \{3,4\}, \{3,5\}, \{3,6\}, \{3,9\},$   
 $\{3,11\}, \{4,5\}, \{4,9\}, \{4,11\}, \{5,7\}, \{5,8\}, \{5,9\}, \{5,10\}, \{5,11\}, \{6,7\}, \{6,8\},$   
 $\{6,9\}, \{7,8\}, \{7,9\}, \{7,10\}, \{8,9\}, \{8,10\}, \{9,10\}, \{9,11\}, \{\{1,2\}, \{1,3\},$   
 $\{1,5\}, \{1,6\}, \{1,8\}, \{1,10\}, \{1,11\}, \{2,3\}, \{2,4\}, \{2,5\}, \{2,7\}, \{2,9\}, \{2,10\},$   
 $\{2,11\}, \{3,4\}, \{3,7\}, \{3,8\}, \{3,11\}, \{4,7\}, \{4,8\}, \{4,9\}, \{5,6\}, \{5,7\}, \{5,10\},$   
 $\{6,7\}, \{6,8\}, \{6,10\}, \{7,8\}, \{8,9\}, \{8,10\}, \{9,10\}, \{\{1,2\}, \{1,4\}, \{1,5\},$   
 $\{1,6\}, \{1,7\}, \{2,4\}, \{2,5\}, \{2,6\}, \{2,11\}, \{3,4\}, \{3,6\}, \{3,7\}, \{3,8\}, \{3,11\},$   
 $\{4,5\}, \{4,7\}, \{4,11\}, \{5,7\}, \{5,8\}, \{5,9\}, \{5,10\}, \{5,11\}, \{6,7\}, \{6,8\}, \{6,11\},$   
 $\{7,8\}, \{7,9\}, \{7,10\}, \{8,9\}, \{8,10\}, \{8,11\}, \{9,10\}, \{\{1,2\}, \{1,8\}, \{1,11\},$   
 $\{2,3\}, \{2,6\}, \{2,8\}, \{2,10\}, \{2,11\}, \{3,4\}, \{3,5\}, \{3,6\}, \{3,8\}, \{4,5\}, \{4,6\},$   
 $\{4,7\}, \{4,10\}, \{5,6\}, \{5,7\}, \{5,8\}, \{5,9\}, \{6,9\}, \{6,10\}, \{6,11\}, \{7,8\}, \{7,9\},$   
 $\{7,10\}, \{7,11\}, \{8,9\}, \{8,11\}, \{9,11\}, \{10,11\}, \{\{1,2\}, \{1,5\}, \{1,6\}, \{1,8\},$   
 $\{1,9\}, \{1,11\}, \{2,5\}, \{2,7\}, \{2,8\}, \{2,9\}, \{2,11\}, \{3,4\}, \{3,5\}, \{3,7\}, \{3,10\},$   
 $\{4,5\}, \{4,6\}, \{4,7\}, \{4,9\}, \{4,10\}, \{5,6\}, \{5,7\}, \{5,10\}, \{5,11\}, \{6,9\}, \{7,9\},$   
 $\{7,10\}, \{8,9\}, \{8,11\}, \{9,10\}, \{9,11\}, \{10,11\}, \{\{1,2\}, \{1,3\}, \{1,4\}, \{1,6\},$   
 $\{1,7\}, \{1,8\}, \{2,4\}, \{2,6\}, \{2,9\}, \{2,10\}, \{3,4\}, \{3,5\}, \{3,6\}, \{3,7\}, \{3,8\},$   
 $\{3,10\}, \{4,7\}, \{4,9\}, \{4,10\}, \{5,6\}, \{5,10\}, \{6,8\}, \{6,9\}, \{6,10\}, \{6,11\},$   
 $\{7,8\}, \{7,9\}, \{7,11\}, \{8,11\}, \{9,10\}, \{9,11\}, \{\{1,2\}, \{1,3\}, \{1,4\}, \{1,5\},$   
 $\{1,9\}, \{1,10\}, \{2,5\}, \{2,6\}, \{2,8\}, \{2,9\}, \{2,10\}, \{2,11\}, \{3,4\}, \{3,5\}, \{3,6\},$   
 $\{3,7\}, \{3,10\}, \{4,7\}, \{4,8\}, \{4,9\}, \{5,6\}, \{5,9\}, \{6,8\}, \{6,11\}, \{7,8\}, \{7,10\},$   
 $\{7,11\}, \{8,9\}, \{8,11\}, \{10,11\}, \{\{1,2\}, \{1,5\}, \{1,6\}, \{1,7\}, \{1,8\}, \{1,9\},$   
 $\{2,5\}, \{2,8\}, \{2,9\}, \{3,4\}, \{3,5\}, \{3,6\}, \{3,10\}, \{3,11\}, \{4,6\}, \{4,8\}, \{4,10\},$   
 $\{4,11\}, \{5,6\}, \{5,8\}, \{5,9\}, \{5,10\}, \{6,7\}, \{6,8\}, \{6,11\}, \{7,9\}, \{7,10\},$   
 $\{7,11\}, \{8,9\}, \{8,10\}, \{9,10\}, \{10,11\}, \{\{1,2\}, \{1,6\}, \{1,7\}, \{1,9\}, \{1,10\},$   
 $\{1,11\}, \{2,3\}, \{2,4\}, \{2,5\}, \{2,7\}, \{2,8\}, \{2,10\}, \{2,11\}, \{3,4\}, \{3,6\}, \{3,7\},$   
 $\{3,8\}, \{3,10\}, \{4,5\}, \{4,6\}, \{4,7\}, \{5,6\}, \{5,9\}, \{5,11\}, \{6,7\}, \{6,9\}, \{6,10\},$   
 $\{8,10\}, \{9,10\}, \{9,11\}, \{10,11\}, \{\{1,2\}, \{1,3\}, \{1,4\}, \{1,9\}, \{1,11\}, \{2,4\},$   
 $\{2,5\}, \{2,6\}, \{2,9\}, \{2,11\}, \{3,4\}, \{3,8\}, \{3,10\}, \{3,11\}, \{4,5\}, \{4,6\}, \{4,7\},$   
 $\{4,8\}, \{5,6\}, \{5,7\}, \{5,11\}, \{6,7\}, \{6,9\}, \{6,10\}, \{7,8\}, \{7,10\}, \{7,11\},$   
 $\{8,10\}, \{9,10\}, \{9,11\}, \{10,11\}, \{\{1,2\}, \{1,3\}, \{1,5\}, \{1,6\}, \{1,8\}, \{1,10\},$   
 $\{2,3\}, \{2,4\}, \{2,5\}, \{2,7\}, \{2,9\}, \{2,10\}, \{3,8\}, \{3,9\}, \{3,10\}, \{4,5\}, \{4,6\},$   
 $\{4,7\}, \{4,10\}, \{5,6\}, \{5,7\}, \{6,7\}, \{6,8\}, \{6,10\}, \{6,11\}, \{7,8\}, \{7,9\}, \{7,11\},$

$\{8,9\}, \{8,10\}, \{8,11\}, \{1,2\}, \{1,5\}, \{1,8\}, \{1,10\}, \{1,11\}, \{2,3\}, \{2,7\},$   
 $\{2,8\}, \{2,10\}, \{2,11\}, \{3,4\}, \{3,6\}, \{3,7\}, \{3,8\}, \{3,9\}, \{3,10\}, \{4,5\}, \{4,6\},$   
 $\{4,7\}, \{4,8\}, \{4,9\}, \{4,10\}, \{5,7\}, \{5,8\}, \{5,10\}, \{5,11\}, \{6,7\}, \{6,8\}, \{7,8\},$   
 $\{7,11\}, \{9,10\}, \{10,11\}, \{1,2\}, \{1,4\}, \{1,5\}, \{1,6\}, \{1,7\}, \{1,8\}, \{1,9\},$   
 $\{2,3\}, \{2,4\}, \{2,7\}, \{2,10\}, \{3,4\}, \{3,7\}, \{3,10\}, \{3,11\}, \{4,5\}, \{4,6\}, \{4,8\},$   
 $\{4,9\}, \{4,10\}, \{4,11\}, \{5,6\}, \{5,9\}, \{6,7\}, \{6,8\}, \{6,9\}, \{6,10\}, \{7,8\}, \{7,10\},$   
 $\{7,11\}, \{8,9\}, \{8,11\}, \{1,2\}, \{1,4\}, \{1,5\}, \{1,6\}, \{1,7\}, \{1,8\}, \{1,9\},$   
 $\{1,11\}, \{2,5\}, \{2,6\}, \{2,9\}, \{2,10\}, \{3,4\}, \{3,5\}, \{3,6\}, \{3,7\}, \{3,8\}, \{3,9\},$   
 $\{3,10\}, \{3,11\}, \{4,7\}, \{4,9\}, \{5,6\}, \{5,8\}, \{5,10\}, \{6,10\}, \{6,11\}, \{7,8\},$   
 $\{7,11\}, \{8,11\}, \{9,10\}, \{1,2\}, \{1,3\}, \{1,6\}, \{1,8\}, \{2,6\}, \{2,7\}, \{2,8\},$   
 $\{2,10\}, \{2,11\}, \{3,4\}, \{3,5\}, \{3,6\}, \{3,8\}, \{3,9\}, \{4,5\}, \{4,6\}, \{4,7\}, \{4,9\},$   
 $\{5,6\}, \{5,9\}, \{5,10\}, \{5,11\}, \{6,7\}, \{6,11\}, \{7,8\}, \{7,9\}, \{7,10\}, \{8,9\},$   
 $\{8,10\}, \{9,10\}, \{10,11\}, \{1,2\}, \{1,5\}, \{1,6\}, \{1,7\}, \{1,9\}, \{1,10\}, \{2,3\},$   
 $\{2,6\}, \{2,7\}, \{2,8\}, \{2,10\}, \{3,4\}, \{3,6\}, \{3,8\}, \{3,10\}, \{4,5\}, \{4,6\}, \{4,7\},$   
 $\{4,8\}, \{4,9\}, \{4,11\}, \{5,6\}, \{5,7\}, \{5,11\}, \{6,11\}, \{7,8\}, \{7,9\}, \{8,9\}, \{8,10\},$   
 $\{9,10\}, \{1,2\}, \{1,3\}, \{1,4\}, \{1,5\}, \{1,6\}, \{1,7\}, \{1,8\}, \{1,10\}, \{2,3\}, \{2,4\},$   
 $\{2,9\}, \{2,10\}, \{3,4\}, \{3,5\}, \{3,9\}, \{4,5\}, \{4,6\}, \{4,8\}, \{4,10\}, \{4,11\}, \{5,8\},$   
 $\{5,9\}, \{6,7\}, \{6,9\}, \{6,10\}, \{6,11\}, \{7,8\}, \{7,9\}, \{7,11\}, \{8,9\}, \{8,11\},$   
 $\{9,10\}, \{9,11\}, \{1,2\}, \{1,3\}, \{1,4\}, \{1,8\}, \{1,9\}, \{1,11\}, \{2,3\}, \{2,4\},$   
 $\{2,6\}, \{2,7\}, \{2,9\}, \{3,4\}, \{3,7\}, \{3,9\}, \{3,10\}, \{4,7\}, \{4,11\}, \{5,6\}, \{5,7\},$   
 $\{5,8\}, \{5,10\}, \{6,7\}, \{6,8\}, \{6,9\}, \{6,10\}, \{7,8\}, \{7,10\}, \{7,11\}, \{8,9\},$   
 $\{8,10\}, \{8,11\}, \{9,10\}, \{1,2\}, \{1,6\}, \{1,7\}, \{1,9\}, \{1,10\}, \{2,3\}, \{2,4\},$   
 $\{2,5\}, \{2,6\}, \{2,8\}, \{2,9\}, \{3,4\}, \{3,5\}, \{3,6\}, \{3,8\}, \{4,5\}, \{4,6\}, \{4,9\},$   
 $\{4,10\}, \{5,6\}, \{5,7\}, \{5,8\}, \{5,9\}, \{5,11\}, \{6,7\}, \{6,8\}, \{6,10\}, \{7,9\}, \{7,10\},$   
 $\{7,11\}, \{9,10\}, \{9,11\}, \{1,2\}, \{1,3\}, \{1,4\}, \{1,5\}, \{1,9\}, \{2,5\}, \{2,6\},$   
 $\{2,9\}, \{3,4\}, \{3,5\}, \{3,8\}, \{3,9\}, \{3,10\}, \{4,5\}, \{4,7\}, \{4,8\}, \{5,6\}, \{5,7\},$   
 $\{5,10\}, \{6,7\}, \{6,9\}, \{6,10\}, \{7,8\}, \{7,10\}, \{7,11\}, \{8,9\}, \{8,11\}, \{9,10\},$   
 $\{9,11\}, \{10,11\}, \{1,2\}, \{1,3\}, \{1,5\}, \{1,6\}, \{1,10\}, \{1,11\}, \{2,5\}, \{2,7\},$   
 $\{2,8\}, \{2,9\}, \{2,10\}, \{3,4\}, \{3,5\}, \{3,6\}, \{3,8\}, \{3,10\}, \{3,11\}, \{4,5\}, \{4,8\},$   
 $\{5,6\}, \{5,7\}, \{5,8\}, \{5,9\}, \{6,7\}, \{6,10\}, \{6,11\}, \{7,8\}, \{7,9\}, \{7,10\}, \{8,9\},$   
 $\{8,10\}, \{10,11\}, \{1,2\}, \{1,6\}, \{1,7\}, \{1,9\}, \{1,10\}, \{1,11\}, \{2,6\}, \{2,8\},$   
 $\{2,10\}, \{3,4\}, \{3,5\}, \{3,6\}, \{3,7\}, \{3,8\}, \{3,9\}, \{3,11\}, \{4,8\}, \{4,9\}, \{4,10\},$   
 $\{4,11\}, \{5,6\}, \{5,11\}, \{6,7\}, \{6,8\}, \{6,11\}, \{7,8\}, \{7,9\}, \{8,10\}, \{9,11\},$   
 $\{10,11\}, \{1,2\}, \{1,3\}, \{1,4\}, \{1,5\}, \{1,7\}, \{1,10\}, \{1,11\}, \{2,4\}, \{2,5\},$   
 $\{2,6\}, \{2,7\}, \{3,4\}, \{3,6\}, \{3,8\}, \{3,9\}, \{3,11\}, \{4,6\}, \{4,7\}, \{4,9\}, \{5,6\},$   
 $\{5,7\}, \{5,9\}, \{5,10\}, \{6,8\}, \{6,9\}, \{6,10\}, \{7,9\}, \{8,9\}, \{8,10\}, \{8,11\},$   
 $\{9,10\}, \{10,11\}, \{1,2\}, \{1,3\}, \{1,5\}, \{1,6\}, \{1,9\}, \{2,5\}, \{2,8\}, \{2,9\},$   
 $\{2,11\}, \{3,4\}, \{3,5\}, \{3,6\}, \{3,8\}, \{3,9\}, \{3,10\}, \{4,7\}, \{4,8\}, \{4,10\}, \{4,11\},$   
 $\{5,6\}, \{5,8\}, \{6,7\}, \{6,8\}, \{6,9\}, \{6,10\}, \{7,8\}, \{7,10\}, \{7,11\}, \{8,11\},$   
 $\{9,10\}, \{9,11\}, \{10,11\}, \{1,2\}, \{1,8\}, \{1,10\}, \{1,11\}, \{2,5\}, \{2,6\}, \{2,7\},$   
 $\{2,8\}, \{2,9\}, \{2,10\}, \{2,11\}, \{3,4\}, \{3,5\}, \{3,6\}, \{3,7\}, \{3,9\}, \{4,5\}, \{4,8\},$   
 $\{4,9\}, \{4,10\}, \{5,6\}, \{5,8\}, \{5,9\}, \{6,7\}, \{6,8\}, \{7,9\}, \{7,10\}, \{8,10\}, \{8,11\},$   
 $\{9,10\}, \{10,11\}, \{1,2\}, \{1,3\}, \{1,4\}, \{1,7\}, \{1,9\}, \{2,3\}, \{2,5\}, \{2,9\},$   
 $\{2,10\}, \{2,11\}, \{3,4\}, \{3,5\}, \{3,6\}, \{3,8\}, \{4,7\}, \{4,8\}, \{5,6\}, \{5,8\}, \{5,10\},$   
 $\{5,11\}, \{6,7\}, \{6,8\}, \{6,11\}, \{7,8\}, \{7,9\}, \{7,11\}, \{8,9\}, \{8,10\}, \{9,10\},$   
 $\{9,11\}, \{10,11\}, \{1,2\}, \{1,3\}, \{1,4\}, \{1,5\}, \{1,6\}, \{1,8\}, \{1,11\}, \{2,3\},$   
 $\{2,4\}, \{2,5\}, \{2,7\}, \{2,9\}, \{2,10\}, \{3,5\}, \{3,6\}, \{3,8\}, \{3,9\}, \{4,6\}, \{4,7\},$   
 $\{4,9\}, \{5,6\}, \{5,8\}, \{5,10\}, \{5,11\}, \{6,7\}, \{6,8\}, \{6,9\}, \{6,10\}, \{6,11\}, \{7,9\},$   
 $\{7,10\}, \{8,11\}, \{1,2\}, \{1,3\}, \{1,4\}, \{1,5\}, \{1,7\}, \{1,9\}, \{1,10\}, \{2,4\},$   
 $\{2,5\}, \{2,6\}, \{2,7\}, \{2,8\}, \{2,10\}, \{2,11\}, \{3,4\}, \{3,6\}, \{3,9\}, \{3,10\}, \{4,5\},$

$\{4,6\}, \{4,7\}, \{4,8\}, \{4,11\}, \{5,6\}, \{5,7\}, \{5,8\}, \{5,9\}, \{5,11\}, \{6,8\}, \{6,9\},$   
 $\{6,10\}, \{8,11\}, \{9,10\}\}, \{\{1,2\}, \{1,3\}, \{1,6\}, \{1,7\}, \{1,9\}, \{1,11\}, \{2,3\},$   
 $\{2,6\}, \{2,8\}, \{2,9\}, \{3,4\}, \{3,7\}, \{3,8\}, \{3,9\}, \{4,7\}, \{4,8\}, \{4,9\}, \{4,10\},$   
 $\{5,6\}, \{5,7\}, \{5,9\}, \{5,10\}, \{5,11\}, \{6,7\}, \{6,8\}, \{6,11\}, \{7,8\}, \{7,10\},$   
 $\{9,10\}, \{9,11\}\}, \{\{1,2\}, \{1,5\}, \{1,7\}, \{1,8\}, \{1,11\}, \{2,3\}, \{2,5\}, \{2,6\},$   
 $\{2,8\}, \{2,11\}, \{3,4\}, \{3,6\}, \{3,8\}, \{4,6\}, \{4,7\}, \{4,8\}, \{4,9\}, \{5,6\}, \{5,7\},$   
 $\{5,9\}, \{5,10\}, \{5,11\}, \{6,7\}, \{6,9\}, \{6,10\}, \{7,8\}, \{7,9\}, \{7,10\}, \{8,9\},$   
 $\{8,11\}, \{9,10\}, \{9,11\}\}, \{\{1,2\}, \{1,5\}, \{1,6\}, \{1,8\}, \{1,9\}, \{2,3\}, \{2,6\},$   
 $\{2,7\}, \{2,8\}, \{2,9\}, \{2,10\}, \{3,4\}, \{3,7\}, \{3,8\}, \{3,10\}, \{3,11\}, \{4,5\}, \{4,6\},$   
 $\{4,7\}, \{4,10\}, \{4,11\}, \{5,6\}, \{5,9\}, \{5,10\}, \{5,11\}, \{6,7\}, \{6,8\}, \{6,11\},$   
 $\{7,10\}, \{8,11\}, \{9,10\}\}, \{\{1,2\}, \{1,3\}, \{1,4\}, \{1,5\}, \{1,7\}, \{1,8\}, \{1,11\},$   
 $\{2,3\}, \{2,4\}, \{2,6\}, \{2,7\}, \{2,8\}, \{2,9\}, \{2,10\}, \{3,4\}, \{3,5\}, \{3,6\}, \{3,7\},$   
 $\{4,7\}, \{4,9\}, \{4,11\}, \{5,6\}, \{5,8\}, \{5,10\}, \{5,11\}, \{6,10\}, \{8,9\}, \{8,10\},$   
 $\{8,11\}, \{9,10\}, \{9,11\}\}, \{\{1,2\}, \{1,3\}, \{1,4\}, \{1,5\}, \{1,6\}, \{1,7\}, \{1,9\},$   
 $\{1,10\}, \{2,3\}, \{2,4\}, \{2,6\}, \{2,9\}, \{3,4\}, \{3,9\}, \{4,5\}, \{4,6\}, \{4,7\}, \{4,8\},$   
 $\{4,9\}, \{4,10\}, \{4,11\}, \{5,6\}, \{5,7\}, \{5,10\}, \{6,8\}, \{6,9\}, \{6,10\}, \{7,10\},$   
 $\{8,9\}, \{8,10\}, \{8,11\}, \{9,10\}, \{9,11\}, \{10,11\}\}, \{\{1,2\}, \{1,3\}, \{1,5\}, \{1,7\},$   
 $\{1,8\}, \{1,11\}, \{2,5\}, \{2,7\}, \{2,8\}, \{2,9\}, \{2,10\}, \{2,11\}, \{3,4\}, \{3,5\}, \{3,7\},$   
 $\{3,9\}, \{4,5\}, \{4,6\}, \{4,8\}, \{4,9\}, \{5,8\}, \{5,9\}, \{5,11\}, \{6,7\}, \{6,8\}, \{6,9\},$   
 $\{6,10\}, \{7,9\}, \{7,10\}, \{8,10\}, \{8,11\}\}, \{\{1,2\}, \{1,5\}, \{1,6\}, \{1,7\}, \{2,6\},$   
 $\{2,7\}, \{2,8\}, \{2,10\}, \{2,11\}, \{3,4\}, \{3,7\}, \{3,8\}, \{3,9\}, \{3,10\}, \{4,5\}, \{4,6\},$   
 $\{4,7\}, \{4,9\}, \{5,6\}, \{5,7\}, \{5,9\}, \{5,11\}, \{6,9\}, \{6,10\}, \{7,8\}, \{8,10\}, \{8,11\},$   
 $\{9,10\}, \{9,11\}, \{10,11\}\}, \{\{1,2\}, \{1,3\}, \{1,4\}, \{1,5\}, \{1,6\}, \{1,11\}, \{2,3\},$   
 $\{2,4\}, \{3,4\}, \{3,5\}, \{3,8\}, \{3,9\}, \{3,10\}, \{4,6\}, \{4,8\}, \{4,9\}, \{4,11\}, \{5,6\},$   
 $\{5,7\}, \{5,8\}, \{5,10\}, \{5,11\}, \{6,7\}, \{6,9\}, \{6,10\}, \{6,11\}, \{7,10\}, \{8,9\},$   
 $\{8,10\}, \{8,11\}, \{9,10\}\}, \{\{1,2\}, \{1,3\}, \{1,4\}, \{1,9\}, \{1,10\}, \{2,3\}, \{2,6\},$   
 $\{2,8\}, \{2,9\}, \{3,4\}, \{3,6\}, \{3,10\}, \{3,11\}, \{4,5\}, \{4,8\}, \{5,7\}, \{5,8\}, \{5,9\},$   
 $\{5,10\}, \{5,11\}, \{6,7\}, \{6,9\}, \{6,10\}, \{6,11\}, \{7,9\}, \{7,10\}, \{8,9\}, \{8,11\}\},$   
 $\{\{1,2\}, \{1,3\}, \{1,4\}, \{1,6\}, \{1,7\}, \{1,8\}, \{1,10\}, \{2,4\}, \{2,8\}, \{2,9\}, \{2,10\},$   
 $\{2,11\}, \{3,5\}, \{3,6\}, \{3,9\}, \{3,10\}, \{4,5\}, \{4,8\}, \{4,10\}, \{5,6\}, \{5,7\}, \{5,8\},$   
 $\{5,9\}, \{5,10\}, \{6,7\}, \{6,9\}, \{7,8\}, \{7,9\}, \{8,9\}, \{9,10\}, \{9,11\}, \{10,11\}\},$   
 $\{\{1,2\}, \{1,8\}, \{1,10\}, \{2,5\}, \{2,6\}, \{2,8\}, \{2,9\}, \{2,10\}, \{2,11\}, \{3,4\}, \{3,5\},$   
 $\{3,7\}, \{3,8\}, \{3,9\}, \{3,11\}, \{4,5\}, \{4,6\}, \{4,7\}, \{4,11\}, \{5,7\}, \{5,10\}, \{5,11\},$   
 $\{6,7\}, \{6,8\}, \{6,9\}, \{6,11\}, \{7,8\}, \{7,10\}, \{8,9\}, \{8,10\}, \{9,11\}\}, \{\{1,2\},$   
 $\{1,5\}, \{1,6\}, \{1,7\}, \{1,8\}, \{1,11\}, \{2,3\}, \{2,5\}, \{2,6\}, \{2,8\}, \{2,9\}, \{3,4\},$   
 $\{3,5\}, \{3,6\}, \{3,8\}, \{3,9\}, \{4,6\}, \{4,8\}, \{4,9\}, \{4,10\}, \{5,6\}, \{5,8\}, \{5,11\},$   
 $\{6,7\}, \{6,8\}, \{6,9\}, \{6,10\}, \{6,11\}, \{7,8\}, \{7,11\}, \{8,9\}, \{8,10\}, \{8,11\},$   
 $\{9,10\}\}, \{\{1,2\}, \{1,5\}, \{1,6\}, \{1,7\}, \{1,8\}, \{1,11\}, \{2,3\}, \{2,6\}, \{2,11\},$   
 $\{3,6\}, \{3,7\}, \{3,9\}, \{3,10\}, \{3,11\}, \{4,5\}, \{4,8\}, \{4,9\}, \{4,11\}, \{5,7\}, \{5,9\},$   
 $\{5,10\}, \{5,11\}, \{6,7\}, \{6,8\}, \{6,9\}, \{7,9\}, \{8,9\}, \{8,11\}, \{9,10\}, \{10,11\}\},$   
 $\{\{1,2\}, \{1,3\}, \{1,5\}, \{1,6\}, \{1,10\}, \{2,3\}, \{2,4\}, \{2,6\}, \{2,7\}, \{2,11\}, \{3,4\},$   
 $\{3,5\}, \{3,7\}, \{3,10\}, \{4,5\}, \{4,7\}, \{4,11\}, \{5,6\}, \{5,8\}, \{5,9\}, \{5,10\}, \{5,11\},$   
 $\{6,8\}, \{6,11\}, \{7,8\}, \{7,9\}, \{7,10\}, \{7,11\}, \{8,9\}, \{8,11\}, \{9,10\}\}, \{\{1,2\},$   
 $\{1,4\}, \{1,5\}, \{1,6\}, \{1,7\}, \{1,8\}, \{1,9\}, \{1,11\}, \{2,3\}, \{2,4\}, \{2,5\}, \{2,6\},$   
 $\{2,8\}, \{2,9\}, \{2,10\}, \{2,11\}, \{3,4\}, \{3,7\}, \{3,9\}, \{3,10\}, \{4,5\}, \{4,6\}, \{4,7\},$   
 $\{4,8\}, \{4,11\}, \{5,6\}, \{5,8\}, \{6,11\}, \{7,8\}, \{7,9\}, \{7,10\}, \{8,10\}, \{9,10\}\},$   
 $\{\{1,2\}, \{1,5\}, \{1,7\}, \{1,8\}, \{1,9\}, \{1,10\}, \{1,11\}, \{2,5\}, \{2,6\}, \{2,9\}, \{2,10\},$   
 $\{3,4\}, \{3,6\}, \{3,7\}, \{3,8\}, \{3,9\}, \{3,10\}, \{4,5\}, \{4,7\}, \{4,10\}, \{5,6\}, \{5,7\},$   
 $\{5,10\}, \{6,7\}, \{6,8\}, \{6,9\}, \{7,8\}, \{8,9\}, \{8,11\}, \{9,10\}, \{9,11\}\}, \{\{1,2\},$   
 $\{1,3\}, \{1,4\}, \{1,6\}, \{1,7\}, \{1,8\}, \{1,10\}, \{1,11\}, \{2,3\}, \{2,8\}, \{3,4\}, \{3,5\},$

$\{3,6\}, \{3,8\}, \{3,9\}, \{4,5\}, \{4,6\}, \{4,7\}, \{4,11\}, \{5,6\}, \{5,7\}, \{5,9\}, \{5,10\},$   
 $\{6,10\}, \{7,8\}, \{7,9\}, \{7,10\}, \{7,11\}, \{8,9\}, \{8,10\}, \{9,10\}, \{\{1,2\}, \{1,4\},$   
 $\{1,6\}, \{1,7\}, \{1,8\}, \{1,9\}, \{1,11\}, \{2,5\}, \{2,7\}, \{2,8\}, \{2,10\}, \{2,11\}, \{3,4\},$   
 $\{3,5\}, \{3,6\}, \{4,5\}, \{4,6\}, \{4,8\}, \{4,9\}, \{5,6\}, \{5,7\}, \{5,8\}, \{5,10\}, \{6,7\},$   
 $\{6,9\}, \{7,9\}, \{7,10\}, \{8,9\}, \{8,10\}, \{8,11\}, \{9,10\}, \{\{1,2\}, \{1,3\}, \{1,8\},$   
 $\{1,9\}, \{1,10\}, \{2,4\}, \{2,6\}, \{2,7\}, \{2,8\}, \{2,9\}, \{2,10\}, \{3,4\}, \{3,5\}, \{3,8\},$   
 $\{3,9\}, \{3,10\}, \{3,11\}, \{4,5\}, \{4,6\}, \{4,7\}, \{4,10\}, \{4,11\}, \{5,6\}, \{5,8\},$   
 $\{5,11\}, \{6,7\}, \{6,8\}, \{7,9\}, \{7,11\}, \{8,9\}, \{9,11\}, \{\{1,2\}, \{1,4\}, \{1,6\},$   
 $\{1,7\}, \{1,9\}, \{2,3\}, \{2,4\}, \{2,5\}, \{2,6\}, \{2,8\}, \{2,9\}, \{2,11\}, \{3,5\}, \{3,7\},$   
 $\{3,8\}, \{3,9\}, \{3,11\}, \{4,7\}, \{4,11\}, \{5,9\}, \{6,7\}, \{6,8\}, \{6,9\}, \{6,10\}, \{7,8\},$   
 $\{7,9\}, \{7,10\}, \{7,11\}, \{8,10\}, \{8,11\}, \{\{1,2\}, \{1,4\}, \{1,8\}, \{1,9\}, \{1,10\},$   
 $\{2,3\}, \{2,6\}, \{2,8\}, \{2,10\}, \{2,11\}, \{3,4\}, \{3,6\}, \{3,7\}, \{3,10\}, \{3,11\}, \{4,5\},$   
 $\{4,7\}, \{4,8\}, \{4,9\}, \{5,6\}, \{5,7\}, \{5,8\}, \{5,9\}, \{5,11\}, \{6,9\}, \{6,10\}, \{6,11\},$   
 $\{7,8\}, \{7,11\}, \{8,11\}, \{9,10\}, \{\{1,2\}, \{1,4\}, \{1,5\}, \{1,6\}, \{1,7\}, \{1,8\},$   
 $\{1,11\}, \{2,3\}, \{2,4\}, \{2,6\}, \{2,10\}, \{3,4\}, \{3,5\}, \{3,6\}, \{3,8\}, \{3,9\}, \{3,10\},$   
 $\{4,8\}, \{5,6\}, \{5,7\}, \{5,8\}, \{6,10\}, \{6,11\}, \{7,8\}, \{7,9\}, \{7,11\}, \{8,9\}, \{9,10\},$   
 $\{9,11\}, \{10,11\}, \{\{1,2\}, \{1,3\}, \{1,4\}, \{1,6\}, \{1,8\}, \{1,10\}, \{1,11\}, \{2,6\},$   
 $\{2,8\}, \{3,4\}, \{3,5\}, \{3,6\}, \{3,10\}, \{3,11\}, \{4,5\}, \{4,7\}, \{4,8\}, \{4,9\}, \{4,10\},$   
 $\{5,6\}, \{5,7\}, \{5,9\}, \{6,7\}, \{6,8\}, \{6,9\}, \{6,10\}, \{6,11\}, \{7,9\}, \{7,10\}, \{8,9\},$   
 $\{10,11\}, \{\{1,2\}, \{1,4\}, \{1,5\}, \{1,6\}, \{1,7\}, \{1,9\}, \{1,10\}, \{2,3\}, \{2,4\},$   
 $\{2,9\}, \{2,10\}, \{3,4\}, \{3,7\}, \{3,8\}, \{3,9\}, \{3,10\}, \{3,11\}, \{4,6\}, \{4,10\},$   
 $\{4,11\}, \{5,6\}, \{5,8\}, \{5,10\}, \{6,7\}, \{6,8\}, \{6,11\}, \{7,8\}, \{7,9\}, \{7,11\},$   
 $\{8,10\}, \{8,11\}, \{\{1,2\}, \{1,3\}, \{1,4\}, \{1,10\}, \{2,3\}, \{2,4\}, \{2,5\}, \{2,6\},$   
 $\{2,8\}, \{2,10\}, \{3,4\}, \{3,5\}, \{3,6\}, \{3,7\}, \{3,9\}, \{3,10\}, \{4,7\}, \{4,8\}, \{4,10\},$   
 $\{5,6\}, \{5,7\}, \{5,8\}, \{5,9\}, \{7,8\}, \{7,9\}, \{8,9\}, \{8,10\}, \{8,11\}, \{9,10\}, \{9,11\},$   
 $\{10,11\}, \{\{1,2\}, \{1,3\}, \{1,4\}, \{1,6\}, \{1,7\}, \{1,8\}, \{1,9\}, \{2,3\}, \{2,4\}, \{2,7\},$   
 $\{2,10\}, \{2,11\}, \{3,4\}, \{3,6\}, \{3,10\}, \{4,5\}, \{4,8\}, \{4,10\}, \{5,6\}, \{5,7\}, \{5,8\},$   
 $\{5,9\}, \{5,10\}, \{5,11\}, \{6,9\}, \{6,10\}, \{7,8\}, \{7,9\}, \{7,11\}, \{8,9\}, \{10,11\},$   
 $\{\{1,2\}, \{1,3\}, \{1,8\}, \{1,9\}, \{1,10\}, \{1,11\}, \{2,3\}, \{2,4\}, \{2,5\}, \{2,8\}, \{3,4\},$   
 $\{3,6\}, \{3,7\}, \{3,8\}, \{3,11\}, \{4,5\}, \{4,6\}, \{4,11\}, \{5,6\}, \{5,7\}, \{5,8\}, \{5,9\},$   
 $\{6,7\}, \{6,9\}, \{6,11\}, \{7,8\}, \{7,9\}, \{8,9\}, \{9,10\}, \{9,11\}, \{10,11\}, \{\{1,2\},$   
 $\{1,7\}, \{1,8\}, \{1,9\}, \{1,10\}, \{2,3\}, \{2,4\}, \{2,5\}, \{2,6\}, \{2,7\}, \{2,8\}, \{3,4\},$   
 $\{3,5\}, \{3,6\}, \{3,7\}, \{3,8\}, \{3,9\}, \{3,11\}, \{4,6\}, \{4,7\}, \{5,6\}, \{5,8\}, \{6,7\},$   
 $\{6,8\}, \{6,10\}, \{7,9\}, \{7,10\}, \{7,11\}, \{8,9\}, \{8,10\}, \{9,10\}, \{9,11\}, \{\{1,2\},$   
 $\{1,5\}, \{1,6\}, \{1,7\}, \{1,9\}, \{2,4\}, \{2,5\}, \{2,6\}, \{2,9\}, \{3,4\}, \{3,5\}, \{3,7\},$   
 $\{3,8\}, \{3,10\}, \{4,5\}, \{4,6\}, \{4,8\}, \{4,10\}, \{5,7\}, \{5,8\}, \{5,9\}, \{6,7\}, \{6,9\},$   
 $\{6,10\}, \{6,11\}, \{7,10\}, \{8,9\}, \{8,10\}, \{9,10\}, \{9,11\}, \{10,11\}, \{\{1,2\}, \{1,3\},$   
 $\{1,4\}, \{1,5\}, \{1,6\}, \{1,9\}, \{1,10\}, \{1,11\}, \{2,5\}, \{2,6\}, \{2,7\}, \{2,9\}, \{3,4\},$   
 $\{3,10\}, \{3,11\}, \{4,6\}, \{4,8\}, \{4,9\}, \{4,10\}, \{4,11\}, \{5,6\}, \{5,7\}, \{5,8\},$   
 $\{5,11\}, \{6,8\}, \{7,8\}, \{7,9\}, \{7,11\}, \{8,11\}, \{9,10\}, \{9,11\}, \{10,11\}, \{\{1,2\},$   
 $\{1,3\}, \{1,4\}, \{1,7\}, \{1,10\}, \{1,11\}, \{2,6\}, \{2,8\}, \{2,9\}, \{2,10\}, \{2,11\}, \{3,4\},$   
 $\{3,6\}, \{3,8\}, \{3,9\}, \{3,10\}, \{4,5\}, \{4,6\}, \{4,7\}, \{4,9\}, \{5,6\}, \{5,7\}, \{5,9\},$   
 $\{5,11\}, \{6,7\}, \{6,8\}, \{6,11\}, \{7,11\}, \{8,9\}, \{8,10\}, \{9,10\}, \{9,11\}, \{\{1,2\},$   
 $\{1,7\}, \{1,8\}, \{1,9\}, \{1,10\}, \{1,11\}, \{2,4\}, \{2,7\}, \{2,9\}, \{2,10\}, \{2,11\}, \{3,4\},$   
 $\{3,5\}, \{3,6\}, \{3,7\}, \{3,9\}, \{4,5\}, \{4,7\}, \{4,9\}, \{5,7\}, \{5,9\}, \{5,10\}, \{5,11\},$   
 $\{6,7\}, \{6,8\}, \{6,9\}, \{7,8\}, \{7,11\}, \{8,9\}, \{9,10\}, \{10,11\}, \{\{1,2\}, \{1,3\},$   
 $\{1,5\}, \{1,6\}, \{1,7\}, \{2,5\}, \{2,6\}, \{2,7\}, \{2,8\}, \{3,4\}, \{3,5\}, \{3,6\}, \{3,7\},$   
 $\{3,9\}, \{3,10\}, \{3,11\}, \{4,5\}, \{4,8\}, \{4,10\}, \{5,8\}, \{5,11\}, \{6,8\}, \{6,9\},$   
 $\{6,10\}, \{7,8\}, \{7,9\}, \{7,11\}, \{8,9\}, \{8,10\}, \{8,11\}, \{\{1,2\}, \{1,5\}, \{1,6\},$   
 $\{1,7\}, \{1,8\}, \{2,4\}, \{2,5\}, \{2,8\}, \{3,4\}, \{3,5\}, \{3,7\}, \{3,8\}, \{3,9\}, \{4,5\},$



{4,8},{4,9},{5,6},{5,7},{5,9},{5,10},{5,11},{6,7},{6,8},{6,10},{6,11},  
{7,8},{8,9},{8,10},{9,10},{10,11},{1,2},{1,3},{1,4},{1,5},{1,11},  
{2,3},{2,5},{2,6},{2,7},{2,10},{3,7},{3,8},{3,9},{3,11},{4,5},{4,11},  
{5,6},{5,9},{5,10},{5,11},{6,7},{6,9},{6,10},{7,8},{7,9},{7,10},{8,9},  
{8,10},{8,11},{9,11},{10,11},{1,2},{1,4},{1,5},{1,7},{1,9},{1,10},  
{2,3},{2,4},{2,5},{2,8},{2,9},{3,5},{3,6},{3,7},{3,8},{3,9},{4,5},  
{4,7},{4,8},{4,10},{4,11},{5,6},{5,7},{5,10},{5,11},{6,7},{7,8},{7,9},  
{7,10},{7,11},{8,9},{10,11},{1,2},{1,4},{1,6},{1,9},{1,10},{1,11},  
{2,4},{2,6},{2,7},{2,10},{2,11},{3,4},{3,6},{3,8},{4,6},{4,7},{4,8},  
{4,9},{5,6},{5,8},{5,11},{6,8},{6,10},{6,11},{7,8},{7,9},{7,11},{8,9},  
{8,11},{9,11},{10,11},{1,2},{1,5},{1,8},{1,10},{1,11},{2,4},{2,5},  
{2,8},{2,9},{3,4},{3,5},{3,6},{3,7},{3,8},{4,5},{4,6},{4,7},{4,9},  
{5,6},{5,8},{5,10},{6,7},{6,10},{7,8},{7,9},{7,10},{7,11},{8,9},  
{8,11},{9,11},{10,11},{1,2},{1,6},{1,7},{1,8},{1,9},{1,11},{2,5},  
{2,6},{2,8},{2,9},{2,10},{3,4},{3,5},{3,6},{3,7},{3,9},{3,11},{4,7},  
{4,11},{5,6},{5,10},{5,11},{6,9},{6,11},{7,8},{7,9},{7,10},{7,11},  
{8,10},{10,11},{1,2},{1,3},{1,4},{1,11},{2,3},{2,4},{2,5},{2,6},  
{2,10},{2,11},{3,4},{3,6},{3,11},{4,5},{4,6},{4,7},{4,8},{4,11},{5,7},  
{5,8},{5,10},{6,7},{6,9},{6,10},{6,11},{7,8},{7,9},{7,10},{8,9},  
{8,11},{9,10},{9,11},{1,2},{1,4},{1,6},{1,8},{1,9},{1,10},{2,3},  
{2,4},{2,5},{2,6},{2,10},{3,4},{3,5},{3,6},{3,11},{4,8},{4,11},{5,6},  
{5,7},{5,10},{5,11},{6,7},{6,9},{7,8},{7,9},{7,10},{7,11},{8,9},  
{8,10},{8,11},{9,10},{1,2},{1,4},{1,5},{1,6},{1,7},{1,10},{1,11},  
{2,3},{2,4},{2,7},{2,9},{2,11},{3,7},{3,9},{4,5},{4,6},{4,7},{4,8},  
{4,11},{5,6},{5,9},{5,11},{6,8},{6,9},{6,10},{7,8},{7,9},{7,10},{8,9},  
{8,10},{9,10},{9,11},{1,2},{1,4},{1,5},{1,6},{1,7},{1,11},{2,3},  
{2,4},{2,9},{2,10},{2,11},{3,4},{3,6},{3,7},{3,8},{3,9},{3,10},{4,5},  
{4,7},{4,9},{4,10},{5,6},{5,9},{5,11},{6,7},{6,8},{6,11},{8,9},{8,11},  
{9,10},{9,11},{1,2},{1,3},{1,4},{1,7},{1,8},{1,9},{2,5},{2,6},{2,7},  
{2,9},{2,11},{3,4},{3,5},{3,6},{3,8},{3,9},{3,10},{3,11},{4,7},{4,8},  
{4,10},{5,6},{5,7},{5,10},{6,9},{6,11},{7,8},{7,10},{7,11},{8,11},  
{9,11},{1,2},{1,3},{1,4},{1,6},{1,7},{1,9},{1,10},{2,3},{2,5},{2,7},  
{2,8},{2,11},{3,4},{3,8},{3,9},{3,11},{4,5},{4,6},{4,9},{4,11},{5,6},  
{5,7},{5,8},{5,9},{5,10},{5,11},{6,9},{6,10},{7,10},{8,9},{8,11}},  
{1,2},{1,3},{1,6},{1,9},{1,10},{2,3},{2,5},{2,8},{2,9},{2,11},{3,4},  
{3,5},{3,7},{4,5},{4,6},{4,7},{4,10},{5,7},{5,8},{5,10},{5,11},{6,7},  
{6,9},{6,10},{7,9},{7,11},{8,9},{8,10},{9,10},{9,11},{1,2},{1,3},  
{1,4},{1,5},{1,7},{1,8},{2,5},{2,6},{2,7},{2,8},{2,9},{2,11},{3,4},  
{3,5},{3,8},{3,10},{3,11},{4,5},{4,6},{4,8},{4,11},{5,6},{5,9},{5,10},  
{6,9},{6,11},{7,8},{8,11},{9,10},{9,11},{10,11},{1,2},{1,3},{1,4},  
{1,5},{1,6},{1,9},{1,10},{1,11},{2,4},{2,6},{2,7},{3,4},{3,9},{3,11},  
{4,7},{4,9},{4,11},{5,6},{5,7},{5,8},{5,9},{5,10},{6,7},{6,10},{7,8},  
{7,9},{7,10},{7,11},{8,9},{9,11},{10,11},{1,2},{1,3},{1,5},{1,6},  
{1,8},{2,4},{2,5},{2,7},{2,8},{2,9},{2,10},{3,4},{3,6},{3,7},{3,8},  
{3,9},{3,10},{3,11},{4,7},{4,8},{4,10},{5,6},{5,7},{5,9},{5,11},  
{6,11},{7,9},{7,11},{8,10},{9,10},{9,11},{1,2},{1,5},{1,7},{1,8},  
{1,9},{1,10},{1,11},{2,3},{2,4},{2,5},{2,6},{2,8},{3,4},{3,5},{3,6},  
{3,10},{4,5},{4,6},{4,11},{5,10},{5,11},{6,7},{6,8},{6,10},{6,11},  
{7,8},{7,9},{7,10},{7,11},{8,9},{10,11},{1,2},{1,4},{1,6},{1,7},  
{1,8},{2,4},{2,5},{2,6},{2,7},{2,11},{3,4},{3,5},{3,6},{3,7},{3,10},

{3,11},{4,6},{4,7},{5,7},{5,10},{5,11},{6,8},{6,10},{6,11},{7,8},  
{7,9},{7,10},{8,9},{8,10},{9,10},{10,11}},{{1,2},{1,3},{1,4},{1,7},  
{1,8},{1,9},{2,4},{2,5},{2,6},{2,9},{3,4},{3,7},{3,8},{3,10},{3,11},  
{4,5},{4,6},{4,7},{4,11},{5,6},{5,7},{5,8},{5,9},{6,9},{6,10},{6,11},  
{7,8},{8,9},{8,10},{9,10},{10,11}},{{1,2},{1,3},{1,4},{1,7},{1,8},  
{2,3},{2,4},{2,5},{2,6},{2,8},{2,10},{2,11},{3,4},{3,5},{3,6},{3,7},  
{3,8},{3,9},{3,10},{4,6},{4,7},{5,8},{5,9},{5,10},{6,7},{6,8},{6,9},  
{6,10},{6,11},{7,8},{8,9},{8,11},{9,10}},{{1,2},{1,4},{1,5},{1,7},  
{1,10},{1,11},{2,5},{2,7},{2,8},{2,10},{3,4},{3,6},{3,8},{3,9},{3,10},  
{4,9},{4,10},{4,11},{5,6},{5,7},{5,9},{5,10},{6,8},{6,9},{6,10},{7,8},  
{7,9},{7,11},{8,9},{8,10},{9,11}},{{1,2},{1,3},{1,4},{1,5},{1,6},  
{1,8},{2,4},{2,5},{2,8},{3,4},{3,6},{3,7},{3,10},{4,5},{4,7},{4,8},  
{4,10},{4,11},{5,6},{5,8},{5,9},{5,11},{6,7},{6,8},{6,9},{6,10},  
{6,11},{7,10},{7,11},{8,10},{9,11}},{{1,2},{1,6},{1,8},{2,3},{2,4},  
{2,6},{2,7},{2,8},{2,9},{2,10},{2,11},{3,5},{3,7},{3,8},{3,9},{3,10},  
{3,11},{4,5},{4,6},{4,7},{4,9},{5,6},{5,7},{5,8},{5,9},{6,8},{6,9},  
{7,8},{7,11},{8,11},{9,10}},{{1,2},{1,3},{1,5},{1,8},{1,9},{1,10},  
{1,11},{2,3},{2,10},{3,4},{3,5},{3,6},{3,7},{3,8},{3,10},{4,5},{4,7},  
{4,8},{4,9},{4,11},{5,6},{5,11},{6,7},{6,9},{6,10},{6,11},{7,9},{8,9},  
{9,10},{9,11}},{{1,2},{1,3},{1,4},{1,5},{1,6},{1,8},{1,10},{2,3},  
{2,7},{2,8},{2,10},{3,4},{3,7},{3,8},{4,5},{4,7},{4,10},{4,11},{5,6},  
{5,8},{5,10},{5,11},{6,8},{7,8},{7,9},{7,10},{7,11},{8,9},{8,11},  
{9,11},{10,11}},{{1,2},{1,3},{1,4},{1,5},{1,6},{1,11},{2,4},{2,5},  
{2,6},{2,7},{3,4},{3,5},{3,8},{3,9},{4,6},{4,8},{5,7},{5,9},{5,11},  
{6,7},{6,8},{6,11},{7,8},{7,9},{7,10},{7,11},{8,9},{8,10},{9,10},  
{9,11}},{{1,2},{1,3},{1,5},{1,9},{1,10},{2,3},{2,6},{2,7},{2,8},{2,9},  
{2,10},{2,11},{3,4},{3,5},{3,8},{3,10},{3,11},{4,5},{4,6},{4,7},{4,8},  
{4,9},{5,7},{5,9},{5,10},{6,7},{6,8},{6,9},{7,10},{8,9},{8,11}},  
{{1,2},{1,3},{1,4},{1,5},{1,7},{1,10},{1,11},{2,5},{2,7},{3,4},{3,5},  
{3,6},{3,8},{3,10},{3,11},{4,10},{4,11},{5,6},{5,7},{5,8},{6,7},{6,8},  
{6,9},{6,11},{7,8},{7,9},{7,10},{7,11},{8,10},{9,11},{10,11}},{{1,2},  
{1,5},{1,6},{1,7},{1,9},{1,10},{2,7},{2,10},{2,11},{3,4},{3,6},{3,9},  
{3,10},{3,11},{4,6},{4,8},{4,11},{5,6},{5,7},{5,8},{5,11},{6,8},{6,9},  
{7,8},{7,9},{7,11},{8,9},{8,11},{9,10},{10,11}},{{1,2},{1,4},{1,5},  
{1,6},{1,7},{1,11},{2,5},{2,7},{2,10},{2,11},{3,4},{3,5},{3,6},{3,8},  
{3,9},{4,5},{4,6},{5,8},{5,9},{5,10},{5,11},{6,7},{6,8},{6,9},{7,8},  
{7,9},{7,10},{7,11},{8,9},{8,10},{9,11}},{{1,2},{1,4},{1,5},{1,6},  
{1,7},{2,4},{2,5},{2,8},{3,4},{3,6},{3,7},{3,10},{3,11},{4,8},{4,11},  
{5,6},{5,8},{5,9},{5,11},{6,7},{6,9},{6,11},{7,8},{7,9},{8,9},{8,10},  
{9,10},{10,11}},{{1,2},{1,3},{1,4},{1,5},{1,6},{1,8},{1,10},{2,6},  
{2,7},{2,8},{2,9},{2,10},{2,11},{3,4},{3,6},{3,7},{3,8},{4,5},{4,7},  
{4,8},{5,7},{5,9},{5,10},{5,11},{6,7},{6,9},{6,10},{6,11},{7,8},{7,9},  
{9,11},{10,11}},{{1,2},{1,4},{1,7},{1,8},{2,3},{2,4},{2,6},{2,8},  
{2,10},{2,11},{3,4},{3,6},{3,8},{3,9},{3,10},{3,11},{4,5},{4,6},{4,7},  
{4,9},{5,6},{5,7},{5,8},{5,9},{6,8},{6,10},{6,11},{7,8},{7,9},{8,9},  
{8,10},{10,11}},{{1,2},{1,3},{1,7},{1,8},{1,11},{2,4},{2,7},{2,9},  
{2,11},{3,4},{3,5},{3,6},{3,8},{3,11},{4,6},{4,9},{4,10},{4,11},{5,6},  
{5,8},{6,8},{6,9},{6,10},{7,8},{7,9},{7,10},{7,11},{8,9},{9,10},  
{10,11}},{{1,2},{1,3},{1,4},{1,5},{1,6},{1,7},{1,8},{1,11},{2,5},  
{2,9},{2,11},{3,5},{3,6},{3,8},{3,9},{4,6},{4,7},{4,11},{5,8},{5,9},

$\{6,7\}, \{6,9\}, \{6,10\}, \{6,11\}, \{7,8\}, \{7,9\}, \{7,10\}, \{7,11\}, \{8,9\}, \{9,10\},$   
 $\{9,11\}, \{10,11\}, \{\{1,2\}, \{1,4\}, \{1,6\}, \{1,7\}, \{1,8\}, \{1,10\}, \{2,3\}, \{2,5\},$   
 $\{2,6\}, \{2,8\}, \{2,10\}, \{2,11\}, \{3,5\}, \{3,6\}, \{3,7\}, \{3,9\}, \{3,11\}, \{4,5\}, \{4,6\},$   
 $\{4,7\}, \{4,8\}, \{4,9\}, \{5,6\}, \{5,8\}, \{5,9\}, \{5,11\}, \{6,7\}, \{6,11\}, \{7,9\}, \{8,9\},$   
 $\{8,10\}\}, \{\{1,2\}, \{1,3\}, \{1,4\}, \{1,5\}, \{1,6\}, \{1,7\}, \{1,10\}, \{1,11\}, \{2,5\},$   
 $\{2,7\}, \{2,8\}, \{2,10\}, \{3,4\}, \{3,5\}, \{3,6\}, \{3,9\}, \{4,6\}, \{4,9\}, \{4,10\}, \{5,8\},$   
 $\{5,9\}, \{5,10\}, \{6,7\}, \{6,8\}, \{6,9\}, \{6,11\}, \{7,8\}, \{7,11\}, \{8,9\}, \{8,10\},$   
 $\{9,10\}\}, \{\{1,2\}, \{1,3\}, \{1,6\}, \{1,9\}, \{1,10\}, \{1,11\}, \{2,3\}, \{2,6\}, \{2,8\},$   
 $\{2,9\}, \{2,10\}, \{3,4\}, \{3,5\}, \{3,8\}, \{3,9\}, \{3,11\}, \{4,6\}, \{4,8\}, \{4,11\}, \{5,8\},$   
 $\{5,10\}, \{5,11\}, \{6,7\}, \{6,8\}, \{6,11\}, \{7,8\}, \{7,10\}, \{7,11\}, \{8,10\}, \{10,11\}\},$   
 $\{\{1,2\}, \{1,10\}, \{1,11\}, \{2,4\}, \{2,5\}, \{2,7\}, \{2,10\}, \{2,11\}, \{3,4\}, \{3,7\},$   
 $\{3,8\}, \{3,9\}, \{3,11\}, \{4,5\}, \{4,6\}, \{4,7\}, \{4,8\}, \{4,9\}, \{4,10\}, \{5,6\}, \{5,7\},$   
 $\{5,8\}, \{5,11\}, \{6,8\}, \{7,11\}, \{8,9\}, \{8,11\}, \{9,10\}, \{9,11\}, \{10,11\}\}, \{\{1,2\},$   
 $\{1,3\}, \{1,4\}, \{1,5\}, \{1,8\}, \{1,9\}, \{1,10\}, \{1,11\}, \{2,9\}, \{2,11\}, \{3,6\}, \{3,8\},$   
 $\{3,9\}, \{3,10\}, \{4,5\}, \{4,7\}, \{4,10\}, \{4,11\}, \{5,7\}, \{5,8\}, \{5,10\}, \{6,7\}, \{6,8\},$   
 $\{6,9\}, \{6,10\}, \{6,11\}, \{7,8\}, \{7,10\}, \{7,11\}, \{8,9\}, \{9,11\}\}, \{\{1,2\}, \{1,4\},$   
 $\{1,5\}, \{1,6\}, \{1,7\}, \{1,11\}, \{2,3\}, \{2,4\}, \{2,6\}, \{2,7\}, \{2,11\}, \{3,4\}, \{3,5\},$   
 $\{3,9\}, \{3,11\}, \{4,5\}, \{4,7\}, \{4,8\}, \{4,9\}, \{4,10\}, \{5,9\}, \{5,11\}, \{6,7\}, \{6,8\},$   
 $\{6,11\}, \{7,8\}, \{8,9\}, \{8,10\}, \{8,11\}, \{9,10\}, \{9,11\}\}, \{\{1,2\}, \{1,3\}, \{1,6\},$   
 $\{1,9\}, \{1,10\}, \{1,11\}, \{2,3\}, \{2,4\}, \{2,8\}, \{2,9\}, \{2,10\}, \{3,4\}, \{3,6\}, \{3,10\},$   
 $\{4,5\}, \{4,6\}, \{4,8\}, \{5,6\}, \{5,7\}, \{5,8\}, \{5,10\}, \{6,8\}, \{6,11\}, \{7,8\}, \{7,9\},$   
 $\{7,10\}, \{7,11\}, \{8,9\}, \{8,11\}, \{9,11\}\}, \{\{1,2\}, \{1,4\}, \{1,6\}, \{1,8\}, \{1,9\},$   
 $\{1,10\}, \{2,3\}, \{2,4\}, \{2,6\}, \{2,10\}, \{3,4\}, \{3,5\}, \{3,6\}, \{3,7\}, \{3,8\}, \{3,9\},$   
 $\{3,10\}, \{3,11\}, \{4,8\}, \{4,9\}, \{5,6\}, \{5,7\}, \{5,9\}, \{6,7\}, \{6,9\}, \{6,10\}, \{7,9\},$   
 $\{8,9\}, \{8,10\}, \{8,11\}, \{10,11\}\}, \{\{1,2\}, \{1,5\}, \{1,7\}, \{1,9\}, \{1,10\}, \{2,4\},$   
 $\{2,5\}, \{2,7\}, \{2,9\}, \{3,4\}, \{3,5\}, \{3,9\}, \{3,10\}, \{4,5\}, \{4,6\}, \{4,7\}, \{4,8\},$   
 $\{4,9\}, \{5,6\}, \{5,10\}, \{6,7\}, \{6,10\}, \{7,8\}, \{7,10\}, \{7,11\}, \{8,9\}, \{8,11\},$   
 $\{9,10\}, \{9,11\}, \{10,11\}\}, \{\{1,2\}, \{1,3\}, \{1,4\}, \{1,5\}, \{1,9\}, \{1,10\}, \{1,11\},$   
 $\{2,3\}, \{2,4\}, \{2,7\}, \{2,8\}, \{2,11\}, \{3,4\}, \{3,5\}, \{3,7\}, \{4,7\}, \{4,8\}, \{4,9\},$   
 $\{5,6\}, \{5,7\}, \{5,10\}, \{6,7\}, \{6,8\}, \{6,10\}, \{7,8\}, \{8,9\}, \{8,10\}, \{8,11\},$   
 $\{9,10\}, \{9,11\}, \{10,11\}\}, \{\{1,2\}, \{1,3\}, \{1,4\}, \{1,6\}, \{1,9\}, \{1,10\}, \{2,3\},$   
 $\{2,5\}, \{2,6\}, \{2,7\}, \{3,4\}, \{3,5\}, \{3,7\}, \{3,8\}, \{3,10\}, \{4,5\}, \{4,6\}, \{4,9\},$   
 $\{4,10\}, \{5,6\}, \{5,7\}, \{6,7\}, \{6,8\}, \{6,9\}, \{7,8\}, \{8,9\}, \{8,10\}, \{8,11\}, \{9,10\},$   
 $\{9,11\}, \{10,11\}\}, \{\{1,2\}, \{1,3\}, \{1,5\}, \{1,8\}, \{1,9\}, \{1,10\}, \{1,11\}, \{2,3\},$   
 $\{2,6\}, \{2,7\}, \{2,9\}, \{2,10\}, \{3,4\}, \{3,7\}, \{3,9\}, \{3,11\}, \{4,5\}, \{4,6\}, \{4,8\},$   
 $\{4,9\}, \{4,10\}, \{5,6\}, \{5,8\}, \{5,10\}, \{6,7\}, \{6,8\}, \{6,10\}, \{7,8\}, \{7,11\},$   
 $\{8,11\}, \{9,10\}\}, \{\{1,2\}, \{1,3\}, \{1,4\}, \{1,7\}, \{1,8\}, \{1,9\}, \{2,6\}, \{2,7\}, \{2,8\},$   
 $\{3,4\}, \{3,5\}, \{3,8\}, \{3,9\}, \{3,10\}, \{3,11\}, \{4,5\}, \{4,6\}, \{4,8\}, \{5,6\}, \{5,9\},$   
 $\{5,10\}, \{6,7\}, \{6,8\}, \{6,11\}, \{7,9\}, \{7,10\}, \{7,11\}, \{8,11\}, \{9,10\}, \{10,11\}\},$   
 $\{\{1,2\}, \{1,4\}, \{1,7\}, \{1,9\}, \{1,10\}, \{1,11\}, \{2,3\}, \{2,4\}, \{2,7\}, \{2,8\}, \{2,9\},$   
 $\{3,4\}, \{3,5\}, \{3,6\}, \{3,8\}, \{4,5\}, \{4,6\}, \{4,10\}, \{4,11\}, \{5,6\}, \{5,8\}, \{5,10\},$   
 $\{6,8\}, \{6,11\}, \{7,8\}, \{7,9\}, \{7,10\}, \{8,9\}, \{8,10\}, \{8,11\}, \{9,11\}\}, \{\{1,2\},$   
 $\{1,5\}, \{1,6\}, \{1,9\}, \{1,10\}, \{1,11\}, \{2,4\}, \{2,7\}, \{2,8\}, \{2,9\}, \{2,10\}, \{3,4\},$   
 $\{3,5\}, \{3,8\}, \{4,5\}, \{4,7\}, \{4,8\}, \{4,10\}, \{4,11\}, \{5,6\}, \{5,8\}, \{5,9\}, \{5,11\},$   
 $\{6,7\}, \{6,8\}, \{6,9\}, \{6,10\}, \{7,8\}, \{7,10\}, \{8,9\}, \{10,11\}\}, \{\{1,2\}, \{1,3\},$   
 $\{1,5\}, \{1,7\}, \{1,8\}, \{2,3\}, \{2,4\}, \{2,5\}, \{2,10\}, \{2,11\}, \{3,4\}, \{3,6\}, \{3,8\},$   
 $\{3,10\}, \{4,5\}, \{4,6\}, \{4,11\}, \{5,7\}, \{5,9\}, \{5,11\}, \{6,7\}, \{6,8\}, \{6,9\}, \{7,8\},$   
 $\{7,9\}, \{8,9\}, \{8,10\}, \{9,10\}, \{9,11\}, \{10,11\}\}, \{\{1,2\}, \{1,4\}, \{1,5\}, \{1,7\},$   
 $\{1,10\}, \{2,3\}, \{2,4\}, \{2,7\}, \{2,9\}, \{2,11\}, \{3,4\}, \{3,6\}, \{3,8\}, \{3,9\}, \{4,5\},$   
 $\{4,6\}, \{5,6\}, \{5,7\}, \{5,8\}, \{5,10\}, \{6,8\}, \{6,9\}, \{6,10\}, \{6,11\}, \{7,8\}, \{7,10\},$

{7,11},{8,9},{9,11},{10,11}},{{1,2},{1,3},{1,6},{1,7},{1,9},{1,10},  
 {1,11},{2,3},{2,4},{2,5},{2,6},{2,9},{3,4},{3,6},{3,8},{3,9},{4,5},  
 {4,7},{4,8},{4,9},{5,6},{5,7},{5,8},{6,7},{6,8},{6,10},{7,8},{7,9},  
 {7,10},{7,11},{9,11}},{{1,2},{1,5},{1,6},{1,7},{1,8},{1,9},{2,6},  
 {2,7},{2,9},{2,11},{3,4},{3,5},{3,7},{3,8},{3,9},{3,10},{3,11},{4,6},  
 {4,7},{4,10},{4,11},{5,7},{5,8},{6,7},{6,9},{6,10},{7,11},{8,9},  
 {9,10},{9,11},{10,11}},{{1,2},{1,4},{1,5},{1,6},{1,7},{1,9},{2,4},  
 {2,7},{2,8},{2,10},{2,11},{3,4},{3,5},{3,7},{3,8},{3,9},{3,10},{4,7},  
 {4,8},{4,9},{4,11},{5,6},{5,9},{5,10},{6,7},{6,10},{7,10},{8,9},  
 {8,10},{8,11}},{{1,2},{1,5},{1,6},{1,7},{1,8},{1,11},{2,3},{2,6},  
 {2,7},{2,9},{2,11},{3,4},{3,5},{3,7},{3,9},{4,5},{4,6},{4,7},{4,9},  
 {5,7},{5,8},{5,9},{6,7},{6,9},{6,11},{8,9},{8,10},{8,11},{9,10},  
 {9,11},{10,11}},{{1,2},{1,3},{1,4},{1,6},{1,8},{1,10},{2,3},{2,5},  
 {2,7},{2,8},{2,9},{3,4},{3,7},{3,9},{3,10},{4,5},{4,6},{4,7},{4,10},  
 {5,6},{5,7},{5,8},{6,8},{7,9},{8,9},{8,10},{8,11},{9,10},{9,11},  
 {10,11}},{{1,2},{1,3},{1,5},{1,7},{1,10},{1,11},{2,4},{2,5},{2,8},  
 {2,9},{3,5},{3,6},{3,7},{3,8},{4,5},{4,6},{4,7},{4,9},{4,10},{4,11},  
 {5,6},{5,11},{6,7},{6,8},{7,10},{7,11},{8,9},{8,10},{9,10}},{{1,2},  
 {1,5},{1,6},{1,7},{1,8},{2,3},{2,6},{2,8},{2,9},{3,4},{3,6},{3,8},  
 {3,9},{4,5},{4,6},{4,8},{5,6},{5,7},{5,8},{6,7},{6,9},{6,11},{7,8},  
 {7,9},{7,10},{7,11},{8,9},{8,10},{9,10},{9,11}},{{1,2},{1,4},{1,8},  
 {1,9},{1,10},{2,4},{2,6},{2,7},{2,10},{3,4},{3,5},{3,7},{3,8},{3,10},  
 {3,11},{4,9},{4,10},{4,11},{5,6},{5,8},{5,9},{5,11},{6,7},{6,9},  
 {6,11},{7,8},{7,10},{8,9},{8,10},{9,11}},{{1,2},{1,5},{1,8},{1,9},  
 {1,10},{1,11},{2,4},{2,10},{2,11},{3,4},{3,7},{3,10},{3,11},{4,6},  
 {4,9},{4,10},{4,11},{5,6},{5,7},{5,8},{5,9},{5,10},{6,7},{6,9},{6,10},  
 {7,8},{7,10},{7,11},{8,9},{8,11}},{{1,2},{1,3},{1,4},{1,5},{1,7},  
 {1,10},{2,5},{2,6},{2,7},{2,10},{2,11},{3,4},{3,5},{3,7},{3,8},{4,5},  
 {4,6},{4,8},{4,9},{4,10},{4,11},{5,11},{6,7},{6,8},{6,9},{6,10},  
 {6,11},{7,8},{7,10},{8,11},{9,10}},{{1,2},{1,5},{1,8},{1,9},{1,11},  
 {2,3},{2,5},{2,7},{2,11},{3,4},{3,6},{3,7},{3,8},{3,11},{4,5},{4,6},  
 {4,7},{4,8},{4,9},{4,10},{4,11},{5,7},{5,9},{5,10},{5,11},{6,7},{7,9},  
 {8,9},{8,11},{10,11}},{{1,2},{1,4},{1,6},{1,7},{1,9},{1,10},{1,11},  
 {2,3},{2,4},{2,6},{2,9},{3,4},{3,5},{3,6},{3,9},{4,5},{4,7},{4,8},  
 {4,10},{5,6},{5,8},{5,9},{6,7},{6,8},{6,11},{7,8},{8,9},{8,10},{8,11},  
 {9,10},{9,11}},{{1,2},{1,4},{1,5},{1,10},{1,11},{2,3},{2,4},{2,9},  
 {2,10},{3,4},{3,6},{3,8},{3,9},{3,10},{4,5},{4,6},{4,8},{5,6},{5,7},  
 {5,11},{6,7},{6,8},{6,10},{7,8},{7,9},{7,11},{8,9},{9,10},{9,11},  
 {10,11}},{{1,2},{1,3},{1,4},{1,5},{1,6},{1,7},{1,8},{2,3},{2,5},{2,6},  
 {2,9},{2,11},{3,4},{3,6},{3,10},{4,5},{4,7},{4,10},{5,7},{5,11},{6,8},  
 {6,9},{6,10},{7,8},{7,11},{8,9},{8,10},{8,11},{9,10},{9,11}},{{1,2},  
 {1,3},{1,4},{1,5},{1,8},{1,9},{2,3},{2,6},{2,7},{2,9},{2,10},{3,5},  
 {3,6},{4,5},{4,6},{4,8},{4,9},{4,11},{5,6},{5,11},{6,7},{6,9},{6,11},  
 {7,8},{7,10},{7,11},{8,9},{8,10},{8,11},{9,10}},{{1,2},{1,3},{1,5},  
 {1,9},{1,10},{2,7},{2,8},{2,9},{2,10},{3,4},{3,5},{3,10},{4,5},{4,6},  
 {4,7},{4,10},{4,11},{5,6},{5,8},{5,9},{5,11},{6,7},{6,9},{7,8},{7,9},  
 {7,10},{7,11},{8,9},{8,11},{10,11}},{{1,2},{1,3},{1,4},{1,6},{1,7},  
 {1,9},{2,5},{2,6},{2,7},{2,8},{2,9},{3,4},{3,5},{3,7},{3,9},{3,10},  
 {3,11},{4,5},{4,6},{4,10},{5,6},{5,8},{5,9},{5,10},{6,7},{6,8},{6,10},  
 {6,11},{7,9},{7,11},{10,11}},{{1,2},{1,5},{1,6},{1,9},{1,10},{1,11},

{2,3},{2,4},{2,5},{2,6},{2,9},{3,4},{3,5},{3,6},{3,7},{4,6},{4,7},  
{4,8},{4,9},{5,7},{5,9},{6,8},{6,10},{7,8},{7,9},{7,10},{7,11},{8,10},  
{9,11},{10,11}},{{1,2},{1,4},{1,5},{1,6},{1,7},{1,9},{2,3},{2,4},  
{2,5},{2,10},{3,4},{3,5},{3,7},{3,8},{3,10},{4,8},{4,9},{5,6},{5,7},  
{5,10},{6,7},{6,8},{6,10},{6,11},{7,8},{7,9},{7,11},{8,9},{8,10},  
{8,11}},{{1,2},{1,3},{1,5},{1,8},{1,10},{1,11},{2,5},{2,6},{2,8},  
{2,9},{2,10},{3,4},{3,8},{3,10},{3,11},{4,7},{4,8},{4,11},{5,6},{5,7},  
{5,8},{5,9},{5,11},{6,7},{6,9},{6,10},{6,11},{7,8},{7,11},{10,11}},  
{{1,2},{1,4},{1,5},{1,6},{1,7},{1,8},{1,9},{1,10},{2,3},{2,4},{2,5},  
{2,7},{2,8},{3,4},{3,8},{3,10},{3,11},{4,6},{4,10},{5,6},{5,7},{5,8},  
{5,11},{6,10},{6,11},{7,8},{8,9},{8,10},{8,11},{9,10},{10,11}},{{1,2},  
{1,6},{1,11},{2,4},{2,6},{2,8},{2,9},{2,10},{2,11},{3,4},{3,5},{3,6},  
{3,7},{3,9},{3,11},{4,5},{4,8},{4,9},{4,10},{4,11},{5,9},{6,7},{6,9},  
{6,11},{7,8},{7,9},{7,10},{7,11},{8,10},{8,11},{9,10}},{{1,2},{1,3},  
{1,6},{1,7},{1,9},{1,11},{2,4},{2,9},{2,10},{2,11},{3,4},{3,6},{3,7},  
{3,10},{3,11},{4,6},{4,8},{4,9},{4,10},{5,6},{5,7},{5,8},{5,9},{6,7},  
{6,9},{7,8},{7,10},{8,9},{8,10},{10,11}},{{1,2},{1,6},{1,8},{1,10},  
{1,11},{2,3},{2,4},{2,8},{2,10},{3,4},{3,5},{3,7},{3,10},{4,5},{4,6},  
{4,8},{5,6},{5,7},{5,9},{6,8},{6,9},{6,11},{7,9},{7,10},{7,11},{8,9},  
{8,10},{9,10},{9,11},{10,11}},{{1,2},{1,3},{1,6},{1,7},{2,3},{2,6},  
{2,10},{2,11},{3,4},{3,5},{3,7},{3,9},{3,10},{3,11},{4,5},{4,6},{4,7},  
{4,8},{4,9},{5,6},{5,11},{6,7},{6,8},{6,9},{6,10},{6,11},{7,8},{7,9},  
{8,9},{9,10},{10,11}},{{1,2},{1,3},{1,5},{1,6},{1,8},{1,9},{2,4},  
{2,5},{2,6},{2,9},{3,4},{3,7},{3,8},{3,9},{3,10},{4,5},{4,7},{4,8},  
{4,9},{5,6},{5,7},{5,8},{6,7},{6,9},{6,10},{6,11},{7,8},{7,10},{7,11},  
{9,10},{10,11}},{{1,2},{1,3},{1,4},{1,5},{2,3},{2,4},{2,5},{2,9},  
{2,10},{2,11},{3,4},{3,5},{3,6},{3,8},{3,10},{3,11},{4,5},{4,6},{4,8},  
{4,9},{6,7},{6,8},{6,9},{6,10},{7,9},{7,10},{8,9},{8,11},{9,10},  
{9,11},{10,11}},{{1,2},{1,4},{1,6},{1,7},{2,3},{2,4},{2,5},{2,7},  
{2,9},{3,4},{3,6},{3,9},{3,10},{4,6},{4,10},{4,11},{5,7},{5,9},{5,11},  
{6,7},{6,8},{6,10},{7,8},{7,11},{8,9},{8,10},{8,11},{9,10},{9,11},  
{10,11}},{{1,2},{1,6},{1,7},{1,8},{1,9},{1,11},{2,3},{2,4},{2,6},  
{2,9},{2,11},{3,4},{3,5},{3,7},{3,8},{3,9},{4,5},{4,11},{5,6},{5,7},  
{5,8},{5,10},{5,11},{6,7},{6,10},{6,11},{7,8},{7,9},{7,10},{8,11}},  
{{1,2},{1,3},{1,4},{1,5},{1,9},{1,10},{2,3},{2,5},{2,6},{2,7},{2,10},  
{3,4},{3,7},{3,8},{3,10},{3,11},{4,8},{4,9},{5,6},{5,8},{5,9},{6,7},  
{6,8},{6,9},{6,10},{7,8},{7,11},{8,9},{8,11},{9,10}},{{1,2},{1,3},  
{1,5},{1,6},{1,11},{2,3},{2,6},{2,7},{2,8},{2,9},{2,10},{2,11},{3,4},  
{3,5},{3,9},{3,11},{4,5},{4,7},{4,9},{4,10},{5,6},{5,7},{5,8},{5,10},  
{5,11},{6,7},{7,9},{7,10},{8,10},{8,11},{9,10}},{{1,2},{1,3},{1,4},  
{1,9},{1,10},{2,8},{2,9},{2,10},{2,11},{3,4},{3,5},{3,6},{3,10},  
{3,11},{4,6},{4,7},{4,9},{4,11},{5,6},{5,8},{5,9},{5,10},{6,7},{6,8},  
{6,11},{7,8},{7,9},{8,9},{8,11},{9,10}},{{1,2},{1,3},{1,4},{1,5},  
{1,9},{1,10},{1,11},{2,3},{2,5},{2,8},{2,10},{3,5},{3,6},{3,8},{3,9},  
{3,11},{4,5},{4,6},{4,7},{4,10},{5,6},{6,7},{6,8},{7,8},{7,9},{7,10},  
{8,9},{8,10},{9,10},{9,11}},{{1,2},{1,3},{1,4},{1,5},{1,6},{1,7},  
{1,8},{1,10},{1,11},{2,4},{2,5},{2,6},{2,9},{3,4},{3,8},{3,9},{4,6},  
{4,9},{5,9},{5,11},{6,9},{6,10},{7,8},{7,9},{7,10},{7,11},{8,9},  
{9,10},{9,11},{10,11}},{{1,2},{1,3},{1,5},{1,6},{1,10},{1,11},{2,3},  
{2,6},{2,7},{2,9},{2,10},{3,4},{3,5},{3,7},{3,10},{3,11},{4,5},{4,7},

{4,8},{4,9},{4,10},{5,6},{5,7},{5,11},{6,7},{6,9},{7,8},{7,9},{8,9},  
{9,10}},{{1,2},{1,3},{1,5},{1,8},{2,4},{2,5},{2,7},{2,8},{2,11},{3,4},  
{3,5},{3,6},{3,7},{3,8},{4,5},{4,7},{4,9},{4,10},{5,6},{5,9},{5,10},  
{5,11},{6,8},{6,10},{7,8},{7,10},{8,10},{8,11},{9,10},{10,11}},{{1,2},  
{1,6},{1,8},{1,11},{2,3},{2,6},{2,9},{2,10},{2,11},{3,4},{3,7},{3,9},  
{3,10},{4,5},{4,7},{4,8},{4,9},{4,11},{5,6},{5,7},{5,8},{6,7},{6,8},  
{6,10},{7,10},{8,9},{8,10},{8,11},{9,10},{9,11}},{{1,2},{1,5},{1,6},  
{1,9},{1,10},{2,5},{2,6},{2,8},{2,9},{3,4},{3,5},{3,7},{3,11},{4,5},  
{4,6},{4,7},{4,9},{5,8},{5,9},{5,10},{5,11},{6,7},{6,8},{6,9},{6,10},  
{6,11},{7,11},{8,10},{8,11},{10,11}},{{1,2},{1,4},{1,6},{1,8},{1,10},  
{1,11},{2,3},{2,9},{2,10},{2,11},{3,4},{3,5},{3,7},{3,9},{3,10},  
{3,11},{4,5},{4,6},{4,10},{5,6},{5,11},{6,7},{6,8},{6,11},{7,8},{7,9},  
{7,11},{8,9},{8,10},{9,10}},{{1,2},{1,6},{1,7},{1,8},{1,10},{2,3},  
{2,4},{2,5},{2,7},{2,9},{2,10},{2,11},{3,4},{3,8},{3,9},{3,10},{3,11},  
{4,5},{4,8},{4,10},{4,11},{5,7},{5,8},{5,9},{6,7},{6,8},{7,8},{7,9},  
{8,9},{8,10},{10,11}},{{1,2},{1,3},{1,4},{1,5},{1,6},{1,9},{2,3},  
{2,6},{2,7},{2,8},{2,9},{2,10},{3,4},{3,8},{3,10},{4,5},{4,6},{4,8},  
{4,9},{4,10},{4,11},{5,6},{5,9},{6,7},{6,9},{6,11},{7,8},{7,11},  
{8,10},{8,11},{9,10}},{{1,2},{1,3},{1,4},{1,7},{1,8},{1,11},{2,3},  
{2,6},{2,8},{2,10},{2,11},{3,4},{3,5},{3,6},{3,9},{3,11},{4,7},{4,8},  
{4,9},{5,6},{5,8},{5,9},{6,8},{6,10},{7,8},{7,10},{7,11},{8,9},{8,10},  
{10,11}},{{1,2},{1,3},{1,4},{1,5},{1,7},{2,3},{2,5},{2,7},{2,8},{2,9},  
{2,10},{3,4},{3,6},{3,7},{3,10},{4,5},{4,6},{4,10},{4,11},{5,6},{5,7},  
{5,8},{5,11},{6,7},{6,10},{6,11},{8,9},{8,10},{8,11},{9,10},{10,11}},  
{{1,2},{1,5},{1,6},{1,7},{1,9},{1,11},{2,3},{2,5},{2,6},{2,8},{2,11},  
{3,4},{3,5},{3,7},{3,8},{3,10},{3,11},{4,7},{4,9},{4,11},{5,6},{5,7},  
{6,8},{6,9},{6,10},{7,9},{8,10},{9,10},{9,11},{10,11}},{{1,2},{1,5},  
{1,6},{1,7},{1,8},{1,9},{1,10},{2,3},{2,4},{2,5},{2,7},{2,8},{2,10},  
{3,4},{3,6},{3,8},{3,11},{4,7},{4,11},{5,7},{5,9},{5,11},{6,7},{6,8},  
{6,9},{6,11},{7,11},{8,9},{8,10},{9,11}},{{1,2},{1,3},{1,4},{1,5},  
{1,6},{1,7},{2,4},{2,7},{2,9},{2,10},{2,11},{3,4},{3,5},{3,7},{3,9},  
{4,6},{4,9},{4,11},{5,6},{5,7},{5,8},{6,8},{6,10},{6,11},{7,8},{7,9},  
{8,9},{8,10},{9,10},{10,11}},{{1,2},{1,4},{1,5},{1,6},{1,8},{1,10},  
{2,3},{2,7},{2,8},{2,10},{3,4},{3,7},{3,9},{3,10},{4,6},{4,9},{4,10},  
{5,6},{5,7},{5,8},{5,11},{6,7},{6,9},{7,9},{7,11},{8,9},{8,10},{8,11},  
{9,10},{9,11}},{{1,2},{1,3},{1,6},{1,8},{2,3},{2,4},{2,5},{2,10},  
{3,4},{3,7},{3,10},{3,11},{4,5},{4,8},{4,9},{4,11},{5,6},{5,8},{5,9},  
{6,7},{6,8},{6,10},{7,8},{7,9},{7,10},{7,11},{8,11},{9,10}},{{1,2},  
{1,4},{1,5},{1,6},{1,10},{1,11},{2,4},{2,5},{2,8},{2,9},{2,10},{3,4},  
{3,6},{3,7},{3,8},{3,11},{4,8},{4,9},{4,11},{5,6},{5,7},{5,8},{5,10},  
{6,7},{6,11},{7,8},{7,9},{7,10},{8,9},{9,10}},{{1,2},{1,4},{1,8},  
{1,10},{1,11},{2,3},{2,4},{2,5},{2,10},{2,11},{3,4},{3,5},{3,6},{3,7},  
{3,8},{3,9},{3,11},{4,9},{4,10},{4,11},{5,6},{5,7},{5,10},{6,7},{6,8},  
{6,10},{7,9},{7,10},{8,10},{8,11},{9,10}},{{1,2},{1,4},{1,8},{1,9},  
{1,10},{1,11},{2,4},{2,5},{2,6},{2,7},{2,8},{3,4},{3,6},{3,8},{3,9},  
{3,10},{3,11},{4,6},{4,9},{4,11},{5,6},{5,7},{6,7},{6,8},{7,9},{7,10},  
{8,10},{8,11},{9,10}},{{1,2},{1,3},{1,5},{1,11},{2,4},{2,5},{2,6},  
{2,10},{2,11},{3,4},{3,5},{3,8},{3,9},{3,11},{4,5},{4,7},{4,9},{4,10},  
{5,6},{5,9},{6,9},{6,10},{6,11},{7,9},{7,10},{8,9},{8,10},{8,11},  
{9,10},{10,11}},{{1,2},{1,3},{1,5},{1,7},{1,8},{1,9},{1,10},{1,11},

{2,7},{2,9},{3,4},{3,5},{3,6},{3,7},{3,8},{3,10},{3,11},{4,6},{4,7},  
{4,9},{4,11},{5,6},{5,9},{5,11},{6,7},{6,9},{7,8},{7,9},{7,10},{8,10},  
{9,11}},{{1,2},{1,5},{1,7},{1,9},{1,10},{2,3},{2,4},{2,7},{2,8},{2,9},  
{2,10},{3,4},{3,10},{4,5},{4,6},{4,7},{4,8},{4,10},{5,6},{5,7},{5,10},  
{6,7},{6,9},{6,10},{6,11},{7,8},{7,9},{9,10},{9,11},{10,11}},{{1,2},  
{1,5},{1,6},{1,8},{1,9},{1,11},{2,3},{2,4},{2,5},{2,6},{3,4},{3,5},  
{3,6},{3,7},{4,5},{4,6},{4,8},{4,10},{5,7},{5,8},{5,9},{6,7},{6,10},  
{6,11},{7,8},{7,10},{7,11},{8,9},{8,10},{8,11},{10,11}},{{1,2},{1,4},  
{1,5},{1,6},{1,11},{2,3},{2,4},{2,7},{2,10},{2,11},{3,4},{3,5},{3,7},  
{4,5},{4,6},{4,10},{5,6},{5,7},{5,8},{6,8},{6,9},{6,10},{7,8},{7,10},  
{7,11},{8,9},{8,11},{9,10},{9,11},{10,11}},{{1,2},{1,3},{1,5},{1,7},  
{1,9},{1,11},{2,3},{2,5},{2,6},{3,4},{3,6},{3,7},{3,8},{3,9},{4,8},  
{4,9},{5,6},{5,8},{5,9},{5,11},{6,7},{6,8},{6,11},{7,10},{7,11},{8,9},  
{8,10},{9,10},{10,11}},{{1,2},{1,5},{1,8},{1,11},{2,3},{2,7},{2,8},  
{2,9},{2,10},{2,11},{3,4},{3,6},{3,8},{3,9},{3,10},{4,5},{4,6},{4,7},  
{4,9},{4,10},{4,11},{5,6},{5,8},{5,9},{5,11},{6,8},{7,10},{7,11},  
{8,10},{9,11}},{{1,2},{1,4},{1,6},{1,9},{1,10},{2,4},{2,5},{2,6},  
{2,10},{3,4},{3,5},{3,6},{3,7},{3,8},{3,9},{3,11},{4,5},{4,7},{4,9},  
{4,10},{5,6},{5,9},{6,7},{6,8},{6,9},{6,10},{6,11},{7,8},{7,10},  
{7,11},{8,11}},{{1,2},{1,4},{1,6},{1,7},{1,10},{2,3},{2,4},{2,5},  
{2,7},{2,9},{2,10},{3,6},{3,7},{3,8},{3,9},{3,10},{3,11},{4,5},{4,7},  
{4,8},{4,11},{5,9},{5,11},{6,7},{6,8},{6,10},{7,8},{8,11},{9,10},  
{9,11}},{{1,2},{1,3},{1,4},{1,8},{1,11},{2,3},{2,5},{2,6},{2,9},  
{2,11},{3,4},{3,6},{3,8},{3,10},{4,7},{4,8},{4,10},{4,11},{5,6},{5,7},  
{5,9},{5,10},{6,7},{6,8},{7,8},{7,10},{7,11},{9,10},{9,11},{10,11}},  
{{1,2},{1,6},{1,7},{1,11},{2,3},{2,4},{2,7},{2,8},{2,11},{3,4},{3,5},  
{3,6},{3,7},{4,5},{4,7},{4,8},{4,9},{5,6},{5,8},{5,9},{5,10},{6,7},  
{6,9},{6,10},{6,11},{7,9},{8,10},{8,11},{9,10},{10,11}},{{1,2},{1,5},  
{1,6},{1,7},{2,3},{2,5},{2,7},{2,10},{2,11},{3,4},{3,8},{3,9},{3,10},  
{3,11},{4,5},{4,8},{4,11},{5,6},{5,8},{5,11},{6,7},{6,8},{6,9},{6,10},  
{7,9},{7,10},{7,11},{8,9},{9,10},{9,11}},{{1,2},{1,4},{1,5},{1,6},  
{1,8},{1,10},{2,5},{2,8},{2,10},{3,4},{3,5},{3,6},{3,9},{3,10},{4,6},  
{4,9},{4,10},{5,6},{5,8},{5,10},{6,7},{6,8},{6,9},{6,11},{7,9},{7,10},  
{7,11},{8,10},{8,11},{9,10},{10,11}},{{1,2},{1,3},{1,6},{1,7},{1,8},  
{1,10},{2,4},{2,7},{2,8},{3,4},{3,5},{3,8},{3,9},{3,10},{4,5},{4,7},  
{4,8},{4,11},{5,6},{5,7},{5,9},{5,10},{5,11},{6,7},{6,10},{7,11},  
{8,9},{8,11},{9,10},{9,11}},{{1,2},{1,3},{1,4},{1,5},{1,6},{1,8},  
{1,9},{2,4},{2,5},{2,9},{2,10},{2,11},{3,4},{3,6},{3,7},{3,8},{3,10},  
{4,10},{4,11},{5,8},{5,9},{5,10},{6,7},{6,8},{6,9},{6,10},{7,8},  
{7,10},{8,10},{9,10},{10,11}},{{1,2},{1,4},{1,5},{1,6},{1,7},{1,10},  
{1,11},{2,3},{2,4},{2,9},{2,10},{2,11},{3,4},{3,8},{3,9},{4,7},{4,8},  
{4,11},{5,6},{5,7},{6,7},{6,8},{6,9},{6,10},{6,11},{7,8},{8,9},{8,10},  
{9,10},{9,11}},{{1,2},{1,3},{1,5},{1,7},{1,8},{1,9},{2,3},{2,4},{2,7},  
{2,9},{2,10},{2,11},{3,4},{3,5},{3,8},{3,10},{3,11},{4,6},{4,7},{4,8},  
{4,10},{4,11},{5,6},{5,8},{5,9},{6,7},{6,8},{6,9},{7,8},{7,9},  
{10,11}},{{1,2},{1,4},{1,6},{1,8},{1,10},{2,4},{2,6},{2,8},{2,11},  
{3,4},{3,7},{3,9},{4,5},{4,6},{4,7},{4,9},{4,10},{4,11},{5,6},{5,7},  
{6,7},{6,8},{7,8},{7,9},{8,9},{8,10},{8,11},{9,10},{9,11},{10,11}},  
{{1,2},{1,3},{1,4},{1,7},{1,8},{1,10},{2,3},{2,4},{2,5},{2,10},{3,4},  
{3,5},{3,8},{3,11},{4,7},{4,11},{5,6},{5,8},{5,9},{5,10},{5,11},{6,7},

{6,8},{6,9},{6,10},{7,9},{7,10},{7,11},{8,10},{9,11}},{{1,2},{1,3},  
 {1,5},{1,8},{1,11},{2,4},{2,5},{2,7},{2,8},{2,9},{2,10},{3,4},{3,6},  
 {3,7},{3,8},{3,10},{3,11},{4,7},{4,8},{4,9},{4,11},{5,6},{5,9},{5,11},  
 {6,9},{6,10},{6,11},{7,10},{9,10},{9,11}},{{1,2},{1,3},{1,4},{1,5},  
 {1,9},{2,3},{2,5},{2,6},{2,9},{3,4},{3,6},{3,8},{3,10},{4,5},{4,7},  
 {4,8},{4,9},{4,10},{5,6},{5,9},{5,10},{6,8},{6,9},{6,10},{6,11},{7,8},  
 {7,9},{8,9},{8,10},{8,11},{9,11}},{{1,2},{1,4},{1,6},{1,9},{1,11},  
 {2,3},{2,4},{2,7},{2,11},{3,4},{3,5},{3,7},{3,8},{3,9},{3,11},{4,5},  
 {4,9},{5,7},{5,9},{5,10},{6,7},{6,9},{6,10},{6,11},{7,10},{7,11},  
 {8,9},{8,11},{9,10},{9,11}},{{1,2},{1,4},{1,5},{1,10},{1,11},{2,3},  
 {2,5},{2,6},{2,9},{2,11},{3,4},{3,5},{3,6},{3,7},{3,8},{3,9},{4,5},  
 {4,7},{4,10},{4,11},{5,6},{5,10},{6,7},{6,10},{7,8},{7,9},{7,10},  
 {7,11},{8,9},{9,11}},{{1,2},{1,3},{1,7},{1,8},{1,10},{2,3},{2,4},  
 {2,5},{2,6},{2,8},{2,10},{2,11},{3,4},{3,6},{3,7},{3,9},{3,10},{4,6},  
 {4,9},{4,11},{5,6},{5,8},{5,9},{5,11},{6,9},{7,8},{7,9},{8,9},{8,11},  
 {9,11}},{{1,2},{1,3},{1,4},{1,6},{1,10},{2,6},{2,7},{2,8},{3,4},{3,5},  
 {3,6},{3,8},{3,9},{3,11},{4,7},{4,8},{4,9},{4,11},{5,6},{5,7},{5,8},  
 {5,11},{6,10},{7,8},{7,10},{7,11},{8,9},{10,11}},{{1,2},{1,3},{1,4},  
 {1,6},{1,8},{2,3},{2,7},{2,8},{2,11},{3,4},{3,5},{3,6},{3,7},{3,9},  
 {3,11},{4,6},{4,8},{4,11},{5,6},{5,7},{5,9},{5,10},{6,7},{6,8},{6,9},  
 {6,10},{7,8},{7,9},{7,10},{7,11},{8,11},{9,10}},{{1,2},{1,3},{1,7},  
 {1,10},{1,11},{2,3},{2,5},{2,7},{2,9},{2,11},{3,4},{3,8},{3,11},{4,5},  
 {4,6},{4,8},{4,9},{4,11},{5,6},{5,7},{5,8},{5,9},{6,8},{6,10},{6,11},  
 {7,8},{7,10},{8,10},{9,11},{10,11}},{{1,2},{1,3},{1,5},{1,6},{1,7},  
 {1,9},{1,11},{2,5},{2,8},{2,9},{2,10},{3,4},{3,5},{3,9},{3,11},{4,5},  
 {4,6},{4,7},{4,9},{4,10},{5,7},{5,10},{5,11},{6,7},{6,8},{6,9},{7,8},  
 {8,10},{9,10}},{{1,2},{1,4},{1,6},{1,7},{1,9},{1,11},{2,4},{2,6},  
 {2,8},{2,10},{2,11},{3,4},{3,5},{3,7},{3,8},{3,9},{4,7},{4,8},{4,11},  
 {5,8},{5,9},{5,10},{6,7},{6,8},{6,9},{6,10},{7,8},{7,9},{8,10},  
 {9,10}},{{1,2},{1,3},{1,4},{1,6},{1,9},{2,3},{2,5},{2,9},{2,10},  
 {2,11},{3,4},{3,5},{3,6},{3,8},{3,11},{4,6},{4,7},{4,11},{5,8},{5,10},  
 {5,11},{6,7},{6,8},{6,9},{7,8},{7,9},{7,11},{8,9},{8,10},{9,10}},  
 {{1,2},{1,5},{1,7},{2,3},{2,5},{2,7},{2,10},{2,11},{3,4},{3,6},{3,9},  
 {3,10},{3,11},{4,6},{4,7},{4,8},{4,9},{4,10},{5,6},{5,7},{5,8},{5,11},  
 {6,8},{6,11},{7,8},{7,10},{8,10},{8,11},{9,10},{10,11}},{{1,5},{1,6},  
 {1,7},{1,9},{1,10},{2,6},{2,8},{2,9},{2,10},{2,11},{3,7},{3,8},{3,9},  
 {3,11},{4,7},{4,8},{4,10},{4,11},{5,7},{5,9},{5,10},{5,11},{6,8},  
 {6,9},{6,10},{7,8},{9,11},{10,11}},{{1,4},{1,6},{1,7},{1,9},{1,10},  
 {2,5},{2,7},{2,8},{2,9},{2,11},{3,6},{3,8},{3,9},{3,10},{3,11},{4,7},  
 {4,9},{4,10},{4,11},{5,7},{5,8},{5,10},{5,11},{6,8},{6,9},{6,10},  
 {9,11},{10,11}},{{1,5},{1,6},{1,8},{1,9},{1,10},{2,5},{2,7},{2,8},  
 {2,9},{2,10},{3,6},{3,7},{3,8},{3,10},{3,11},{4,6},{4,7},{4,9},{4,10},  
 {4,11},{5,8},{5,9},{6,10},{6,11},{7,10},{7,11},{8,11},{9,11}},{{1,5},  
 {1,6},{1,7},{1,8},{1,10},{2,6},{2,7},{2,9},{2,11},{3,6},{3,8},{3,9},  
 {3,11},{4,7},{4,8},{4,9},{4,10},{4,11},{5,7},{5,8},{5,11},{6,9},  
 {6,10},{7,10},{7,11},{8,10},{8,11},{9,10}},{{1,4},{1,5},{1,7},{1,8},  
 {1,10},{2,5},{2,6},{2,8},{2,9},{2,11},{3,6},{3,7},{3,8},{3,10},{3,11},  
 {4,7},{4,8},{4,11},{5,9},{5,10},{6,9},{6,10},{7,9},{7,10},{7,11},  
 {8,10},{8,11},{9,11}},{{1,2},{1,3},{1,4},{1,5},{1,6},{2,6},{2,7},  
 {2,8},{2,9},{3,5},{3,6},{3,7},{3,10},{4,5},{4,6},{4,9},{4,10},{4,11},



{5,7},{5,9},{5,10},{5,11},{6,8},{6,10},{7,8},{8,9},{8,10},{10,11},  
{1,2},{1,3},{1,4},{1,5},{1,6},{2,6},{2,7},{2,8},{2,9},{2,11},{3,5},  
{3,6},{3,7},{3,10},{4,5},{4,6},{4,9},{4,10},{5,7},{5,9},{5,10},{6,8},  
{6,10},{7,8},{7,11},{8,9},{8,10},{8,11}},{{1,2},{1,3},{1,4},{1,5},  
{1,6},{2,6},{2,7},{2,8},{2,9},{3,5},{3,6},{3,7},{3,10},{4,5},{4,6},  
{4,9},{4,10},{5,7},{5,9},{5,10},{6,8},{6,10},{6,11},{7,8},{8,9},  
{8,10},{8,11},{10,11}},{{1,2},{1,3},{1,4},{1,5},{1,6},{2,6},{2,7},  
{2,8},{2,9},{3,5},{3,6},{3,7},{3,10},{3,11},{4,5},{4,6},{4,9},{4,10},  
{5,7},{5,9},{5,10},{5,11},{6,8},{6,10},{7,8},{7,11},{8,9},{8,10}},  
{{1,2},{1,3},{1,4},{1,5},{1,6},{2,6},{2,7},{2,8},{2,9},{2,11},{3,5},  
{3,6},{3,7},{3,10},{4,5},{4,6},{4,9},{4,10},{5,7},{5,9},{5,10},{6,8},  
{6,10},{6,11},{7,8},{8,9},{8,10},{8,11}},{{1,4},{1,6},{1,7},{1,8},  
{1,9},{2,5},{2,6},{2,8},{2,9},{2,10},{3,6},{3,7},{3,9},{3,10},{4,6},  
{4,7},{4,8},{4,10},{4,11},{5,7},{5,8},{5,9},{5,10},{6,9},{6,10},  
{6,11},{7,9},{7,10},{10,11}},{{1,4},{1,7},{1,8},{1,9},{1,10},{2,5},  
{2,7},{2,9},{2,10},{2,11},{3,6},{3,7},{3,10},{3,11},{4,7},{4,8},{4,9},  
{4,11},{5,8},{5,9},{5,10},{5,11},{6,8},{6,10},{6,11},{7,10},{7,11},  
{8,10},{8,11}},{{1,5},{1,7},{1,8},{1,9},{1,10},{2,6},{2,7},{2,9},  
{2,10},{2,11},{3,6},{3,8},{3,10},{3,11},{4,8},{4,9},{4,10},{4,11},  
{5,7},{5,8},{5,9},{5,11},{6,7},{6,10},{6,11},{8,10},{8,11},{9,10},  
{9,11}},{{1,4},{1,5},{1,8},{1,9},{1,10},{2,6},{2,7},{2,8},{2,10},  
{2,11},{3,6},{3,7},{3,9},{3,10},{3,11},{4,5},{4,8},{4,11},{5,9},  
{5,11},{6,8},{6,10},{6,11},{7,9},{7,10},{7,11},{8,10},{8,11},{9,10},  
{9,11}},{{1,4},{1,5},{1,7},{1,10},{1,11},{2,5},{2,6},{2,8},{2,9},  
{2,10},{2,11},{3,6},{3,7},{3,9},{3,11},{4,8},{4,10},{4,11},{5,7},  
{5,9},{5,10},{5,11},{6,8},{6,9},{6,11},{7,9},{7,11},{8,10},{8,11},  
{9,10}},{{1,4},{1,6},{1,8},{1,10},{1,11},{2,5},{2,8},{2,9},{2,10},  
{3,6},{3,7},{3,9},{3,10},{3,11},{4,7},{4,8},{4,10},{4,11},{5,8},{5,9},  
{5,11},{6,9},{6,10},{6,11},{7,10},{7,11},{8,10},{8,11},{9,10},{9,11}},  
{{1,4},{1,6},{1,8},{1,9},{1,10},{2,5},{2,6},{2,10},{2,11},{3,6},{3,7},  
{3,8},{3,9},{3,11},{4,7},{4,8},{4,9},{4,10},{4,11},{5,7},{5,10},  
{5,11},{6,8},{6,10},{6,11},{7,9},{7,10},{7,11},{8,9},{8,11}},{{1,5},  
{1,6},{1,8},{1,9},{1,10},{2,5},{2,7},{2,9},{2,10},{2,11},{3,6},{3,7},  
{3,8},{3,9},{3,11},{4,6},{4,7},{4,8},{4,10},{4,11},{5,9},{5,10},{6,8},  
{6,9},{6,11},{7,8},{7,10},{7,11},{8,10},{9,11}},{{1,5},{1,6},{1,8},  
{1,10},{1,11},{2,5},{2,6},{2,9},{2,10},{2,11},{3,7},{3,8},{3,9},  
{3,10},{4,7},{4,8},{4,9},{4,11},{5,8},{5,10},{5,11},{6,9},{6,10},  
{6,11},{7,8},{7,9},{8,10},{8,11},{9,10},{9,11}},{{1,5},{1,6},{1,8},  
{1,10},{1,11},{2,5},{2,7},{2,9},{2,10},{2,11},{3,6},{3,9},{3,10},  
{3,11},{4,7},{4,8},{4,10},{4,11},{5,10},{5,11},{6,8},{6,10},{6,11},  
{7,9},{7,10},{7,11},{8,10},{8,11},{9,10},{9,11}},{{1,5},{1,6},{1,8},  
{1,10},{1,11},{2,5},{2,7},{2,10},{2,11},{3,6},{3,8},{3,9},{3,10},  
{3,11},{4,7},{4,9},{4,10},{4,11},{5,8},{5,10},{5,11},{6,9},{6,10},  
{6,11},{7,10},{7,11},{8,10},{8,11},{9,10},{9,11}},{{1,4},{1,5},{1,8},  
{1,9},{1,10},{2,5},{2,6},{2,8},{2,9},{2,11},{3,6},{3,7},{3,8},{3,10},  
{3,11},{4,7},{4,9},{4,10},{5,8},{5,9},{5,10},{5,11},{6,8},{6,11},  
{7,9},{7,10},{7,11},{8,10},{9,11},{10,11}},{{1,4},{1,5},{1,8},{1,10},  
{1,11},{2,5},{2,6},{2,8},{2,9},{2,10},{3,6},{3,7},{3,10},{3,11},{4,7},  
{4,8},{4,9},{4,10},{4,11},{5,8},{5,9},{5,11},{6,9},{6,10},{6,11},  
{7,10},{7,11},{8,9},{8,10},{9,11}},{{1,4},{1,5},{1,6},{1,7},{1,9},

{2,5},{2,6},{2,8},{2,9},{2,10},{2,11},{3,6},{3,7},{3,8},{3,9},{3,10},  
 {4,5},{4,7},{4,8},{4,10},{5,8},{5,9},{6,7},{6,9},{6,10},{7,10},{8,9},  
 {8,10},{8,11},{10,11}},{{1,4},{1,5},{1,6},{1,7},{1,9},{2,5},{2,6},  
 {2,8},{2,9},{2,10},{3,6},{3,7},{3,8},{3,9},{3,10},{4,5},{4,7},{4,8},  
 {4,10},{4,11},{5,8},{5,9},{6,7},{6,9},{6,10},{7,10},{8,9},{8,10},  
 {8,11},{10,11}},{{1,4},{1,5},{1,7},{1,8},{1,9},{1,10},{2,5},{2,6},  
 {2,7},{2,9},{2,10},{2,11},{3,6},{3,8},{3,10},{4,6},{4,7},{4,8},{4,9},  
 {5,8},{5,9},{5,10},{5,11},{6,7},{6,8},{6,10},{7,9},{7,10},{8,10},  
 {10,11}},{{1,4},{1,5},{1,7},{1,8},{1,9},{1,10},{2,5},{2,6},{2,7},  
 {2,9},{2,10},{2,11},{3,6},{3,8},{3,10},{4,7},{4,10},{5,8},{5,9},  
 {5,10},{5,11},{6,7},{6,8},{6,9},{6,10},{7,9},{7,10},{8,9},{8,10},  
 {9,11}},{{1,4},{1,5},{1,7},{1,8},{1,9},{1,10},{2,5},{2,6},{2,7},{2,9},  
 {2,10},{2,11},{3,6},{3,8},{3,10},{4,7},{4,10},{5,8},{5,9},{5,10},  
 {5,11},{6,7},{6,8},{6,9},{6,10},{7,9},{7,10},{8,9},{8,10},{10,11}},  
 {{1,4},{1,5},{1,7},{1,8},{1,9},{1,10},{2,5},{2,6},{2,7},{2,9},{2,10},  
 {3,6},{3,8},{3,10},{4,6},{4,7},{4,8},{4,9},{4,11},{5,8},{5,9},{5,10},  
 {6,7},{6,8},{6,10},{6,11},{7,9},{7,10},{7,11},{8,10}},{{1,4},{1,5},  
 {1,7},{1,8},{1,9},{1,10},{2,5},{2,6},{2,8},{2,9},{2,10},{2,11},{3,6},  
 {3,7},{3,9},{3,10},{4,8},{4,10},{5,7},{5,9},{5,10},{5,11},{6,8},{6,9},  
 {6,10},{7,9},{7,10},{8,9},{8,10},{10,11}},{{1,4},{1,5},{1,7},{1,8},  
 {1,9},{2,4},{2,6},{2,7},{2,9},{2,10},{2,11},{3,5},{3,6},{3,8},{3,9},  
 {3,10},{4,7},{4,8},{4,10},{5,7},{5,8},{5,9},{5,10},{6,9},{6,10},  
 {6,11},{7,9},{7,10},{8,10},{9,11}},{{1,4},{1,5},{1,7},{1,8},{1,9},  
 {2,4},{2,6},{2,7},{2,9},{2,10},{2,11},{3,5},{3,6},{3,8},{3,9},{3,10},  
 {4,7},{4,8},{4,10},{5,7},{5,8},{5,9},{5,10},{6,9},{6,10},{6,11},{7,9},  
 {7,10},{8,10},{10,11}},{{1,4},{1,5},{1,7},{1,8},{1,9},{2,4},{2,6},  
 {2,7},{2,9},{2,10},{2,11},{3,5},{3,6},{3,8},{3,9},{3,10},{4,7},{4,8},  
 {4,10},{5,7},{5,8},{5,9},{5,10},{6,9},{6,10},{7,9},{7,10},{7,11},  
 {8,10},{9,11}},{{1,4},{1,5},{1,7},{1,8},{1,9},{2,4},{2,6},{2,7},{2,9},  
 {2,10},{3,5},{3,6},{3,8},{3,9},{3,10},{4,7},{4,8},{4,10},{4,11},{5,7},  
 {5,8},{5,9},{5,10},{6,9},{6,10},{7,9},{7,10},{8,10},{8,11},{10,11}},  
 {{1,4},{1,5},{1,7},{1,8},{1,10},{1,11},{2,4},{2,6},{2,9},{3,5},{3,6},  
 {3,7},{3,8},{3,9},{3,10},{4,6},{4,7},{4,9},{4,10},{5,7},{5,8},{5,9},  
 {5,11},{6,8},{6,9},{6,10},{7,9},{7,10},{8,10},{8,11}},{{1,4},{1,5},  
 {1,7},{1,8},{1,10},{2,4},{2,6},{2,9},{3,5},{3,6},{3,7},{3,8},{3,9},  
 {3,10},{3,11},{4,6},{4,7},{4,9},{4,10},{5,7},{5,8},{5,9},{6,8},{6,9},  
 {6,10},{7,9},{7,10},{7,11},{8,10},{10,11}},{{1,4},{1,5},{1,7},{1,8},  
 {1,10},{2,4},{2,6},{2,9},{3,5},{3,6},{3,7},{3,8},{3,9},{3,10},{4,6},  
 {4,7},{4,9},{4,10},{4,11},{5,7},{5,8},{5,9},{6,8},{6,9},{6,10},{7,9},  
 {7,10},{7,11},{8,10},{9,11}},{{1,4},{1,5},{1,7},{1,9},{1,10},{2,4},  
 {2,6},{2,9},{2,10},{2,11},{3,5},{3,6},{3,7},{3,8},{3,9},{3,10},{4,6},  
 {4,7},{4,8},{4,10},{4,11},{5,7},{5,8},{5,9},{6,8},{6,9},{7,8},{7,10},  
 {9,10},{10,11}},{{1,4},{1,5},{1,7},{1,9},{1,10},{2,4},{2,6},{2,9},  
 {2,10},{2,11},{3,5},{3,6},{3,7},{3,8},{3,9},{3,10},{4,6},{4,7},{4,8},  
 {4,10},{5,7},{5,8},{5,9},{6,8},{6,9},{6,11},{7,8},{7,10},{9,10},  
 {9,11}},{{1,4},{1,5},{1,7},{1,9},{1,10},{2,4},{2,6},{2,9},{2,10},  
 {3,5},{3,6},{3,7},{3,8},{3,9},{3,10},{3,11},{4,6},{4,7},{4,8},{4,10},  
 {5,7},{5,8},{5,9},{6,8},{6,9},{6,11},{7,8},{7,10},{9,10},{9,11}},  
 {{1,4},{1,5},{1,7},{1,9},{1,10},{2,4},{2,6},{2,9},{2,10},{3,5},{3,6},  
 {3,7},{3,8},{3,9},{3,10},{3,11},{4,6},{4,7},{4,8},{4,10},{5,7},{5,8},

{5,9},{6,8},{6,9},{7,8},{7,10},{9,10},{9,11},{10,11}},{{1,4},{1,5},  
 {1,7},{1,9},{1,10},{2,4},{2,6},{2,9},{2,10},{3,5},{3,6},{3,7},{3,8},  
 {3,9},{3,10},{4,6},{4,7},{4,8},{4,10},{4,11},{5,7},{5,8},{5,9},{6,8},  
 {6,9},{6,11},{7,8},{7,10},{8,11},{9,10}},{{1,4},{1,5},{1,7},{1,9},  
 {1,10},{2,5},{2,6},{2,8},{2,9},{2,10},{2,11},{3,6},{3,7},{3,9},{3,10},  
 {4,8},{4,9},{4,10},{5,7},{5,9},{5,10},{5,11},{6,8},{6,9},{6,10},{7,9},  
 {7,10},{8,9},{8,10},{10,11}},{{1,4},{1,5},{1,8},{1,9},{1,10},{1,11},  
 {2,5},{2,6},{2,7},{2,9},{2,10},{3,6},{3,7},{3,8},{3,9},{3,10},{4,8},  
 {4,10},{5,7},{5,9},{5,10},{5,11},{6,8},{6,9},{6,10},{7,9},{7,10},  
 {8,9},{8,10},{9,11}},{{1,4},{1,5},{1,8},{1,9},{1,10},{1,11},{2,5},  
 {2,6},{2,7},{2,9},{2,10},{3,6},{3,7},{3,8},{3,9},{3,10},{4,8},{4,10},  
 {5,7},{5,9},{5,10},{6,8},{6,9},{6,10},{7,9},{7,10},{8,9},{8,10},  
 {8,11},{9,11}},{{1,4},{1,5},{1,8},{1,9},{1,10},{2,5},{2,6},{2,7},  
 {2,9},{2,10},{3,6},{3,7},{3,8},{3,9},{3,10},{3,11},{4,8},{4,10},{5,7},  
 {5,9},{5,10},{6,8},{6,9},{6,10},{7,9},{7,10},{7,11},{8,9},{8,10},  
 {10,11}},{{1,4},{1,5},{1,9},{1,10},{1,11},{2,5},{2,6},{2,7},{2,9},  
 {2,10},{3,6},{3,7},{3,8},{3,9},{3,10},{4,8},{4,9},{4,10},{4,11},{5,7},  
 {5,9},{5,10},{6,8},{6,9},{6,10},{7,9},{7,10},{8,9},{8,10},{9,11}},  
 {{1,4},{1,5},{1,9},{1,10},{2,5},{2,6},{2,7},{2,9},{2,10},{3,6},{3,7},  
 {3,8},{3,9},{3,10},{3,11},{4,8},{4,9},{4,10},{5,7},{5,9},{5,10},{6,8},  
 {6,9},{6,10},{7,9},{7,10},{7,11},{8,9},{8,10},{9,11}},{{1,4},{1,5},  
 {1,9},{1,10},{2,5},{2,6},{2,7},{2,9},{2,10},{3,6},{3,7},{3,8},{3,9},  
 {3,10},{4,8},{4,9},{4,10},{4,11},{5,7},{5,9},{5,10},{6,8},{6,9},  
 {6,10},{7,9},{7,10},{8,9},{8,10},{8,11},{9,11}},{{1,4},{1,7},{1,8},  
 {1,9},{1,11},{2,5},{2,6},{2,7},{2,9},{2,10},{3,5},{3,6},{3,8},{3,9},  
 {3,10},{4,7},{4,8},{4,10},{4,11},{5,7},{5,9},{5,10},{6,8},{6,9},  
 {6,10},{7,9},{7,10},{7,11},{8,9},{8,10}},{{1,4},{1,7},{1,8},{1,9},  
 {2,5},{2,6},{2,7},{2,9},{2,10},{2,11},{3,5},{3,6},{3,8},{3,9},{3,10},  
 {4,7},{4,8},{4,10},{5,7},{5,9},{5,10},{6,8},{6,9},{6,10},{6,11},{7,9},  
 {7,10},{8,9},{8,10},{10,11}},{{1,5},{1,6},{1,7},{1,9},{1,10},{2,5},  
 {2,6},{2,8},{2,9},{3,5},{3,7},{3,8},{3,10},{3,11},{4,6},{4,7},{4,8},  
 {4,9},{4,10},{5,7},{5,8},{5,9},{5,11},{6,8},{6,9},{6,10},{7,9},{7,10},  
 {7,11},{8,10}},{{1,6},{1,7},{1,8},{1,9},{1,11},{2,6},{2,7},{2,9},  
 {2,10},{2,11},{3,6},{3,8},{3,9},{3,10},{4,7},{4,8},{4,10},{4,11},  
 {5,8},{5,9},{5,10},{5,11},{6,7},{6,9},{7,11},{8,10},{9,11}},{{1,4},  
 {1,6},{1,7},{1,9},{1,10},{2,5},{2,9},{2,10},{2,11},{3,6},{3,7},{3,8},  
 {3,9},{3,11},{4,7},{4,8},{4,10},{4,11},{5,9},{5,10},{5,11},{6,8},  
 {6,9},{6,10},{7,9},{7,11},{8,10},{8,11},{9,10},{9,11},{10,11}},{{1,5},  
 {1,6},{1,8},{1,9},{1,11},{2,5},{2,6},{2,8},{2,10},{2,11},{3,7},{3,9},  
 {3,10},{3,11},{4,7},{4,9},{4,10},{4,11},{5,8},{5,9},{5,11},{6,8},  
 {6,10},{6,11},{7,9},{7,10},{7,11},{8,9},{8,10},{9,10},{9,11},{10,11}},  
 {{1,4},{1,5},{1,8},{1,10},{1,11},{2,6},{2,7},{2,8},{2,9},{2,11},{3,6},  
 {3,7},{3,9},{3,10},{3,11},{4,5},{4,8},{4,10},{4,11},{5,10},{5,11},  
 {6,8},{6,9},{6,11},{7,9},{7,10},{7,11},{8,9},{8,10},{8,11},{9,10},  
 {10,11}}
